# Supplementary material for: High-dimensional statistical inference for linkage disequilibrium score regression and its cross-ancestry extensions
Source: arXiv:2306.15779 source file (2025-04-15)
Supplement: Supplementary file 1 [file Supplement_aos.pdf]

*Submitted to the Annals of Statistics*

# SUPPLEMENT TO "HIGH-DIMENSIONAL STATISTICAL INFERENCE FOR LINKAGE DISEQUILIBRIUM SCORE REGRESSION AND ITS CROSS-ANCESTRY EXTENSIONS"

BY FEI XUE[1,a] AND BINGXIN ZHAO[2,b]

[1]*Department of Statistics, Purdue University,* [a]*feixue@purdue.edu*

[2]*Department of Statistics and Data Science, University of Pennsylvania,* [b]*bxzhao@upenn.edu*

## S1. Supplementary Note.

S1.1. *Technical comparison between LDSC and other existing methods.* Many methods have been proposed for heritability estimation, including [11], GWASH [34], PCGC [16], MQS [56], LDSC [6], GRE [21], EstHer [2], SumHer [40], CHIVE [43], and Mahalanobis distance-based approaches [27]. Among these, LDSC [6] has become one of the most popular methods in real data applications, with several subsequent extensions, including HDL [29], LDER [39], i-LDSC [38], and d-LDSC [31]. For example, HDL [29] and LDER [39] enhance LDSC's statistical efficiency by comprehensively incorporating the LD matrix across the genome. Additionally, i-LDSC [38] and d-LDSC [31] introduce models for genetic non-additive interactions and dominance, respectively. Compared to LDSC [6], SumHer [40] and GRE [21] relax assumptions about genetic effects, offering greater flexibility across different genetic architectures. Several of these heritability estimation methods, including LDSC [6], HDL [29], LDER [39], and SumHer [40], have been extended to perform bivariate analysis of genetic covariance using summary data. Additionally, there are methods specifically designed for genetic covariance estimation, such as GNOVA [26], FDEs [18], as well as methods proposed by [45] and [55].

Among existing methods, those most related to LDSC [6] are the method of moments (MoM) estimators in [11, 45, 26, 27, 34, 56], as they are all conceptually linked to the Haseman-Elston regression [19]. To help readers understand their connections and differences, we have focused on two existing methods with established theoretical properties and provided a technical comparison with LDSC [6]. The first one is [11] for genetic variance estimation, and the second one is [45] for both genetic variance and covariance estimation. Although these methods can all accept GWAS summary statistics as input, there are several key differences due to the nature of the proposed estimators and the modeling frameworks used. These differences include whether the methods and derived theoretical properties require consistent estimators of high-dimensional covariance/precision matrices, whether they model the randomness associated with using reference panels, and whether they consider bivariate and cross-ancestry applications. Further details are provided below.

Specifically, [11] proposes two MoM estimators for genetic variance when the population GWAS covariance matrix is unknown. Suppose we consider the estimation of genetic variance of the GWAS-I cohort using $(\boldsymbol{X}_\alpha, \boldsymbol{y}_\alpha)$ and reference panel-I data $\boldsymbol{Z}_\alpha$, the first MoM estimator in [11] can be expressed by

$$\hat{\tau}^2(\widetilde{\boldsymbol{\Sigma}}) = -\frac{p}{n_\alpha(n_\alpha+1)}\|\boldsymbol{y}_\alpha\|^2 + \frac{1}{n_\alpha(n_\alpha+1)}\|\widetilde{\boldsymbol{\Sigma}}^{-1/2}\boldsymbol{X}_\alpha^T\boldsymbol{y}_\alpha\|^2.$$

This estimator requires an estimate for the unknown norm $\|\boldsymbol{y}_\alpha\|^2$ and a positive definite estimator $\widetilde{\boldsymbol{\Sigma}}$ for the covariance matrix $\boldsymbol{\Sigma}_\alpha$, where $\|\cdot\|$ denotes the $\ell^2$ norm. For $\|\boldsymbol{y}_\alpha\|^2$,

it may need to be additionally estimated and provided by the researchers who have access to individual-level data in the GWAS-I cohort. For the positive definite estimator $\widetilde{\mathbf{\Sigma}}$, even leveraging the block-wise LD structure modeled by the present paper, the inverse square root $\widetilde{\mathbf{\Sigma}}^{-1/2}$ across the genome is computationally much more expensive compared to the idea of calculating the marginal LD scores used by the LDSC [6]. Furthermore, [11] does not consider and explicitly model the randomness of reference panels, which has been a common approach to estimate LD-related information. It is not clear whether the $\widetilde{\mathbf{\Sigma}}^{-1/2}$ estimated in hundreds of subjects (which is the typical size of reference panels, such as the 1KG project [1]) is doable and reliable. In addition, the sample covariance matrix is not norm-consistent in general if its dimension is larger than the sample size [34]. On the other hand, LDSC [6] does not require a positive definite estimator or additional information of $\|\boldsymbol{y}_\alpha\|^2$ and is computationally very fast. Using our framework, we also show that LD scores can be estimated by a small reference panel, explaining why a relatively small sample size is sufficient for the reference panel in practical applications.

The second estimator in [11] is

$$\tilde{\tau}^2 = -\frac{p\hat{m}_1^2}{n_\alpha(n_\alpha+1)\hat{m}_2}\|\boldsymbol{y}_\alpha\|^2 + \frac{\hat{m}_1}{n_\alpha(n_\alpha+1)\hat{m}_2}\|\boldsymbol{X}_\alpha^T\boldsymbol{y}_\alpha\|^2,$$

where

$$\hat{m}_1 = \frac{1}{p}\text{tr}(\frac{1}{n_\alpha}\boldsymbol{X}_\alpha^T\boldsymbol{X}_\alpha)$$

and

$$\hat{m}_2 = \frac{1}{p}\text{tr}\{(\frac{1}{n_\alpha}\boldsymbol{X}_\alpha^T\boldsymbol{X}_\alpha)^2\} - \frac{1}{pn_\alpha}\{\text{tr}(\frac{1}{n_\alpha}\boldsymbol{X}_\alpha^T\boldsymbol{X}_\alpha)\}^2.$$

This estimator still needs additional information of $\|\boldsymbol{y}_\alpha\|^2$ but does not require a positive definite covariance matrix estimator. Instead, by [11, Proposition 2], it assumes

$$\sum_{k=1}^{3}|\tau_k^2 - \tau_0^2 m_k| = o_p(n_\alpha^{-1/2})$$

to achieve the asymptotic normality, where $\tau_k^2 = \boldsymbol{\alpha}^T\mathbf{\Sigma}_\alpha^k\boldsymbol{\alpha}$ and $m_k = p^{-1}\text{tr}(\mathbf{\Sigma}_\alpha^k)$ for $k = 0, 1, 2, 3$. This assumption requires that the quadratic form $\tau_k^2 = \boldsymbol{\alpha}^T\mathbf{\Sigma}_\alpha^k\boldsymbol{\alpha}$ can be approximated by the product of the trace of the covariance matrix $\mathbf{\Sigma}_\alpha^k$ and signal strength $\|\boldsymbol{\alpha}\|^2$ for $k = 1, 2, 3$, which is similar to Condition **??** of the present paper required by LDSC [6]. Nevertheless, our Condition **??** mainly requires that for $k = 2$ instead of the higher order approximation with $k = 3$. Furthermore, similar to the first estimator, the role of the reference panel in the asymptotic normality of the proposed method is unclear. In the present paper, we have explicitly modeled the randomness of using external reference panels, which is a major contribution compared to existing theoretical studies of genetic variance and covariance estimation methods.

Next, [45] proposes MoM estimators for both genetic variance and covariance, which are

$$\widehat{Q}_\alpha = \widehat{\boldsymbol{a}}^T\widehat{\mathbf{\Omega}}\widehat{\boldsymbol{a}} - \frac{\text{tr}(\widehat{\mathbf{\Omega}}\widehat{\mathbf{\Sigma}})}{n_\alpha^2}\|\boldsymbol{y}_\alpha\|^2 \quad \text{and} \quad \widehat{I} = \widehat{\boldsymbol{b}}^T\widehat{\mathbf{\Omega}}\widehat{\boldsymbol{a}},$$

respectively. Here $\widehat{\mathbf{\Omega}}$ and $\widehat{\mathbf{\Sigma}}$ are the estimated precision matrix and the sample covariance matrix, respectively, for $\mathbf{\Sigma}_\alpha$ based on a reference panel. According to [45, Theorem 4], the asymptotic normality of the estimators $\widehat{Q}_\alpha$ and $\widehat{I}$ requires that the sample size of the reference panel $n_{r\alpha}$ is much larger than the sample sizes $n_\alpha$ and $n_\beta$ of the GWAS datasets. This may be

hard to achieve in the current practice. In contrast, LDSC [6] allows $n_{r\alpha}$ to be much smaller than $n_\alpha$ and $n_\beta$. This is mainly because the asymptotic normality of $\widehat{Q}_\alpha$ and $\widehat{I}$ requires a consistent precision matrix estimator $\widehat{\mathbf{\Omega}}$, while LDSC [6] does not need that by using the LD scores instead. In addition, when considering the estimation of genetic covariance between two GWAS datasets, [45] assumes that the population covariance matrices of the two GWAS datasets are the same, while in the present study, we provide novel extension of LDSC [6] to allow the two population covariance matrices to be different to conduct cross-ancestry analyses.

An overview of the summary is provided in Supplementary Table 1. In summary, while all these estimators may accept similar input summary data, they differ in their theoretical properties and the conditions required for their applications due to the distinct nature of each proposed estimator. A key difference of the LDSC method is its use of LD scores, which avoids the need to estimate high-dimensional covariance/precision matrices. By leveraging the block patterns of the LD structure, it offers both good computational efficiency and theoretical properties. In addition, the LDSC method has been further extended to perform cross-ancestry analysis in the present study, which can not be performed by the above-mentioned existing methods.

S1.2. *Intercept in LDSC regression.* Recall that, for genetic variance estimation, we have

$$\varepsilon_{a,j} = \frac{n_\alpha + 1}{n_\alpha}\boldsymbol{\alpha}^T(\mathbf{\Sigma}_{\alpha,\cdot j}\mathbf{\Sigma}_{\alpha,\cdot j}^T)\boldsymbol{\alpha} - \sigma_\alpha^2 \cdot \sum_{i=1}^{p}\mathbf{\Sigma}_{\alpha,ij}^2 + \frac{\boldsymbol{\alpha}^T\mathbf{\Sigma}_\alpha\boldsymbol{\alpha} + \sigma_{\epsilon_\alpha}^2}{n_\alpha}.$$

In the original random-effect model [6], it is assumed that $\alpha_i \overset{i.i.d.}{\sim} N(0, \sigma_\alpha^2)$, which implies

$$\boldsymbol{E}\varepsilon_{a,j} = \frac{\sigma_\alpha^2(p + \ell_{a,j}) + \sigma_{\epsilon_\alpha}^2}{n_\alpha}.$$

Under Condition **??** and the assumptions $\sigma_\alpha^2 = O(1)$ and $p = O(n_\alpha)$, the expected value of $\varepsilon_{a,j}$ is bounded above by a constant. That is, the average of all $\varepsilon_{a,j}$'s could be close to a non-zero constant, which differs from the typical linear model setting where the noise term has a mean of zero. This observation suggests that it may be more appropriate to introduce an intercept term in our LDSC regression for genetic variance analysis.

Additionally, it is important to note that the noise term in the bivariate LDSC analysis for genetic covariance in Section **??** already has a mean of zero, primarily due to the non-overlapping samples between the two traits. Specifically, recall that, for genetic covariance, the noise term is

$$\varepsilon_{ab,j} = \sum_{i=1}^{p}\alpha_i\beta_i\mathbf{\Sigma}_{\alpha,ij}\mathbf{\Sigma}_{\beta,ij} - \sigma_{\alpha\beta} \cdot \sum_{i=1}^{p}\mathbf{\Sigma}_{\alpha,ij}\mathbf{\Sigma}_{\beta,ij} + \sum_{i\neq k}\alpha_i\beta_k\mathbf{\Sigma}_{\alpha,ij}\mathbf{\Sigma}_{\beta,kj}.$$

Under the original random-effect model [5] for genetic covariance, it is assumed that

$$\begin{pmatrix}\alpha_i\\ \beta_i\end{pmatrix} \overset{iid}{\sim} N\left(\begin{pmatrix}0\\0\end{pmatrix}, \begin{pmatrix}\sigma_\alpha^2 & \sigma_{\alpha\beta}\\ \sigma_{\alpha\beta} & \sigma_\beta^2,\end{pmatrix}\right),$$

which implies $\boldsymbol{E}\varepsilon_{ab,j} = 0$.

S1.3. *Condition on orthogonality.* In this section, we offer further investigations and insights into the orthogonality assumption in Condition **??**. Since

$$\varepsilon_{a,j} - \mu_{\boldsymbol{\varepsilon}_a} = \frac{n_\alpha + 1}{n_\alpha}\boldsymbol{\alpha}^T\left(\mathbf{\Sigma}_{\alpha,\cdot j}\mathbf{\Sigma}_{\alpha,\cdot j}^T - \frac{1}{p}\mathbf{\Sigma}_\alpha^2\right)\boldsymbol{\alpha} - \sigma_\alpha^2 \cdot (\ell_{a,j} - \mu_{\boldsymbol{\ell}_a}),$$

we have

$$
\begin{aligned}
\boldsymbol{\ell}_a^T \boldsymbol{H} \boldsymbol{\varepsilon}_a =& \sum_{j=1}^{p} [(\ell_{a,j} - \mu_{\boldsymbol{\ell}_a})(\varepsilon_{a,j} - \mu_{\boldsymbol{\varepsilon}_a})] \\
=& \frac{n_\alpha + 1}{n_\alpha} \sum_{i,j=1}^{p} \alpha_i^2 \left( \boldsymbol{\Sigma}_{\alpha,ij}^2 - \frac{1}{p} \ell_{a,i} \right) (\ell_{a,j} - \mu_{\boldsymbol{\ell}_a}) - \sigma_\alpha^2 \cdot \sum_{j=1}^{p} (\ell_{a,j} - \mu_{\boldsymbol{\ell}_a})^2 \\
&+ \frac{n_\alpha + 1}{n_\alpha} \sum_{i \neq k} \alpha_i \alpha_k \sum_{j=1}^{p} \left( \boldsymbol{\Sigma}_{\alpha,ij} \boldsymbol{\Sigma}_{\alpha,kj} - \frac{1}{p} \sum_{s=1}^{p} \boldsymbol{\Sigma}_{\alpha,is} \boldsymbol{\Sigma}_{\alpha,ks} \right) (\ell_{a,j} - \mu_{\boldsymbol{\ell}_a}).
\end{aligned}
$$

Under the original random-effect framework with $\alpha_i \overset{i.i.d.}{\sim} N(0, \sigma_\alpha^2)$, we have

$$
\boldsymbol{E} \left( \frac{\boldsymbol{\ell}_a^T \boldsymbol{H} \boldsymbol{\varepsilon}_a}{p^{1/2}} \right) = \frac{p^{1/2} \sigma_\alpha^2}{n_\alpha} \cdot \frac{1}{p} \sum_{j=1}^{p} (\ell_{a,j} - \mu_{\boldsymbol{\ell}_a})^2.
$$

Note that $\max_{1 \le j \le p} |\ell_{a,j}| = O(1)$ and $|\mu_{\boldsymbol{\ell}_a}| = O(1)$ under Condition **??**. This implies

$$
\frac{p^{1/2} \sigma_\alpha^2}{n_\alpha} \cdot \frac{1}{p} \sum_{j=1}^{p} (\ell_{a,j} - \mu_{\boldsymbol{\ell}_a})^2 \to 0
$$

as $n_\alpha \to \infty$ when $\sigma_\alpha^2 = O(1)$ and $p = O(n_\alpha)$. That is, under Condition **??** and assumptions $\sigma_\alpha^2 = O(1)$ and $p = O(n_\alpha)$, the expected value of $\boldsymbol{\ell}_a^T \boldsymbol{H} \boldsymbol{\varepsilon}_a / p^{1/2}$ approaches zero, ensuring the expected level of orthogonality.

Now, let us consider our more general fixed-effects model. Recall that $\sigma_\alpha^2 = \boldsymbol{\alpha}^T \boldsymbol{\alpha} / p$. Define $\boldsymbol{A}_j = \boldsymbol{\Sigma}_{\alpha,\cdot j} \boldsymbol{\Sigma}_{\alpha,\cdot j}^T - \boldsymbol{\Sigma}_\alpha^2 / p$. Then $\text{tr}(\boldsymbol{A}_j) = \ell_{a,j} - \mu_{\boldsymbol{\ell}_a}$ and we can rewrite $\varepsilon_{a,j} - \mu_{\boldsymbol{\varepsilon}_a}$ as

$$
\varepsilon_{a,j} - \mu_{\boldsymbol{\varepsilon}_a} = \frac{n_\alpha + 1}{n_\alpha} \boldsymbol{\alpha}^T \boldsymbol{A}_j \boldsymbol{\alpha} - \boldsymbol{\alpha}^T \boldsymbol{\alpha} \cdot \frac{\text{tr}(\boldsymbol{A}_j)}{p}.
$$

Consider

$$
\frac{|\boldsymbol{\ell}_a^T \boldsymbol{H} \boldsymbol{\varepsilon}_a|}{p^{1/2}} = \frac{1}{p^{1/2}} \left| \sum_{j=1}^{p} [(\ell_{a,j} - \mu_{\boldsymbol{\ell}_a})(\varepsilon_{a,j} - \mu_{\boldsymbol{\varepsilon}_a})] \right| \le \left[ \frac{1}{p} \sum_{j=1}^{p} (\ell_{a,j} - \mu_{\boldsymbol{\ell}_a})^2 \sum_{j=1}^{p} (\varepsilon_{a,j} - \mu_{\boldsymbol{\varepsilon}_a})^2 \right]^{1/2}.
$$

Intuitively, this suggests that the orthogonality assumption $\left| \boldsymbol{\ell}_a^T \boldsymbol{H} \boldsymbol{\varepsilon}_a \right| = o(p^{1/2})$ in Condition **??** can be satisfied when the variation in LD scores is not too large, and when $\boldsymbol{\alpha}^T \boldsymbol{\alpha} \cdot [\text{tr}(\boldsymbol{A}_j)/p]$ can adequately approximate $\boldsymbol{\alpha}^T \boldsymbol{A}_j \boldsymbol{\alpha}$.

More technically, $\boldsymbol{\ell}_a^T \boldsymbol{H} \boldsymbol{\varepsilon}_a / p^{1/2}$ can be expressed as $\boldsymbol{\ell}_a^T \boldsymbol{H} \boldsymbol{\varepsilon}_a / p^{1/2} = \boldsymbol{\alpha}^T \boldsymbol{B} \boldsymbol{\alpha}$, where

$$
\boldsymbol{B} = \frac{1}{\sqrt{p}} \sum_{j=1}^{p} \text{tr}(\boldsymbol{A}_j) \cdot \left[ \frac{n_\alpha + 1}{n_\alpha} \boldsymbol{A}_j - \frac{\text{tr}(\boldsymbol{A}_j)}{p} \boldsymbol{I}_p \right].
$$

Note that

$$
\text{tr}(\boldsymbol{B}) = \frac{1}{n_\alpha \sqrt{p}} \sum_{j=1}^{p} [\text{tr}(\boldsymbol{A}_j)]^2 = \frac{1}{n_\alpha \sqrt{p}} \sum_{j=1}^{p} (\ell_{a,j} - \mu_{\boldsymbol{\ell}_a})^2
$$

goes to zero as $n_\alpha \to \infty$ under the assumption $p = O(n_\alpha)$ and Condition **??**, implying that the eigenvalues of $\boldsymbol{B}$ are all very small or can be cancelled out. This ensures that there exists a $\boldsymbol{\alpha}$ such that $\boldsymbol{\alpha}^T \boldsymbol{B} \boldsymbol{\alpha}$ approaches zero. Thus, the orthogonality assumption $\left| \boldsymbol{\ell}_a^T \boldsymbol{H} \boldsymbol{\varepsilon}_a \right| = o(p^{1/2})$ essentially requires $\boldsymbol{\alpha}$ to have this property.

S1.4. *Analyzing a small set of genetic variants.* Our theoretical results suggest that LDSC may face challenges when the number of genetic variants $p$ is small, such as when working with a small subset of genetic variants defined by functional annotations [3]. Specifically, there may be increased uncertainty in LDSC estimates, compromising their reliability and accuracy. These findings align with numerical observations in the stratified LDSC (SLDSC) applications [13, 14]. Particularly, [41] used numerical simulations to illustrate potential issues with SLDSC when the annotation files are small. In general, they suggest that the SLDSC framework is suitable for analyzing large annotations that contain approximately $0.5\%$ or more genetic variants. For example, given a GWAS sample size of $50{,}000$, extensive numerical analyses suggest that standard stratified LDSC analyses may be performed only on annotations covering at least $1.7\%$ of $0.01$ cM genome blocks [41].

We evaluate the size of a wide range of existing functional annotations. For the 52 categories of baseline models provided by SLDSC [13], we find that their sizes vary widely, ranging from $0.55\%$ to $76.5\%$ (Supplementary Figure 18A). Therefore, these baseline annotations may have different degrees of statistical power in analysis. In contrast, annotations of tissue and cell type-specific regulatory elements from the Roadmap Epigenomics Consortium [24] have more comparable sizes, ranging from $2.62\%$ to $10.8\%$ (Supplementary Figure 18B). SLDSC analysis of these Roadmap functional annotations may be reliable, and importantly, it may make sense to compare the statistical significance across different tissues and cell types and report the top-ranking ones (a typical strategy used in the SLDSC analysis), as their annotation sizes are comparable. We further evaluate functional annotations from more refined regions and at the cell type levels, an emerging field in functional genomics. First, we examine the chromatin accessibility data from neurons and glia brain cell types sampled from 14 cortical and subcortical brain regions [15]. Naturally, these functional annotations have much smaller sizes, ranging from $0.50\%$ to $1.96\%$ (Supplementary Figure 18C). Second, we look at the chromatin accessibility of two neuron subtypes (GABAergic and glutamatergic neurons) and two glial subtypes (oligodendrocytes and microglia) [20], which have even smaller sizes, ranging from $0.33\%$ to $0.81\%$ (Supplementary Figure 18D). In summary, we find that the majority of existing functional annotations have over $0.5\%$ of genetic variants, suggesting that our developed theoretical results are applicable to these applications. However, smaller annotations also exist and are expected to become more prevalent with emerging data resources that provide fine-grained details in functional genomics, such as single-cell RNAseq data [12]. Additionally, when screening many functional annotations and reporting the top-ranking ones based on their significance levels, this approach may be more suitable for functional annotations with comparable sizes.

Analyzing the local genetic architecture of a small subset of genetic variants, including the SLDSC functional annotation analysis discussed above, is a fundamental area in statistical genetics and genomics. Here we discuss existing efforts in these fields and provide suggestions for practical data analysis and future directions. We primarily focus on two areas: (i) connecting GWAS to tissue and cell types, which examines the biological insights into GWAS signals by integrating functional genomic data; and (ii) local genetic correlation and heritability analyses, which focus on window size or LD-defined local genomic regions.

In addition to SLDSC, methods such as CELLEX [42], DIALOGUE [23], EPIC [46], EWCE [37], MAGMA-set/FUMA [47], RolyPoly [8], sc-linker [22], and scDRS [51] have been proposed to connect GWAS results to functional genomic data (such as from different tissue and cell types) and may yield results similar to SLDSC analysis. Some of these methods differ from SLDSC's genetic variant-level regression by using gene-level regression (e.g., MAGMA-set [47]) or per-cell scoring methods (e.g., scDRS [51]). For example, MAGMA-set [47] applies specificity metrics to define gene set-based annotations before integrating them with GWAS summary statistics for gene-level regression. In addition, unlike SLDSC

and MAGMA-set [47], which first use functional genomic data to define annotations and then link to GWAS summary statistics, scDRS [51] is annotation-free. Briefly, scDRS [51] uses an opposite approach by first selecting a set of top-ranking associated genes from GWAS signals and then calculating polygenic disease enrichment in each cell type. In summary, these gene-level and annotation-free alternative analyses may work better when the annotations are small. We suggest exploring these methods for small annotations to see if they provide convergent evidence with SLDSC. As GWAS power continues to increase, methods that start from the GWAS signals to link to functional data (instead of using functional data to define genome annotations) may have more stable performance.

Furthermore, given that genome-wide genetic variance and covariance estimators (such as LDSC) do not easily translate to a local scale, various methods have been developed specifically for local analyses at each genomic region, such as HESS [35], rho-HESS [36], SUPERGNOVA [52], LOGOdetect [17], LAVA [48], and HEELS [25]. For example, HESS [35] treats genetic effect sizes as fixed effects and projects their estimates onto the eigenvectors derived from the truncated singular value decomposition (SVD) of the LD matrix at the specific locus/region. A key assumption is that truncated SVD acts as an appropriate regularization method to manage noise in the estimated LD matrices. Similar SVD-based approaches are used in the recently proposed LAVA [48] and HEELS [25] methods. We suggest using these methods for local heritability and genetic correlation analysis. It would be interesting to benchmark these methods through numerical analysis and explore their theoretical properties in future research [50].

S1.5. *Alternative definitions of genetic variance and covariance.* In this paper, we use the definition of genetic variance and covariance proposed by the LDSC [6, 5] and GREML [49]. While these definitions are broadly used, alternative definitions may better model intricate genetic architecture. In this section, we discuss the performance of LDSC under alternative definitions, focusing mainly on two directions: indirect genetic effects [54, 45] and frequency-dependent genetic effects [33, 28, 40].

First, for fixed genetic effects, we may have two definitions of genetic variances and covariances with different biological meanings, as discussed in [45]. Briefly, the terms $g_\alpha^2 = \boldsymbol{\alpha}^\top\boldsymbol{\alpha}$ and $g_{\alpha\beta} = \boldsymbol{\alpha}^\top\boldsymbol{\beta}$ represent the "pleiotropic genetic effect" version, which considers the direct genetic effects from genetic variants to phenotypes. Alternatively, the second definition is given by $g_\alpha^{2*} = \boldsymbol{\alpha}^\top\boldsymbol{\Sigma}\boldsymbol{\alpha}$ and $g_{\alpha\beta}^* = \boldsymbol{\alpha}^\top\boldsymbol{\Sigma}\boldsymbol{\beta}$, which includes additionally indirect genetic effects of variants on traits induced by LD structure (See Figure 1 of [45]). Both versions are biologically meaningful and popular in existing methods and real data applications, including cross-ancestry genetic analysis. For example, the "pleiotropic effect" version is referred to as "genetic-effect correlation" in tools such as Popcorn [4] for transethnic genetic correlation estimation and has been used as the default option.

The popular LDSC and GREML estimators are developed using the "pleiotropic effect" version. Therefore, we continue to use this definition in the present paper. Furthermore, [53] highlights the connections between the two versions on a technical level. Briefly, for genetic covariance, it can be shown that

$$g_{\alpha\beta}^* = g_{\alpha\beta} \cdot c(\boldsymbol{\Sigma}) + o_p(1),$$

where $c(\boldsymbol{\Sigma})$ is a constant related to the first moment of the eigenvalue distribution of the LD matrix $\boldsymbol{\Sigma}$. Therefore, by using a consistent estimator of $c(\boldsymbol{\Sigma})$, we can obtain a consistent estimator of $g_{\alpha\beta}^*$ by using the LDSC-based estimator of $g_{\alpha\beta}$. Similar results also hold for genetic variance $g_\alpha^{2*}$. Practical approaches to estimate $c(\boldsymbol{\Sigma})$ have been provided in [53]. It is also worth mentioning that the $c(\boldsymbol{\Sigma})$ terms in genetic variance and genetic covariance may largely cancel out when calculating genetic correlation. Therefore, the main difference

between the two definitions may exist in heritability estimation, while for genetic correlation estimation, they may provide similar results.

Second, we can consider the general trend of negative selection on complex trait architecture by inducing a relationship between minor allele frequency (MAF) and effect size [33], such as in SumHer [40]. Considering the same setups in our HAPNEST data analysis in Section **??**, we have evaluated the performance of LDSC given the MAF-effect size dependence in two ancestry cohorts. Specifically, we set heritability and genetic correlation as $0.5$ and vary the $\alpha$ parameter defined in [33] from $-1$, $-0.6$, to $-0.3$. Other settings remain are the same. Here $\alpha = -1$ corresponds to the LDSC definition without accounting for negative selection and larger $\alpha$ indicates stronger negative selection. There are several interesting observations (Supplementary Figure 16). First, in the presence of negative selection, LDSC tends to produce biased heritability estimates in both 1KG-EUR-like and 1KG-EAS-like populations. This bias occurs regardless of the window size used ("1MB-Window" and "2MB-Window") and is stronger when the GWAS sample size increases from $16{,}800$ to $168{,}000$. The bias in heritability estimates of 1KG-EUR-like population is larger than that in 1KG-EAS-like population. Second, different from heritability estimates, the estimates of genetic correlation are largely unbiased. This could be due to both genetic variance and covariance being biased, thus canceling each other out when calculating genetic correlation. This observation is consistent with findings from [40], which also reported that LDSC may produce biased heritability estimates under negative control, but genetic correlation estimates remain more robust. In summary, when there is strong evidence of negative selection, other methods, such as SumHer [40], may provide better heritability estimation. However, LDSC and its cross-ancestry extensions may still be robust in genetic correlation estimation under this alternative assumption across different degrees of negative controls.

S1.6. *Biobank Japan data analysis.* We analyze GWAS summary statistics from the Biobank Japan [32] and UK Biobank [7] for 34 pairs of complex traits and diseases. Briefly, we go through the Biobank Japan phenotypes listed in https://pheweb.jp/downloads and selected all continuous traits and all diseases with cases larger than $5{,}000$. Then we manually matched these traits with those of the UK Biobank phenotypes in Neale's Lab database (http://www.nealelab.is/uk-biobank). In total, we are able to match 18 traits and 16 diseases. We then examine the cross-ancestry genetic correlation using the four methods evaluated in the simulation analysis of Section **??**, including "1MB-Window", "2MB-Window", "Independent", and "Pooled subjects". We find similar patterns to those in the HAPNEST simulations (Supplementary Table 2 and Supplementary Figure 15). First, the "1MB-Window" and "2MB-Window" estimates are highly consistent across all pairs of phenotypes. Second, the results of "Independent" are also largely consistent with those of "1MB-Window" and "2MB-Window". Third, the pooled sample LD scores ("Pooled subjects") overall have smaller estimates than other methods, though the general pattern across phenotypes remains. These real data results suggest that the LDSC framework can be extended to cross-ancestry genetic correlation estimation and the window-based LD blocks work well in real data analysis.

**S2. Consistency theorems.** In this section, we establish the consistency of $\widehat{\sigma}_{\alpha}^2$ and $\widehat{\sigma}_{\alpha\beta}$. As expected, consistency requires weaker conditions compared to normality. Specifically, Conditions **??** and **??** for asymptotic normality of $\widehat{\sigma}_{\alpha}^2$ can be replaced by the following condition.

CONDITION 18. There exists a constant $c_1 \in (0,1)$ such that $n_{r\alpha}^{c_1} \gg \log p$. That is, $\log p = o(n_{r\alpha}^{c_1})$.

THEOREM S1. *Under Conditions* **??**–**??**, **??**, *and* 18, *we have*

$$\widehat{\sigma}_\alpha^2 - \sigma_\alpha^2 \xrightarrow{p} 0$$

*as* $\min(n_\alpha, n_{r\alpha}, p) \to \infty$.

The same result holds if we replace $\alpha$ with $\beta$. It is worth noting that Condition 18 can be implied by Condition **??**. Next, we establish the consistency of $\widehat{\sigma}_{\alpha\beta}$ in Theorem 2 below. We find that Conditions **??**, **??** and **??** for asymptotic normality of $\widehat{\sigma}_{\alpha\beta}$ can be relaxed to the following conditions.

CONDITION 19. We assume that

$$\frac{\|\boldsymbol{w}_{ab}\|^2}{p^2}\left(\frac{1}{n_{r\alpha}} + \frac{1}{n_{r\beta}}\right) = o(1).$$

CONDITION 20. There exist constants $c_1, c_2 \in (0,1)$ such that $n_{r\alpha}^{c_1} \gg \log p$ and $n_{r\beta}^{c_2} \gg \log p$. That is, $\log p = o(n_{r\alpha}^{c_1})$ and $\log p = o(n_{r\beta}^{c_2})$.

THEOREM S2. *Under Conditions* **??**, **??**, **??**–**??**, **??**, 19, *and* 20, *we have*

$$\widehat{\sigma}_{\alpha\beta} - \sigma_{\alpha\beta} \xrightarrow{p} 0,$$

*as* $\min(n_\alpha, n_{r\alpha}, n_\beta, n_{r\beta}, p) \to \infty$.

**S3. Overlapping samples.** For two GWAS cohorts with overlapping samples, we let $\boldsymbol{X}^{(1)}$, $\boldsymbol{X}^{(2)}$, and $\boldsymbol{X}^{(3)}$ denote $n_1 \times p$, $n_2 \times p$, and $n_3 \times p$ matrices, respectively, for $p$ genetic variants, where $\boldsymbol{X}^{(1)}$ and $\boldsymbol{X}^{(2)}$ represent non-overlapping samples in the first and second cohorts, respectively, and $\boldsymbol{X}^{(3)}$ represents overlapping samples in the two cohorts. Similar to Condition **??**, we assume that $\boldsymbol{X}^{(1)} = \boldsymbol{X}_0^{(1)}\boldsymbol{\Sigma}^{1/2}$, $\boldsymbol{X}^{(2)} = \boldsymbol{X}_0^{(2)}\boldsymbol{\Sigma}^{1/2}$, and $\boldsymbol{X}^{(3)} = \boldsymbol{X}_0^{(3)}\boldsymbol{\Sigma}^{1/2}$, where entries of $\boldsymbol{X}_0^{(1)}$, $\boldsymbol{X}_0^{(2)}$, and $\boldsymbol{X}_0^{(3)}$ are i.i.d. random variables with mean zero and variance one, and $\boldsymbol{\Sigma}$ is a $p \times p$ covariance matrix. We also let

$$\boldsymbol{y}^{(\alpha)} = \boldsymbol{X}^{(1)}\boldsymbol{\alpha} + \boldsymbol{\epsilon}^{(\alpha)}, \quad \boldsymbol{y}^{(\alpha o)} = \boldsymbol{X}^{(3)}\boldsymbol{\alpha} + \boldsymbol{\epsilon}^{(\alpha o)},$$

and

$$\boldsymbol{y}^{(\beta)} = \boldsymbol{X}^{(2)}\boldsymbol{\beta} + \boldsymbol{\epsilon}^{(\beta)}, \quad \boldsymbol{y}^{(\beta o)} = \boldsymbol{X}^{(3)}\boldsymbol{\beta} + \boldsymbol{\epsilon}^{(\beta o)},$$

where $\boldsymbol{y}^{(\alpha)}$ and $\boldsymbol{y}^{(\alpha o)}$ are samples of the first complex trait in the first cohort, $\boldsymbol{y}^{(\beta)}$ and $\boldsymbol{y}^{(\beta o)}$ are samples of the second complex trait in the second cohort, and $\boldsymbol{\epsilon}^{(\alpha)}$, $\boldsymbol{\epsilon}^{(\alpha o)}$, $\boldsymbol{\epsilon}^{(\beta)}$, and $\boldsymbol{\epsilon}^{(\beta o)}$ represent independent Gaussian error vectors that are independent of $\boldsymbol{X}^{(1)}$, $\boldsymbol{X}^{(2)}$, and $\boldsymbol{X}^{(3)}$. For $j = 1, \ldots, p$, the GWAS estimators of the marginal genetic effects of the $j$th genetic variant are

$$\widehat{a}_j = \frac{1}{n_1 + n_3}([\boldsymbol{X}_j^{(1)}]^T\boldsymbol{y}^{(\alpha)} + [\boldsymbol{X}_j^{(3)}]^T\boldsymbol{y}^{(\alpha o)}), \quad \widehat{b}_j = \frac{1}{n_2 + n_3}([\boldsymbol{X}_j^{(2)}]^T\boldsymbol{y}^{(\beta)} + [\boldsymbol{X}_j^{(3)}]^T\boldsymbol{y}^{(\beta o)}).$$

Recall that $\sigma_{\alpha\beta} = \sum_{i=1}^p \alpha_i\beta_i/p = g_{\alpha\beta}/p$. Let $\boldsymbol{\Sigma}_j$ denote the $j$th row of $\boldsymbol{\Sigma}$, $\boldsymbol{\Sigma}_{ij}$ denote the $(i,j)$ element of $\boldsymbol{\Sigma}$, $\boldsymbol{X}_{1\cdot}^{(3)}$ represent the first row of $\boldsymbol{X}^{(3)}$, $\boldsymbol{X}_{1j}^{(3)}$ represent the $(1,j)$ element

of $\boldsymbol{X}^{(3)}$, and $\ell_j = \sum_{i=1}^p \boldsymbol{\Sigma}_{ji}^2$ be the LD score of the $j$th genetic variant. Then we have

$$\begin{aligned}
E(\widehat{a}_j\widehat{b}_j) =& \boldsymbol{\alpha}^T\boldsymbol{\Sigma}_j^T\boldsymbol{\Sigma}_j\boldsymbol{\beta} + \frac{n_3}{(n_1+n_3)(n_2+n_3)}\boldsymbol{\alpha}^T\text{Var}(\boldsymbol{X}_{1j}^{(3)}\boldsymbol{X}_{1\cdot}^{(3)})\boldsymbol{\beta} \\
=& \sigma_{\alpha\beta}\ell_j + \sum_{i=1}^p \alpha_i\beta_i\boldsymbol{\Sigma}_{ij}^2 - \sigma_{\alpha\beta}\cdot\sum_{i=1}^p \boldsymbol{\Sigma}_{ij}^2 + \sum_{i\neq k}\alpha_i\beta_k\boldsymbol{\Sigma}_{ij}\boldsymbol{\Sigma}_{kj} \\
&+ \frac{n_3}{(n_1+n_3)(n_2+n_3)}\boldsymbol{\alpha}^T\text{Var}(\boldsymbol{X}_{1j}^{(3)}\boldsymbol{X}_{1\cdot}^{(3)})\boldsymbol{\beta} \\
=& \sigma_{\alpha\beta}\ell_j + \epsilon_j,
\end{aligned}$$

where

$$\begin{aligned}
\epsilon_j =& \sum_{i=1}^p \alpha_i\beta_i\boldsymbol{\Sigma}_{ij}^2 - \sigma_{\alpha\beta}\cdot\sum_{i=1}^p \boldsymbol{\Sigma}_{ij}^2 + \sum_{i\neq k}\alpha_i\beta_k\boldsymbol{\Sigma}_{ij}\boldsymbol{\Sigma}_{kj} \\
&+ \frac{n_3}{(n_1+n_3)(n_2+n_3)}\boldsymbol{\alpha}^T\text{Var}(\boldsymbol{X}_{1j}^{(3)}\boldsymbol{X}_{1\cdot}^{(3)})\boldsymbol{\beta}.
\end{aligned}$$

These results indicate that the presence of overlapping samples between the two GWAS cohorts does not affect the slope in LDSC when there is a certain level of orthogonality between mean-centered vectors $\boldsymbol{H}(\ell_1,\ell_2,\ldots,\ell_p)^T$ and $\boldsymbol{H}(\epsilon_1,\epsilon_2,\ldots,\epsilon_p)^T$. Therefore, LDSC can be used effectively to estimate genetic covariance, irrespective of whether the samples partially or fully overlap.

**S4. Useful lemmas and propositions.** In this section, we present useful lemmas and propositions in our proof. Lemma S1 states that the estimated LD scores in different LD blocks are independent.

LEMMA S1. *Under Condition* **??**, *the* $\widehat{\ell}_{a,j}$*'s corresponding to genetic variants in different* $\mathcal{N}(k)$*'s are independent.*

PROOF. For each $s\in\mathcal{N}(k)$, $t\in\mathcal{N}(m)$, and $m\neq k$, we have

$$\widehat{\ell}_{a,s} = \sum_{i\in\mathcal{N}(k)}\widehat{\boldsymbol{\Sigma}}_{\alpha,si}^2 \quad\text{and}\quad \widehat{\ell}_{a,t} = \sum_{j\in\mathcal{N}(m)}\widehat{\boldsymbol{\Sigma}}_{\alpha,tj}^2.$$

Note that, for each $s,i\in\mathcal{N}(k)$ and $t,j\in\mathcal{N}(m)$, we have

$$\widehat{\boldsymbol{\Sigma}}_{\alpha,si} = \frac{1}{n_\alpha}\boldsymbol{X}_{\alpha,s}^T\boldsymbol{X}_{\alpha,i} \quad\text{and}\quad \widehat{\boldsymbol{\Sigma}}_{\alpha,tj} = \frac{1}{n_\alpha}\boldsymbol{X}_{\alpha,t}^T\boldsymbol{X}_{\alpha,j}.$$

By Condition **??**, $\boldsymbol{X}_{\alpha,s}$ and $\boldsymbol{X}_{\alpha,i}$ are independent of $\boldsymbol{X}_{\alpha,t}$ and $\boldsymbol{X}_{\alpha,j}$, which implies that $\widehat{\ell}_{a,s}$ and $\widehat{\ell}_{a,t}$ are independent. □

Lemmas S2 and S3 quantify the moments of random variables and their products.

LEMMA S2. *Suppose that* $(X_1,Y_1,Z_1,W_1),\ldots,(X_n,Y_n,Z_n,W_n)$ *are i.i.d. samples with mean zero. Then we have*

$$E\left(\frac{\sum_{i=1}^n Z_i}{n}\right)^2 = n^{-1}\cdot EZ_1^2,$$

$$E\left(\frac{\sum_{i=1}^n Z_i}{n}\right)^3 = n^{-2}\cdot EZ_1^3,$$

$$E\left(\frac{\sum_{i=1}^n Z_i}{n}\right)^4 = n^{-3}\cdot EZ_1^4 + \frac{6(n-1)}{n^3}\cdot (EZ_1^2)^2,$$

*and*

$$E\left|\frac{\sum_{i=1}^n Z_i}{n}\right|^3 \le \left\{E\left(\frac{\sum_{i=1}^n Z_i}{n}\right)^4\right\}^{3/4} = \left\{n^{-3}\cdot EZ_1^4 + \frac{6(n-1)}{n^3}\cdot (EZ_1^2)^2\right\}^{3/4}.$$

*In addition, we have*

$$\begin{aligned}
&E\left\{\left(\frac{\sum_{i=1}^n Z_i}{n}\right)^2\left(\frac{\sum_{i=1}^n W_i}{n}\right)^2\right\}\\
&= n^{-4}\cdot\left[n\cdot E(Z_1^2W_1^2) + n(n-1)\cdot EZ_1^2EW_1^2 + 2n(n-1)\cdot\{E(Z_1W_1)\}^2\right]\\
&= n^{-3}\cdot\left[E(Z_1^2W_1^2) + (n-1)\cdot EZ_1^2EW_1^2 + 2(n-1)\cdot\{E(Z_1W_1)\}^2\right],
\end{aligned}$$

$$E\left\{\left(\frac{\sum_{i=1}^n Z_i}{n}\right)^2\left(\frac{\sum_{i=1}^n W_i}{n}\right)\right\} = n^{-2}\cdot E(Z_1^2W_1),$$

$$E\left\{\left(\frac{\sum_{i=1}^n Z_i}{n}\right)\left(\frac{\sum_{i=1}^n W_i}{n}\right)\right\} = n^{-1}\cdot E(Z_1W_1),$$

$$E\left\{\left(\frac{\sum_{i=1}^n X_i}{n}\right)\left(\frac{\sum_{i=1}^n Y_i}{n}\right)\left(\frac{\sum_{i=1}^n Z_i}{n}\right)\right\} = n^{-2}\cdot E(X_1Y_1Z_1),$$

*and*

$$\begin{aligned}
&E\left\{\left(\frac{\sum_{i=1}^n X_i}{n}\right)\left(\frac{\sum_{i=1}^n Y_i}{n}\right)\left(\frac{\sum_{i=1}^n Z_i}{n}\right)\left(\frac{\sum_{i=1}^n W_i}{n}\right)\right\}\\
=&n^{-3}\cdot[E(X_1Y_1Z_1W_1) + (n-1)\cdot\{E(X_1Y_1)E(Z_1W_1)\\
&+ E(X_1Z_1)E(Y_1W_1) + E(X_1W_1)E(Y_1Z_1)\}].
\end{aligned}$$

*If $EX_i^8$, $EY_i^8$, $EZ_i^8$, and $EW_i^8$ are finite, then*

$$E\left\{\left(\frac{\sum_{i=1}^n X_i}{n}\right)^2\left(\frac{\sum_{i=1}^n Y_i}{n}\right)^2\left(\frac{\sum_{i=1}^n Z_i}{n}\right)^2\left(\frac{\sum_{i=1}^n W_i}{n}\right)^2\right\} = O(n^{-4}),$$

$$E\left\{\left(\frac{\sum_{i=1}^n X_i}{n}\right)\left(\frac{\sum_{i=1}^n Y_i}{n}\right)^2\left(\frac{\sum_{i=1}^n Z_i}{n}\right)^2\left(\frac{\sum_{i=1}^n W_i}{n}\right)^2\right\} = O(n^{-4}),$$

$$E\left\{\left(\frac{\sum_{i=1}^n Y_i}{n}\right)^2\left(\frac{\sum_{i=1}^n Z_i}{n}\right)^2\left(\frac{\sum_{i=1}^n W_i}{n}\right)^2\right\} = O(n^{-3}),$$

$$E\left\{\left(\frac{\sum_{i=1}^n Y_i}{n}\right)\left(\frac{\sum_{i=1}^n Z_i}{n}\right)^2\left(\frac{\sum_{i=1}^n W_i}{n}\right)^2\right\} = O(n^{-3}),$$

$$E\left\{\left(\frac{\sum_{i=1}^n Y_i}{n}\right)\left(\frac{\sum_{i=1}^n Z_i}{n}\right)\left(\frac{\sum_{i=1}^n W_i}{n}\right)^2\right\} = O(n^{-2}),$$

$$E\left\{\left(\frac{\sum_{i=1}^n X_i}{n}\right)\left(\frac{\sum_{i=1}^n Y_i}{n}\right)\left(\frac{\sum_{i=1}^n Z_i}{n}\right)^2\left(\frac{\sum_{i=1}^n W_i}{n}\right)^2\right\} = O(n^{-3}),$$

*and*

$$E\left\{\left(\frac{\sum_{i=1}^n X_i}{n}\right)\left(\frac{\sum_{i=1}^n Y_i}{n}\right)\left(\frac{\sum_{i=1}^n Z_i}{n}\right)\left(\frac{\sum_{i=1}^n W_i}{n}\right)^2\right\} = O(n^{-3}).$$

PROOF. The proofs of these equations are straightforward and are ignored. □

LEMMA S3. *Suppose that $(Z_1, W_1), \ldots, (Z_n, W_n)$ are i.i.d. samples with mean $(\mu, \theta)$. Let $X_1 = Z_1 - \mu$ and $Y_1 = W_1 - \theta$. Then we have*

$$\begin{aligned}
&E\left\{\left(\frac{\sum_{i=1}^n Z_i}{n}\right)^2\left(\frac{\sum_{i=1}^n W_i}{n}\right)^2\right\} \\
=&E\left\{\left(\frac{\sum_{i=1}^n (Z_i-\mu)}{n}+\mu\right)^2\left(\frac{\sum_{i=1}^n (W_i-\theta)}{n}+\theta\right)^2\right\} \\
=&n^{-3}\cdot E(X_1^2Y_1^2)+\frac{n-1}{n^3}\cdot EX_1^2EY_1^2+\frac{n-1}{n^3}\cdot\{E(X_1Y_1)\}^2 \\
&+2n^{-2}\cdot\theta E(X_1^2Y_1)+2n^{-2}\cdot\mu E(X_1Y_1^2) \\
&+n^{-1}\cdot\theta^2EX_1^2+4n^{-1}\cdot\mu\theta E(X_1Y_1)+n^{-1}\cdot\mu^2EY_1^2+\mu^2\theta^2 \qquad (12)
\end{aligned}$$

*and*

$$\begin{aligned}
&E\left\{\left(\frac{\sum_{i=1}^n Z_i}{n}\right)\left(\frac{\sum_{i=1}^n W_i}{n}\right)\right\} \\
=&E\left\{\left(\frac{\sum_{i=1}^n (Z_i-\mu)}{n}+\mu\right)\left(\frac{\sum_{i=1}^n (W_i-\theta)}{n}+\theta\right)\right\} \\
=&n^{-1}\cdot E(X_1Y_1)+\mu\theta. \qquad (13)
\end{aligned}$$

PROOF. The last equations in (12) and (13) follow from Lemma S2. □

Lemma S4 provides upper and lower bounds for the trace of the product of matrices.

LEMMA S4. *Let $A$ and $B$ be two symmetric $n \times n$ matrices. Suppose that $A$ is positive definite and that $B$ is semi-positive definite. Then $tr(ABA) \geq \lambda_{\min}^2(A)tr(B)$ and $tr(ABA) \leq \lambda_{\max}^2(A)tr(B)$.*

PROOF. Let $\lambda_k(B)$ denote the $k$th smallest eigenvalue of $B$. By the Courant–Fischer–Weyl min-max principle, we have

$$\lambda_k(B) = \min_U \max_{x\in U}\{x^TBx/\|x\|^2 \mid dim(U)=k\} = \min_U \max_{x\in U, \|x\|=1}\{x^TBx \mid dim(U)=k\}.$$

It suffices to show that $\lambda_{\min}^2(A)\lambda_k(B) \le \lambda_k(ABA)$. For any $U$ with $dim(U) = k$, let $U' = AU$. Then $dim(U') = k$, and there exist $x_0 \in U$ and $y_0 = Ax_0 \in U'$ such that $\|x_0\| = 1$ and $y_0^T B y_0/\|y_0\|^2 = \max_{y\in U'} y^T By/\|y\|^2$. Thus, we have

$$\max_{x\in U,\|x\|=1} x^T ABAx \ge \frac{x_0^T ABAx_0}{\|y_0\|^2}\cdot\|y_0\|^2 = \max_{y\in U'}\frac{y^T By}{\|y\|^2}\cdot\|y_0\|^2 \ge \lambda_k(B)\lambda_{\min}^2(A),$$

implying that $\lambda_k(ABA) \ge \lambda_k(B)\lambda_{\min}^2(A)$. Let $C = ABA$, then we have $B = A^{-1}CA^{-1}$. It follows that

$$\mathrm{tr}(B) = \mathrm{tr}(A^{-1}CA^{-1}) \ge \lambda_{\min}(A^{-1})\mathrm{tr}(C) = \mathrm{tr}(A^{-1}CA^{-1}) \ge \lambda_{\min}^2(A^{-1})\mathrm{tr}(ABA).$$

□

Lemma S5 indicates the sixth moment of eigenvalues of sample covariance matrices are bounded.

LEMMA S5. *Under Conditions* **??** *and* **??**, *we have*

$$E\left[\{\lambda_{\max}(\boldsymbol{X}_\alpha^T\boldsymbol{X}_\alpha/n_\alpha)\}^6\right] = O(1) \quad \text{and} \quad E\left[\{\lambda_{\max}(\boldsymbol{X}_\beta^T\boldsymbol{X}_\beta/n_\beta)\}^6\right] = O(1)$$

*for sufficiently large* $p$.

PROOF. For sufficiently large $p$ and $K$, there exists positive constants $c_1$ and $c_2$ such that

$$\begin{aligned}
&E\left[\|\boldsymbol{X}_\alpha^T\boldsymbol{X}_\alpha/n_\alpha - \boldsymbol{\Sigma}_\alpha\|^6\right]\\
=&\int_{\|\boldsymbol{X}_\alpha^T\boldsymbol{X}_\alpha/n_\alpha-\boldsymbol{\Sigma}_\alpha\|\le\max\{c_1K\sqrt{p}/\sqrt{n_\alpha},c_1^2K^2p/n_\alpha\}}\|\boldsymbol{X}_\alpha^T\boldsymbol{X}_\alpha/n_\alpha - \boldsymbol{\Sigma}_\alpha\|^6 d\boldsymbol{X}_\alpha +\\
&\sum_{k=K}^{+\infty}\int_{\mathcal{A}(k)}\|\boldsymbol{X}_\alpha^T\boldsymbol{X}_\alpha/n_\alpha - \boldsymbol{\Sigma}_\alpha\|^6 d\boldsymbol{X}_\alpha\\
\le&\max\left\{\frac{c_1^6K^6p^3}{n_\alpha^3},\frac{c_1^{12}K^{12}p^6}{n_\alpha^6}\right\} + \sum_{k=K}^{+\infty}\max\left\{\frac{c_1^6(k+1)^6p^3}{n_\alpha^3},\frac{c_1^{12}(k+1)^{12}p^6}{n_\alpha^6}\right\}\\
&\cdot P(\|\boldsymbol{X}_\alpha^T\boldsymbol{X}_\alpha/n_\alpha - \boldsymbol{\Sigma}_\alpha\| > \max\{c_1k\sqrt{p}/\sqrt{n_\alpha}, c_1^2k^2p/n_\alpha\})\\
\le&\max\left\{\frac{c_1^6K^6p^3}{n_\alpha^3},\frac{c_1^{12}K^{12}p^6}{n_\alpha^6}\right\} + \sum_{k=K}^{+\infty}\max\left\{\frac{c_1^6(k+1)^6p^3}{n_\alpha^3},\frac{c_1^{12}(k+1)^{12}p^6}{n_\alpha^6}\right\}\\
&\cdot 2\exp(-c_2(k-1)^2p)\\
\lesssim&\max\left\{\frac{c_1^6K^6p^3}{n_\alpha^3},\frac{c_1^{12}K^{12}p^6}{n_\alpha^6}\right\} + \sum_{k=K}^{+\infty}\max\left\{\frac{c_1^6(k+1)^6p^3}{n_\alpha^3},\frac{c_1^{12}(k+1)^{12}p^6}{n_\alpha^6}\right\}\cdot\frac{1}{(k-1)^{14}},
\end{aligned}$$

where $\mathcal{A}(k) = \{\boldsymbol{X}_\alpha : \max\{c_1k\sqrt{p}/\sqrt{n_\alpha}, c_1^2k^2p/n_\alpha\} < \|\boldsymbol{X}_\alpha^T\boldsymbol{X}_\alpha/n_\alpha - \boldsymbol{\Sigma}_\alpha\| \le \max\{c_1(k+1)\sqrt{p}/\sqrt{n_\alpha}, c_1^2(k+1)^2p/n_\alpha\}\}$.

The second inequality above follows from [44, (5.25)]. By Condition **??**, we have $p = O(n_\alpha)$, then

$$E\left[\|\boldsymbol{X}_\alpha^T\boldsymbol{X}_\alpha/n_\alpha - \boldsymbol{\Sigma}_\alpha\|^6\right] = O(1).$$

By Condition **??**, we have $\|\boldsymbol{\Sigma}_\alpha\|^6 = O(1)$. It follows that

$$\begin{aligned}
E\left[\{\lambda_{\max}(\boldsymbol{X}_\alpha^T\boldsymbol{X}_\alpha/n_\alpha)\}^6\right] &= E\left[\|\boldsymbol{X}_\alpha^T\boldsymbol{X}_\alpha/n_\alpha\|^6\right]\\
&\le E\left[\|\boldsymbol{X}_\alpha^T\boldsymbol{X}_\alpha/n_\alpha - \boldsymbol{\Sigma}_\alpha\|^6\right] + \|\boldsymbol{\Sigma}_\alpha\|^6 = O(1).
\end{aligned}$$

□

Lemmas S6-S10 quantify the behavior of various functions used in our proof, many of which are related to the estimated LD scores.

LEMMA S6. *Under Condition ??, there exists positive constants $c_1$ and $c_2$ such that for every $t \in (0, 1/2)$, we have*

$$P\left(|\widehat{\mathbf{\Sigma}}_{\alpha,ji} - \mathbf{\Sigma}_{\alpha,ji}| \le \frac{1}{n_{r\alpha}^{1/2-t}}\right) \ge 1 - \exp\{-c_1 n_{r\alpha}^{2t}\},$$

$$P\left(|\widehat{\mathbf{\Sigma}}_{\beta,ji} - \mathbf{\Sigma}_{\beta,ji}| \le \frac{1}{n_{r\beta}^{1/2-t}}\right) \ge 1 - \exp\{-c_1 n_{r\beta}^{2t}\},$$

$$P\left(|\widehat{\ell}_{ab,i}(n_{r\alpha}, n_{r\beta}) - \ell_{ab,i}| \le \frac{c_2}{n_{r\alpha}^{1/2-t}} + \frac{c_2}{n_{r\beta}^{1/2-t}}\right) \ge 1 - \exp\{-c_1 n_{r\alpha}^{2t}\} - \exp\{-c_1 n_{r\beta}^{2t}\},$$

$$P\left(|\widehat{\ell}_{a,i}(n_{r\alpha}) - \ell_{a,i}| \le \frac{c_2}{n_{r\alpha}^{1/2-t}}\right) \ge 1 - \exp\{-c_1 n_{r\alpha}^{2t}\},$$

*and*

$$P\left(|\widehat{\ell}_{b,i}(n_{r\beta}) - \ell_{b,i}| \le \frac{c_2}{n_{r\beta}^{1/2-t}}\right) \ge 1 - \exp\{-c_1 n_{r\beta}^{2t}\},$$

*for $i, j = 1, \ldots, p$.*

PROOF. Under Condition ??, $\widehat{\mathbf{\Sigma}}_\alpha - \mathbf{\Sigma}_\alpha$ is a block-diagonal matrix where sizes of blocks are bounded by constants. Then the spectral norm of $\widehat{\mathbf{\Sigma}}_\alpha - \mathbf{\Sigma}_\alpha$ is the maximum of spectral norms of all blocks. By [44, (5.25)], there exists a positive constant $c$ such that for every $t \in (0, 1/2)$, we have

$$P\left(\|\widehat{\mathbf{\Sigma}}_\alpha - \mathbf{\Sigma}_\alpha\| \le \frac{1}{n_{r\alpha}^{1/2-t}}\right) \ge 1 - \exp\{-c n_{r\alpha}^{2t}\}.$$

Note that, for $i, j = 1, \ldots, p$, we have

$$|\widehat{\mathbf{\Sigma}}_{\alpha,ji} - \mathbf{\Sigma}_{\alpha,ji}| \le \|\widehat{\mathbf{\Sigma}}_\alpha - \mathbf{\Sigma}_\alpha\|,$$

$$\begin{aligned}|\widehat{\ell}_{ab,i}(n_{r\alpha}, n_{r\beta}) - \ell_{ab,i}| &\le \sum_{j\in\mathcal{N}(m)} |\widehat{\mathbf{\Sigma}}_{\alpha,ji}\widehat{\mathbf{\Sigma}}_{\beta,ji} - \mathbf{\Sigma}_{\alpha,ji}\mathbf{\Sigma}_{\beta,ji}| \\ &\le \sum_{j\in\mathcal{N}(m)} |\widehat{\mathbf{\Sigma}}_{\alpha,ji}| \cdot |\widehat{\mathbf{\Sigma}}_{\beta,ji} - \mathbf{\Sigma}_{\beta,ji}| + \sum_{j\in\mathcal{N}(m)} |\widehat{\mathbf{\Sigma}}_{\alpha,ji} - \mathbf{\Sigma}_{\alpha,ji}| \cdot |\mathbf{\Sigma}_{\beta,ji}|,\end{aligned}$$

and

$$\begin{aligned}|\widehat{\ell}_{a,i} - \ell_{a,i}| &\le \sum_{j\in\mathcal{N}(m)} |\widehat{\mathbf{\Sigma}}^2_{\alpha,ji} - \mathbf{\Sigma}^2_{\alpha,ji}| \\ &\le \sum_{j\in\mathcal{N}(m)} (\widehat{\mathbf{\Sigma}}_{\alpha,ji} - \mathbf{\Sigma}_{\alpha,ji})^2 + 2|\mathbf{\Sigma}_{\alpha,ji}||\widehat{\mathbf{\Sigma}}_{\alpha,ji} - \mathbf{\Sigma}_{\alpha,ji}|.\end{aligned}$$

This completes the proof. □

LEMMA S7. *Under Conditions **??** and 20, for sufficiently large $n_{r\alpha}$ and $n_{r\beta}$, we have*

$$\max_{1\le i\le p} |\widehat{\ell}_{ab,i}(n_{r\alpha}, n_{r\beta}) - \ell_{ab,i}| \xrightarrow{p} 0,$$

$$\max_{1\le i\le p} |\widehat{\ell}_{a,i}(n_{r\alpha}) - \ell_{a,i}| \xrightarrow{p} 0,$$

*and*

$$\max_{1\le i\le p} |\widehat{\ell}_{b,i}(n_{r\beta}) - \ell_{b,i}| \xrightarrow{p} 0,$$

*as $n_{r\alpha}$ and $n_{r\beta} \to \infty$.*

PROOF. For any positive constant $c$ and sufficiently large $n_{r\alpha}$ and $n_{r\beta}$, there exists a positive constant $c_1$ such that for every $t \in (0, 1/2)$, we have

$$\begin{aligned}
&P(\max_{1\le i\le p} |\widehat{\ell}_{ab,i}(n_{r\alpha}, n_{r\beta}) - \ell_{ab,i}| < c) \\
=&P(|\widehat{\ell}_{ab,1}(n_{r\alpha}, n_{r\beta}) - \ell_{ab,1}| < c, \dots, |\widehat{\ell}_{ab,p}(n_{r\alpha}, n_{r\beta}) - \ell_{ab,p}| < c) \\
\ge& \prod_{m=1}^{p_b} \left\{ 1 - \sum_{i\in\mathcal{N}(m)} P(|\widehat{\ell}_{ab,i}(n_{r\alpha}, n_{r\beta}) - \ell_{ab,i}| \ge c) \right\} \\
\gtrsim& \left(1 - \exp\{-c_1 n_{r\alpha}^{2t}\} - \exp\{-c_1 n_{r\beta}^{2t}\}\right)^{p_b}.
\end{aligned}$$

The last inequality above follows from Lemma S6. Similarly, we have

$$P(\max_{1\le i\le p} |\widehat{\ell}_{a,i}(n_{r\alpha}) - \ell_{a,i}| < c) \gtrsim \left(1 - \exp\{-c_1 n_{r\alpha}^{2t}\}\right)^{p_b}.$$

By Taylor expansion, we have

$$\begin{aligned}
&\log\left[\left(1 - \exp\{-c_1 n_{r\alpha}^{2t}\} - \exp\{-c_1 n_{r\beta}^{2t}\}\right)^{p_b}\right] \\
=&p_b \log\left(1 - \exp\{-c_1 n_{r\alpha}^{2t}\} - \exp\{-c_1 n_{r\beta}^{2t}\}\right) \\
=&p_b \left[-\exp\{-c_1 n_{r\alpha}^{2t}\} - \exp\{-c_1 n_{r\beta}^{2t}\} + o(\exp\{-c_1 n_{r\alpha}^{2t}\}) + o(\exp\{-c_1 n_{r\beta}^{2t}\})\right].
\end{aligned}$$

Since $n_{r\alpha}^{s_1} \gg \log p$ and $n_{r\beta}^{s_1} \gg \log p$ for certain $s_1, s_2 \in (0,1)$ by Condition 20,

$$\max_{1\le i\le p} |\widehat{\ell}_{ab,i}(n_{r\alpha}, n_{r\beta}) - \ell_{ab,i}| \xrightarrow{p} 0,$$

as $n_{r\alpha}, n_{r\beta} \to \infty$. Similarly, we can show that

$$\max_{1\le i\le p} |\widehat{\ell}_{a,i}(n_{r\alpha}) - \ell_{a,i}| \xrightarrow{p} 0,$$

and

$$\max_{1\le i\le p} |\widehat{\ell}_{b,i}(n_{r\beta}) - \ell_{b,i}| \xrightarrow{p} 0.$$

□

LEMMA S8. *Under Condition **??**, for any $\epsilon > 0$ and $i = 1, \dots, p$, we have*

$$P(|\widehat{\ell}_{ab,i}(n_{r\alpha}, n_{r\beta}) - \ell_{ab,i}| \ge \epsilon) = O(n_{r\alpha}^{-2} + n_{r\beta}^{-2}).$$

PROOF. For any $\epsilon > 0$, by the extended version of Markov's inequality, we have

$$P(|\widehat{\ell}_{ab,i}(n_{r\alpha}, n_{r\beta}) - \ell_{ab,i}| \geq \epsilon) \leq \frac{E[\widehat{\ell}_{ab,i}(n_{r\alpha}, n_{r\beta}) - \ell_{ab,i}]^4}{\epsilon^4}.$$

For any $m = 1, \ldots, p_b$ and $j \in \mathcal{N}(m)$, we have

$$\begin{aligned} E\{\widehat{\ell}_{ab,j}(n_{r\alpha}, n_{r\beta}) - \ell_{ab,j}\}^4 =& E\left\{\sum_{i \in \mathcal{N}(m)} (\widehat{\mathbf{\Sigma}}_{\alpha,ji}\widehat{\mathbf{\Sigma}}_{\beta,ji} - \mathbf{\Sigma}_{\alpha,ji}\mathbf{\Sigma}_{\beta,ji})\right\}^4 \\ &\lesssim \sum_{i \in \mathcal{N}(m)} E(\widehat{\mathbf{\Sigma}}_{\alpha,ji}\widehat{\mathbf{\Sigma}}_{\beta,ji} - \mathbf{\Sigma}_{\alpha,ji}\mathbf{\Sigma}_{\beta,ji})^4. \end{aligned}$$

Note that

$$\begin{aligned} & E(\widehat{\mathbf{\Sigma}}_{\alpha,ji}\widehat{\mathbf{\Sigma}}_{\beta,ji} - \mathbf{\Sigma}_{\alpha,ji}\mathbf{\Sigma}_{\beta,ji})^4 \\ =& E\{(\widehat{\mathbf{\Sigma}}_{\alpha,ji} - \mathbf{\Sigma}_{\alpha,ji} + \mathbf{\Sigma}_{\alpha,ji})(\widehat{\mathbf{\Sigma}}_{\beta,ji} - \mathbf{\Sigma}_{\beta,ji} + \mathbf{\Sigma}_{\beta,ji}) - \mathbf{\Sigma}_{\alpha,ji}\mathbf{\Sigma}_{\beta,ji}\}^4 \\ =& E\{(\widehat{\mathbf{\Sigma}}_{\alpha,ji} - \mathbf{\Sigma}_{\alpha,ji})(\widehat{\mathbf{\Sigma}}_{\beta,ji} - \mathbf{\Sigma}_{\beta,ji}) + \mathbf{\Sigma}_{\alpha,ji}(\widehat{\mathbf{\Sigma}}_{\beta,ji} - \mathbf{\Sigma}_{\beta,ji}) \\ & + \mathbf{\Sigma}_{\beta,ji}(\widehat{\mathbf{\Sigma}}_{\alpha,ji} - \mathbf{\Sigma}_{\alpha,ji})\}^4 \\ \lesssim& E\{(\widehat{\mathbf{\Sigma}}_{\alpha,ji} - \mathbf{\Sigma}_{\alpha,ji})^4(\widehat{\mathbf{\Sigma}}_{\beta,ji} - \mathbf{\Sigma}_{\beta,ji})^4\} + \mathbf{\Sigma}_{\alpha,ji}^4 E(\widehat{\mathbf{\Sigma}}_{\beta,ji} - \mathbf{\Sigma}_{\beta,ji})^4 \\ & + \mathbf{\Sigma}_{\beta,ji}^4 E(\widehat{\mathbf{\Sigma}}_{\alpha,ji} - \mathbf{\Sigma}_{\alpha,ji})^4 \\ =& E(\widehat{\mathbf{\Sigma}}_{\alpha,ji} - \mathbf{\Sigma}_{\alpha,ji})^4 E(\widehat{\mathbf{\Sigma}}_{\beta,ji} - \mathbf{\Sigma}_{\beta,ji})^4 + \mathbf{\Sigma}_{\alpha,ji}^4 E(\widehat{\mathbf{\Sigma}}_{\beta,ji} - \mathbf{\Sigma}_{\beta,ji})^4 \\ & + \mathbf{\Sigma}_{\beta,ji}^4 E(\widehat{\mathbf{\Sigma}}_{\alpha,ji} - \mathbf{\Sigma}_{\alpha,ji})^4. \end{aligned}$$

The last equation above follows from the independence of the two reference panels $\boldsymbol{Z}_\alpha$ and $\boldsymbol{Z}_\beta$. By Condition **??** and Lemma S2, we have

$$E(\widehat{\mathbf{\Sigma}}_{\alpha,ji}\widehat{\mathbf{\Sigma}}_{\beta,ji} - \mathbf{\Sigma}_{\alpha,ji}\mathbf{\Sigma}_{\beta,ji})^4 \lesssim n_{r\alpha}^{-2} + n_{r\beta}^{-2}$$

and

$$E\{\widehat{\ell}_{ab,j}(n_{r\alpha}, n_{r\beta}) - \ell_{ab,j}\}^4 \lesssim n_{r\alpha}^{-2} + n_{r\beta}^{-2}.$$

Therefore, for any $\epsilon > 0$ and $i = 1, \ldots, p$, we have

$$P(|\widehat{\ell}_{ab,i}(n_{r\alpha}, n_{r\beta}) - \ell_{ab,i}| \geq \epsilon) = O(n_{r\alpha}^{-2} + n_{r\beta}^{-2}).$$

□

LEMMA S9. *Under Condition **??**, for bounded constants $c_{ij}$, $1 \leq i, j \leq p$, we have*

$$h_1(p, n_{r\alpha}, n_{r\beta}) \cdot \sum_{m=1}^{p_b} \sum_{i,j \in \mathcal{N}(m)} c_{ij}(\widehat{\boldsymbol{\ell}}_{ab,i}\widehat{\boldsymbol{\ell}}_{ab,j} - \boldsymbol{\ell}_{ab,i}\boldsymbol{\ell}_{ab,j}) \xrightarrow{p} 0,$$

*as $n_{r\alpha}$ and $n_{r\beta} \to \infty$, where $h_1(p, n_{r\alpha}, n_{r\beta}) > 0$,*

$$h_1^2(p, n_{r\alpha}, n_{r\beta}) \cdot p_b(n_{r\alpha}^{-1} + n_{r\beta}^{-1}) = o(1),$$

*and*

$$h_1(p, n_{r\alpha}, n_{r\beta}) \cdot p_b(n_{r\alpha}^{-1} + n_{r\beta}^{-1}) = o(1).$$

PROOF. Note that

$$\sum_{m=1}^{p_b}\sum_{i,j\in\mathcal{N}(m)} c_{ij}(\widehat{\boldsymbol{\ell}}_{ab,i}\widehat{\boldsymbol{\ell}}_{ab,j}-\boldsymbol{\ell}_{ab,i}\boldsymbol{\ell}_{ab,j})$$

$$=\sum_{m=1}^{p_b}\sum_{i,j\in\mathcal{N}(m)} c_{ij}\{\widehat{\boldsymbol{\ell}}_{ab,i}\widehat{\boldsymbol{\ell}}_{ab,j}-E(\widehat{\boldsymbol{\ell}}_{ab,i}\widehat{\boldsymbol{\ell}}_{ab,j})+E(\widehat{\boldsymbol{\ell}}_{ab,i}\widehat{\boldsymbol{\ell}}_{ab,j})-\boldsymbol{\ell}_{ab,i}\boldsymbol{\ell}_{ab,j}\}$$

Let

$$G(p)=h_1(p,n_{r\alpha},n_{r\beta})\cdot\sum_{m=1}^{p_b}\sum_{i,j\in\mathcal{N}(m)} c_{ij}\{\widehat{\boldsymbol{\ell}}_{ab,i}\widehat{\boldsymbol{\ell}}_{ab,j}-E(\widehat{\boldsymbol{\ell}}_{ab,i}\widehat{\boldsymbol{\ell}}_{ab,j})\}$$

and

$$H(p)=\sum_{m=1}^{p_b}\sum_{i,j\in\mathcal{N}(m)} c_{ij}\{E(\widehat{\boldsymbol{\ell}}_{ab,i}\widehat{\boldsymbol{\ell}}_{ab,j})-\boldsymbol{\ell}_{ab,i}\boldsymbol{\ell}_{ab,j}\}$$

$$=\sum_{m=1}^{p_b}\sum_{i,j\in\mathcal{N}(m)} c_{ij}\mathrm{Cov}(\widehat{\boldsymbol{\ell}}_{ab,i},\widehat{\boldsymbol{\ell}}_{ab,j}).$$

Under Condition **??**, by (44), for any $i,j=1,\dots,p$, we have

$$\mathrm{Cov}(\widehat{\boldsymbol{\ell}}_{ab,i},\widehat{\boldsymbol{\ell}}_{ab,j})=O(n_{r\alpha}^{-1}+n_{r\beta}^{-1}).$$

Under Condition **??**, since

$$h_1(p,n_{r\alpha},n_{r\beta})\cdot p_b(n_{r\alpha}^{-1}+n_{r\beta}^{-1})=o(1),$$

we have

$$h_1(p,n_{r\alpha},n_{r\beta})\cdot|H(p)|\lesssim h_1(p,n_{r\alpha},n_{r\beta})\cdot p_b(n_{r\alpha}^{-1}+n_{r\beta}^{-1})\to 0.$$

By Chebyshev's inequality, we have

$$P(|G(p)|>\epsilon)\le\frac{\mathrm{Var}\{G(p)\}}{\epsilon^2}.$$

Note that

$$\mathrm{Var}\{G(p)\}=h_1^2(p,n_{r\alpha},n_{r\beta})\cdot\sum_{m=1}^{p_b}\mathrm{Var}[\sum_{i,j\in\mathcal{N}(m)} c_{ij}\{\widehat{\boldsymbol{\ell}}_{ab,i}\widehat{\boldsymbol{\ell}}_{ab,j}-E(\widehat{\boldsymbol{\ell}}_{ab,i}\widehat{\boldsymbol{\ell}}_{ab,j})\}],$$

$$\mathrm{Cov}(\widehat{\boldsymbol{\ell}}_{ab,i}\widehat{\boldsymbol{\ell}}_{ab,j},\widehat{\boldsymbol{\ell}}_{ab,k}\widehat{\boldsymbol{\ell}}_{ab,l})\le\sqrt{\mathrm{Var}(\widehat{\boldsymbol{\ell}}_{ab,i}\widehat{\boldsymbol{\ell}}_{ab,j})\mathrm{Var}(\widehat{\boldsymbol{\ell}}_{ab,k}\widehat{\boldsymbol{\ell}}_{ab,l})}$$

for $i,j\in\mathcal{N}(m)$,

$$\mathrm{Var}(\widehat{\boldsymbol{\ell}}_{ab,i}\widehat{\boldsymbol{\ell}}_{ab,j})=\mathrm{Var}(\sum_{u\in\mathcal{N}(m)}\widehat{\boldsymbol{\Sigma}}_{\alpha,iu}\widehat{\boldsymbol{\Sigma}}_{\beta,iu}\sum_{u\in\mathcal{N}(m)}\widehat{\boldsymbol{\Sigma}}_{\alpha,ju}\widehat{\boldsymbol{\Sigma}}_{\beta,ju}),$$

and for $u,v\in\mathcal{N}(m)$, we have

$$\begin{aligned}&\mathrm{Var}(\widehat{\boldsymbol{\Sigma}}_{\alpha,iu}\widehat{\boldsymbol{\Sigma}}_{\beta,iu}\widehat{\boldsymbol{\Sigma}}_{\alpha,jv}\widehat{\boldsymbol{\Sigma}}_{\beta,jv})\\&=E(\widehat{\boldsymbol{\Sigma}}_{\alpha,iu}\widehat{\boldsymbol{\Sigma}}_{\beta,iu}\widehat{\boldsymbol{\Sigma}}_{\alpha,jv}\widehat{\boldsymbol{\Sigma}}_{\beta,jv})^2-\{E(\widehat{\boldsymbol{\Sigma}}_{\alpha,iu}\widehat{\boldsymbol{\Sigma}}_{\beta,iu}\widehat{\boldsymbol{\Sigma}}_{\alpha,jv}\widehat{\boldsymbol{\Sigma}}_{\beta,jv})\}^2\\&=E(\widehat{\boldsymbol{\Sigma}}_{\alpha,iu}\widehat{\boldsymbol{\Sigma}}_{\alpha,jv})^2E(\widehat{\boldsymbol{\Sigma}}_{\beta,iu}\widehat{\boldsymbol{\Sigma}}_{\beta,jv})^2-\{E(\widehat{\boldsymbol{\Sigma}}_{\alpha,iu}\widehat{\boldsymbol{\Sigma}}_{\alpha,jv})\}^2\{E(\widehat{\boldsymbol{\Sigma}}_{\beta,iu}\widehat{\boldsymbol{\Sigma}}_{\beta,jv})\}^2.\end{aligned}$$

By Lemma S3, since $EX_{\alpha,j}^8$ and $EX_{\beta,j}^8$ are bounded under Condition **??** for $j=1,\dots,p$, then we have

$$\text{Var}(\widehat{\boldsymbol{\Sigma}}_{\alpha,iu}\widehat{\boldsymbol{\Sigma}}_{\beta,iu}\widehat{\boldsymbol{\Sigma}}_{\alpha,jv}\widehat{\boldsymbol{\Sigma}}_{\beta,jv}) = O(n_{r\alpha}^{-1}+n_{r\beta}^{-1}),$$

which implies $\text{Var}\{G(p)\}\to 0$. □

LEMMA S10. *Under Conditions **??** and 20, for bounded constants $c_{ij}$ $(1\le i,j\le p)$, we have*

$$p^{-1}\cdot\sum_{m=1}^{p_b}\sum_{i,j\in\mathcal{N}(m)} c_{ij}(\widehat{\boldsymbol{\ell}}_{a,i}^2\widehat{\boldsymbol{\ell}}_{a,j}^2-\boldsymbol{\ell}_{a,i}^2\boldsymbol{\ell}_{a,j}^2)\xrightarrow{p}0,$$

*as $n_{r\alpha}\to\infty$.*

PROOF. By Condition **??**, $\max_{1\le i\le p}|\boldsymbol{\ell}_{a,i}|=O(1)$. Note that

$$\begin{aligned}
&p^{-1}\cdot\sum_{m=1}^{p_b}\sum_{i,j\in\mathcal{N}(m)} c_{ij}(\widehat{\boldsymbol{\ell}}_{a,i}^2\widehat{\boldsymbol{\ell}}_{a,j}^2-\boldsymbol{\ell}_{a,i}^2\boldsymbol{\ell}_{a,j}^2)\\
=&p^{-1}\cdot\sum_{m=1}^{p_b}\sum_{i,j\in\mathcal{N}(m)} c_{ij}[(\widehat{\boldsymbol{\ell}}_{a,i}-\boldsymbol{\ell}_{a,i})(\widehat{\boldsymbol{\ell}}_{a,i}+\boldsymbol{\ell}_{a,i})\widehat{\boldsymbol{\ell}}_{a,j}^2-\boldsymbol{\ell}_{a,i}^2(\boldsymbol{\ell}_{a,j}-\widehat{\boldsymbol{\ell}}_{a,j})(\boldsymbol{\ell}_{a,j}+\widehat{\boldsymbol{\ell}}_{a,j})].
\end{aligned}$$

By the proof of Lemma S7, for any positive constant $c$ and sufficiently large $n_{r\alpha}$, we have

$$P(|\widehat{\ell}_{a,1}-\ell_{a,1}|<c,\dots,|\widehat{\ell}_{a,p}-\ell_{a,p}|<c)\to 0,$$

as $n_{r\alpha}\to\infty$, which completes the proof. □

Lemma S11 provides bounds for different functions of $\boldsymbol{w}_a$.

LEMMA S11. *Under Condition **??**, we have*

$$\sum_{i=1}^p \boldsymbol{w}_{a,i}\lesssim\|\boldsymbol{\alpha}\|_2^2+\frac{p}{n_\alpha}\|\boldsymbol{\alpha}\|_2^2,$$

$$\left(\|\boldsymbol{\alpha}\|_4^4+\frac{p}{n_\alpha^2}\|\boldsymbol{\alpha}\|_2^4\right)^{1/2}\lesssim\|\boldsymbol{w}_a\|_2\lesssim\left(\|\boldsymbol{\alpha}\|_4^4+\frac{p}{n_\alpha^2}\|\boldsymbol{\alpha}\|_2^4\right)^{1/2},$$

*and*

$$\|\boldsymbol{w}_a\|_3\lesssim\left(\|\boldsymbol{\alpha}\|_6^6+\frac{p}{n_\alpha^3}\|\boldsymbol{\alpha}\|_2^6\right)^{1/3}.$$

PROOF. Recall that $\boldsymbol{w}_a=(a_1^2,\dots,a_p^2)^T+\{\text{Var}(\widehat{a}_1),\dots,\text{Var}(\widehat{a}_p)\}^T$. Note that

$$\sum_{i=1}^p\boldsymbol{w}_{a,i}\lesssim\sum_{i=1}^p a_i^2+\sum_{i=1}^p\text{Var}(\widehat{a}_i),$$

$$\sum_{i=1}^p a_i^4+\sum_{i=1}^p\text{Var}(\widehat{a}_i)^2\lesssim\|\boldsymbol{w}_a\|_2^2\lesssim\sum_{i=1}^p a_i^4+\sum_{i=1}^p\text{Var}(\widehat{a}_i)^2,$$

and

$$\|\boldsymbol{w}_a\|_3^3 \lesssim \sum_{i=1}^p a_i^6 + \sum_{i=1}^p \text{Var}(\widehat{a}_i)^3.$$

By Condition **??**, we have

$$\begin{aligned}\text{Var}(\widehat{a}_i) =& n_\alpha^{-1} \cdot \text{Var}(X_{\alpha,1i} y_{\alpha,1})\\ =& n_\alpha^{-1} \cdot \text{Var}\left(X_{\alpha,1i}\boldsymbol{X}_{\alpha,1\cdot}\boldsymbol{\alpha}\right) + n_\alpha^{-1} \cdot \text{Var}\left(X_{\alpha,1i}\epsilon_{\alpha,1}\right)\\ \leq& n_\alpha^{-1} \cdot \left[\lambda_{\max}\left\{\text{Var}\left(X_{\alpha,1i}\boldsymbol{X}_{\alpha,1\cdot}\right)\right\}\|\boldsymbol{\alpha}\|^2 + \sigma_{\epsilon_\alpha}^2\right]\end{aligned}$$

and

$$\text{Var}(\widehat{a}_i) \geq n_\alpha^{-1} \cdot \left[\lambda_{\min}\left\{\text{Var}\left(X_{\alpha,1i}\boldsymbol{X}_{\alpha,1\cdot}\right)\right\}\|\boldsymbol{\alpha}\|^2 + \sigma_{\epsilon_\alpha}^2\right].$$

By the proof of Lemma **??**, $\lambda_{\max}\left\{\text{Var}\left(X_{\alpha,1i}\boldsymbol{X}_{\alpha,1\cdot}\right)\right\} = O(1)$ and $\lambda_{\min}\left\{\text{Var}\left(X_{\alpha,1i}\boldsymbol{X}_{\alpha,1\cdot}\right)\right\} > c$ for some positive constant $c$. By Condition **?? ??**, we have $\sigma_{\epsilon_\alpha}^2 \asymp \|\boldsymbol{\alpha}\|^2$. It follows that

$$\sum_{i=1}^p \text{Var}(\widehat{a}_i) \lesssim \frac{p}{n_\alpha}\|\boldsymbol{\alpha}\|^2,$$

$$\frac{p}{n_\alpha^2}\|\boldsymbol{\alpha}\|^4 \lesssim \sum_{i=1}^p \text{Var}(\widehat{a}_i)^2 \lesssim \frac{p}{n_\alpha^2}\|\boldsymbol{\alpha}\|^4,$$

and

$$\sum_{i=1}^p \text{Var}(\widehat{a}_i)^3 \lesssim \frac{p}{n_\alpha^3}\|\boldsymbol{\alpha}\|^6.$$

By Condition **??**, we have

$$\sum_{i=1}^p a_i^2 = \sum_{m=1}^{p_b}\sum_{i\in\mathcal{N}(m)}\left(\sum_{j\in\mathcal{N}(m)}\boldsymbol{\Sigma}_{\alpha,ij}\alpha_j\right)^2 \lesssim \sum_{i=1}^p \alpha_j^2 = \|\boldsymbol{\alpha}\|_2^2,$$

$$\sum_{i=1}^p a_i^4 = \sum_{m=1}^{p_b}\sum_{i\in\mathcal{N}(m)}\left(\sum_{j\in\mathcal{N}(m)}\boldsymbol{\Sigma}_{\alpha,ij}\alpha_j\right)^4 \lesssim \sum_{i=1}^p \alpha_j^4 = \|\boldsymbol{\alpha}\|_4^4,$$

and

$$\sum_{i=1}^p a_i^6 = \sum_{m=1}^{p_b}\sum_{i\in\mathcal{N}(m)}\left(\sum_{j\in\mathcal{N}(m)}\boldsymbol{\Sigma}_{\alpha,ij}\alpha_j\right)^6 \lesssim \sum_{i=1}^p \alpha_j^6 = \|\boldsymbol{\alpha}\|_6^6.$$

Since the inverse of $\boldsymbol{\Sigma}_\alpha$ is also block-diagonal with bounded eigenvalues, we have

$$\|\boldsymbol{\alpha}\|_4^4 \lesssim \sum_{i=1}^p a_i^4.$$

It follows that

$$\sum_{i=1}^p \boldsymbol{w}_{a,i} \lesssim \|\boldsymbol{\alpha}\|_2^2 + \frac{p}{n_\alpha}\|\boldsymbol{\alpha}\|_2^2,$$

$$\left(\|\boldsymbol{\alpha}\|_4^4+\frac{p}{n_\alpha^2}\|\boldsymbol{\alpha}\|_2^4\right)^{1/2}\lesssim\|\boldsymbol{w}_a\|_2\lesssim\left(\|\boldsymbol{\alpha}\|_4^4+\frac{p}{n_\alpha^2}\|\boldsymbol{\alpha}\|_2^4\right)^{1/2},$$

and

$$\|\boldsymbol{w}_a\|_3\lesssim\left(\|\boldsymbol{\alpha}\|_6^6+\frac{p}{n_\alpha^3}\|\boldsymbol{\alpha}\|_2^6\right)^{1/3}.$$

□

Lemmas S12-S14 summarize some useful results for multivariate Gaussian random variables.

LEMMA S12. *Suppose that $\boldsymbol{\epsilon}\sim N_n(\mathbf{0},\sigma^2\boldsymbol{I}_n)$ and $\boldsymbol{A}$ is a $n\times n$ symmetric matrix. Then we have $\boldsymbol{\epsilon}^T\boldsymbol{A}\boldsymbol{\epsilon}/\sigma^2\sim\sum_{i=1}^n\lambda_i\chi^2(1)$, $E(\boldsymbol{\epsilon}^T\boldsymbol{A}\boldsymbol{\epsilon})=\sigma^2\sum_{i=1}^n\lambda_i=\sigma^2tr(\boldsymbol{A})$, $Var(\boldsymbol{\epsilon}^T\boldsymbol{A}\boldsymbol{\epsilon})=2\sigma^4\sum_{i=1}^n\lambda_i^2=2\sigma^4tr(\boldsymbol{A}^2)$, and $E(\boldsymbol{A}\boldsymbol{\epsilon}\cdot\boldsymbol{\epsilon}^T\boldsymbol{A}\boldsymbol{\epsilon})=\mathbf{0}$, where $\lambda_1,\dots,\lambda_n$ are eigenvalues of $\boldsymbol{A}$.*

PROOF. Since $\boldsymbol{A}$ is symmetric, by spectral decomposition, there exists a unitary matrix $\boldsymbol{U}$ such that $\boldsymbol{A}=\boldsymbol{U}\boldsymbol{\Lambda}\boldsymbol{U}^T$, where $\boldsymbol{\Lambda}$ is a diagonal matrix with eigenvalues $\lambda_1,\dots,\lambda_n$ as diagonal elements. Let $\boldsymbol{y}=\boldsymbol{U}^T\boldsymbol{\epsilon}$, we have

$$\boldsymbol{\epsilon}^T\boldsymbol{A}\boldsymbol{\epsilon}=\boldsymbol{y}^T\boldsymbol{\Lambda}\boldsymbol{y}=\sum_{i=1}^n\lambda_iy_i^2,$$

$$\boldsymbol{A}\boldsymbol{\epsilon}\cdot\boldsymbol{\epsilon}^T\boldsymbol{A}\boldsymbol{\epsilon}=\boldsymbol{U}\boldsymbol{\Lambda}\boldsymbol{U}^T\boldsymbol{\epsilon}\boldsymbol{y}^T\boldsymbol{\Lambda}\boldsymbol{y}=\boldsymbol{U}\boldsymbol{\Lambda}\boldsymbol{y}\cdot\left(\sum_{i=1}^n\lambda_iy_i^2\right),$$

and $\boldsymbol{y}\sim N_n(\mathbf{0},\sigma^2\boldsymbol{I}_n)$, where $y_i$ is the $i$th element in $\boldsymbol{y}$. Thus, we have

$$E(\boldsymbol{A}\boldsymbol{\epsilon}\cdot\boldsymbol{\epsilon}^T\boldsymbol{A}\boldsymbol{\epsilon})=\boldsymbol{U}\boldsymbol{\Lambda}E\left\{\boldsymbol{y}\cdot\left(\sum_{i=1}^n\lambda_iy_i^2\right)\right\}=\mathbf{0},$$

$(y_i/\sigma)^2\sim\chi^2(1)$, $\boldsymbol{\epsilon}^T\boldsymbol{A}\boldsymbol{\epsilon}/\sigma^2\sim\sum_{i=1}^n\lambda_i\chi^2(1)$,

$$E(\boldsymbol{\epsilon}^T\boldsymbol{A}\boldsymbol{\epsilon})=\sum_{i=1}^n\lambda_iEy_i^2=\sigma^2\sum_{i=1}^n\lambda_i=\sigma^2\mathrm{tr}(\boldsymbol{A}),$$

and

$$\mathrm{Var}(\boldsymbol{\epsilon}^T\boldsymbol{A}\boldsymbol{\epsilon})=\sum_{i=1}^n\lambda_i^2\sigma^4\mathrm{Var}((y_i/\sigma)^2)=2\sigma^4\sum_{i=1}^n\lambda_i^2=2\sigma^4\mathrm{tr}(\boldsymbol{A}^2).$$

□

LEMMA S13. *Suppose that $\boldsymbol{\epsilon}\sim N_{n_1}(\mathbf{0},\sigma_1^2\boldsymbol{I}_{n_1})$, $\boldsymbol{\eta}\sim N_{n_2}(\mathbf{0},\sigma_2^2\boldsymbol{I}_{n_2})$, and $\boldsymbol{A}$ is a $n_1\times n_2$ matrix. Further assume that $\boldsymbol{\epsilon}$ and $\boldsymbol{\eta}$ are independent. Then we have $E(\boldsymbol{A}\boldsymbol{\eta}\cdot\boldsymbol{\epsilon}^T\boldsymbol{A}\boldsymbol{\eta})=\mathbf{0}$, $E(\boldsymbol{A}^T\boldsymbol{\epsilon}\cdot\boldsymbol{\epsilon}^T\boldsymbol{A}\boldsymbol{\eta})=\mathbf{0}$, $E(\boldsymbol{\epsilon}^T\boldsymbol{A}\boldsymbol{\eta})=0$, and $Var(\boldsymbol{\epsilon}^T\boldsymbol{A}\boldsymbol{\eta})=\sigma_1^2\sigma_2^2\sum_{i=1}^n\lambda_i^2=\sigma_1^2\sigma_2^2tr(\boldsymbol{A}\boldsymbol{A}^T)$, where $\lambda_1,\dots,\lambda_n$ are eigenvalues of $\boldsymbol{A}$.*

PROOF. By singular value decomposition, there exist unitary matrices $\boldsymbol{U}_{n_1\times n_1}$ and $\boldsymbol{V}_{n_2\times n_2}$ such that $\boldsymbol{A}=\boldsymbol{U}\boldsymbol{\Lambda}\boldsymbol{V}^T$, where $\boldsymbol{\Lambda}$ is a $n_1\times n_2$ rectangular diagonal matrix with singular values $\lambda_1,\ldots,\lambda_r$ as diagonal elements, and $r=\min\{n_1,n_2\}$. Let $\boldsymbol{y}=\boldsymbol{U}^T\boldsymbol{\epsilon}$ and $\boldsymbol{z}=\boldsymbol{V}^T\boldsymbol{\eta}$, we have

$$\boldsymbol{\epsilon}^T\boldsymbol{A}\boldsymbol{\eta}=\boldsymbol{y}^T\boldsymbol{\Lambda}\boldsymbol{z}=\sum_{i=1}^r\lambda_i y_i z_i,$$

$\boldsymbol{y}\sim N_{n_1}(\boldsymbol{0},\sigma_1^2\boldsymbol{I}_{n_1})$ and $\boldsymbol{z}\sim N_{n_2}(\boldsymbol{0},\sigma_2^2\boldsymbol{I}_{n_2})$, where $y_i$ is the $i$th element in $\boldsymbol{y}$ and $z_i$ is the $i$th element in $\boldsymbol{z}$. Thus, we have

$$E(\boldsymbol{A}\boldsymbol{\eta}\cdot\boldsymbol{\epsilon}^T\boldsymbol{A}\boldsymbol{\eta})=\boldsymbol{U}\boldsymbol{\Lambda}E\left\{\boldsymbol{z}\cdot\left(\sum_{i=1}^r\lambda_i y_i z_i\right)\right\}=\boldsymbol{0},$$

$$E(\boldsymbol{A}^T\boldsymbol{\epsilon}\cdot\boldsymbol{\epsilon}^T\boldsymbol{A}\boldsymbol{\eta})=\boldsymbol{V}\boldsymbol{\Lambda}^TE\left\{\boldsymbol{y}\cdot\left(\sum_{i=1}^r\lambda_i y_i z_i\right)\right\}=\boldsymbol{0},$$

$$E(\boldsymbol{\epsilon}^T\boldsymbol{A}\boldsymbol{\eta})=0,$$

and

$$\mathrm{Var}(\boldsymbol{\epsilon}^T\boldsymbol{A}\boldsymbol{\eta})=\sum_{i=1}^r\lambda_i^2\mathrm{Var}(y_i z_i)=\sigma_1^2\sigma_2^2\sum_{i=1}^r\lambda_i^2=\sigma_1^2\sigma_2^2\mathrm{tr}(\boldsymbol{A}\boldsymbol{A}^T).$$

□

LEMMA S14. *Suppose that $\boldsymbol{X}$ is a $n\times p$ matrix and $\boldsymbol{\alpha},\boldsymbol{\beta}\in R^p$, where each row $\boldsymbol{x}_i$ is i.i.d. from a multivariate Gaussian distribution $N_p(\boldsymbol{0},\boldsymbol{\Sigma})$. Then we have*

$$E[(\boldsymbol{\alpha}^T\boldsymbol{X}^T\boldsymbol{X}\boldsymbol{\beta})^2]=n\boldsymbol{\alpha}^T\boldsymbol{\Sigma}\boldsymbol{\alpha}\cdot\boldsymbol{\beta}^T\boldsymbol{\Sigma}\boldsymbol{\beta}+(n^2+n)(\boldsymbol{\alpha}^T\boldsymbol{\Sigma}\boldsymbol{\beta})^2.$$

PROOF. Let $\boldsymbol{a}=\boldsymbol{X}\boldsymbol{\alpha}$ and $\boldsymbol{b}=\boldsymbol{X}\boldsymbol{\beta}$. Then the elements $a_i$'s in $\boldsymbol{a}$ are i.i.d. Gaussian random variables with mean 0 and variance $\boldsymbol{\alpha}^T\boldsymbol{\Sigma}\boldsymbol{\alpha}$. Similarly, elements $b_i$'s in $\boldsymbol{b}$ are i.i.d. Gaussian random variables with mean 0 and variance $\boldsymbol{\beta}^T\boldsymbol{\Sigma}\boldsymbol{\beta}$. It follows that

$$E[(\boldsymbol{\alpha}^T\boldsymbol{X}^T\boldsymbol{X}\boldsymbol{\beta})^2]=E[(\sum_{i=1}^n a_i b_i)^2]=nE(a_1^2b_1^2)+n(n-1)(E(a_1b_1))^2.$$

□

LEMMA S15. *Suppose $\boldsymbol{\alpha}\in\mathbb{R}^p$ and $\boldsymbol{S}\in\mathbb{R}^{p\times p}$ is a symmetric matrix. Then we have $(\boldsymbol{\alpha}^T\boldsymbol{S}\boldsymbol{\alpha})^2\le(\boldsymbol{\alpha}^T\boldsymbol{\alpha})\cdot(\boldsymbol{\alpha}^T\boldsymbol{S}^2\boldsymbol{\alpha})$.*

PROOF. The proofs follow by applying diagonalization and the Cauchy–Schwarz inequality. □

The following proposition extends the results in [11, Proposition S1] to more general cases, which will be used in proof of Theorem **??**.

PROPOSITION S1. *Suppose $\boldsymbol{\alpha} \in \mathbb{R}^p$ and $\boldsymbol{W}$ follows a Wishart$(n_\alpha, \boldsymbol{\Sigma}_\alpha)$ distribution with a $p \times p$ positive-definite matrix $\boldsymbol{\Sigma}_\alpha$. Let $\boldsymbol{D}_\alpha$ be a $\mathbb{R}^{p\times p}$ diagonal matrix. Then we have*

$$E\left[tr(\boldsymbol{W}\boldsymbol{D}_\alpha)\right] = n_\alpha tr\left(\boldsymbol{\Sigma}_\alpha \boldsymbol{D}_\alpha\right),$$

$$E\left\{\left[tr(\boldsymbol{W}\boldsymbol{D}_\alpha)\right]^2\right\} = n_\alpha^2\left[tr\left(\boldsymbol{\Sigma}_\alpha \boldsymbol{D}_\alpha\right)\right]^2 + 2n_\alpha tr\left(\boldsymbol{\Sigma}_\alpha \boldsymbol{D}_\alpha \boldsymbol{\Sigma}_\alpha \boldsymbol{D}_\alpha\right),$$

$$E\left[tr(\boldsymbol{W}\boldsymbol{D}_\alpha \boldsymbol{W}\boldsymbol{D}_\alpha)\right] = n_\alpha(n_\alpha+1) tr\left(\boldsymbol{\Sigma}_\alpha \boldsymbol{D}_\alpha \boldsymbol{\Sigma}_\alpha \boldsymbol{D}_\alpha\right) + n_\alpha\left[tr\left(\boldsymbol{\Sigma}_\alpha \boldsymbol{D}_\alpha\right)\right]^2,$$

$$E(\boldsymbol{\alpha}^T \boldsymbol{W}\boldsymbol{D}_\alpha \boldsymbol{W}\boldsymbol{\alpha}) = n_\alpha(n_\alpha+1)\boldsymbol{\alpha}^T\boldsymbol{\Sigma}_\alpha \boldsymbol{D}_\alpha \boldsymbol{\Sigma}_\alpha \boldsymbol{\alpha} + n_\alpha tr\left(\boldsymbol{\Sigma}_\alpha \boldsymbol{D}_\alpha\right)\boldsymbol{\alpha}^T\boldsymbol{\Sigma}_\alpha\boldsymbol{\alpha},$$

$$\begin{aligned}
&E(\boldsymbol{\alpha}^T \boldsymbol{W}\boldsymbol{D}_\alpha \boldsymbol{W}\boldsymbol{D}_\alpha \boldsymbol{W}\boldsymbol{\alpha}) \\
=&n_\alpha(n_\alpha^2+3n_\alpha+4)\boldsymbol{\alpha}^T\boldsymbol{\Sigma}_\alpha \boldsymbol{D}_\alpha \boldsymbol{\Sigma}_\alpha \boldsymbol{D}_\alpha \boldsymbol{\Sigma}_\alpha \boldsymbol{\alpha} + n_\alpha\left[tr\left(\boldsymbol{\Sigma}_\alpha \boldsymbol{D}_\alpha\right)\right]^2\boldsymbol{\alpha}^T\boldsymbol{\Sigma}_\alpha\boldsymbol{\alpha} \\
&+2n_\alpha(n_\alpha+1) tr\left(\boldsymbol{\Sigma}_\alpha \boldsymbol{D}_\alpha\right)\boldsymbol{\alpha}^T\boldsymbol{\Sigma}_\alpha \boldsymbol{D}_\alpha \boldsymbol{\Sigma}_\alpha\boldsymbol{\alpha} + n_\alpha(n_\alpha+1) tr\left(\boldsymbol{\Sigma}_\alpha \boldsymbol{D}_\alpha \boldsymbol{\Sigma}_\alpha \boldsymbol{D}_\alpha\right)\boldsymbol{\alpha}^T\boldsymbol{\Sigma}_\alpha\boldsymbol{\alpha},
\end{aligned}$$

$$\begin{aligned}
&E\left[tr(\boldsymbol{W}\boldsymbol{D}_\alpha)\cdot \boldsymbol{\alpha}^T\boldsymbol{W}\boldsymbol{D}_\alpha\boldsymbol{W}\boldsymbol{\alpha}\right] \\
=&n_\alpha(n_\alpha^2+n_\alpha+2) tr\left(\boldsymbol{\Sigma}_\alpha \boldsymbol{D}_\alpha\right)\boldsymbol{\alpha}^T\boldsymbol{\Sigma}_\alpha \boldsymbol{D}_\alpha \boldsymbol{\Sigma}_\alpha\boldsymbol{\alpha} + n_\alpha^2\left[tr\left(\boldsymbol{\Sigma}_\alpha \boldsymbol{D}_\alpha\right)\right]^2\boldsymbol{\alpha}^T\boldsymbol{\Sigma}_\alpha\boldsymbol{\alpha} \\
&+4n_\alpha(n_\alpha+1)\boldsymbol{\alpha}^T\boldsymbol{\Sigma}_\alpha \boldsymbol{D}_\alpha \boldsymbol{\Sigma}_\alpha \boldsymbol{D}_\alpha \boldsymbol{\Sigma}_\alpha\boldsymbol{\alpha} + 2n_\alpha tr\left(\boldsymbol{\Sigma}_\alpha \boldsymbol{D}_\alpha \boldsymbol{\Sigma}_\alpha \boldsymbol{D}_\alpha\right)\boldsymbol{\alpha}^T\boldsymbol{\Sigma}_\alpha\boldsymbol{\alpha},
\end{aligned}$$

*and*

$$\begin{aligned}
&E\left[(\boldsymbol{\alpha}^T\boldsymbol{W}\boldsymbol{D}_\alpha\boldsymbol{W}\boldsymbol{\alpha})^2\right] \\
=&n_\alpha(n_\alpha+1)(n_\alpha+2)(n_\alpha+3)(\boldsymbol{\alpha}^T\boldsymbol{\Sigma}_\alpha \boldsymbol{D}_\alpha \boldsymbol{\Sigma}_\alpha\boldsymbol{\alpha})^2 \\
&+4n_\alpha(n_\alpha+2)(n_\alpha+3)\boldsymbol{\alpha}^T\boldsymbol{\Sigma}_\alpha\boldsymbol{\alpha}\cdot\boldsymbol{\alpha}^T\boldsymbol{\Sigma}_\alpha \boldsymbol{D}_\alpha \boldsymbol{\Sigma}_\alpha \boldsymbol{D}_\alpha \boldsymbol{\Sigma}_\alpha\boldsymbol{\alpha} \\
&+2n_\alpha(n_\alpha+2)(n_\alpha+3)\boldsymbol{\alpha}^T\boldsymbol{\Sigma}_\alpha\boldsymbol{\alpha}\cdot tr(\boldsymbol{\Sigma}_\alpha \boldsymbol{D}_\alpha)\boldsymbol{\alpha}^T\boldsymbol{\Sigma}_\alpha \boldsymbol{D}_\alpha \boldsymbol{\Sigma}_\alpha\boldsymbol{\alpha} \\
&+2n_\alpha(n_\alpha+2)(\boldsymbol{\alpha}^T\boldsymbol{\Sigma}_\alpha\boldsymbol{\alpha})^2 tr(\boldsymbol{\Sigma}_\alpha \boldsymbol{D}_\alpha \boldsymbol{\Sigma}_\alpha \boldsymbol{D}_\alpha) \\
&+n_\alpha(n_\alpha+2)(\boldsymbol{\alpha}^T\boldsymbol{\Sigma}_\alpha\boldsymbol{\alpha})^2\left[tr\left(\boldsymbol{\Sigma}_\alpha \boldsymbol{D}_\alpha\right)\right]^2.
\end{aligned}$$

PROOF. The proof steps for all equations are similar to those in [11, Proposition S1]. However, unlike [11, Proposition S1], our trace functionals are more general and include an additional diagonal matrix $\boldsymbol{D}_\alpha$. Therefore, in our proofs, we use the standard basis $\boldsymbol{e}_i$ $(1 \le i \le p)$ to account for both $\boldsymbol{D}_\alpha$ and $\boldsymbol{\alpha}$, where $\boldsymbol{e}_i$ is a $p$-dimensional column vector with all components equal to zero, except the $i$th component, which equals 1. This differs from the basis defined in [11, Proposition S1], which is only designed for the vector $\boldsymbol{\alpha}$.

Specifically, let $d_i$ be the $i$th diagonal element of $\boldsymbol{D}_\alpha$, $\alpha_i$ be the $i$th element in $\boldsymbol{\alpha}$,

$$\boldsymbol{H}_{ij} = \frac{\boldsymbol{e}_i\boldsymbol{e}_j^T + \boldsymbol{e}_i\boldsymbol{e}_j^T}{2}.$$

Then we have $\boldsymbol{D}_\alpha = \sum_{j=1}^p d_j\boldsymbol{e}_j\boldsymbol{e}_j^T$, $\boldsymbol{\alpha} = \sum_{i=1}^p \alpha_i\boldsymbol{e}_i$, and

$$\begin{aligned}
E(\boldsymbol{\alpha}^T\boldsymbol{W}\boldsymbol{D}_\alpha\boldsymbol{W}\boldsymbol{\alpha}) =&E\left[\left(\sum_{i=1}^p \alpha_i\boldsymbol{e}_i\right)^T\boldsymbol{W}\left(\sum_{j=1}^p d_j\boldsymbol{e}_j\boldsymbol{e}_j^T\right)\boldsymbol{W}\left(\sum_{l=1}^p \alpha_l\boldsymbol{e}_l\right)\right] \\
=&\sum_{i,j,l}\alpha_i d_j \alpha_l\cdot E\left[\boldsymbol{e}_i^T\boldsymbol{W}\boldsymbol{e}_j\boldsymbol{e}_j^T\boldsymbol{W}\boldsymbol{e}_l\right] \\
=&\sum_{i,j,l}\alpha_i d_j \alpha_l\cdot E\left[\mathrm{tr}(\boldsymbol{W}\boldsymbol{H}_{ij})\mathrm{tr}(\boldsymbol{W}\boldsymbol{H}_{jl})\right]
\end{aligned}$$

By [11, (S16)], we have

$$
\begin{aligned}
E(\boldsymbol{\alpha}^T \boldsymbol{W} \boldsymbol{D}_\alpha \boldsymbol{W} \boldsymbol{\alpha}) =& n_\alpha^2 \sum_{i,j,l} \alpha_i d_j \alpha_l \cdot \text{tr}(\boldsymbol{\Sigma} \boldsymbol{H}_{ij}) \cdot \text{tr}(\boldsymbol{\Sigma} \boldsymbol{H}_{jl}) \\
& + 2n_\alpha \sum_{i,j,l} \alpha_i d_j \alpha_l \cdot \text{tr}(\boldsymbol{\Sigma} \boldsymbol{H}_{ij} \boldsymbol{\Sigma} \boldsymbol{H}_{jl}) \\
=& n_\alpha^2 \sum_{i,j,l} \alpha_i d_j \alpha_l \cdot \boldsymbol{e}_i^T \boldsymbol{W} \boldsymbol{e}_j \cdot \boldsymbol{e}_j^T \boldsymbol{W} \boldsymbol{e}_l \\
& + \frac{n_\alpha}{2} \sum_{i,j,l} \alpha_i d_j \alpha_l \left[ \text{tr}(\boldsymbol{\Sigma} \boldsymbol{e}_i \boldsymbol{e}_j^T \boldsymbol{\Sigma} \boldsymbol{e}_j \boldsymbol{e}_l^T) + \text{tr}(\boldsymbol{\Sigma} \boldsymbol{e}_i \boldsymbol{e}_j^T \boldsymbol{\Sigma} \boldsymbol{e}_l \boldsymbol{e}_j^T) \right. \\
& \left. \text{tr}(\boldsymbol{\Sigma} \boldsymbol{e}_j \boldsymbol{e}_i^T \boldsymbol{\Sigma} \boldsymbol{e}_j \boldsymbol{e}_l^T) + \text{tr}(\boldsymbol{\Sigma} \boldsymbol{e}_j \boldsymbol{e}_i^T \boldsymbol{\Sigma} \boldsymbol{e}_l \boldsymbol{e}_j^T) \right] \\
& = n_\alpha (n_\alpha + 1) \boldsymbol{\alpha}^T \boldsymbol{\Sigma}_\alpha \boldsymbol{D}_\alpha \boldsymbol{\Sigma}_\alpha \boldsymbol{\alpha} + n_\alpha \text{tr} \left( \boldsymbol{\Sigma}_\alpha \boldsymbol{D}_\alpha \right) \boldsymbol{\alpha}^T \boldsymbol{\Sigma}_\alpha \boldsymbol{\alpha}.
\end{aligned}
$$

The calculations of other equations are similar and thus are skipped. □

Lemma S16 below quantifies the estimation accuracy of $\widehat{\mu}_{\boldsymbol{\ell}_a} = \widehat{\boldsymbol{\ell}}_a^T \mathbf{1}_p / p$ for the average of LD scores, which plays an important role in the proof of Theorem **??**.

LEMMA S16. *Under Condition **??**, we have*

$$
\frac{(\widehat{\boldsymbol{\ell}}_a - E\widehat{\boldsymbol{\ell}}_a)^T \mathbf{1}_p}{\bar{\rho}_a} \xrightarrow{d} N(0,1)
$$

*as* $\min(n_{r\alpha}, p) \to \infty$, *where* $\bar{\rho}_a^2 = Var(\widehat{\boldsymbol{\ell}}_a^T \mathbf{1}_p)$. *Moreover, we have* $\bar{\rho}_a \asymp \sqrt{p/n_{r\alpha}}$ *and*

$$
(E\widehat{\boldsymbol{\ell}}_a - \boldsymbol{\ell}_a)^T \mathbf{1}_p = O\left(\frac{p}{n_{r\alpha}}\right).
$$

PROOF. The proof is similar to that of Theorem **??**, with replacing $\boldsymbol{H}\boldsymbol{w}_a$ by $\mathbf{1}_p$. □

**S5. Estimated LD scores.** In this section, we present the proofs for Lemmas **??** and **??**. These lemmas provide the statistical properties of the estimated LD scores.

S5.1. *Proof of Lemma* **??**.

PROOF. Note that

(14)

$$
\text{Var}(\widehat{\boldsymbol{\ell}}_a^T \widehat{\boldsymbol{\ell}}_a) = \text{Var}(\sum_{m=1}^{p_b} \sum_{i \in \mathcal{N}(m)} \widehat{\ell}_{a,i}^2) = \sum_{m=1}^{p_b} \text{Var}(\sum_{i \in \mathcal{N}(m)} \widehat{\ell}_{a,i}^2) = \sum_{m=1}^{p_b} \sum_{i,j \in \mathcal{N}(m)} \text{Cov}(\widehat{\boldsymbol{\ell}}_{a,i}^2, \widehat{\boldsymbol{\ell}}_{a,j}^2),
$$

where

$$
\begin{aligned}
\text{Cov}(\widehat{\boldsymbol{\ell}}_{a,k}^2, \widehat{\boldsymbol{\ell}}_{a,j}^2) =& E(\widehat{\boldsymbol{\ell}}_{a,k}^2 \widehat{\boldsymbol{\ell}}_{a,j}^2) - E\widehat{\boldsymbol{\ell}}_{a,k}^2 E\widehat{\boldsymbol{\ell}}_{a,j}^2 \\
=& E\{(\sum_{i \in \mathcal{N}(m)} \widehat{\boldsymbol{\Sigma}}_{\alpha,ki}^2)^2 (\sum_{i \in \mathcal{N}(m)} \widehat{\boldsymbol{\Sigma}}_{\alpha,ji}^2)^2\} - E\{(\sum_{i \in \mathcal{N}(m)} \widehat{\boldsymbol{\Sigma}}_{\alpha,ki}^2)^2\} E\{(\sum_{i \in \mathcal{N}(m)} \widehat{\boldsymbol{\Sigma}}_{\alpha,ji}^2)^2\} \\
=& \sum_{i,l,u,v \in \mathcal{N}(m)} \{E(\widehat{\boldsymbol{\Sigma}}_{\alpha,ki}^2 \widehat{\boldsymbol{\Sigma}}_{\alpha,kl}^2 \widehat{\boldsymbol{\Sigma}}_{\alpha,ju}^2 \widehat{\boldsymbol{\Sigma}}_{\alpha,jv}^2) - E(\widehat{\boldsymbol{\Sigma}}_{\alpha,ki}^2 \widehat{\boldsymbol{\Sigma}}_{\alpha,kl}^2) E(\widehat{\boldsymbol{\Sigma}}_{\alpha,ju}^2 \widehat{\boldsymbol{\Sigma}}_{\alpha,jv}^2)\}
\end{aligned}
$$

and

$$
\begin{aligned}
&E(\widehat{\boldsymbol{\Sigma}}^2_{\alpha,ki}\widehat{\boldsymbol{\Sigma}}^2_{\alpha,kl}\widehat{\boldsymbol{\Sigma}}^2_{\alpha,ju}\widehat{\boldsymbol{\Sigma}}^2_{\alpha,jv})\\
=&E\{(\widehat{\boldsymbol{\Sigma}}_{\alpha,ki}-\boldsymbol{\Sigma}_{\alpha,ki}+\boldsymbol{\Sigma}_{\alpha,ki})^2(\widehat{\boldsymbol{\Sigma}}_{\alpha,kl}-\boldsymbol{\Sigma}_{\alpha,kl}+\boldsymbol{\Sigma}_{\alpha,kl})^2(\widehat{\boldsymbol{\Sigma}}_{\alpha,ju}-\boldsymbol{\Sigma}_{\alpha,ju}\\
&+\boldsymbol{\Sigma}_{\alpha,ju})^2(\widehat{\boldsymbol{\Sigma}}_{\alpha,jv}-\boldsymbol{\Sigma}_{\alpha,jv}+\boldsymbol{\Sigma}_{\alpha,jv})^2\}\\
=&E\{(\widehat{\boldsymbol{\Sigma}}_{\alpha,ki}-\boldsymbol{\Sigma}_{\alpha,ki})^2(\widehat{\boldsymbol{\Sigma}}_{\alpha,kl}-\boldsymbol{\Sigma}_{\alpha,kl})^2(\widehat{\boldsymbol{\Sigma}}_{\alpha,ju}-\boldsymbol{\Sigma}_{\alpha,ju})^2(\widehat{\boldsymbol{\Sigma}}_{\alpha,jv}-\boldsymbol{\Sigma}_{\alpha,jv})^2\}\\
&+\boldsymbol{\Sigma}^2_{\alpha,jv}E\{(\widehat{\boldsymbol{\Sigma}}_{\alpha,ki}-\boldsymbol{\Sigma}_{\alpha,ki})^2(\widehat{\boldsymbol{\Sigma}}_{\alpha,kl}-\boldsymbol{\Sigma}_{\alpha,kl})^2(\widehat{\boldsymbol{\Sigma}}_{\alpha,ju}-\boldsymbol{\Sigma}_{\alpha,ju})^2\}\\
&+\dots\\
&+\boldsymbol{\Sigma}^2_{\alpha,jv}\boldsymbol{\Sigma}^2_{\alpha,ju}E\{(\widehat{\boldsymbol{\Sigma}}_{\alpha,ki}-\boldsymbol{\Sigma}_{\alpha,ki})^2(\widehat{\boldsymbol{\Sigma}}_{\alpha,kl}-\boldsymbol{\Sigma}_{\alpha,kl})^2\}\\
&+\boldsymbol{\Sigma}^2_{\alpha,jv}\boldsymbol{\Sigma}^2_{\alpha,kl}E\{(\widehat{\boldsymbol{\Sigma}}_{\alpha,ki}-\boldsymbol{\Sigma}_{\alpha,ki})^2(\widehat{\boldsymbol{\Sigma}}_{\alpha,ju}-\boldsymbol{\Sigma}_{\alpha,ju})^2\}\\
&+\dots\\
&+\boldsymbol{\Sigma}^2_{\alpha,jv}\boldsymbol{\Sigma}^2_{\alpha,ju}\boldsymbol{\Sigma}^2_{\alpha,kl}E\{(\widehat{\boldsymbol{\Sigma}}_{\alpha,ki}-\boldsymbol{\Sigma}_{\alpha,ki})^2\}\\
&+\dots\\
&+4\boldsymbol{\Sigma}^2_{\alpha,jv}\boldsymbol{\Sigma}^2_{\alpha,ju}\boldsymbol{\Sigma}_{\alpha,ki}\boldsymbol{\Sigma}_{\alpha,kl}E\{(\widehat{\boldsymbol{\Sigma}}_{\alpha,ki}-\boldsymbol{\Sigma}_{\alpha,ki})(\widehat{\boldsymbol{\Sigma}}_{\alpha,kl}-\boldsymbol{\Sigma}_{\alpha,kl})\}\\
&+4\boldsymbol{\Sigma}^2_{\alpha,jv}\boldsymbol{\Sigma}^2_{\alpha,kl}\boldsymbol{\Sigma}_{\alpha,ki}\boldsymbol{\Sigma}_{\alpha,ju}E\{(\widehat{\boldsymbol{\Sigma}}_{\alpha,ki}-\boldsymbol{\Sigma}_{\alpha,ki})(\widehat{\boldsymbol{\Sigma}}_{\alpha,ju}-\boldsymbol{\Sigma}_{\alpha,ju})\}\\
&+\dots\\
&+\boldsymbol{\Sigma}^2_{\alpha,jv}\boldsymbol{\Sigma}^2_{\alpha,ju}\boldsymbol{\Sigma}^2_{\alpha,ki}\boldsymbol{\Sigma}^2_{\alpha,kl}.
\end{aligned}
$$

Note that

$$
\begin{aligned}
&E(\widehat{\boldsymbol{\Sigma}}^2_{\alpha,ju}\widehat{\boldsymbol{\Sigma}}^2_{\alpha,jv})\\
=&E\{(\widehat{\boldsymbol{\Sigma}}_{\alpha,ju}-\boldsymbol{\Sigma}_{\alpha,ju}+\boldsymbol{\Sigma}_{\alpha,ju})^2(\widehat{\boldsymbol{\Sigma}}_{\alpha,jv}-\boldsymbol{\Sigma}_{\alpha,jv}+\boldsymbol{\Sigma}_{\alpha,jv})^2\}\\
=&E\{(\widehat{\boldsymbol{\Sigma}}_{\alpha,ju}-\boldsymbol{\Sigma}_{\alpha,ju})^2(\widehat{\boldsymbol{\Sigma}}_{\alpha,jv}-\boldsymbol{\Sigma}_{\alpha,jv})^2\}+4\boldsymbol{\Sigma}_{\alpha,ju}\boldsymbol{\Sigma}_{\alpha,jv}E\{(\widehat{\boldsymbol{\Sigma}}_{\alpha,ju}-\boldsymbol{\Sigma}_{\alpha,ju})(\widehat{\boldsymbol{\Sigma}}_{\alpha,jv}-\boldsymbol{\Sigma}_{\alpha,jv})\}\\
&+\boldsymbol{\Sigma}^2_{\alpha,jv}E\{(\widehat{\boldsymbol{\Sigma}}_{\alpha,ju}-\boldsymbol{\Sigma}_{\alpha,ju})^2\}+\boldsymbol{\Sigma}^2_{\alpha,ju}E\{(\widehat{\boldsymbol{\Sigma}}_{\alpha,jv}-\boldsymbol{\Sigma}_{\alpha,jv})^2\}+\cdots+\boldsymbol{\Sigma}^2_{\alpha,ju}\boldsymbol{\Sigma}^2_{\alpha,jv},
\end{aligned}
$$

$$
\begin{aligned}
&E\{(\widehat{\boldsymbol{\Sigma}}_{\alpha,ki}-\boldsymbol{\Sigma}_{\alpha,ki})(\widehat{\boldsymbol{\Sigma}}_{\alpha,ju}-\boldsymbol{\Sigma}_{\alpha,ju})\}\\
=&n_{r\alpha}^{-1}\cdot E[\{X_{\alpha,1k}X_{\alpha,1i}-E(X_{\alpha,1k}X_{\alpha,1i})\}\{X_{\alpha,1j}X_{\alpha,1u}-E(X_{\alpha,1j}X_{\alpha,1u})\}],
\end{aligned}
$$

and

$$
\begin{aligned}
&\sum_{i,l,u,v\in\mathcal{N}(m)}\boldsymbol{\Sigma}^2_{\alpha,jv}\boldsymbol{\Sigma}^2_{\alpha,kl}\boldsymbol{\Sigma}_{\alpha,ki}\boldsymbol{\Sigma}_{\alpha,ju}E\{(\widehat{\boldsymbol{\Sigma}}_{\alpha,ki}-\boldsymbol{\Sigma}_{\alpha,ki})(\widehat{\boldsymbol{\Sigma}}_{\alpha,ju}-\boldsymbol{\Sigma}_{\alpha,ju})\}\\
=&(\sum_{l\in\mathcal{N}(m)}\boldsymbol{\Sigma}^2_{\alpha,kl})(\sum_{v\in\mathcal{N}(m)}\boldsymbol{\Sigma}^2_{\alpha,jv})[\sum_{i,u\in\mathcal{N}(m)}\boldsymbol{\Sigma}_{\alpha,ki}\boldsymbol{\Sigma}_{\alpha,ju}E\{(\widehat{\boldsymbol{\Sigma}}_{\alpha,ki}-\boldsymbol{\Sigma}_{\alpha,ki})(\widehat{\boldsymbol{\Sigma}}_{\alpha,ju}-\boldsymbol{\Sigma}_{\alpha,ju})\}]\\
=&n_{r\alpha}^{-1}\cdot\ell_{a,k}\ell_{a,j}\boldsymbol{\Sigma}^T_{\alpha,\mathcal{N}(m)j}\text{Cov}(X_{\alpha,1k}\boldsymbol{X}_{\alpha,1\mathcal{N}(m)},X_{\alpha,1j}\boldsymbol{X}_{\alpha,1\mathcal{N}(m)})\boldsymbol{\Sigma}_{\alpha,\mathcal{N}(m)k}.
\end{aligned}
$$

Let $\boldsymbol{W}_m$ be a vector consisting of $X^2_{\alpha,1i}$ and $X_{\alpha,1i}X_{\alpha,1j}$ for $i,j\in\mathcal{N}(m)$ and $i\neq j$. We also let $\boldsymbol{v}_m$ be a corresponding vector consisting of $\ell_{a,i}\boldsymbol{\Sigma}_{\alpha,ii}$ and $(\ell_{a,i}+\ell_{a,j})\boldsymbol{\Sigma}_{\alpha,ij}$ for $i,j\in\mathcal{N}(m)$

and $i \neq j$. Let

$$T_{\alpha,1} = \sum_{m=1}^{p_b} \sum_{k,j \in \mathcal{N}(m)} \sum_{i,l,u,v \in \mathcal{N}(m)} \boldsymbol{\Sigma}_{\alpha,jv}^2 \boldsymbol{\Sigma}_{\alpha,kl}^2 \boldsymbol{\Sigma}_{\alpha,ki} \boldsymbol{\Sigma}_{\alpha,ju} E\{(\widehat{\boldsymbol{\Sigma}}_{\alpha,ki} - \boldsymbol{\Sigma}_{\alpha,ki})(\widehat{\boldsymbol{\Sigma}}_{\alpha,ju} - \boldsymbol{\Sigma}_{\alpha,ju})\},$$

then we have

$$\begin{aligned} T_{\alpha,1} =& n_{r\alpha}^{-1} \cdot \sum_{m=1}^{p_b} \sum_{k,j \in \mathcal{N}(m)} \ell_{a,k} \ell_{a,j} \boldsymbol{\Sigma}_{\alpha,\cdot j}^T \mathrm{Cov}(X_{\alpha,1k} \boldsymbol{X}_{\alpha,1\cdot}, X_{\alpha,1j} \boldsymbol{X}_{\alpha,1\cdot}) \boldsymbol{\Sigma}_{\alpha,\cdot k} \\ =& n_{r\alpha}^{-1} \cdot \sum_{m=1}^{p_b} \boldsymbol{v}_m^T \mathrm{Cov}(\boldsymbol{W}_m) \boldsymbol{v}_m \\ \geq& n_{r\alpha}^{-1} \cdot \sum_{m=1}^{p_b} \lambda_{\min}\{\mathrm{Cov}(\boldsymbol{W}_m)\} \|\boldsymbol{v}_m\|^2. \end{aligned}$$

Note that elements in $\boldsymbol{W}_m$ are unique elements in $\boldsymbol{X}_{\alpha,1\mathcal{N}(m)}^T \boldsymbol{X}_{\alpha,1\mathcal{N}(m)}$. Let $Y = \boldsymbol{X}_{\alpha,1\mathcal{N}(m)} \cdot \boldsymbol{\Sigma}_{\alpha,\mathcal{N}(m)\mathcal{N}(m)}^{-1/2}$, where $\boldsymbol{\Sigma}_{\alpha,\mathcal{N}(m)\mathcal{N}(m)}$ represents a sub-matrix of $\boldsymbol{\Sigma}_\alpha$ indexed by $\mathcal{N}(m)$. By Condition **??**, elements in $Y$ are independent Gaussian, implying that unique elements in $Y^T Y$ are uncorrelated with non-zero variance. Let $\mathcal{S}$ be the linear space spanned by unique elements in $Y^T Y$, which does not contain non-zero constant random variable. Since $\boldsymbol{X}_{\alpha,1\mathcal{N}(m)}^T \boldsymbol{X}_{\alpha,1\mathcal{N}(m)} = \boldsymbol{\Sigma}_\alpha Y^T Y \boldsymbol{\Sigma}_\alpha$, the linear space spanned by unique elements in $\boldsymbol{X}_{\alpha,1\mathcal{N}(m)}^T \boldsymbol{X}_{\alpha,1\mathcal{N}(m)}$ is also $\mathcal{S}$, indicating that $\lambda_{\min}\{\mathrm{Cov}(\boldsymbol{W}_m)\} > 0$. Also, under Condition **??**, we can show that $\lambda_{\max}\{\mathrm{Cov}(\boldsymbol{W}_m)\} < c$ for some positive constant $c$ and

$$\boldsymbol{\ell}_a^T \boldsymbol{\ell}_a \gtrsim p. \tag{15}$$

It follows that

$$T_{\alpha,1} \gtrsim \sum_{m=1}^{p_b} \|\boldsymbol{v}_m\|^2 / n_{r\alpha} \gtrsim \boldsymbol{\ell}_a^T \boldsymbol{\ell}_a / n_{r\alpha} \gtrsim p / n_{r\alpha}.$$

Note that there are multiple terms in (14) for $\mathrm{Var}(\widehat{\boldsymbol{\ell}}_a^T \widehat{\boldsymbol{\ell}}_a)$, which are equal to $T_{\alpha,1}$. Let $R$ denote the remaining parts. By Lemma S2 and Condition **??**, we have $|R| = o(p_b/n_{r\alpha}) = o(p/n_{r\alpha})$. Then

$$\mathrm{Var}(\widehat{\boldsymbol{\ell}}_a^T \widehat{\boldsymbol{\ell}}_a) \gtrsim T_{\alpha,1} - |R| \gtrsim p/n_{r\alpha}.$$

By Condition **??**, we also have

$$\mathrm{Var}(\widehat{\boldsymbol{\ell}}_a^T \widehat{\boldsymbol{\ell}}_a) \lesssim p/n_{r\alpha}.$$

It follows that $\rho_{l_a}^2 = \mathrm{Var}(\widehat{\boldsymbol{\ell}}_a^T \widehat{\boldsymbol{\ell}}_a) \asymp p/n_{r\alpha}$. Let

$$S = \frac{\widehat{\boldsymbol{\ell}}_a^T \widehat{\boldsymbol{\ell}}_a - E(\widehat{\boldsymbol{\ell}}_a^T \widehat{\boldsymbol{\ell}}_a)}{\rho_{l_a}}.$$

Then $\mathrm{Var}(S) = 1$. For $1 \leq m \leq p_b$, let $V_m = [\widehat{\boldsymbol{\ell}}_{a,\mathcal{N}(m)}^T \widehat{\boldsymbol{\ell}}_{a,\mathcal{N}(m)} - E\{\widehat{\boldsymbol{\ell}}_{a,\mathcal{N}(m)}^T \widehat{\boldsymbol{\ell}}_{a,\mathcal{N}(m)}\}]/\rho_{l_a}$, where $\widehat{\boldsymbol{\ell}}_{a,\mathcal{N}(m)}$ is a sub-vector of $\widehat{\boldsymbol{\ell}}_a$, consisting of elements corresponding to $\mathcal{N}(m)$. Then $V_1, \ldots, V_{p_b}$ are independent and $\sum_{m=1}^{p_b} V_m = S$. Let

$$\gamma_{l_a} = \sum_{m=1}^{p_b} E[|V_m|^3] = \rho_{l_a}^{-3} \cdot \sum_{m=1}^{p_b} E|\widehat{\boldsymbol{\ell}}_{a,\mathcal{N}(m)}^T \widehat{\boldsymbol{\ell}}_{a,\mathcal{N}(m)} - E[\widehat{\boldsymbol{\ell}}_{a,\mathcal{N}(m)}^T \widehat{\boldsymbol{\ell}}_{a,\mathcal{N}(m)}]|^3.$$

Since

$$\begin{aligned}
&E|\widehat{\boldsymbol{\ell}}_{a,\mathcal{N}(m)}^T\widehat{\boldsymbol{\ell}}_{a,\mathcal{N}(m)} - E[\widehat{\boldsymbol{\ell}}_{a,\mathcal{N}(m)}^T\widehat{\boldsymbol{\ell}}_{a,\mathcal{N}(m)}]|^3 \\
\lesssim &\sum_{j\in\mathcal{N}(m)} E|\widehat{\ell}_{a,j}^2 - E(\widehat{\ell}_{a,j}^2)|^3 \\
= &\sum_{j\in\mathcal{N}(m)} E|(\sum_{i\in\mathcal{N}(m)} \widehat{\boldsymbol{\Sigma}}_{\alpha,ji}^2)^2 - E(\sum_{i\in\mathcal{N}(m)} \widehat{\boldsymbol{\Sigma}}_{\alpha,ji}^2)^2|^3 \\
\lesssim &\sum_{j\in\mathcal{N}(m)} \sum_{i,k\in\mathcal{N}(m)} E|\widehat{\boldsymbol{\Sigma}}_{\alpha,ji}^2\widehat{\boldsymbol{\Sigma}}_{\alpha,jk}^2 - E(\widehat{\boldsymbol{\Sigma}}_{\alpha,ji}^2\widehat{\boldsymbol{\Sigma}}_{\alpha,jk}^2)|^3 \lesssim n_{r\alpha}^{-3/2},
\end{aligned}$$

we have

$$\gamma_{l_a} \lesssim \frac{p_b/n_{r\alpha}^{3/2}}{(p/n_{r\alpha})^{3/2}} \lesssim p^{-1/2} \to 0,$$

as $p\to\infty$. Then by the Berry–Esseen Theorem in [30], we have $S \xrightarrow{d} N(0,1)$ as $p\to\infty$. By (18), we have

$$\frac{E(\widehat{\boldsymbol{\ell}}_a^T\widehat{\boldsymbol{\ell}}_a) - (E\widehat{\boldsymbol{\ell}}_a)^T E\widehat{\boldsymbol{\ell}}_a}{p} = p^{-1}\cdot\sum_{i=1}^p \mathrm{Var}(\widehat{\ell}_{a,i}) = O(n_{r\alpha}^{-1}).$$

Note that, by Lemma S2, we also have

$$\frac{(E\widehat{\boldsymbol{\ell}}_a)^T(E\widehat{\boldsymbol{\ell}}_a) - \boldsymbol{\ell}_a^T\boldsymbol{\ell}_a}{p} = p^{-1}\cdot\sum_{j=1}^p\left[\left(\sum_{i\in\mathcal{N}(m)} E\widehat{\boldsymbol{\Sigma}}_{\alpha,ij}^2\right)^2 - \left(\sum_{i\in\mathcal{N}(m)} \boldsymbol{\Sigma}_{\alpha,ij}^2\right)^2\right] = O(n_{r\alpha}^{-1}).$$

□

S5.2. *Proof of Lemma* **??**.

PROOF. Note that

(16)

$$\mathrm{Var}(\widehat{\boldsymbol{\ell}}_{ab}^T\widehat{\boldsymbol{\ell}}_{ab}) = \mathrm{Var}(\sum_{m=1}^{p_b}\sum_{i\in\mathcal{N}(m)}\widehat{\ell}_{ab,i}^2) = \sum_{m=1}^{p_b}\mathrm{Var}(\sum_{i\in\mathcal{N}(m)}\widehat{\ell}_{ab,i}^2) = \sum_{m=1}^{p_b}\sum_{i,j\in\mathcal{N}(m)}\mathrm{Cov}(\widehat{\boldsymbol{\ell}}_{ab,i}^2,\widehat{\boldsymbol{\ell}}_{ab,j}^2),$$

where

$$\begin{aligned}
\mathrm{Cov}(\widehat{\boldsymbol{\ell}}_{ab,k}^2,\widehat{\boldsymbol{\ell}}_{ab,j}^2) =&E(\widehat{\boldsymbol{\ell}}_{ab,k}^2\widehat{\boldsymbol{\ell}}_{ab,j}^2) - E\widehat{\boldsymbol{\ell}}_{ab,k}^2 E\widehat{\boldsymbol{\ell}}_{ab,j}^2 \\
=&E\{(\sum_{i\in\mathcal{N}(m)}\widehat{\boldsymbol{\Sigma}}_{\alpha,ki}\widehat{\boldsymbol{\Sigma}}_{\beta,ki})^2(\sum_{i\in\mathcal{N}(m)}\widehat{\boldsymbol{\Sigma}}_{\alpha,ji}\widehat{\boldsymbol{\Sigma}}_{\beta,ji})^2\} \\
&- E\{(\sum_{i\in\mathcal{N}(m)}\widehat{\boldsymbol{\Sigma}}_{\alpha,ki}\widehat{\boldsymbol{\Sigma}}_{\beta,ki})^2\}E\{(\sum_{i\in\mathcal{N}(m)}\widehat{\boldsymbol{\Sigma}}_{\alpha,ji}\widehat{\boldsymbol{\Sigma}}_{\beta,ji})^2\} \\
=&\sum_{i,l,u,v\in\mathcal{N}(m)}\{E(\widehat{\boldsymbol{\Sigma}}_{\alpha,ki}\widehat{\boldsymbol{\Sigma}}_{\alpha,kl}\widehat{\boldsymbol{\Sigma}}_{\alpha,ju}\widehat{\boldsymbol{\Sigma}}_{\alpha,jv})E(\widehat{\boldsymbol{\Sigma}}_{\beta,ki}\widehat{\boldsymbol{\Sigma}}_{\beta,kl}\widehat{\boldsymbol{\Sigma}}_{\beta,ju}\widehat{\boldsymbol{\Sigma}}_{\beta,jv}) \\
&- E(\widehat{\boldsymbol{\Sigma}}_{\alpha,ki}\widehat{\boldsymbol{\Sigma}}_{\alpha,kl})E(\widehat{\boldsymbol{\Sigma}}_{\alpha,ju}\widehat{\boldsymbol{\Sigma}}_{\alpha,jv})E(\widehat{\boldsymbol{\Sigma}}_{\beta,ki}\widehat{\boldsymbol{\Sigma}}_{\beta,kl})E(\widehat{\boldsymbol{\Sigma}}_{\beta,ju}\widehat{\boldsymbol{\Sigma}}_{\beta,jv})\},
\end{aligned}$$

and

$$
\begin{aligned}
&E(\widehat{\boldsymbol{\Sigma}}_{\alpha,ki}\widehat{\boldsymbol{\Sigma}}_{\alpha,kl}\widehat{\boldsymbol{\Sigma}}_{\alpha,ju}\widehat{\boldsymbol{\Sigma}}_{\alpha,jv})\\
=&E\{(\widehat{\boldsymbol{\Sigma}}_{\alpha,ki}-\boldsymbol{\Sigma}_{\alpha,ki}+\boldsymbol{\Sigma}_{\alpha,ki})(\widehat{\boldsymbol{\Sigma}}_{\alpha,kl}-\boldsymbol{\Sigma}_{\alpha,kl}+\boldsymbol{\Sigma}_{\alpha,kl})(\widehat{\boldsymbol{\Sigma}}_{\alpha,ju}-\boldsymbol{\Sigma}_{\alpha,ju}\\
&+\boldsymbol{\Sigma}_{\alpha,ju})(\widehat{\boldsymbol{\Sigma}}_{\alpha,jv}-\boldsymbol{\Sigma}_{\alpha,jv}+\boldsymbol{\Sigma}_{\alpha,jv})\}\\
=&E\{(\widehat{\boldsymbol{\Sigma}}_{\alpha,ki}-\boldsymbol{\Sigma}_{\alpha,ki})(\widehat{\boldsymbol{\Sigma}}_{\alpha,kl}-\boldsymbol{\Sigma}_{\alpha,kl})(\widehat{\boldsymbol{\Sigma}}_{\alpha,ju}-\boldsymbol{\Sigma}_{\alpha,ju})(\widehat{\boldsymbol{\Sigma}}_{\alpha,jv}-\boldsymbol{\Sigma}_{\alpha,jv})\}\\
&+\boldsymbol{\Sigma}_{\alpha,jv}E\{(\widehat{\boldsymbol{\Sigma}}_{\alpha,ki}-\boldsymbol{\Sigma}_{\alpha,ki})(\widehat{\boldsymbol{\Sigma}}_{\alpha,kl}-\boldsymbol{\Sigma}_{\alpha,kl})(\widehat{\boldsymbol{\Sigma}}_{\alpha,ju}-\boldsymbol{\Sigma}_{\alpha,ju})\}\\
&+\dots\\
&+\boldsymbol{\Sigma}_{\alpha,jv}\boldsymbol{\Sigma}_{\alpha,ju}E\{(\widehat{\boldsymbol{\Sigma}}_{\alpha,ki}-\boldsymbol{\Sigma}_{\alpha,ki})(\widehat{\boldsymbol{\Sigma}}_{\alpha,kl}-\boldsymbol{\Sigma}_{\alpha,kl})\}\\
&+\boldsymbol{\Sigma}_{\alpha,jv}\boldsymbol{\Sigma}_{\alpha,kl}E\{(\widehat{\boldsymbol{\Sigma}}_{\alpha,ki}-\boldsymbol{\Sigma}_{\alpha,ki})(\widehat{\boldsymbol{\Sigma}}_{\alpha,ju}-\boldsymbol{\Sigma}_{\alpha,ju})\}\\
&+\dots\\
&+\boldsymbol{\Sigma}_{\alpha,jv}\boldsymbol{\Sigma}_{\alpha,ju}\boldsymbol{\Sigma}_{\alpha,ki}\boldsymbol{\Sigma}_{\alpha,kl}.
\end{aligned}
$$

Since

$$
\begin{aligned}
E(\widehat{\boldsymbol{\Sigma}}_{\alpha,ju}\widehat{\boldsymbol{\Sigma}}_{\alpha,jv})=&E\{(\widehat{\boldsymbol{\Sigma}}_{\alpha,ju}-\boldsymbol{\Sigma}_{\alpha,ju}+\boldsymbol{\Sigma}_{\alpha,ju})(\widehat{\boldsymbol{\Sigma}}_{\alpha,jv}-\boldsymbol{\Sigma}_{\alpha,jv}+\boldsymbol{\Sigma}_{\alpha,jv})\}\\
=&E\{(\widehat{\boldsymbol{\Sigma}}_{\alpha,ju}-\boldsymbol{\Sigma}_{\alpha,ju})(\widehat{\boldsymbol{\Sigma}}_{\alpha,jv}-\boldsymbol{\Sigma}_{\alpha,jv})\}+\boldsymbol{\Sigma}_{\alpha,ju}\boldsymbol{\Sigma}_{\alpha,jv},
\end{aligned}
$$

we have

$$
\begin{aligned}
&E(\widehat{\boldsymbol{\Sigma}}_{\alpha,ki}\widehat{\boldsymbol{\Sigma}}_{\alpha,kl})E(\widehat{\boldsymbol{\Sigma}}_{\alpha,ju}\widehat{\boldsymbol{\Sigma}}_{\alpha,jv})\\
=&E\{(\widehat{\boldsymbol{\Sigma}}_{\alpha,ki}-\boldsymbol{\Sigma}_{\alpha,ki})(\widehat{\boldsymbol{\Sigma}}_{\alpha,kl}-\boldsymbol{\Sigma}_{\alpha,kl})\}E\{(\widehat{\boldsymbol{\Sigma}}_{\alpha,ju}-\boldsymbol{\Sigma}_{\alpha,ju})(\widehat{\boldsymbol{\Sigma}}_{\alpha,jv}-\boldsymbol{\Sigma}_{\alpha,jv})\}\\
&+\boldsymbol{\Sigma}_{\alpha,ju}\boldsymbol{\Sigma}_{\alpha,jv}E\{(\widehat{\boldsymbol{\Sigma}}_{\alpha,ki}-\boldsymbol{\Sigma}_{\alpha,ki})(\widehat{\boldsymbol{\Sigma}}_{\alpha,kl}-\boldsymbol{\Sigma}_{\alpha,kl})\}\\
&+\boldsymbol{\Sigma}_{\alpha,ki}\boldsymbol{\Sigma}_{\alpha,kl}E\{(\widehat{\boldsymbol{\Sigma}}_{\alpha,ju}-\boldsymbol{\Sigma}_{\alpha,ju})(\widehat{\boldsymbol{\Sigma}}_{\alpha,jv}-\boldsymbol{\Sigma}_{\alpha,jv})\}\\
&+\boldsymbol{\Sigma}_{\alpha,jv}\boldsymbol{\Sigma}_{\alpha,ju}\boldsymbol{\Sigma}_{\alpha,ki}\boldsymbol{\Sigma}_{\alpha,kl}.
\end{aligned}
$$

Note that

$$
\begin{aligned}
&E\{(\widehat{\boldsymbol{\Sigma}}_{\alpha,ki}-\boldsymbol{\Sigma}_{\alpha,ki})(\widehat{\boldsymbol{\Sigma}}_{\alpha,ju}-\boldsymbol{\Sigma}_{\alpha,ju})\}\\
&=n_{r\alpha}^{-1}\cdot E[\{X_{\alpha,1k}X_{\alpha,1i}-E(X_{\alpha,1k}X_{\alpha,1i})\}\{X_{\alpha,1j}X_{\alpha,1u}-E(X_{\alpha,1j}X_{\alpha,1u})\}],
\end{aligned}
$$

and

$$
\begin{aligned}
&\sum_{i,l,u,v\in\mathcal{N}(m)}\boldsymbol{\Sigma}_{\beta,jv}\boldsymbol{\Sigma}_{\beta,ju}\boldsymbol{\Sigma}_{\beta,ki}\boldsymbol{\Sigma}_{\beta,kl}\boldsymbol{\Sigma}_{\alpha,kl}\boldsymbol{\Sigma}_{\alpha,jv}E\{(\widehat{\boldsymbol{\Sigma}}_{\alpha,ki}-\boldsymbol{\Sigma}_{\alpha,ki})(\widehat{\boldsymbol{\Sigma}}_{\alpha,ju}-\boldsymbol{\Sigma}_{\alpha,ju})\}\\
=&(\sum_{l\in\mathcal{N}(m)}\boldsymbol{\Sigma}_{\beta,kl}\boldsymbol{\Sigma}_{\alpha,kl})(\sum_{v\in\mathcal{N}(m)}\boldsymbol{\Sigma}_{\beta,jv}\boldsymbol{\Sigma}_{\alpha,jv})\\
&\cdot[\sum_{i,u\in\mathcal{N}(m)}\boldsymbol{\Sigma}_{\beta,ju}\boldsymbol{\Sigma}_{\beta,ki}E\{(\widehat{\boldsymbol{\Sigma}}_{\alpha,ki}-\boldsymbol{\Sigma}_{\alpha,ki})(\widehat{\boldsymbol{\Sigma}}_{\alpha,ju}-\boldsymbol{\Sigma}_{\alpha,ju})\}]\\
=&n_{r\alpha}^{-1}\cdot\ell_{ab,k}\ell_{ab,j}\boldsymbol{\Sigma}_{\beta,\mathcal{N}(m)j}^{T}\mathrm{Cov}(X_{\alpha,1k}\boldsymbol{X}_{\alpha,1\mathcal{N}(m)},X_{\alpha,1j}\boldsymbol{X}_{\alpha,1\mathcal{N}(m)})\boldsymbol{\Sigma}_{\beta,\mathcal{N}(m)k},
\end{aligned}
$$

where $\boldsymbol{\Sigma}_{\beta,\mathcal{N}(m)j}$ represents a column vector consisting of $\boldsymbol{\Sigma}_{\beta,ij}$ for $i\in\mathcal{N}(m)$ and $\boldsymbol{X}_{\alpha,1\mathcal{N}(m)}$ represents a row vector consisting of $\boldsymbol{X}_{\alpha,1i}$ for $i\in\mathcal{N}(m)$.

Let $\boldsymbol{W}_m$ be a vector consisting of $X_{\alpha,1i}^2$ and $X_{\alpha,1i}X_{\alpha,1j}$ for $i,j \in \mathcal{N}(m)$ and $i \neq j$. We also let $\boldsymbol{v}_m$ be a corresponding vector consisting of $\ell_{ab,i}\boldsymbol{\Sigma}_{\beta,ii}$ and $(\ell_{ab,i}+\ell_{ab,j})\boldsymbol{\Sigma}_{\beta,ij}$ for $i,j \in \mathcal{N}(m)$ and $i \neq j$. Let

$$T_{\alpha,1} = \sum_{m=1}^{p_b} \sum_{k,j\in\mathcal{N}(m)} \sum_{i,l,u,v\in\mathcal{N}(m)} \boldsymbol{\Sigma}_{\beta,jv}\boldsymbol{\Sigma}_{\beta,ju}\boldsymbol{\Sigma}_{\beta,ki}\boldsymbol{\Sigma}_{\beta,kl}\boldsymbol{\Sigma}_{\alpha,kl}\boldsymbol{\Sigma}_{\alpha,jv} \cdot E\{(\widehat{\boldsymbol{\Sigma}}_{\alpha,ki}-\boldsymbol{\Sigma}_{\alpha,ki})(\widehat{\boldsymbol{\Sigma}}_{\alpha,ju}-\boldsymbol{\Sigma}_{\alpha,ju})\},$$

then we have

$$\begin{aligned} T_{\alpha,1} =& n_{r\alpha}^{-1}\cdot \sum_{m=1}^{p_b}\sum_{k,j\in\mathcal{N}(m)} \ell_{ab,k}\ell_{ab,j}\boldsymbol{\Sigma}_{\beta,\cdot j}^T \mathrm{Cov}(X_{\alpha,1k}\boldsymbol{X}_{\alpha,1\cdot}, X_{\alpha,1j}\boldsymbol{X}_{\alpha,1\cdot})\boldsymbol{\Sigma}_{\beta,\cdot k} \\ =& n_{r\alpha}^{-1}\cdot \sum_{m=1}^{p_b} \boldsymbol{v}_m^T\mathrm{Cov}(\boldsymbol{W}_m)\boldsymbol{v}_m \\ \geq& n_{r\alpha}^{-1}\cdot \sum_{m=1}^{p_b} \lambda_{\min}\{\mathrm{Cov}(\boldsymbol{W}_m)\}\|\boldsymbol{v}_m\|^2. \end{aligned}$$

Note that elements in $\boldsymbol{W}_m$ are unique elements in $X_{\alpha,1\mathcal{N}(m)}^T X_{\alpha,1\mathcal{N}(m)}$. Let $Y = X_{\alpha,1\mathcal{N}(m)}\cdot \boldsymbol{\Sigma}_{\alpha,\mathcal{N}(m)\mathcal{N}(m)}^{-1/2}$, where $\boldsymbol{\Sigma}_{\alpha,\mathcal{N}(m)\mathcal{N}(m)}$ represents a sub-matrix of $\boldsymbol{\Sigma}_\alpha$ indexed by $\mathcal{N}(m)$. By Condition **??**, elements in $Y$ are independent Gaussian, implying that unique elements in $Y^TY$ are uncorrelated with non-zero variance. Let $\mathcal{S}$ be the linear space spanned by unique elements in $Y^TY$, which does not contain non-zero constant random variable. Since $X_{\alpha,1\mathcal{N}(m)}^T X_{\alpha,1\mathcal{N}(m)} = \boldsymbol{\Sigma}_\alpha Y^TY\boldsymbol{\Sigma}_\alpha$, the linear space spanned by unique elements in $X_{\alpha,1\mathcal{N}(m)}^T X_{\alpha,1\mathcal{N}(m)}$ is also $\mathcal{S}$, indicating that $\lambda_{\min}\{\mathrm{Cov}(\boldsymbol{W}_m)\} > 0$. Thus, by Condition **??** and (51), we have

$$T_{\alpha,1} \gtrsim \sum_{m=1}^{p_b} \|\boldsymbol{v}_m\|^2/n_{r\alpha} \gtrsim \boldsymbol{\ell}_{ab}^T\boldsymbol{\ell}_{ab}/n_{r\alpha} \gtrsim p/n_{r\alpha}.$$

Similarly, we can define $T_{\beta,1}$ and show that $T_{\beta,1} \gtrsim p/n_{r\beta}$. Note that there are multiple terms in (16) for $\mathrm{Var}(\widehat{\boldsymbol{\ell}}_{ab}^T\widehat{\boldsymbol{\ell}}_{ab})$, which are equal to $T_{\alpha,1}$ or $T_{\beta,1}$. Let $R$ denote the remaining parts. By Lemma S2 and Condition **??**, we have $|R| = O(p_b/n_{r\alpha}^2 + p_b/n_{r\beta}^2) = O(p/n_{r\alpha}^2 + p/n_{r\beta}^2)$. It follows that

$$\mathrm{Var}(\widehat{\boldsymbol{\ell}}_{ab}^T\widehat{\boldsymbol{\ell}}_{ab}) \gtrsim T_{\alpha,1} + T_{\beta,1} - |R| \gtrsim p/n_{r\alpha} + p/n_{r\beta}.$$

By Condition **??**, we have

$$\mathrm{Var}(\widehat{\boldsymbol{\ell}}_{ab}^T\widehat{\boldsymbol{\ell}}_{ab}) \lesssim p/n_{r\alpha} + p/n_{r\beta}.$$

Therefore,

$$\mathrm{Var}(\widehat{\boldsymbol{\ell}}_{ab}^T\widehat{\boldsymbol{\ell}}_{ab}) \asymp p/n_{r\alpha} + p/n_{r\beta}.$$

Let

$$S = \frac{\widehat{\boldsymbol{\ell}}_{ab}^T\widehat{\boldsymbol{\ell}}_{ab} - E\widehat{\boldsymbol{\ell}}_{ab}^T\widehat{\boldsymbol{\ell}}_{ab}}{\rho_{l_{ab}}},$$

then we have $\mathrm{Var}(S) = 1$. For $1 \leq m \leq p_b$, let

$$V_m = [\widehat{\boldsymbol{\ell}}_{ab,\mathcal{N}(m)}^T\widehat{\boldsymbol{\ell}}_{ab,\mathcal{N}(m)} - E\{\widehat{\boldsymbol{\ell}}_{ab,\mathcal{N}(m)}^T\widehat{\boldsymbol{\ell}}_{ab,\mathcal{N}(m)}\}]/\rho_{l_{ab}},$$

where $\widehat{\boldsymbol{\ell}}_{ab,\mathcal{N}(m)}$ is a sub-vector of $\widehat{\boldsymbol{\ell}}_{ab}$, consisting of elements corresponding to $\mathcal{N}(m)$. Note that $V_1,\ldots,V_{p_b}$ are independent and $\sum_{m=1}^{p_b} V_m = S$. Let

$$\gamma_{l_{ab}} = \sum_{m=1}^{p_b} E[|V_m|^3] = \frac{1}{\rho_{l_{ab}}^3}\sum_{m=1}^{p_b} E|\widehat{\boldsymbol{\ell}}_{ab,\mathcal{N}(m)}^T\widehat{\boldsymbol{\ell}}_{ab,\mathcal{N}(m)} - E[\widehat{\boldsymbol{\ell}}_{ab,\mathcal{N}(m)}^T\widehat{\boldsymbol{\ell}}_{ab,\mathcal{N}(m)}]|^3.$$

Since

$$\begin{aligned}
&E|\widehat{\boldsymbol{\ell}}_{ab,\mathcal{N}(m)}^T\widehat{\boldsymbol{\ell}}_{ab,\mathcal{N}(m)} - E[\widehat{\boldsymbol{\ell}}_{ab,\mathcal{N}(m)}^T\widehat{\boldsymbol{\ell}}_{ab,\mathcal{N}(m)}]|^3\\
\lesssim &\sum_{j\in\mathcal{N}(m)} E|\widehat{\boldsymbol{\ell}}_{ab,j}^2 - E(\widehat{\boldsymbol{\ell}}_{ab,j}^2)|^3\\
= &\sum_{j\in\mathcal{N}(m)} E|(\sum_{i\in\mathcal{N}(m)}\widehat{\boldsymbol{\Sigma}}_{\alpha,ji}\widehat{\boldsymbol{\Sigma}}_{\beta,ji})^2 - E(\sum_{i\in\mathcal{N}(m)}\widehat{\boldsymbol{\Sigma}}_{\alpha,ji}\widehat{\boldsymbol{\Sigma}}_{\beta,ji})^2|^3\\
\lesssim &\sum_{j\in\mathcal{N}(m)}\sum_{i,k\in\mathcal{N}(m)} E|\widehat{\boldsymbol{\Sigma}}_{\alpha,ji}\widehat{\boldsymbol{\Sigma}}_{\beta,ji}\widehat{\boldsymbol{\Sigma}}_{\alpha,jk}\widehat{\boldsymbol{\Sigma}}_{\beta,jk} - E(\widehat{\boldsymbol{\Sigma}}_{\alpha,ji}\widehat{\boldsymbol{\Sigma}}_{\alpha,jk})E(\widehat{\boldsymbol{\Sigma}}_{\beta,ji}\widehat{\boldsymbol{\Sigma}}_{\beta,jk})|^3\\
\lesssim &n_{r\alpha}^{-3/2} + n_{r\beta}^{-3/2},
\end{aligned}$$

we have

$$\gamma_{l_{ab}} \lesssim \frac{p_b/n_{r\alpha}^{3/2} + p_b/n_{r\beta}^{3/2}}{(p/n_{r\alpha} + p/n_{r\beta})^{3/2}} \lesssim p^{-1/2} \to 0,$$

as $p\to\infty$. By the Berry–Esseen Theorem in [30], we have $S \xrightarrow{d} N(0,1)$ as $p\to\infty$. By (44), we have

$$\frac{E(\widehat{\boldsymbol{\ell}}_{ab}^T\widehat{\boldsymbol{\ell}}_{ab}) - \boldsymbol{\ell}_{ab}^T\boldsymbol{\ell}_{ab}}{p} = p^{-1}\cdot\sum_{i=1}^{p}\text{Var}(\widehat{\ell}_{ab,i}) = O(n_{r\alpha}^{-1} + n_{r\beta}^{-1}).$$

□

**S6. Univariate LDSC.** In this section, we present the proofs of Theorems **??**-**??** and S1. We begin by providing more derivations of the univariate LDSC estimator. Recall that $\sigma_\alpha^2 = \sum_{i=1}^p \alpha_i^2/p$ and $\ell_{a,j} = \sum_{i=1}^p \boldsymbol{\Sigma}_{\alpha,ji}^2$, we have

$$\begin{aligned}
E\widehat{a}_j^2 =& E\left(n_\alpha^{-1}\cdot\boldsymbol{X}_{\alpha,\cdot j}^T\boldsymbol{X}_\alpha\boldsymbol{\alpha} + n_\alpha^{-1}\cdot\boldsymbol{X}_{\alpha,\cdot j}^T\boldsymbol{\epsilon}_\alpha\right)^2\\
=&\boldsymbol{\alpha}^T E\left(n_\alpha^{-2}\cdot\boldsymbol{X}_\alpha^T\boldsymbol{X}_{\alpha,\cdot j}\cdot\boldsymbol{X}_{\alpha,\cdot j}^T\boldsymbol{X}_\alpha\right)\boldsymbol{\alpha} + 2\boldsymbol{\alpha}^T E\left(n_\alpha^{-2}\cdot\boldsymbol{X}_\alpha^T\boldsymbol{X}_{\alpha,\cdot j}\cdot\boldsymbol{X}_{\alpha,\cdot j}^T\boldsymbol{\epsilon}_\alpha\right)\\
&+ E\left(n_\alpha^{-2}\cdot\boldsymbol{\epsilon}_\alpha^T\boldsymbol{X}_{\alpha,\cdot j}\cdot\boldsymbol{X}_{\alpha,\cdot j}^T\boldsymbol{\epsilon}_\alpha\right)\\
=&\boldsymbol{\alpha}^T E(\widetilde{\boldsymbol{\Sigma}}_{\alpha,j}\widetilde{\boldsymbol{\Sigma}}_{\alpha,j}^T)\boldsymbol{\alpha} + n_\alpha^{-1}\cdot\sigma_{\epsilon_\alpha}^2\\
=&\sum_{i=1}^p \alpha_i^2 E(\widetilde{\boldsymbol{\Sigma}}_{\alpha,ij})^2 + \sum_{i\neq k}\alpha_i\alpha_k E(\widetilde{\boldsymbol{\Sigma}}_{\alpha,ij}\widetilde{\boldsymbol{\Sigma}}_{\alpha,kj}) + n_\alpha^{-1}\cdot\sigma_{\epsilon_\alpha}^2\\
=&\sum_{i=1}^p \alpha_i^2\boldsymbol{\Sigma}_{\alpha,ij}^2 + \sum_{i\neq k}\alpha_i\alpha_k\boldsymbol{\Sigma}_{\alpha,ij}\boldsymbol{\Sigma}_{\alpha,kj} + n_\alpha^{-1}\cdot\sum_{i=1}^p\alpha_i^2\text{Var}(\boldsymbol{X}_{\alpha,1i}\boldsymbol{X}_{\alpha,1j})\\
&+ n_\alpha^{-1}\cdot\sum_{i\neq k}\alpha_i\alpha_k\text{Cov}(\boldsymbol{X}_{\alpha,1i}\boldsymbol{X}_{\alpha,1j},\boldsymbol{X}_{\alpha,1j}\boldsymbol{X}_{\alpha,1k}) + n_\alpha^{-1}\cdot\sigma_{\epsilon_\alpha}^2
\end{aligned}$$

$$
\begin{aligned}
=&\sum_{i=1}^{p}\alpha_i^2\boldsymbol{\Sigma}_{\alpha,ij}^2+\sum_{i\neq k}\alpha_i\alpha_k\boldsymbol{\Sigma}_{\alpha,ij}\boldsymbol{\Sigma}_{\alpha,kj}+n_\alpha^{-1}\cdot\boldsymbol{\alpha}^T\text{Var}(\boldsymbol{X}_{\alpha,1j}\boldsymbol{X}_{\alpha,1\cdot})\boldsymbol{\alpha}+n_\alpha^{-1}\cdot\sigma_{\epsilon_\alpha}^2\\
=&\sigma_\alpha^2\sum_{i=1}^{p}\boldsymbol{\Sigma}_{\alpha,ij}^2+\sum_{i=1}^{p}\alpha_i^2\boldsymbol{\Sigma}_{\alpha,ij}^2-\sigma_\alpha^2\sum_{i=1}^{p}\boldsymbol{\Sigma}_{\alpha,ij}^2+\sum_{i\neq k}\alpha_i\alpha_k\boldsymbol{\Sigma}_{\alpha,ij}\boldsymbol{\Sigma}_{\alpha,kj}\\
&+n_\alpha^{-1}\cdot\boldsymbol{\alpha}^T\text{Var}(\boldsymbol{X}_{\alpha,1j}\boldsymbol{X}_{\alpha,1\cdot})\boldsymbol{\alpha}+n_\alpha^{-1}\cdot\sigma_{\epsilon_\alpha}^2\\
=&\sigma_\alpha^2\cdot\ell_{a,j}+\sum_{i=1}^{p}\alpha_i^2\boldsymbol{\Sigma}_{\alpha,ij}^2-\sigma_\alpha^2\sum_{i=1}^{p}\boldsymbol{\Sigma}_{\alpha,ij}^2+\sum_{i\neq k}\alpha_i\alpha_k\boldsymbol{\Sigma}_{\alpha,ij}\boldsymbol{\Sigma}_{\alpha,kj}\\
&+n_\alpha^{-1}\cdot\boldsymbol{\alpha}^T\text{Var}(\boldsymbol{X}_{\alpha,1j}\boldsymbol{X}_{\alpha,1\cdot})\boldsymbol{\alpha}+n_\alpha^{-1}\cdot\sigma_{\epsilon_\alpha}^2,
\end{aligned}
$$

where $\widetilde{\boldsymbol{\Sigma}}_{\alpha,j}$ is the $j$th column of $\widetilde{\boldsymbol{\Sigma}}_\alpha=\boldsymbol{X}_\alpha^T\boldsymbol{X}_\alpha/n_\alpha$ and $\widetilde{\boldsymbol{\Sigma}}_{\alpha,ij}$ is the $(i,j)$ element of $\widetilde{\boldsymbol{\Sigma}}_\alpha$.

S6.1. *Proof of Theorem* **??**.

PROOF. Let

$$
S_p=\frac{(\widehat{\boldsymbol{\ell}}_a-E\widehat{\boldsymbol{\ell}}_a)^T\boldsymbol{H}\boldsymbol{w}_a}{\rho_a},
$$

then $\text{Var}(S_p)=1$. Note that

$$
\text{Var}(\widehat{\boldsymbol{\ell}}_a^T\boldsymbol{H}\boldsymbol{w}_a)=\boldsymbol{H}\boldsymbol{w}_a^T\text{Cov}(\widehat{\boldsymbol{\ell}}_a)\boldsymbol{H}\boldsymbol{w}_a.
$$

Since the elements in $\widehat{\boldsymbol{\ell}}_a$ corresponding to genetic variants in different $\mathcal{N}$'s are independent under Condition **??**, $\text{Cov}(\widehat{\boldsymbol{\ell}}_a)$ is block-diagonal with the same structure as $\mathcal{A}$.

For $1\le m\le p_b$, let $W_m=(\widehat{\boldsymbol{\ell}}_{a,\mathcal{N}(m)}-E\widehat{\boldsymbol{\ell}}_{a,\mathcal{N}(m)})^T[\boldsymbol{H}\boldsymbol{w}_a]_{\mathcal{N}(m)}/\rho_a$, where $\widehat{\boldsymbol{\ell}}_{a,\mathcal{N}(m)}$ and $[\boldsymbol{H}\boldsymbol{w}_a]_{\mathcal{N}(m)}$ are sub-vectors of $\widehat{\boldsymbol{\ell}}_a$ and $\boldsymbol{H}\boldsymbol{w}_a$, respectively, consisting of elements corresponding to $\mathcal{N}(m)$. Then, $W_1,\dots,W_{p_b}$ are independent, and $\sum_{m=1}^{p_b}W_m=S_p$. For $j,k\in\mathcal{N}(m)$, we have

$$
\text{Cov}(\widehat{\ell}_{a,j},\widehat{\ell}_{a,k})=\sum_{i\in\mathcal{N}(m)}\sum_{l\in\mathcal{N}(m)}\text{Cov}(\widehat{\boldsymbol{\Sigma}}_{\alpha,ji}^2,\widehat{\boldsymbol{\Sigma}}_{\alpha,kl}^2).
$$

Note that

$$
\begin{aligned}
\text{Cov}(\widehat{\boldsymbol{\Sigma}}_{\alpha,ji}^2,\widehat{\boldsymbol{\Sigma}}_{\alpha,kl}^2)&=E(\widehat{\boldsymbol{\Sigma}}_{\alpha,ji}^2\widehat{\boldsymbol{\Sigma}}_{\alpha,kl}^2)-E(\widehat{\boldsymbol{\Sigma}}_{\alpha,ji}^2)E(\widehat{\boldsymbol{\Sigma}}_{\alpha,kl}^2)\\
&=4\boldsymbol{\Sigma}_{\alpha,ji}\boldsymbol{\Sigma}_{\alpha,kl}E\{(\widehat{\boldsymbol{\Sigma}}_{\alpha,ji}-\boldsymbol{\Sigma}_{\alpha,ji})(\widehat{\boldsymbol{\Sigma}}_{\alpha,kl}-\boldsymbol{\Sigma}_{\alpha,kl})\}+o(n_{r\alpha}^{-1}). \qquad (17)
\end{aligned}
$$

Since

$$
\begin{aligned}
&E\{(\widehat{\boldsymbol{\Sigma}}_{\alpha,kl}-\boldsymbol{\Sigma}_{\alpha,kl})(\widehat{\boldsymbol{\Sigma}}_{\alpha,ji}-\boldsymbol{\Sigma}_{\alpha,ji})\}\\
&=n_{r\alpha}^{-1}\cdot E[\{X_{\alpha,1k}X_{\alpha,1l}-E(X_{\alpha,1k}X_{\alpha,1l})\}\{X_{\alpha,1j}X_{\alpha,1i}-E(X_{\alpha,1j}X_{\alpha,1i})\}],
\end{aligned}
$$

we have

$$
\begin{aligned}
\text{Cov}(\widehat{\ell}_{a,j},\widehat{\ell}_{a,k})=&n_{r\alpha}^{-1}\cdot\sum_{i\in\mathcal{N}(m)}\sum_{l\in\mathcal{N}(m)}4\boldsymbol{\Sigma}_{\alpha,ji}\boldsymbol{\Sigma}_{\alpha,kl}\text{Cov}(X_{\alpha,1k}X_{\alpha,1l},X_{\alpha,1j}X_{\alpha,1i})+o(n_{r\alpha}^{-1})\\
=&4n_{r\alpha}^{-1}\cdot\boldsymbol{\Sigma}_{\alpha,k\mathcal{N}(m)}\text{Cov}(X_{\alpha,1k}X_{\alpha,1\mathcal{N}(m)},X_{\alpha,1j}X_{\alpha,1\mathcal{N}(m)})\boldsymbol{\Sigma}_{\alpha,j\mathcal{N}(m)}^T+o(n_{r\alpha}^{-1}). \qquad (18)
\end{aligned}
$$

It follows that

$$\begin{aligned}
&\mathrm{Var}(\widehat{\boldsymbol{\ell}}_a^T \boldsymbol{H}\boldsymbol{w}_a)\\
=&\sum_{m=1}^{p_b}\sum_{j,k\in\mathcal{N}(m)} [\boldsymbol{H}\boldsymbol{w}_a]_j[\boldsymbol{H}\boldsymbol{w}_a]_k \mathrm{Cov}(\widehat{\ell}_{a,j},\widehat{\ell}_{a,k})\\
=&4n_{r\alpha}^{-1}\cdot\sum_{m=1}^{p_b}\sum_{j,k\in\mathcal{N}(m)}\left\{\boldsymbol{\Sigma}_{\alpha,k\mathcal{N}(m)}\mathrm{Cov}(X_{\alpha,1k}X_{\alpha,1\mathcal{N}(m)},X_{\alpha,1j}X_{\alpha,1\mathcal{N}(m)})\boldsymbol{\Sigma}_{\alpha,j\mathcal{N}(m)}^T\right\}\\
&\cdot[\boldsymbol{H}\boldsymbol{w}_a]_j[\boldsymbol{H}\boldsymbol{w}_a]_k + o\left(\frac{\|\boldsymbol{H}\boldsymbol{w}_a\|^2}{n_{r\alpha}}\right), \qquad (19)
\end{aligned}$$

where $[\boldsymbol{H}\boldsymbol{w}_a]_j$ is the $j$th element of $\boldsymbol{H}\boldsymbol{w}_a$. Let $\boldsymbol{V}_m$ be a vector consisting of $X_{\alpha,1i}^2$ and $X_{\alpha,1i}X_{\alpha,1j}$ for $i,j\in\mathcal{N}(m)$ and $i\neq j$. We also let $\boldsymbol{v}_m$ be a corresponding vector consisting of $[\boldsymbol{H}\boldsymbol{w}_a]_i\boldsymbol{\Sigma}_{\alpha,ii}$ and $([\boldsymbol{H}\boldsymbol{w}_a]_i+[\boldsymbol{H}\boldsymbol{w}_a]_j)\boldsymbol{\Sigma}_{\alpha,ij}$ for $i,j\in\mathcal{N}(m)$ and $i\neq j$. Let

$$\begin{aligned}
T_{\alpha,1} =&4n_{r\alpha}^{-1}\cdot\sum_{m=1}^{p_b}\sum_{j,k\in\mathcal{N}(m)}[\boldsymbol{H}\boldsymbol{w}_a]_j[\boldsymbol{H}\boldsymbol{w}_a]_k\left\{\boldsymbol{\Sigma}_{\alpha,k\mathcal{N}(m)}\mathrm{Cov}(X_{\alpha,1k}X_{\alpha,1\mathcal{N}(m)},X_{\alpha,1j}X_{\alpha,1\mathcal{N}(m)})\right.\\
&\left.\boldsymbol{\Sigma}_{\alpha,j\mathcal{N}(m)}^T\right\}.
\end{aligned}$$

Therefore, we have

$$\begin{aligned}
T_{\alpha,1} =&4n_{r\alpha}^{-1}\cdot\sum_{m=1}^{p_b}\boldsymbol{v}_m^T\mathrm{Cov}(\boldsymbol{V}_m)\boldsymbol{v}_m\\
\geq& n_{r\alpha}^{-1}\cdot\sum_{m=1}^{p_b}\lambda_{\min}\{\mathrm{Cov}(\boldsymbol{V}_m)\}\|\boldsymbol{v}_m\|^2.
\end{aligned}$$

Note that elements in $\boldsymbol{V}_m$ are unique elements in $X_{\alpha,1\mathcal{N}(m)}^T X_{\alpha,1\mathcal{N}(m)}$. Let $Y = X_{\alpha,1\mathcal{N}(m)}\cdot\boldsymbol{\Sigma}_{\alpha,\mathcal{N}(m)\mathcal{N}(m)}^{-1/2}$, where $\boldsymbol{\Sigma}_{\alpha,\mathcal{N}(m)\mathcal{N}(m)}$ represents a sub-matrix of $\boldsymbol{\Sigma}_\alpha$ indexed by $\mathcal{N}(m)$. By Condition **??**, elements in $Y$ are independent Gaussian, implying that unique elements in $Y^TY$ are uncorrelated with non-zero variance. Let $\mathcal{S}$ be the linear space spanned by unique elements in $Y^TY$, which does not contain non-zero constant random variable. Since $X_{\alpha,1\mathcal{N}(m)}^T X_{\alpha,1\mathcal{N}(m)} = \boldsymbol{\Sigma}_\alpha Y^TY\boldsymbol{\Sigma}_\alpha$, the linear space spanned by unique elements in $X_{\alpha,1\mathcal{N}(m)}^T X_{\alpha,1\mathcal{N}(m)}$ is also $\mathcal{S}$, indicating that $\lambda_{\min}\{\mathrm{Cov}(\boldsymbol{V}_m)\}>0$. Thus, by Condition **??**, we have

$$T_{\alpha,1}\gtrsim\sum_{m=1}^{p_b}\|\boldsymbol{v}_m\|^2/n_{r\alpha}\gtrsim\|\boldsymbol{H}\boldsymbol{w}_a\|^2/n_{r\alpha}$$

and

$$T_{\alpha,1}\lesssim\|\boldsymbol{H}\boldsymbol{w}_a\|^2/n_{r\alpha}.$$

By (19), we have

$$\mathrm{Var}(\widehat{\boldsymbol{\ell}}_a^T\boldsymbol{H}\boldsymbol{w}_a)\asymp T_{\alpha,1}\asymp\|\boldsymbol{H}\boldsymbol{w}_a\|^2/n_{r\alpha}.$$

That is, $\rho_a\asymp\|\boldsymbol{H}\boldsymbol{w}_a\|/\sqrt{n_{r\alpha}}$. Let

$$\gamma_a=\sum_{m=1}^{p_b}E(|W_m|^3)=\frac{1}{\rho_a^3}\sum_{m=1}^{p_b}E\{|(\widehat{\ell}_{a,\mathcal{N}(m)}-E\widehat{\ell}_{a,\mathcal{N}(m)})^T[\boldsymbol{H}\boldsymbol{w}_a]_{\mathcal{N}(m)}|^3\}.$$

Then we have

$$\gamma_a \lesssim \frac{1}{\rho_a^3}\sum_{j=1}^{p} |[\boldsymbol{H}\boldsymbol{w}_a]_j|^3 E|\widehat{\ell}_{a,j} - E\widehat{\ell}_{a,j}|^3.$$

For $j \in \mathcal{N}(m)$, by Condition **??** and Lemma S2, we have

$$\begin{aligned} E|\widehat{\ell}_{a,j} - E\widehat{\ell}_{a,j}|^3 =& E|\sum_{i\in\mathcal{N}(m)} \widehat{\boldsymbol{\Sigma}}^2_{\alpha,ji} - \sum_{i\in\mathcal{N}(m)} E\widehat{\boldsymbol{\Sigma}}^2_{\alpha,ji}|^3 \\ \lesssim& \sum_{i\in\mathcal{N}(m)} E|\widehat{\boldsymbol{\Sigma}}_{\alpha,ji} - \boldsymbol{\Sigma}_{\alpha,ji}|^3 \\ \lesssim& n_{r\alpha}^{-3/2}. \end{aligned} \tag{20}$$

It follows that

$$\gamma_a \lesssim \frac{n_{r\alpha}^{-3/2}}{\rho_a^3}\|\boldsymbol{H}\boldsymbol{w}_a\|_3^3 \lesssim \frac{n_{r\alpha}^{-3/2}\|\boldsymbol{H}\boldsymbol{w}_a\|_3^3}{\|\boldsymbol{H}\boldsymbol{w}_a\|_2^3 n_{r\alpha}^{-3/2}} = \left(\frac{\|\boldsymbol{H}\boldsymbol{w}_a\|_3}{\|\boldsymbol{H}\boldsymbol{w}_a\|_2}\right)^3.$$

By Condition **??**, we have $\gamma_a = o(1)$, which implies the convergence in distribution to a normal distribution. By Lemma S3, we have

$$(E\widehat{\boldsymbol{\ell}}_a - \boldsymbol{\ell}_a)^T\boldsymbol{H}\boldsymbol{w}_a = \sum_{j=1}^{p}[\boldsymbol{H}\boldsymbol{w}_a]_j\left(\sum_{i\in\mathcal{N}(m)} E\widehat{\boldsymbol{\Sigma}}^2_{\alpha,ij} - \sum_{i\in\mathcal{N}(m)}\boldsymbol{\Sigma}^2_{\alpha,ij}\right) = O\left(\frac{\sum_{i=1}^p |[\boldsymbol{H}\boldsymbol{w}_a]_i|}{n_{r\alpha}}\right).$$

□

S6.2. *Proof of Theorem* **??**.

PROOF. Recall that $\widehat{\boldsymbol{w}}_a = (\widehat{a}_1^2,\dots,\widehat{a}_j^2,\dots,\widehat{a}_p^2)^T$, $\widehat{\boldsymbol{w}}_b = (\widehat{b}_1^2,\dots,\widehat{b}_j^2,\dots,\widehat{b}_p^2)^T$, and $\widehat{\boldsymbol{w}}_{ab} = (\widehat{a}_1\widehat{b}_1,\dots,\widehat{a}_j\widehat{b}_j,\dots,\widehat{a}_p\widehat{b}_p)^T$. We also recall that

$$\zeta_\alpha^2(\boldsymbol{\ell}_a) = \mathrm{Var}(\widetilde{\sigma}_\alpha^2) = (\boldsymbol{\ell}_a^T\boldsymbol{H}\boldsymbol{\ell}_a)^{-2}\mathrm{Var}(\boldsymbol{\ell}_a^T\boldsymbol{H}\widehat{\boldsymbol{w}}_a)$$

and $\boldsymbol{D}_\alpha = \mathrm{diag}([\boldsymbol{H}\boldsymbol{\ell}_a]_1,\dots,[\boldsymbol{H}\boldsymbol{\ell}_a]_p)$, where $[\boldsymbol{H}\boldsymbol{\ell}_a]_i$ is the $i$th element in $\boldsymbol{H}\boldsymbol{\ell}_a$. Since

$$\boldsymbol{\ell}_a^T\boldsymbol{H}\widehat{\boldsymbol{w}}_a = \sum_{j=1}^{p}[\boldsymbol{H}\boldsymbol{\ell}_a]_j\widehat{a}_j^2 = n_\alpha^{-2}\cdot\sum_{j=1}^{p}(\sqrt{[\boldsymbol{H}\boldsymbol{\ell}_a]_j}\boldsymbol{X}_{\alpha,\cdot j}^T\boldsymbol{y}_\alpha)^2 = n_\alpha^{-2}\cdot(\boldsymbol{X}_\alpha^T\boldsymbol{y}_\alpha)^T\boldsymbol{D}_\alpha\boldsymbol{X}_\alpha^T\boldsymbol{y}_\alpha,$$

we have

$$\mathrm{Var}(\boldsymbol{\ell}_a^T\boldsymbol{H}\widehat{\boldsymbol{w}}_a) = n_\alpha^{-4}\cdot\mathrm{Var}\left[(\boldsymbol{X}_\alpha^T\boldsymbol{y}_\alpha)^T\boldsymbol{D}_\alpha\boldsymbol{X}_\alpha^T\boldsymbol{y}_\alpha\right].$$

Note that

$$\begin{aligned}\mathrm{Var}\left[(\boldsymbol{X}_\alpha^T\boldsymbol{y}_\alpha)^T\boldsymbol{D}_\alpha\boldsymbol{X}_\alpha^T\boldsymbol{y}_\alpha\right] =& E\left\{\mathrm{Var}\left[(\boldsymbol{X}_\alpha^T\boldsymbol{y}_\alpha)^T\boldsymbol{D}_\alpha\boldsymbol{X}_\alpha^T\boldsymbol{y}_\alpha \mid \boldsymbol{X}_\alpha\right]\right\} \\ &+ \mathrm{Var}\left\{E\left[(\boldsymbol{X}_\alpha^T\boldsymbol{y}_\alpha)^T\boldsymbol{D}_\alpha\boldsymbol{X}_\alpha^T\boldsymbol{y}_\alpha \mid \boldsymbol{X}_\alpha)\right]\right\}.\end{aligned}$$

Since

$$\boldsymbol{D}_\alpha\boldsymbol{X}_\alpha^T\boldsymbol{y}_\alpha = \boldsymbol{D}_\alpha\boldsymbol{X}_\alpha^T(\boldsymbol{X}_\alpha\boldsymbol{\alpha}+\boldsymbol{\epsilon}_\alpha) = \boldsymbol{D}_\alpha\boldsymbol{X}_\alpha^T\boldsymbol{X}_\alpha\boldsymbol{\alpha} + \boldsymbol{D}_\alpha\boldsymbol{X}_\alpha^T\boldsymbol{\epsilon}_\alpha,$$

we have

$$
\begin{aligned}
&\text{Var}\left((\boldsymbol{X}_\alpha^T \boldsymbol{y}_\alpha)^T \boldsymbol{D}_\alpha \boldsymbol{X}_\alpha^T \boldsymbol{y}_\alpha \mid \boldsymbol{X}_\alpha\right) \\
=&4\text{Var}\left(\boldsymbol{\alpha}^T \boldsymbol{X}_\alpha^T \boldsymbol{X}_\alpha \boldsymbol{D}_\alpha \boldsymbol{X}_\alpha^T \boldsymbol{\epsilon}_\alpha \mid \boldsymbol{X}_\alpha\right) + \text{Var}\left(\boldsymbol{\epsilon}_\alpha^T \boldsymbol{X}_\alpha \boldsymbol{D}_\alpha \boldsymbol{X}_\alpha^T \boldsymbol{\epsilon}_\alpha \mid \boldsymbol{X}_\alpha\right) \\
&+ 4\text{Cov}\left(\boldsymbol{\alpha}^T \boldsymbol{X}_\alpha^T \boldsymbol{X}_\alpha \boldsymbol{D}_\alpha \boldsymbol{X}_\alpha^T \boldsymbol{\epsilon}_\alpha, \boldsymbol{\epsilon}_\alpha^T \boldsymbol{X}_\alpha \boldsymbol{D}_\alpha \boldsymbol{X}_\alpha^T \boldsymbol{\epsilon}_\alpha \mid \boldsymbol{X}_\alpha\right) \\
=&4\sigma_{\epsilon_\alpha}^2 \cdot \boldsymbol{\alpha}^T \boldsymbol{X}_\alpha^T \boldsymbol{X}_\alpha \boldsymbol{D}_\alpha \boldsymbol{X}_\alpha^T \boldsymbol{X}_\alpha \boldsymbol{D}_\alpha \boldsymbol{X}_\alpha^T \boldsymbol{X}_\alpha \boldsymbol{\alpha} + 2\sigma_{\epsilon_\alpha}^4 \cdot \text{tr}\{(\boldsymbol{X}_\alpha \boldsymbol{D}_\alpha \boldsymbol{X}_\alpha^T)^2\} \\
&+ 4\boldsymbol{\alpha}^T \boldsymbol{X}_\alpha^T E\left(\boldsymbol{X}_\alpha \boldsymbol{D}_\alpha \boldsymbol{X}_\alpha^T \boldsymbol{\epsilon}_\alpha \cdot \boldsymbol{\epsilon}_\alpha^T \boldsymbol{X}_\alpha \boldsymbol{D}_\alpha \boldsymbol{X}_\alpha^T \boldsymbol{\epsilon}_\alpha\right) \\
=&4\sigma_{\epsilon_\alpha}^2 \cdot \boldsymbol{\alpha}^T \boldsymbol{X}_\alpha^T \boldsymbol{X}_\alpha \boldsymbol{D}_\alpha \boldsymbol{X}_\alpha^T \boldsymbol{X}_\alpha \boldsymbol{D}_\alpha \boldsymbol{X}_\alpha^T \boldsymbol{X}_\alpha \boldsymbol{\alpha} + 2\sigma_{\epsilon_\alpha}^4 \cdot \text{tr}(\boldsymbol{D}_\alpha \boldsymbol{X}_\alpha^T \boldsymbol{X}_\alpha \boldsymbol{D}_\alpha \boldsymbol{X}_\alpha^T \boldsymbol{X}_\alpha).
\end{aligned}
$$

The last two equalities follow from $\boldsymbol{\epsilon}_\alpha \sim N(\mathbf{0}, \sigma_{\epsilon_\alpha}^2 \boldsymbol{I})$ and Lemma S12. In addition, we have

$$
\begin{aligned}
&E\left((\boldsymbol{X}_\alpha^T \boldsymbol{y}_\alpha)^T \boldsymbol{D}_\alpha \boldsymbol{X}_\alpha^T \boldsymbol{y}_\alpha \mid \boldsymbol{X}_\alpha\right) \\
=&\boldsymbol{\alpha}^T \boldsymbol{X}_\alpha^T \boldsymbol{X}_\alpha \boldsymbol{D}_\alpha \boldsymbol{X}_\alpha^T \boldsymbol{X}_\alpha \boldsymbol{\alpha} + E\left(\boldsymbol{\epsilon}_\alpha^T \boldsymbol{X}_\alpha \boldsymbol{D}_\alpha \boldsymbol{X}_\alpha^T \boldsymbol{\epsilon}_\alpha \mid \boldsymbol{X}_\alpha\right) \\
=&\boldsymbol{\alpha}^T \boldsymbol{X}_\alpha^T \boldsymbol{X}_\alpha \boldsymbol{D}_\alpha \boldsymbol{X}_\alpha^T \boldsymbol{X}_\alpha \boldsymbol{\alpha} + \sigma_{\epsilon_\alpha}^2 \cdot \text{tr}(\boldsymbol{X}_\alpha^T \boldsymbol{X}_\alpha \boldsymbol{D}_\alpha).
\end{aligned}
$$

It follows that

$$
\begin{aligned}
&\text{Var}\left[(\boldsymbol{X}_\alpha^T \boldsymbol{y}_\alpha)^T \boldsymbol{D}_\alpha \boldsymbol{X}_\alpha^T \boldsymbol{y}_\alpha\right] \\
=&4\sigma_{\epsilon_\alpha}^2 \cdot E\left\{\boldsymbol{\alpha}^T \boldsymbol{X}_\alpha^T \boldsymbol{X}_\alpha \boldsymbol{D}_\alpha \boldsymbol{X}_\alpha^T \boldsymbol{X}_\alpha \boldsymbol{D}_\alpha \boldsymbol{X}_\alpha^T \boldsymbol{X}_\alpha \boldsymbol{\alpha}\right\} + 2\sigma_{\epsilon_\alpha}^4 \cdot E\left[\text{tr}(\boldsymbol{D}_\alpha \boldsymbol{X}_\alpha^T \boldsymbol{X}_\alpha \boldsymbol{D}_\alpha \boldsymbol{X}_\alpha^T \boldsymbol{X}_\alpha)\right] \\
&+ \text{Var}\left\{\boldsymbol{\alpha}^T \boldsymbol{X}_\alpha^T \boldsymbol{X}_\alpha \boldsymbol{D}_\alpha \boldsymbol{X}_\alpha^T \boldsymbol{X}_\alpha \boldsymbol{\alpha} + \sigma_{\epsilon_\alpha}^2 \cdot \text{tr}(\boldsymbol{X}_\alpha^T \boldsymbol{X}_\alpha \boldsymbol{D}_\alpha)\right\} \\
=&4\sigma_{\epsilon_\alpha}^2 \cdot E\left\{\boldsymbol{\alpha}^T \boldsymbol{X}_\alpha^T \boldsymbol{X}_\alpha \boldsymbol{D}_\alpha \boldsymbol{X}_\alpha^T \boldsymbol{X}_\alpha \boldsymbol{D}_\alpha \boldsymbol{X}_\alpha^T \boldsymbol{X}_\alpha \boldsymbol{\alpha}\right\} + 2\sigma_{\epsilon_\alpha}^4 \cdot E\left[\text{tr}(\boldsymbol{D}_\alpha \boldsymbol{X}_\alpha^T \boldsymbol{X}_\alpha \boldsymbol{D}_\alpha \boldsymbol{X}_\alpha^T \boldsymbol{X}_\alpha)\right] \\
&+ E\left\{\boldsymbol{\alpha}^T \boldsymbol{X}_\alpha^T \boldsymbol{X}_\alpha \boldsymbol{D}_\alpha \boldsymbol{X}_\alpha^T \boldsymbol{X}_\alpha \boldsymbol{\alpha}\right\}^2 + \sigma_{\epsilon_\alpha}^4 \cdot E\left\{\text{tr}(\boldsymbol{X}_\alpha^T \boldsymbol{X}_\alpha \boldsymbol{D}_\alpha)\right\}^2 \\
&+ 2\sigma_{\epsilon_\alpha}^2 \cdot E\left\{\boldsymbol{\alpha}^T \boldsymbol{X}_\alpha^T \boldsymbol{X}_\alpha \boldsymbol{D}_\alpha \boldsymbol{X}_\alpha^T \boldsymbol{X}_\alpha \boldsymbol{\alpha} \cdot \text{tr}(\boldsymbol{X}_\alpha^T \boldsymbol{X}_\alpha \boldsymbol{D}_\alpha)\right\} \\
&- \left[E\left\{\boldsymbol{\alpha}^T \boldsymbol{X}_\alpha^T \boldsymbol{X}_\alpha \boldsymbol{D}_\alpha \boldsymbol{X}_\alpha^T \boldsymbol{X}_\alpha \boldsymbol{\alpha}\right\}\right]^2 - \sigma_{\epsilon_\alpha}^4 \cdot \left[E\left\{\text{tr}(\boldsymbol{X}_\alpha^T \boldsymbol{X}_\alpha \boldsymbol{D}_\alpha)\right\}\right]^2
\end{aligned}
$$

(21)

$$
- 2\sigma_{\epsilon_\alpha}^2 \cdot E\left\{\boldsymbol{\alpha}^T \boldsymbol{X}_\alpha^T \boldsymbol{X}_\alpha \boldsymbol{D}_\alpha \boldsymbol{X}_\alpha^T \boldsymbol{X}_\alpha \boldsymbol{\alpha}\right\} E\left\{\text{tr}(\boldsymbol{X}_\alpha^T \boldsymbol{X}_\alpha \boldsymbol{D}_\alpha)\right\}.
$$

Here $\boldsymbol{X}_\alpha$ is a $n \times p$ matrix with independent and identically distributed rows. By assuming that $\boldsymbol{X}_\alpha$ is normally distributed, each row in $\boldsymbol{X}_\alpha$ follows a multivariate normal distribution with mean $\mathbf{0}$ and covariance matrix $\boldsymbol{\Sigma}_\alpha$, which implies that $\boldsymbol{X}_\alpha^T \boldsymbol{X}_\alpha$ is a Wishart$(n, \boldsymbol{\Sigma}_\alpha)$. By Proposition S1, we have

$$
\begin{aligned}
&\text{Var}\left[(\boldsymbol{X}_\alpha^T \boldsymbol{y}_\alpha)^T \boldsymbol{D}_\alpha \boldsymbol{X}_\alpha^T \boldsymbol{y}_\alpha\right] \\
=&4\sigma_{\epsilon_\alpha}^2 \cdot \Big\{n_\alpha(n_\alpha+2)(n_\alpha+3)\boldsymbol{\alpha}^T \boldsymbol{\Sigma}_\alpha \boldsymbol{D}_\alpha \boldsymbol{\Sigma}_\alpha \boldsymbol{D}_\alpha \boldsymbol{\Sigma}_\alpha \boldsymbol{\alpha} + n_\alpha \left[\text{tr}\left(\boldsymbol{\Sigma}_\alpha \boldsymbol{D}_\alpha\right)\right]^2 \boldsymbol{\alpha}^T \boldsymbol{\Sigma}_\alpha \boldsymbol{\alpha} \\
&+n_\alpha(2n_\alpha+3)\text{tr}\left(\boldsymbol{\Sigma}_\alpha \boldsymbol{D}_\alpha\right) \boldsymbol{\alpha}^T \boldsymbol{\Sigma}_\alpha \boldsymbol{D}_\alpha \boldsymbol{\Sigma}_\alpha \boldsymbol{\alpha} + n_\alpha(n_\alpha+2)\text{tr}\left(\boldsymbol{\Sigma}_\alpha \boldsymbol{D}_\alpha \boldsymbol{\Sigma}_\alpha \boldsymbol{D}_\alpha\right) \boldsymbol{\alpha}^T \boldsymbol{\Sigma}_\alpha \boldsymbol{\alpha}\Big\} \\
&+ 2\sigma_{\epsilon_\alpha}^4 \cdot \Big\{n_\alpha(n_\alpha+2)\text{tr}\left(\boldsymbol{\Sigma}_\alpha \boldsymbol{D}_\alpha \boldsymbol{\Sigma}_\alpha \boldsymbol{D}_\alpha\right) + n_\alpha \left[\text{tr}\left(\boldsymbol{\Sigma}_\alpha \boldsymbol{D}_\alpha\right)\right]^2\Big\} \\
&+ 2n_\alpha(2n_\alpha^2+5n_\alpha+3)(\boldsymbol{\alpha}^T \boldsymbol{\Sigma}_\alpha \boldsymbol{D}_\alpha \boldsymbol{\Sigma}_\alpha \boldsymbol{\alpha})^2 + 2n_\alpha(\boldsymbol{\alpha}^T \boldsymbol{\Sigma}_\alpha \boldsymbol{\alpha})^2 \left[\text{tr}\left(\boldsymbol{\Sigma}_\alpha \boldsymbol{D}_\alpha\right)\right]^2 \\
&+ 4n_\alpha(n_\alpha+2)(n_\alpha+3)\boldsymbol{\alpha}^T \boldsymbol{\Sigma}_\alpha \boldsymbol{\alpha} \cdot \boldsymbol{\alpha}^T \boldsymbol{\Sigma}_\alpha \boldsymbol{D}_\alpha \boldsymbol{\Sigma}_\alpha \boldsymbol{D}_\alpha \boldsymbol{\Sigma}_\alpha \boldsymbol{\alpha} \\
&+ 4n_\alpha(2n_\alpha+3)\boldsymbol{\alpha}^T \boldsymbol{\Sigma}_\alpha \boldsymbol{\alpha} \cdot \text{tr}(\boldsymbol{\Sigma}_\alpha \boldsymbol{D}_\alpha)\boldsymbol{\alpha}^T \boldsymbol{\Sigma}_\alpha \boldsymbol{D}_\alpha \boldsymbol{\Sigma}_\alpha \boldsymbol{\alpha}
\end{aligned}
$$

$$+ 2n_\alpha(n_\alpha+2)(\boldsymbol{\alpha}^T\boldsymbol{\Sigma}_\alpha\boldsymbol{\alpha})^2\text{tr}(\boldsymbol{\Sigma}_\alpha\boldsymbol{D}_\alpha\boldsymbol{\Sigma}_\alpha\boldsymbol{D}_\alpha).$$

Thus,

$$\begin{aligned}
\zeta_\alpha^2(\boldsymbol{\ell}_a) =& (\boldsymbol{\ell}_a^T\boldsymbol{H}\boldsymbol{\ell}_a)^{-2}n_\alpha^{-4}\cdot \text{Var}\left[(\boldsymbol{X}_\alpha^T\boldsymbol{y}_\alpha)^T\boldsymbol{D}_\alpha\boldsymbol{X}_\alpha^T\boldsymbol{y}_\alpha\right] \\
=& \frac{2}{n_\alpha^3(\boldsymbol{\ell}_a^T\boldsymbol{H}\boldsymbol{\ell}_a)^2}\left[2\sigma_{\epsilon_\alpha}^2\cdot\left\{(n_\alpha+2)(n_\alpha+3)\boldsymbol{\alpha}^T\boldsymbol{\Sigma}_\alpha\boldsymbol{D}_\alpha\boldsymbol{\Sigma}_\alpha\boldsymbol{D}_\alpha\boldsymbol{\Sigma}_\alpha\boldsymbol{\alpha}\right.\right. \\
&+ \left[\text{tr}\left(\boldsymbol{\Sigma}_\alpha\boldsymbol{D}_\alpha\right)\right]^2\boldsymbol{\alpha}^T\boldsymbol{\Sigma}_\alpha\boldsymbol{\alpha} + (n_\alpha+2)\text{tr}\left(\boldsymbol{\Sigma}_\alpha\boldsymbol{D}_\alpha\boldsymbol{\Sigma}_\alpha\boldsymbol{D}_\alpha\right)\boldsymbol{\alpha}^T\boldsymbol{\Sigma}_\alpha\boldsymbol{\alpha} \\
&\left.+(2n_\alpha+3)\text{tr}\left(\boldsymbol{\Sigma}_\alpha\boldsymbol{D}_\alpha\right)\boldsymbol{\alpha}^T\boldsymbol{\Sigma}_\alpha\boldsymbol{D}_\alpha\boldsymbol{\Sigma}_\alpha\boldsymbol{\alpha}\right\} \\
&+ \sigma_{\epsilon_\alpha}^4\cdot\left\{(n_\alpha+2)\text{tr}\left(\boldsymbol{\Sigma}_\alpha\boldsymbol{D}_\alpha\boldsymbol{\Sigma}_\alpha\boldsymbol{D}_\alpha\right) + \left[\text{tr}\left(\boldsymbol{\Sigma}_\alpha\boldsymbol{D}_\alpha\right)\right]^2\right\} \\
&+ (2n_\alpha^2+5n_\alpha+3)(\boldsymbol{\alpha}^T\boldsymbol{\Sigma}_\alpha\boldsymbol{D}_\alpha\boldsymbol{\Sigma}_\alpha\boldsymbol{\alpha})^2 + (\boldsymbol{\alpha}^T\boldsymbol{\Sigma}_\alpha\boldsymbol{\alpha})^2\left[\text{tr}\left(\boldsymbol{\Sigma}_\alpha\boldsymbol{D}_\alpha\right)\right]^2 \\
&+ 2(n_\alpha+2)(n_\alpha+3)\boldsymbol{\alpha}^T\boldsymbol{\Sigma}_\alpha\boldsymbol{\alpha}\cdot\boldsymbol{\alpha}^T\boldsymbol{\Sigma}_\alpha\boldsymbol{D}_\alpha\boldsymbol{\Sigma}_\alpha\boldsymbol{D}_\alpha\boldsymbol{\Sigma}_\alpha\boldsymbol{\alpha} \\
&+ 2(2n_\alpha+3)\boldsymbol{\alpha}^T\boldsymbol{\Sigma}_\alpha\boldsymbol{\alpha}\cdot\text{tr}(\boldsymbol{\Sigma}_\alpha\boldsymbol{D}_\alpha)\boldsymbol{\alpha}^T\boldsymbol{\Sigma}_\alpha\boldsymbol{D}_\alpha\boldsymbol{\Sigma}_\alpha\boldsymbol{\alpha} \\
&\left.+(n_\alpha+2)(\boldsymbol{\alpha}^T\boldsymbol{\Sigma}_\alpha\boldsymbol{\alpha})^2\text{tr}(\boldsymbol{\Sigma}_\alpha\boldsymbol{D}_\alpha\boldsymbol{\Sigma}_\alpha\boldsymbol{D}_\alpha)\right].
\end{aligned}$$

By Lemma S15, we have $\boldsymbol{\alpha}^T\boldsymbol{\Sigma}_\alpha\boldsymbol{\alpha}\cdot\boldsymbol{\alpha}^T\boldsymbol{\Sigma}_\alpha\boldsymbol{D}_\alpha\boldsymbol{\Sigma}_\alpha\boldsymbol{D}_\alpha\boldsymbol{\Sigma}_\alpha\boldsymbol{\alpha} \geq (\boldsymbol{\alpha}^T\boldsymbol{\Sigma}_\alpha\boldsymbol{D}_\alpha\boldsymbol{\Sigma}_\alpha\boldsymbol{\alpha})^2$. It follows that

$$\begin{aligned}
&\text{Var}\left[(\boldsymbol{X}_\alpha^T\boldsymbol{y}_\alpha)^T\boldsymbol{D}_\alpha\boldsymbol{X}_\alpha^T\boldsymbol{y}_\alpha\right] \\
\geq& 4\sigma_{\epsilon_\alpha}^2\cdot\left\{n_\alpha(n_\alpha+2)(n_\alpha+3)\boldsymbol{\alpha}^T\boldsymbol{\Sigma}_\alpha\boldsymbol{D}_\alpha\boldsymbol{\Sigma}_\alpha\boldsymbol{D}_\alpha\boldsymbol{\Sigma}_\alpha\boldsymbol{\alpha}\right. \\
&\left.+n_\alpha(n_\alpha+2)\text{tr}\left(\boldsymbol{\Sigma}_\alpha\boldsymbol{D}_\alpha\boldsymbol{\Sigma}_\alpha\boldsymbol{D}_\alpha\right)\boldsymbol{\alpha}^T\boldsymbol{\Sigma}_\alpha\boldsymbol{\alpha}\right\} \\
&+ 2\sigma_{\epsilon_\alpha}^4\cdot n_\alpha(n_\alpha+2)\text{tr}\left(\boldsymbol{\Sigma}_\alpha\boldsymbol{D}_\alpha\boldsymbol{\Sigma}_\alpha\boldsymbol{D}_\alpha\right) \\
&+ 6n_\alpha(n_\alpha+2)\boldsymbol{\alpha}^T\boldsymbol{\Sigma}_\alpha\boldsymbol{\alpha}\cdot\boldsymbol{\alpha}^T\boldsymbol{\Sigma}_\alpha\boldsymbol{D}_\alpha\boldsymbol{\Sigma}_\alpha\boldsymbol{D}_\alpha\boldsymbol{\Sigma}_\alpha\boldsymbol{\alpha} \\
&+ 2n_\alpha(n_\alpha+2)(\boldsymbol{\alpha}^T\boldsymbol{\Sigma}_\alpha\boldsymbol{\alpha})^2\text{tr}(\boldsymbol{\Sigma}_\alpha\boldsymbol{D}_\alpha\boldsymbol{\Sigma}_\alpha\boldsymbol{D}_\alpha) \\
&+ \left[\sigma_{\epsilon_\alpha}^2(2n_\alpha)^{1/2}\text{tr}\left(\boldsymbol{\Sigma}_\alpha\boldsymbol{D}_\alpha\right) + (2n_\alpha)^{1/2}(2n+3)\boldsymbol{\alpha}^T\boldsymbol{\Sigma}_\alpha\boldsymbol{D}_\alpha\boldsymbol{\Sigma}_\alpha\boldsymbol{\alpha}\right. \\
&\left.+(2n_\alpha)^{1/2}\boldsymbol{\alpha}^T\boldsymbol{\Sigma}_\alpha\boldsymbol{\alpha}\cdot\text{tr}\left(\boldsymbol{\Sigma}_\alpha\boldsymbol{D}_\alpha\right)\right]^2 \\
\geq& 4\sigma_{\epsilon_\alpha}^2\cdot\left\{n_\alpha(n_\alpha+2)(n_\alpha+3)\boldsymbol{\alpha}^T\boldsymbol{\Sigma}_\alpha\boldsymbol{D}_\alpha\boldsymbol{\Sigma}_\alpha\boldsymbol{D}_\alpha\boldsymbol{\Sigma}_\alpha\boldsymbol{\alpha}\right. \\
&\left.+n_\alpha(n_\alpha+2)\text{tr}\left(\boldsymbol{\Sigma}_\alpha\boldsymbol{D}_\alpha\boldsymbol{\Sigma}_\alpha\boldsymbol{D}_\alpha\right)\boldsymbol{\alpha}^T\boldsymbol{\Sigma}_\alpha\boldsymbol{\alpha}\right\} \\
&+ 2\sigma_{\epsilon_\alpha}^4\cdot n_\alpha(n_\alpha+2)\text{tr}\left(\boldsymbol{\Sigma}_\alpha\boldsymbol{D}_\alpha\boldsymbol{\Sigma}_\alpha\boldsymbol{D}_\alpha\right) \\
&+ 6n_\alpha(n_\alpha+2)\boldsymbol{\alpha}^T\boldsymbol{\Sigma}_\alpha\boldsymbol{\alpha}\cdot\boldsymbol{\alpha}^T\boldsymbol{\Sigma}_\alpha\boldsymbol{D}_\alpha\boldsymbol{\Sigma}_\alpha\boldsymbol{D}_\alpha\boldsymbol{\Sigma}_\alpha\boldsymbol{\alpha} \\
&+ 2n_\alpha(n_\alpha+2)(\boldsymbol{\alpha}^T\boldsymbol{\Sigma}_\alpha\boldsymbol{\alpha})^2\text{tr}(\boldsymbol{\Sigma}_\alpha\boldsymbol{D}_\alpha\boldsymbol{\Sigma}_\alpha\boldsymbol{D}_\alpha).
\end{aligned}$$

By Condition **??** and Lemma S4, we have

$$\zeta_\alpha^2(\boldsymbol{\ell}_a) \gtrsim \frac{\|\boldsymbol{\alpha}\|^4\boldsymbol{\ell}_{a,\min}^2}{n_\alpha^2(\boldsymbol{\ell}_a^T\boldsymbol{H}\boldsymbol{\ell}_a)^2}\cdot(n_\alpha+p) \gtrsim \frac{\|\boldsymbol{\alpha}\|^4\boldsymbol{\ell}_{a,\min}^2}{n_\alpha(\boldsymbol{\ell}_a^T\boldsymbol{H}\boldsymbol{\ell}_a)^2}. \tag{22}$$

Also, since diagonal elements in $\boldsymbol{\Sigma}_\alpha$ are all ones under Condition **??**, we have $\text{tr}\left(\boldsymbol{\Sigma}_\alpha\boldsymbol{D}_\alpha\right) = 0$. Then we can rewrite $\zeta_\alpha^2(\boldsymbol{\ell}_a)$ as

$$\zeta_\alpha^2(\boldsymbol{\ell}_a) = \frac{2}{n_\alpha^3(\boldsymbol{\ell}_a^T\boldsymbol{H}\boldsymbol{\ell}_a)^2}\left[2\sigma_{\epsilon_\alpha}^2\cdot\left\{(n_\alpha+2)(n_\alpha+3)\boldsymbol{\alpha}^T\boldsymbol{\Sigma}_\alpha\boldsymbol{D}_\alpha\boldsymbol{\Sigma}_\alpha\boldsymbol{D}_\alpha\boldsymbol{\Sigma}_\alpha\boldsymbol{\alpha}\right.\right.$$

$$+(n_\alpha+2)\text{tr}\left(\boldsymbol{\Sigma}_\alpha\boldsymbol{D}_\alpha\boldsymbol{\Sigma}_\alpha\boldsymbol{D}_\alpha\right)\boldsymbol{\alpha}^T\boldsymbol{\Sigma}_\alpha\boldsymbol{\alpha}\Big\}+\sigma_{\epsilon_\alpha}^4\cdot(n_\alpha+2)\cdot\text{tr}\left(\boldsymbol{\Sigma}_\alpha\boldsymbol{D}_\alpha\boldsymbol{\Sigma}_\alpha\boldsymbol{D}_\alpha\right)$$
$$+\left(2n_\alpha^2+5n_\alpha+3\right)(\boldsymbol{\alpha}^T\boldsymbol{\Sigma}_\alpha\boldsymbol{D}_\alpha\boldsymbol{\Sigma}_\alpha\boldsymbol{\alpha})^2+(n_\alpha+2)(\boldsymbol{\alpha}^T\boldsymbol{\Sigma}_\alpha\boldsymbol{\alpha})^2\text{tr}(\boldsymbol{\Sigma}_\alpha\boldsymbol{D}_\alpha\boldsymbol{\Sigma}_\alpha\boldsymbol{D}_\alpha)$$
$$+2(n_\alpha+2)(n_\alpha+3)\boldsymbol{\alpha}^T\boldsymbol{\Sigma}_\alpha\boldsymbol{\alpha}\cdot\boldsymbol{\alpha}^T\boldsymbol{\Sigma}_\alpha\boldsymbol{D}_\alpha\boldsymbol{\Sigma}_\alpha\boldsymbol{D}_\alpha\boldsymbol{\Sigma}_\alpha\boldsymbol{\alpha}\Big]. \tag{23}$$

Note that

$$\begin{aligned}\widehat{a}_j &= n_\alpha^{-1}\cdot\sum_{i=1}^{n_\alpha}\boldsymbol{X}_{\alpha,ij}\boldsymbol{y}_{\alpha,i}\\ &= n_\alpha^{-1}\cdot\boldsymbol{X}_{\alpha,\cdot j}^T\boldsymbol{y}_\alpha\\ &= n_\alpha^{-1}\cdot\boldsymbol{X}_{\alpha,\cdot j}^T(\boldsymbol{X}_\alpha\boldsymbol{\alpha}+\boldsymbol{\epsilon}_\alpha)\\ &= n_\alpha^{-1}\cdot\boldsymbol{X}_{\alpha,\cdot j}^T\boldsymbol{X}_\alpha\boldsymbol{\alpha}+n_\alpha^{-1}\cdot\boldsymbol{X}_{\alpha,\cdot j}^T\boldsymbol{\epsilon}_\alpha,\end{aligned}$$

where $\boldsymbol{X}_{\alpha,ij}$ denotes the $(i,j)$th element in $\boldsymbol{X}_\alpha$, $\boldsymbol{y}_{\alpha,i}$ denotes the $i$th element in $\boldsymbol{y}_\alpha$, and $\boldsymbol{X}_{\alpha,\cdot j}$ denotes the $j$th column in $\boldsymbol{X}_\alpha$. Thus, $\widetilde{\sigma}_\alpha^2$ is a continuous function of $\boldsymbol{X}_\alpha$ and $\boldsymbol{\epsilon}_\alpha$. We use $g(\boldsymbol{X}_\alpha,\boldsymbol{\epsilon}_\alpha)$ to denote this function. Let

$$\mathcal{U}=\Big\{\widetilde{\boldsymbol{U}}=(\boldsymbol{u}\,\boldsymbol{U}):\boldsymbol{u}=(u_1,\ldots,u_{n_\alpha})\in\mathbb{R}^{n_\alpha},\boldsymbol{U}=(u_{ij})_{1\le i\le n_\alpha,1\le j\le p},$$
$$\sum_{k=1}^{n_\alpha}u_k^2+\sum_{i=1}^{n_\alpha}\sum_{j=1}^{p}u_{ij}^2=1\Big\}$$

be the collection of partitioned $n_\alpha\times(p+1)$ matrices with Frobenius norm equal to 1. For $\widetilde{\boldsymbol{U}}=(\boldsymbol{u}\,\boldsymbol{U})\in\mathcal{U}$, we define the differential operator

$$D_{\widetilde{\boldsymbol{U}}}=\sum_{i=1}^{n_\alpha}\sum_{j=1}^{p}u_{ij}\frac{\partial}{\partial\boldsymbol{X}_{\alpha,ij}}+\sum_{k=1}^{n_\alpha}u_k\frac{\partial}{\partial\boldsymbol{\epsilon}_{\alpha,i}}.$$

For $\widetilde{\boldsymbol{U}}\in\mathcal{U}$, we have

$$\|\boldsymbol{U}\|^2\le\|\boldsymbol{U}\|_F^2\le 1$$

and $\|\boldsymbol{u}\|\le 1$, where $\|\cdot\|_F$ denotes the Frobenius norm. Note that

$$\begin{aligned}\|\nabla g(\boldsymbol{X}_\alpha,\boldsymbol{\epsilon}_\alpha)\| &= \left\langle\frac{\nabla g(\boldsymbol{X}_\alpha,\boldsymbol{\epsilon}_\alpha)}{\|\nabla g(\boldsymbol{X}_\alpha,\boldsymbol{\epsilon}_\alpha)\|},\nabla g(\boldsymbol{X}_\alpha,\boldsymbol{\epsilon}_\alpha)\right\rangle\\ &\le\sup_{\widetilde{\boldsymbol{U}}\in\mathcal{U}}|D_{\widetilde{\boldsymbol{U}}}g(\boldsymbol{X}_\alpha,\boldsymbol{\epsilon}_\alpha)|\end{aligned}$$

and

$$D_{\widetilde{\boldsymbol{U}}}g(\boldsymbol{X}_\alpha,\boldsymbol{\epsilon}_\alpha)=\left\langle\widetilde{\boldsymbol{U}},\nabla g(\boldsymbol{X}_\alpha,\boldsymbol{\epsilon}_\alpha)\right\rangle\le\|\widetilde{\boldsymbol{U}}\|\|\nabla g(\boldsymbol{X}_\alpha,\boldsymbol{\epsilon}_\alpha)\|\le\|\nabla g(\boldsymbol{X}_\alpha,\boldsymbol{\epsilon}_\alpha)\|.$$

Then we have

$$\|\nabla g(\boldsymbol{X}_\alpha,\boldsymbol{\epsilon}_\alpha)\|=\sup_{\widetilde{\boldsymbol{U}}\in\mathcal{U}}|D_{\widetilde{\boldsymbol{U}}}g(\boldsymbol{X}_\alpha,\boldsymbol{\epsilon}_\alpha)|.$$

Note that

$$D_{\widetilde{\boldsymbol{U}}}g(\boldsymbol{X}_\alpha,\boldsymbol{\epsilon}_\alpha)=2(\boldsymbol{\ell}_a^T\boldsymbol{H}\boldsymbol{\ell}_a)^{-1}\sum_{k=1}^{p}[\boldsymbol{H}\boldsymbol{\ell}_a]_k\widehat{a}_k\cdot n_\alpha^{-1}\cdot\left[\boldsymbol{X}_{\alpha,\cdot k}^T\boldsymbol{U}\boldsymbol{\alpha}+\boldsymbol{U}_{\cdot k}^T\boldsymbol{X}_\alpha\boldsymbol{\alpha}+\boldsymbol{U}_{\cdot k}^T\boldsymbol{\epsilon}_\alpha+\boldsymbol{X}_{\alpha,\cdot k}^T\boldsymbol{u}\right],$$

where $\boldsymbol{U}_{\alpha,\cdot k}$ denotes the $k$th column in $\boldsymbol{U}$. Let $\eta_{x\alpha} = \|\boldsymbol{X}_\alpha/\sqrt{n}_\alpha\|$ , $\eta_{\epsilon\alpha} = \|\epsilon_\alpha/\sqrt{n}_\alpha\|$ , $\eta_\alpha = \|\boldsymbol{\alpha}\|$ , $\eta_{v\alpha} = \|\boldsymbol{\Sigma}_\alpha^{1/2}\|$ and $\eta_{x\epsilon\alpha} = \left\|\boldsymbol{X}_\alpha^T \boldsymbol{\epsilon}_\alpha/n_\alpha\right\|$. It follows that

$$\begin{aligned}\|\widehat{\boldsymbol{a}}\| =& n_\alpha^{-1} \cdot \|\boldsymbol{X}_\alpha^T \boldsymbol{X}_\alpha \boldsymbol{\alpha} + \boldsymbol{X}_\alpha^T \boldsymbol{\epsilon}_\alpha\| \\ \le& \|\boldsymbol{\alpha}\| \|\boldsymbol{X}_\alpha^T \boldsymbol{X}_\alpha/n_\alpha\| + \|\boldsymbol{X}_\alpha^T \boldsymbol{\epsilon}_\alpha/n_\alpha\| \\ =& \eta_\alpha \eta_{x\alpha}^2 + \eta_{x\epsilon\alpha}\end{aligned}$$

and

$$\begin{aligned}&\left|D_{\widetilde{\boldsymbol{U}}} g(\boldsymbol{X}_\alpha, \boldsymbol{\epsilon}_\alpha)\right| \\ \le& 2n_\alpha^{-1} \cdot (\boldsymbol{\ell}_a^T \boldsymbol{H} \boldsymbol{\ell}_a)^{-1} \boldsymbol{\ell}_{a,\max} \left|\widehat{\boldsymbol{a}}^T \left[\boldsymbol{X}_\alpha^T \boldsymbol{U}\boldsymbol{\alpha} + \boldsymbol{U}^T \boldsymbol{X}_\alpha \boldsymbol{\alpha} \; + \; \boldsymbol{U}^T \boldsymbol{\epsilon}_\alpha + \boldsymbol{X}_\alpha^T \boldsymbol{u}\right]\right| \\ \le& 2n_\alpha^{-1} \cdot (\boldsymbol{\ell}_a^T \boldsymbol{H} \boldsymbol{\ell}_a)^{-1} \boldsymbol{\ell}_{a,\max} \|\widehat{\boldsymbol{a}}\| \left[\|\boldsymbol{X}_\alpha^T \boldsymbol{U}\boldsymbol{\alpha}\| + \|\boldsymbol{U}^T \boldsymbol{X}_\alpha \boldsymbol{\alpha}\| \; + \|\boldsymbol{U}^T \boldsymbol{\epsilon}_\alpha\| + \|\boldsymbol{X}_\alpha^T \boldsymbol{u}\|\right] \\ \le& 2n_\alpha^{-1/2} \cdot (\boldsymbol{\ell}_a^T \boldsymbol{H} \boldsymbol{\ell}_a)^{-1} \boldsymbol{\ell}_{a,\max} (\eta_\alpha \eta_{x\alpha}^2 + \eta_{x\epsilon\alpha})(2\|\boldsymbol{U}\|\eta_\alpha \eta_{x\alpha} + \|\boldsymbol{U}\|\eta_{\epsilon\alpha} + \|\boldsymbol{u}\|\eta_{x\alpha}) \\ \le& 2n_\alpha^{-1/2} \cdot (\boldsymbol{\ell}_a^T \boldsymbol{H} \boldsymbol{\ell}_a)^{-1} \boldsymbol{\ell}_{a,\max} (\eta_\alpha \eta_{x\alpha}^2 + \eta_{x\epsilon\alpha})(2\eta_\alpha \eta_{x\alpha} + \eta_{\epsilon\alpha} + \eta_{x\alpha}).\end{aligned}$$

Then we have

$$\begin{aligned}&\left\{E\|\nabla g(\boldsymbol{X}_\alpha, \boldsymbol{\epsilon}_\alpha)\|^4\right\}^{1/4} \\ \le& 2n_\alpha^{-1/2} \cdot (\boldsymbol{\ell}_a^T \boldsymbol{H} \boldsymbol{\ell}_a)^{-1} \boldsymbol{\ell}_{a,\max} \left[E\{(\eta_\alpha \eta_{x\alpha}^2 + \eta_{x\epsilon\alpha})^4 (2\eta_\alpha \eta_{x\alpha} + \eta_{\epsilon\alpha} + \eta_{x\alpha})^4\}\right]^{1/4}.\end{aligned}$$

Note that $\eta_{x\epsilon\alpha} \le \eta_{x\alpha}\eta_{\epsilon\alpha}$ and

$$\begin{aligned}&E\{(\eta_\alpha \eta_{x\alpha}^2 + \eta_{x\epsilon\alpha})^4 (2\eta_\alpha \eta_{x\alpha} + \eta_{\epsilon\alpha} + \eta_{x\alpha})^4\} \\ \lesssim& E[(\eta_\alpha \eta_{x\alpha}^2 + \eta_{x\alpha}\eta_{\epsilon\alpha})^4 \{(2\eta_\alpha + 1)\eta_{x\alpha} + \eta_{\epsilon\alpha}\}^4] \\ \lesssim& E[(\eta_\alpha^4 \eta_{x\alpha}^8 + \eta_{x\alpha}^4 \eta_{\epsilon\alpha}^4)\{(2\eta_\alpha + 1)^4 \eta_{x\alpha}^4 + \eta_{\epsilon\alpha}^4\}] \\ =& \eta_\alpha^4 (2\eta_\alpha + 1)^4 E\eta_{x\alpha}^{12} + \eta_\alpha^4 E\eta_{x\alpha}^8 E\eta_{\epsilon\alpha}^4 + (2\eta_\alpha + 1)^4 E\eta_{\epsilon\alpha}^4 E\eta_{x\alpha}^8 + E\eta_{\epsilon\alpha}^8 E\eta_{x\alpha}^4.\end{aligned}$$

Similar to the proof of Theorem **??**, we have $E\eta_{\epsilon\alpha}^k = O(\|\boldsymbol{\alpha}\|^k)$ under Condition **??**. By Lemma S5, we have

$$E\eta_{x\alpha}^{12} = E\left[\{\lambda_{\max}(\boldsymbol{X}_\alpha^T \boldsymbol{X}_\alpha/n)\}^6\right] = O(1).$$

It follows that $\left[E\{(\eta_\alpha \eta_{x\alpha}^2 + \eta_{x\epsilon\alpha})^4 (2\eta_\alpha \eta_{x\alpha} + \eta_{\epsilon\alpha} + \eta_{x\alpha})^4\}\right]^{1/4} = O(\|\boldsymbol{\alpha}\|^2 + \|\boldsymbol{\alpha}\|)$. We let $\kappa_1 = \left\{E\|\nabla g(\boldsymbol{X}_\alpha, \boldsymbol{\epsilon}_\alpha)\|^4\right\}^{1/4}$, then we have

$$\kappa_1 \lesssim \frac{1}{\sqrt{n}_\alpha} (\boldsymbol{\ell}_a^T \boldsymbol{H} \boldsymbol{\ell}_a)^{-1} \boldsymbol{\ell}_{a,\max} (\|\boldsymbol{\alpha}\|^2 + \|\boldsymbol{\alpha}\|). \tag{24}$$

In addition, note that

$$\begin{aligned}\|\nabla^2 g(\boldsymbol{X}_\alpha, \boldsymbol{\epsilon}_\alpha)\| =& \sqrt{\lambda_{\max}(\{\nabla^2 g(\boldsymbol{X}_\alpha, \boldsymbol{\epsilon}_\alpha)\}^T \nabla^2 g(\boldsymbol{X}_\alpha, \boldsymbol{\epsilon}_\alpha))} \\ =& \max_\lambda |\lambda(\nabla^2 g(\boldsymbol{X}_\alpha, \boldsymbol{\epsilon}_\alpha))| \\ =& \sup_{\widetilde{\boldsymbol{U}} \in \mathcal{U}} |\widetilde{\boldsymbol{U}}^T \nabla^2 g(\boldsymbol{X}_\alpha, \boldsymbol{\epsilon}_\alpha) \widetilde{\boldsymbol{U}}|,\end{aligned}$$

where $\lambda(\cdot)$ denotes the eigenvalue of a matrix and $\lambda_{\max}(\cdot)$ denotes the largest eigenvalue. Then we have

$$\|\nabla^2 g(\boldsymbol{X}_\alpha, \boldsymbol{\epsilon}_\alpha)\| = \sup_{\widetilde{\boldsymbol{U}} \in \mathcal{U}} |D_{\widetilde{\boldsymbol{U}}}^2 g(\boldsymbol{X}_\alpha, \boldsymbol{\epsilon}_\alpha)|.$$

Since

$$D^2_{\widetilde{\boldsymbol{U}}} g(\boldsymbol{X}_\alpha, \boldsymbol{\epsilon}_\alpha) = 2(\boldsymbol{\ell}_a^T \boldsymbol{H}\boldsymbol{\ell}_a)^{-1} \sum_{k=1}^p [\boldsymbol{H}\boldsymbol{\ell}_a]_k \cdot n_\alpha^{-2} \cdot \left(\boldsymbol{X}_{\alpha,\cdot k}^T \boldsymbol{U}\boldsymbol{\alpha} + \boldsymbol{U}_{\cdot k}^T \boldsymbol{X}_\alpha \boldsymbol{\alpha} + \boldsymbol{U}_{\cdot k}^T \boldsymbol{\epsilon}_\alpha + \boldsymbol{X}_{\alpha,\cdot k}^T \boldsymbol{u}\right)^2$$
$$+2(\boldsymbol{\ell}_a^T \boldsymbol{H}\boldsymbol{\ell}_a)^{-1} \sum_{k=1}^p [\boldsymbol{H}\boldsymbol{\ell}_a]_k \widehat{a}_k \cdot 2n_\alpha^{-1} \cdot \left(\boldsymbol{U}_{\cdot k}^T \boldsymbol{U}\boldsymbol{\alpha} + \boldsymbol{U}_{\cdot k}^T \boldsymbol{u}\right),$$

we have

$$\begin{aligned}
|D^2_{\widetilde{\boldsymbol{U}}} g(\boldsymbol{X}_\alpha, \boldsymbol{\epsilon}_\alpha)| \lesssim & n_\alpha^{-1} \cdot (\boldsymbol{\ell}_a^T \boldsymbol{H}\boldsymbol{\ell}_a)^{-1} \boldsymbol{\ell}_{a,\max} \left(\boldsymbol{\alpha}^T \boldsymbol{U}^T \boldsymbol{X}_\alpha \boldsymbol{X}_\alpha^T \boldsymbol{U}\boldsymbol{\alpha}/n_\alpha + \boldsymbol{\alpha}^T \boldsymbol{X}_\alpha^T \boldsymbol{U}\boldsymbol{U}^T \boldsymbol{X}_\alpha \boldsymbol{\alpha}/n_\alpha\right. \\
& \left. + \boldsymbol{\epsilon}_\alpha^T \boldsymbol{U}\boldsymbol{U}^T \boldsymbol{\epsilon}_\alpha/n_\alpha + \boldsymbol{u}^T \boldsymbol{X}_\alpha \boldsymbol{X}_\alpha^T \boldsymbol{u}/n_\alpha\right) \\
& + n_\alpha^{-1} \cdot (\boldsymbol{\ell}_a^T \boldsymbol{H}\boldsymbol{\ell}_a)^{-1} \boldsymbol{\ell}_{a,\max} |\widehat{\boldsymbol{a}}^T (\boldsymbol{U}^T \boldsymbol{U}\boldsymbol{\alpha} + \boldsymbol{U}^T \boldsymbol{u})| \\
\leq & n_\alpha^{-1} \cdot (\boldsymbol{\ell}_a^T \boldsymbol{H}\boldsymbol{\ell}_a)^{-1} \boldsymbol{\ell}_{a,\max} \{2\eta_\alpha^2 \eta_{x\alpha}^2 \|\boldsymbol{U}\|^2 + \eta_{\epsilon\alpha}^2 \|\boldsymbol{U}\|^2 + \eta_{x\alpha}^2 \|\boldsymbol{u}\|^2 \\
& + (\eta_\alpha \eta_{x\alpha}^2 + \eta_{x\epsilon\alpha})(\eta_\alpha \|\boldsymbol{U}\|^2 + \|\boldsymbol{U}\|\|\boldsymbol{u}\|)\} \\
\leq & n_\alpha^{-1} \cdot (\boldsymbol{\ell}_a^T \boldsymbol{H}\boldsymbol{\ell}_a)^{-1} \boldsymbol{\ell}_{a,\max} \{2\eta_\alpha^2 \eta_{x\alpha}^2 + \eta_{\epsilon\alpha}^2 + \eta_{x\alpha}^2 + (\eta_\alpha \eta_{x\alpha}^2 + \eta_{x\epsilon\alpha})(\eta_\alpha + 1)\}.
\end{aligned}$$

Therefore, we have

$$\begin{aligned}
\left(E\|\nabla^2 g(\boldsymbol{X}_{\alpha_0}, \boldsymbol{\epsilon}_\alpha)\|^4\right)^{1/4} \lesssim & n_\alpha^{-1} \cdot (\boldsymbol{\ell}_a^T \boldsymbol{H}\boldsymbol{\ell}_a)^{-1} \boldsymbol{\ell}_{a,\max} \left[E\{2\eta_\alpha^2 \eta_{x\alpha}^2 + \eta_{\epsilon\alpha}^2 + \eta_{x\alpha}^2\right. \\
& \left. + (\eta_\alpha \eta_{x\alpha}^2 + \eta_{x\epsilon\alpha})(\eta_\alpha + 1)\}^4\right]^{1/4}.
\end{aligned}$$

Note that

$$\begin{aligned}
& E\{2\eta_\alpha^2 \eta_{x\alpha}^2 + \eta_{\epsilon\alpha}^2 + \eta_{x\alpha}^2 + (\eta_\alpha \eta_{x\alpha}^2 + \eta_{x\epsilon\alpha})(\eta_\alpha + 1)\}^4 \\
\lesssim & (2\eta_\alpha^2 + 1)^4 E\eta_{x\alpha}^8 + E\eta_{\epsilon\alpha}^8 + (\eta_\alpha + 1)^4 E\{\eta_\alpha \eta_{x\alpha}^2 + \eta_{x\alpha}\eta_{\epsilon\alpha}\}^4 \\
\lesssim & (2\eta_\alpha^2 + 1)^4 E\eta_{x\alpha}^8 + E\eta_{\epsilon\alpha}^8 + (\eta_\alpha + 1)^4 \{\eta_\alpha^4 E\eta_{x\alpha}^8 + E\eta_{x\alpha}^4 E\eta_{\epsilon\alpha}^4\}.
\end{aligned}$$

Recall that $\eta_\alpha = \|\boldsymbol{\alpha}\|$, $E\eta_{\epsilon\alpha}^k = O(\|\boldsymbol{\alpha}\|^k)$, and $E\eta_{x\alpha}^{12} = O(1)$. Thus, we have

$$\left[E\{2\eta_\alpha^2 \eta_{x\alpha}^2 + \eta_{\epsilon\alpha}^2 + \eta_{x\alpha}^2 + (\eta_\alpha \eta_{x\alpha}^2 + \eta_{x\epsilon\alpha})(\eta_\alpha + 1)\}^4\right]^{1/4} = O(\|\boldsymbol{\alpha}\|^2 + 1).$$

Let $\kappa_2 = \left(E\|\nabla^2 g(\boldsymbol{X}_{\alpha_0}, \boldsymbol{\epsilon}_\alpha)\|^4\right)^{1/4}$, then we have

$$\kappa_2 \lesssim n_\alpha^{-1} \cdot (\boldsymbol{\ell}_a^T \boldsymbol{H}\boldsymbol{\ell}_a)^{-1} \boldsymbol{\ell}_{a,\max} (\|\boldsymbol{\alpha}\|^2 + 1). \tag{25}$$

Let $Z$ be a random variable from $N(E\widetilde{\sigma}_\alpha^2, \zeta_\alpha^2)$ and $d_{TV}(\widetilde{\sigma}_\alpha^2, Z)$ be the total variation distance between the laws of $\widetilde{\sigma}_\alpha^2$ and $Z$. By [9, Theorem 2.2], we have

$$d_{TV}(\widetilde{\sigma}_\alpha^2, Z) \lesssim \frac{\|\boldsymbol{\Sigma}_\alpha\|^{3/2} \kappa_1 \kappa_2}{\zeta_\alpha^2(\boldsymbol{\ell}_a)}.$$

By Condition **??**, we have $\lambda_{\max}(\boldsymbol{\Sigma}_\alpha) = O(1)$. By inequalities in (22), (24), and (25), we have

$$\begin{aligned}
\frac{\kappa_1 \kappa_2}{\zeta_\alpha^2(\boldsymbol{\ell}_a)} \lesssim & n_\alpha^{-3/2} \cdot (\boldsymbol{\ell}_a^T \boldsymbol{H}\boldsymbol{\ell}_a)^{-2} \boldsymbol{\ell}_{a,\max}^2 (\|\boldsymbol{\alpha}\|^2 + 1) \cdot (\|\boldsymbol{\alpha}\|^2 + \|\boldsymbol{\alpha}\|) \cdot \frac{(\boldsymbol{\ell}_a^T \boldsymbol{H}\boldsymbol{\ell}_a)^2 \cdot n_\alpha}{\|\boldsymbol{\alpha}\|^4 \boldsymbol{\ell}_{a,\min}^2} \\
= & \frac{(\|\boldsymbol{\alpha}\|^2 + 1)(\|\boldsymbol{\alpha}\| + 1)}{n_\alpha^{1/2} \cdot \|\boldsymbol{\alpha}\|^3} \cdot \left(\frac{\boldsymbol{\ell}_{a,\max}}{\boldsymbol{\ell}_{a,\min}}\right)^2.
\end{aligned}$$

Let $\bar{\boldsymbol{\ell}}_{a,\max} = \max\{|\boldsymbol{\ell}_{a,i}| \text{ for } i = 1,\dots,p\}$ and $\bar{\boldsymbol{\ell}}_{a,\min} = \max\{|\boldsymbol{\ell}_{a,i}| \text{ for } i = 1,\dots,p\}$. By Condition **??**, there exist positive constants $c_1$ and $c_2$ such that $\bar{\boldsymbol{\ell}}_{a,\min} > c_1$ and $\bar{\boldsymbol{\ell}}_{a,\max} \le c_2$, which implies that $\boldsymbol{\ell}_{a,\max} \le c_2$. By Conditions **??** and **??**, we have $\kappa_1\kappa_2/\zeta_\alpha^2(\boldsymbol{\ell}_a) = o(1)$, which implies that

$$\frac{\widetilde{\sigma}_\alpha^2 - E\widetilde{\sigma}_\alpha^2}{\zeta_\alpha(\boldsymbol{\ell}_a)} \xrightarrow{d} N(0,1).$$

□

S6.3. *Proof of Theorem* **??**.

PROOF. **Step 1: To obtain (??)**
By (22) and Condition **??**, we have

$$\zeta_\alpha^2(\boldsymbol{\ell}_a) \gtrsim \frac{\|\boldsymbol{\alpha}\|^4 \boldsymbol{\ell}_{a,\min}^2}{n_\alpha(\boldsymbol{\ell}_a^T\boldsymbol{H}\boldsymbol{\ell}_a)^2} \gtrsim \frac{\|\boldsymbol{\alpha}\|^4}{n_\alpha(\boldsymbol{\ell}_a^T\boldsymbol{H}\boldsymbol{\ell}_a)^2}.$$

By Conditions **??** and **??**, we have

$$\left|\frac{\boldsymbol{\ell}_a^T\boldsymbol{H}\boldsymbol{\varepsilon}_a}{\boldsymbol{\ell}_a^T\boldsymbol{H}\boldsymbol{\ell}_a \cdot \zeta_\alpha(\boldsymbol{\ell}_a)}\right| \lesssim |\boldsymbol{\ell}_a^T\boldsymbol{H}\boldsymbol{\varepsilon}| \cdot \left(\frac{n_\alpha}{\|\boldsymbol{\alpha}\|^4}\right)^{1/2} = o(1),$$

which implies (**??**).

**Step 2: To obtain (??)**
Note that

$$\frac{\{(\widehat{\boldsymbol{\ell}}_a^T\boldsymbol{H}\widehat{\boldsymbol{\ell}}_a)^{-1}\widehat{\boldsymbol{\ell}}_a^T - (\boldsymbol{\ell}_a^T\boldsymbol{H}\boldsymbol{\ell}_a)^{-1}\boldsymbol{\ell}_a^T\}\boldsymbol{H}\boldsymbol{w}_a}{\zeta_\alpha(\boldsymbol{\ell}_a)}$$

$$= \left\{(\widehat{\boldsymbol{\ell}}_a^T\boldsymbol{H}\widehat{\boldsymbol{\ell}}_a/\boldsymbol{\ell}_a^T\boldsymbol{H}\boldsymbol{\ell}_a)^{-1} - 1\right\}\frac{(\widehat{\boldsymbol{\ell}}_a - \boldsymbol{\ell}_a)^T\boldsymbol{H}\boldsymbol{w}_a}{\boldsymbol{\ell}_a^T\boldsymbol{H}\boldsymbol{\ell}_a \cdot \zeta_\alpha(\boldsymbol{\ell}_a)} + \frac{(\widehat{\boldsymbol{\ell}}_a^T\boldsymbol{H}\widehat{\boldsymbol{\ell}}_a/\boldsymbol{\ell}_a^T\boldsymbol{H}\boldsymbol{\ell}_a)^{-1} - 1}{\zeta_\alpha(\boldsymbol{\ell}_a)}\frac{\boldsymbol{\ell}_a^T\boldsymbol{H}\boldsymbol{w}_a}{\boldsymbol{\ell}_a^T\boldsymbol{H}\boldsymbol{\ell}_a}$$

$$+ \frac{(\widehat{\boldsymbol{\ell}}_a - \boldsymbol{\ell}_a)^T\boldsymbol{H}\boldsymbol{w}_a}{\boldsymbol{\ell}_a^T\boldsymbol{H}\boldsymbol{\ell}_a \cdot \zeta_\alpha(\boldsymbol{\ell}_a)}.$$

**Step 2.1:**
By (**??**), we have

$$\frac{\boldsymbol{\ell}_a^T\boldsymbol{H}\boldsymbol{w}_a}{\boldsymbol{\ell}_a^T\boldsymbol{H}\boldsymbol{\ell}_a} = \sigma_\alpha^2 + \frac{\boldsymbol{\ell}_a^T\boldsymbol{H}\boldsymbol{\varepsilon}_a}{\boldsymbol{\ell}_a^T\boldsymbol{H}\boldsymbol{\ell}_a}.$$

By Condition **??**, we have

$$\boldsymbol{\ell}_a^T\boldsymbol{H}\boldsymbol{\ell}_a \gtrsim p. \tag{26}$$

By (26) and Condition **??**, we have $\sigma_\alpha^2 = O(1)$ and

$$\frac{\boldsymbol{\ell}_a^T\boldsymbol{H}\boldsymbol{\varepsilon}_a}{\boldsymbol{\ell}_a^T\boldsymbol{H}\boldsymbol{\ell}_a} = o(1),$$

which implies

$$\frac{\boldsymbol{\ell}_a^T\boldsymbol{H}\boldsymbol{w}_a}{\boldsymbol{\ell}_a^T\boldsymbol{H}\boldsymbol{\ell}_a} = O(1).$$

**Step 2.2:**
If $\boldsymbol{w}_a = \mathbf{0}$, then we have

$$\frac{(\widehat{\boldsymbol{\ell}}_a - \boldsymbol{\ell}_a)^T \boldsymbol{H} \boldsymbol{w}_a}{\boldsymbol{\ell}_a^T \boldsymbol{H} \boldsymbol{\ell}_a \cdot \zeta_\alpha(\boldsymbol{\ell}_a)} = 0.$$

If $\boldsymbol{w}_a \neq \mathbf{0}$, then we have

$$\frac{(\widehat{\boldsymbol{\ell}}_a - \boldsymbol{\ell}_a)^T \boldsymbol{H} \boldsymbol{w}_a}{\boldsymbol{\ell}_a^T \boldsymbol{H} \boldsymbol{\ell}_a \cdot \zeta_\alpha(\boldsymbol{\ell}_a)} = \frac{\|\boldsymbol{H}\boldsymbol{w}_a\|_2}{n_{r\alpha}^{1/2} \boldsymbol{\ell}_a^T \boldsymbol{H} \boldsymbol{\ell}_a \cdot \zeta_\alpha(\boldsymbol{\ell}_a)} \cdot \frac{n_{r\alpha}^{1/2}(\widehat{\boldsymbol{\ell}}_a - E\widehat{\boldsymbol{\ell}}_a)^T \boldsymbol{H} \boldsymbol{w}_a}{\|\boldsymbol{H}\boldsymbol{w}_a\|_2} + \frac{(E\widehat{\boldsymbol{\ell}}_a - \boldsymbol{\ell}_a)^T \boldsymbol{H} \boldsymbol{w}_a}{\boldsymbol{\ell}_a^T \boldsymbol{H} \boldsymbol{\ell}_a \cdot \zeta_\alpha(\boldsymbol{\ell}_a)}. \tag{27}$$

By Theorem **??**,

$$\frac{n_{r\alpha}^{1/2}(\widehat{\boldsymbol{\ell}}_a - E\widehat{\boldsymbol{\ell}}_a)^T \boldsymbol{H} \boldsymbol{w}_a}{\|\boldsymbol{H}\boldsymbol{w}_a\|_2}$$

converges in distribution to a normal distribution as $p \to \infty$. By Lemma S11 and $\lambda_{\max}(\boldsymbol{H}) = 1$, we have

$$\|\boldsymbol{H}\boldsymbol{w}_a\|_2 \lesssim \left( \|\boldsymbol{\alpha}\|_4^4 + \frac{p}{n_\alpha^2} \|\boldsymbol{\alpha}\|_2^4 \right)^{1/2}.$$

Combining it with (22), we have

$$\begin{aligned} \frac{\|\boldsymbol{H}\boldsymbol{w}_a\|_2}{n_{r\alpha}^{1/2} \boldsymbol{\ell}_a^T \boldsymbol{H} \boldsymbol{\ell}_a \cdot \zeta_\alpha(\boldsymbol{\ell}_a)} &\lesssim \left\{ \frac{\|\boldsymbol{\alpha}\|_4^4}{n_{r\alpha}(\boldsymbol{\ell}_a^T \boldsymbol{H} \boldsymbol{\ell}_a)^2 \cdot \zeta_\alpha^2(\boldsymbol{\ell}_a)} + \frac{p\|\boldsymbol{\alpha}\|_2^4}{n_{r\alpha} n_\alpha^2 (\boldsymbol{\ell}_a^T \boldsymbol{H} \boldsymbol{\ell}_a)^2 \cdot \zeta_\alpha^2(\boldsymbol{\ell}_a)} \right\}^{1/2} \\ &\lesssim \left( \frac{n_\alpha \|\boldsymbol{\alpha}\|_4^4}{n_{r\alpha}\|\boldsymbol{\alpha}\|^4} + \frac{p\|\boldsymbol{\alpha}\|_2^4}{n_{r\alpha} n_\alpha \|\boldsymbol{\alpha}\|^4} \right)^{1/2} \\ &\lesssim \left( \frac{n_\alpha \|\boldsymbol{\alpha}\|_4^4}{n_{r\alpha}\|\boldsymbol{\alpha}\|^4} + \frac{p}{n_{r\alpha} n_\alpha} \right)^{1/2}. \end{aligned} \tag{28}$$

By Condition **??**, we have

$$\frac{p}{n_{r\alpha} n_\alpha} \to 0$$

as $n_{r\alpha} \to \infty$. By Condition **??**, we have

$$\frac{n_\alpha \|\boldsymbol{\alpha}\|_4^4}{n_{r\alpha}\|\boldsymbol{\alpha}\|_2^4} \to 0.$$

Thus, we have

$$\frac{\|\boldsymbol{H}\boldsymbol{w}_a\|_2}{n_{r\alpha}^{1/2} \boldsymbol{\ell}_a^T \boldsymbol{H} \boldsymbol{\ell}_a \cdot \zeta_\alpha(\boldsymbol{\ell}_a)} = o(1).$$

By Theorem **??**, Lemma S11, (22), and $\|\boldsymbol{H}\boldsymbol{w}_a\|_1 \lesssim \|\boldsymbol{w}_a\|_1$, we have

$$\begin{aligned} \frac{(E\widehat{\boldsymbol{\ell}}_a - \boldsymbol{\ell}_a)^T \boldsymbol{H} \boldsymbol{w}_a}{\boldsymbol{\ell}_a^T \boldsymbol{H} \boldsymbol{\ell}_a \cdot \zeta_\alpha(\boldsymbol{\ell}_a)} &\lesssim \frac{\|\boldsymbol{H}\boldsymbol{w}_a\|_1}{n_{r\alpha} \boldsymbol{\ell}_a^T \boldsymbol{H} \boldsymbol{\ell}_a \cdot \zeta_\alpha(\boldsymbol{\ell}_a)} \lesssim \frac{\|\boldsymbol{\alpha}\|_2^2}{n_{r\alpha} \boldsymbol{\ell}_a^T \boldsymbol{H} \boldsymbol{\ell}_a \cdot \zeta_\alpha(\boldsymbol{\ell}_a)} + \frac{p\|\boldsymbol{\alpha}\|_2^2}{n_{r\alpha} n_\alpha \boldsymbol{\ell}_a^T \boldsymbol{H} \boldsymbol{\ell}_a \cdot \zeta_\alpha(\boldsymbol{\ell}_a)} \\ &\lesssim \frac{n_\alpha^{1/2} \|\boldsymbol{\alpha}\|_2^2}{n_{r\alpha}\|\boldsymbol{\alpha}\|_2^2} + \frac{p\|\boldsymbol{\alpha}\|_2^2}{n_{r\alpha}\|\boldsymbol{\alpha}\|_2^2 n_\alpha^{1/2}} \\ &\lesssim \frac{n_\alpha^{1/2}}{n_{r\alpha}} + \frac{p}{n_{r\alpha} n_\alpha^{1/2}}. \end{aligned}$$

Under Condition **??**, we have

$$\frac{(E\widehat{\boldsymbol{\ell}}_a - \boldsymbol{\ell}_a)^T \boldsymbol{H} \boldsymbol{w}_a}{\boldsymbol{\ell}_a^T \boldsymbol{H} \boldsymbol{\ell}_a \cdot \zeta_\alpha(\boldsymbol{\ell}_a)} \to 0,$$

as $p \to \infty$. It follows that

$$\frac{(\widehat{\boldsymbol{\ell}}_a - \boldsymbol{\ell}_a)^T \boldsymbol{H} \boldsymbol{w}_a}{\boldsymbol{\ell}_a^T \boldsymbol{H} \boldsymbol{\ell}_a \cdot \zeta_\alpha(\boldsymbol{\ell}_a)} \xrightarrow{p} 0,$$

as $p \to \infty$.

**Step 2.3:**
Note that

$$\begin{aligned} &\frac{(\widehat{\boldsymbol{\ell}}_a^T \boldsymbol{H} \widehat{\boldsymbol{\ell}}_a / \boldsymbol{\ell}_a^T \boldsymbol{H} \boldsymbol{\ell}_a)^{-1} - 1}{\zeta_\alpha(\boldsymbol{\ell}_a)} \\ =& \frac{1}{\zeta_\alpha(\boldsymbol{\ell}_a)} \cdot \frac{(\boldsymbol{\ell}_a^T \boldsymbol{H} \boldsymbol{\ell}_a - \widehat{\boldsymbol{\ell}}_a^T \boldsymbol{H} \widehat{\boldsymbol{\ell}}_a)/(p/n_{r\alpha})}{(\widehat{\boldsymbol{\ell}}_a^T \boldsymbol{H} \widehat{\boldsymbol{\ell}}_a - \boldsymbol{\ell}_a^T \boldsymbol{H} \boldsymbol{\ell}_a)/(p/n_{r\alpha}) + \boldsymbol{\ell}_a^T \boldsymbol{H} \boldsymbol{\ell}_a/(p/n_{r\alpha})}, \end{aligned}$$

$$\frac{\widehat{\boldsymbol{\ell}}_a^T \boldsymbol{H} \widehat{\boldsymbol{\ell}}_a - \boldsymbol{\ell}_a^T \boldsymbol{H} \boldsymbol{\ell}_a}{p/n_{r\alpha}} = \frac{\widehat{\boldsymbol{\ell}}_a^T \widehat{\boldsymbol{\ell}}_a - \boldsymbol{\ell}_a^T \boldsymbol{\ell}_a}{p/n_{r\alpha}} + \frac{(\widehat{\boldsymbol{\ell}}_a^T \mathbf{1}_p/\sqrt{p})^2 - (\boldsymbol{\ell}_a^T \mathbf{1}_p/\sqrt{p})^2}{p/n_{r\alpha}},$$

$$\begin{aligned} &(\widehat{\boldsymbol{\ell}}_a^T \mathbf{1}_p/\sqrt{p})^2 - (\boldsymbol{\ell}_a^T \mathbf{1}_p/\sqrt{p})^2 \\ =&(\widehat{\boldsymbol{\ell}}_a^T \mathbf{1}_p/\sqrt{p} - \boldsymbol{\ell}_a^T \mathbf{1}_p/\sqrt{p})(\widehat{\boldsymbol{\ell}}_a^T \mathbf{1}_p/\sqrt{p} - \boldsymbol{\ell}_a^T \mathbf{1}_p/\sqrt{p} + 2\boldsymbol{\ell}_a^T \mathbf{1}_p/\sqrt{p}) \\ =&(\widehat{\boldsymbol{\ell}}_a^T \mathbf{1}_p/\sqrt{p} - \boldsymbol{\ell}_a^T \mathbf{1}_p/\sqrt{p})^2 + 2(\widehat{\boldsymbol{\ell}}_a^T \mathbf{1}_p/\sqrt{p} - \boldsymbol{\ell}_a^T \mathbf{1}_p/\sqrt{p})(\boldsymbol{\ell}_a^T \mathbf{1}_p/\sqrt{p}), \end{aligned}$$

and

$$(\widehat{\boldsymbol{\ell}}_a^T \mathbf{1}_p/\sqrt{p} - \boldsymbol{\ell}_a^T \mathbf{1}_p/\sqrt{p})^2 \lesssim (\widehat{\boldsymbol{\ell}}_a^T \mathbf{1}_p - E\widehat{\boldsymbol{\ell}}_a^T \mathbf{1}_p)^2/p + (E\widehat{\boldsymbol{\ell}}_a^T \mathbf{1}_p - \boldsymbol{\ell}_a^T \mathbf{1}_p)^2/p.$$

By Lemma S16, we have

$$\frac{(\widehat{\boldsymbol{\ell}}_a^T \mathbf{1}_p - E\widehat{\boldsymbol{\ell}}_a^T \mathbf{1}_p)^2/p}{p/n_{r\alpha}} \xrightarrow{p} 0,$$

and

$$\frac{(E\widehat{\boldsymbol{\ell}}_a^T \mathbf{1}_p - \boldsymbol{\ell}_a^T \mathbf{1}_p)^2/p}{p/n_{r\alpha}} \to 0.$$

By Condition **??**, there exists a positive constant $c$ such that $\bar{\boldsymbol{\ell}}_{a,\max} \leq c$, which implies that $\boldsymbol{\ell}_{a,\max} \leq c$. Together with Lemma S16, we have

$$\left| \frac{(\widehat{\boldsymbol{\ell}}_a^T \mathbf{1}_p/\sqrt{p} - \boldsymbol{\ell}_a^T \mathbf{1}_p/\sqrt{p})(\boldsymbol{\ell}_a^T \mathbf{1}_p/\sqrt{p})}{p/n_{r\alpha}} \right| = O_p(\sqrt{n_{r\alpha}/p} + 1).$$

By Lemma **??**, we have

$$\frac{\widehat{\boldsymbol{\ell}}_a^T \widehat{\boldsymbol{\ell}}_a - \boldsymbol{\ell}_a^T \boldsymbol{\ell}_a}{p/n_{r\alpha}} = O_p(\sqrt{n_{r\alpha}/p} + 1).$$

By (26), we have $\boldsymbol{\ell}_a^T \boldsymbol{H}\boldsymbol{\ell}_a/(p/n_{r\alpha}) \gtrsim n_{r\alpha}$. Note that

$$\zeta_\alpha(\boldsymbol{\ell}_a)\cdot\sqrt{n_{r\alpha}p} \gtrsim \frac{\|\boldsymbol{\alpha}\|^2\sqrt{n_{r\alpha}p}}{\sqrt{n_\alpha}\cdot\boldsymbol{\ell}_a^T\boldsymbol{H}\boldsymbol{\ell}_a} \gtrsim \frac{\|\boldsymbol{\alpha}\|^2\sqrt{n_{r\alpha}}}{\sqrt{n_\alpha p}} \gtrsim \sqrt{n_{r\alpha}} \to \infty.$$

By (22), Condition **??** and Condition **??**, we also have

$$\zeta_\alpha(\boldsymbol{\ell}_a)\cdot n_{r\alpha} \gtrsim \frac{\|\boldsymbol{\alpha}\|^2 n_{r\alpha}}{\sqrt{n_\alpha}\cdot\boldsymbol{\ell}_a^T\boldsymbol{H}\boldsymbol{\ell}_a} \gtrsim \frac{\|\boldsymbol{\alpha}\|^2 n_{r\alpha}}{\sqrt{n_\alpha p}} \to \infty,$$

where the last convergence follows from Condition **??**. Thus, we have

$$\frac{(\widehat{\boldsymbol{\ell}}_a^T\boldsymbol{H}\widehat{\boldsymbol{\ell}}_a/\boldsymbol{\ell}_a^T\boldsymbol{H}\boldsymbol{\ell}_a)^{-1}-1}{\zeta_\alpha(\boldsymbol{\ell}_a)} \xrightarrow{p} 0.$$

Similarly, we have

$$(\widehat{\boldsymbol{\ell}}_a^T\boldsymbol{H}\widehat{\boldsymbol{\ell}}_a/\boldsymbol{\ell}_a^T\boldsymbol{H}\boldsymbol{\ell}_a)^{-1}-1 = \frac{(\boldsymbol{\ell}_a^T\boldsymbol{H}\boldsymbol{\ell}_a-\widehat{\boldsymbol{\ell}}_a^T\boldsymbol{H}\widehat{\boldsymbol{\ell}}_a)/(p/n_{r\alpha})}{(\widehat{\boldsymbol{\ell}}_a^T\boldsymbol{H}\widehat{\boldsymbol{\ell}}_a-\boldsymbol{\ell}_a^T\boldsymbol{H}\boldsymbol{\ell}_a)/(p/n_{r\alpha})+\boldsymbol{\ell}_a^T\boldsymbol{H}\boldsymbol{\ell}_a/(p/n_{r\alpha})} \xrightarrow{p} 0. \tag{29}$$

**Step 3: To obtain (??)**
**Step 3.1:**
Let

$$V(\widehat{\boldsymbol{\ell}}_a) = \frac{(\widehat{\boldsymbol{\ell}}_a^T\boldsymbol{H}\widehat{\boldsymbol{\ell}}_a)^{-1}\widehat{\boldsymbol{\ell}}_a^T\boldsymbol{H}(\widehat{\boldsymbol{w}}_a-\boldsymbol{w}_a)}{\zeta_\alpha(\widehat{\boldsymbol{\ell}}_a)}.$$

Since

$$|\ell_{a,j}| = \left|\sum_{i\in\mathcal{N}(k)}\boldsymbol{\Sigma}_{\alpha,ji}^2\right| \le \sum_{i\in\mathcal{N}(k)}|\boldsymbol{\Sigma}_{\alpha,ji}|^2,$$

by Condition **??**, we have

$$\bar{\boldsymbol{\ell}}_{a,\max} = O(1), \tag{30}$$

which implies that

$$\|\boldsymbol{H}\boldsymbol{\ell}_a\|_\infty = \boldsymbol{\ell}_{a,\max} = O(1). \tag{31}$$

By Condition **??**, we have $\boldsymbol{\ell}_{a,\min} > c$ for some constant $c > 0$. Note that

$$\widehat{\boldsymbol{\ell}}_{a,\max}(n_{r\alpha}) = \|\boldsymbol{H}\widehat{\boldsymbol{\ell}}_a\|_\infty \le \|\boldsymbol{H}\boldsymbol{\ell}_a\|_\infty + \|\boldsymbol{H}\widehat{\boldsymbol{\ell}}_a-\boldsymbol{H}\boldsymbol{\ell}_a\|_\infty,$$

$$\widehat{\boldsymbol{\ell}}_{a,\min}(n_{r\alpha}) \ge \boldsymbol{\ell}_{a,\min} - \|\boldsymbol{H}\widehat{\boldsymbol{\ell}}_a-\boldsymbol{H}\boldsymbol{\ell}_a\|_\infty,$$

and

$$\|\boldsymbol{H}\widehat{\boldsymbol{\ell}}_a-\boldsymbol{H}\boldsymbol{\ell}_a\|_\infty \le \max_{1\le i\le p}|\widehat{\ell}_{a,i}-\ell_{a,i}| + (\widehat{\boldsymbol{\ell}}_a^T\mathbf{1}_p-\boldsymbol{\ell}_a^T\mathbf{1}_p)/p.$$

By Lemmas S7 and S16, we have

$$\max_{1\le i\le p}|\widehat{\ell}_{a,i}-\ell_{a,i}| \xrightarrow{p} 0 \quad\text{and}\quad (\widehat{\boldsymbol{\ell}}_a^T\mathbf{1}_p-\boldsymbol{\ell}_a^T\mathbf{1}_p)/p \xrightarrow{p} 0,$$

as $n_{r\alpha}$ and $p\to\infty$, which implies

$$\|\boldsymbol{H}\widehat{\boldsymbol{\ell}}_a-\boldsymbol{H}\boldsymbol{\ell}_a\|_\infty \xrightarrow{p} 0 \tag{32}$$

and there are positive constants $c_2$ and $c_3$ such that

$$\lim_{n_{r\alpha}\to\infty} P(\widehat{\boldsymbol{\ell}}_{a,\max}(n_{r\alpha}) < c_2) = 1 \tag{33}$$

and

$$\lim_{n_{r\alpha}\to\infty} P(\widehat{\boldsymbol{\ell}}_{a,\min}(n_{r\alpha}) > c_3) = 1. \tag{34}$$

Let $\mathcal{C}(c_2, c_3) = \{\widehat{\boldsymbol{\ell}}_a(n_{r\alpha}) : \widehat{\boldsymbol{\ell}}_{a,\max}(n_{r\alpha}) < c_2, \widehat{\boldsymbol{\ell}}_{a,\min}(n_{r\alpha}) > c_3\}$. For each $\widehat{\boldsymbol{\ell}}_a(n_{r\alpha}) \in \mathcal{C}(c_2, c_3)$, we have $V(\widehat{\boldsymbol{\ell}}_a) \mid \widehat{\boldsymbol{\ell}}_a \xrightarrow{d} N(0,1)$ by Theorem **??** and Remark **??**. Let $Z$ be a normally distributed random variable. Note that

$$\begin{aligned}
&\left| E_{\widehat{\boldsymbol{\ell}}_a}\{P(V(\widehat{\boldsymbol{\ell}}_a) \le t \mid \widehat{\boldsymbol{\ell}}_a)\} - P(Z \le t) \right| \\
=&\left| \int_{\widehat{\boldsymbol{\ell}}_a \in \mathcal{C}(c)} P(V(\widehat{\boldsymbol{\ell}}_a) \le t \mid \widehat{\boldsymbol{\ell}}_a) p(\widehat{\boldsymbol{\ell}}_a) d\widehat{\boldsymbol{\ell}}_a - P(Z \le t) \right. \\
&\left. + \int_{\widehat{\boldsymbol{\ell}}_a \in \mathcal{C}(c)^c} P(V(\widehat{\boldsymbol{\ell}}_a) \le t \mid \widehat{\boldsymbol{\ell}}_a) p(\widehat{\boldsymbol{\ell}}_a) d\widehat{\boldsymbol{\ell}}_a \right| \\
=&\left| \int_{\widehat{\boldsymbol{\ell}}_a \in \mathcal{C}(c)} \{P(Z \le t) + o(1)\} p(\widehat{\boldsymbol{\ell}}_a) d\widehat{\boldsymbol{\ell}}_a - P(Z \le t) \right. \\
&\left. + \int_{\widehat{\boldsymbol{\ell}}_a \in \mathcal{C}(c)^c} P(V(\widehat{\boldsymbol{\ell}}_a) \le t \mid \widehat{\boldsymbol{\ell}}_a) p(\widehat{\boldsymbol{\ell}}_a) d\widehat{\boldsymbol{\ell}}_a \right| \\
\le& o(1) + P(\mathcal{C}(c_2, c_3)^c),
\end{aligned}$$

where $p(\widehat{\boldsymbol{\ell}}_a)$ represents the density function of $\widehat{\boldsymbol{\ell}}_a$. By (33) and (34), we have

$$P(\mathcal{C}(c_2, c_3)^c) \to 0.$$

It follows that

$$P(V(\widehat{\boldsymbol{\ell}}_a) \le t) - P(Z \le t) = E_{\widehat{\boldsymbol{\ell}}_a}\{P(V(\widehat{\boldsymbol{\ell}}_a) \le t \mid \widehat{\boldsymbol{\ell}}_a)\} - P(Z \le t) \to 0.$$

This implies that $V(\widehat{\boldsymbol{\ell}}_a) \xrightarrow{d} N(0,1)$ as $n_{r\alpha}$ and $p \to \infty$.

**Step 3.2:**
Note that

$$\frac{(\widehat{\boldsymbol{\ell}}_a^T \boldsymbol{H} \widehat{\boldsymbol{\ell}}_a)^{-1} \widehat{\boldsymbol{\ell}}_a^T \boldsymbol{H} (\widehat{\boldsymbol{w}}_a - \boldsymbol{w}_a)}{\zeta_\alpha(\boldsymbol{\ell}_a)} = V(\widehat{\boldsymbol{\ell}}_a) \cdot \frac{\zeta_\alpha(\widehat{\boldsymbol{\ell}}_a)}{\zeta_\alpha(\boldsymbol{\ell}_a)} \tag{35}$$

and

$$\frac{\zeta_\alpha(\widehat{\boldsymbol{\ell}}_a)}{\zeta_\alpha(\boldsymbol{\ell}_a)} = \left\{ \frac{f(\widehat{\boldsymbol{\ell}}_a)}{f(\boldsymbol{\ell}_a)} \right\}^{1/2} \cdot \frac{\boldsymbol{\ell}_a^T \boldsymbol{H} \boldsymbol{\ell}_a}{\widehat{\boldsymbol{\ell}}_a^T \boldsymbol{H} \widehat{\boldsymbol{\ell}}_a}, \tag{36}$$

where

$$\begin{aligned}
f(\boldsymbol{\ell}_a) =& 2\sigma_{\epsilon_\alpha}^2 \cdot \big\{ (n_\alpha + 2)(n_\alpha + 3) \boldsymbol{\alpha}^T \boldsymbol{\Sigma}_\alpha \boldsymbol{D}_\alpha \boldsymbol{\Sigma}_\alpha \boldsymbol{D}_\alpha \boldsymbol{\Sigma}_\alpha \boldsymbol{\alpha} \\
&+ (n_\alpha + 2) \operatorname{tr}(\boldsymbol{\Sigma}_\alpha \boldsymbol{D}_\alpha \boldsymbol{\Sigma}_\alpha \boldsymbol{D}_\alpha) \boldsymbol{\alpha}^T \boldsymbol{\Sigma}_\alpha \boldsymbol{\alpha} \big\} + \sigma_{\epsilon_\alpha}^4 \cdot (n_\alpha + 2) \cdot \operatorname{tr}(\boldsymbol{\Sigma}_\alpha \boldsymbol{D}_\alpha \boldsymbol{\Sigma}_\alpha \boldsymbol{D}_\alpha) \\
&+ (2n_\alpha^2 + 5n_\alpha + 3)(\boldsymbol{\alpha}^T \boldsymbol{\Sigma}_\alpha \boldsymbol{D}_\alpha \boldsymbol{\Sigma}_\alpha \boldsymbol{\alpha})^2 + (n_\alpha + 2)(\boldsymbol{\alpha}^T \boldsymbol{\Sigma}_\alpha \boldsymbol{\alpha})^2 \operatorname{tr}(\boldsymbol{\Sigma}_\alpha \boldsymbol{D}_\alpha \boldsymbol{\Sigma}_\alpha \boldsymbol{D}_\alpha) \\
&+ 2(n_\alpha + 2)(n_\alpha + 3) \boldsymbol{\alpha}^T \boldsymbol{\Sigma}_\alpha \boldsymbol{\alpha} \cdot \boldsymbol{\alpha}^T \boldsymbol{\Sigma}_\alpha \boldsymbol{D}_\alpha \boldsymbol{\Sigma}_\alpha \boldsymbol{D}_\alpha \boldsymbol{\Sigma}_\alpha \boldsymbol{\alpha}
\end{aligned}$$

by (23).

Note that

$$f(\widehat{\boldsymbol{\ell}}_a)/f(\boldsymbol{\ell}_a) - 1 = \frac{f(\widehat{\boldsymbol{\ell}}_a) - f(\boldsymbol{\ell}_a)}{f(\boldsymbol{\ell}_a)}. \tag{37}$$

By Condition **??**, we have

$$\begin{aligned}
&|f(\widehat{\boldsymbol{\ell}}_a) - f(\boldsymbol{\ell}_a)| \\
\lesssim & n_\alpha \|\boldsymbol{\alpha}\|^4 |\mathrm{tr}(\boldsymbol{\Sigma}_\alpha \boldsymbol{D}_\alpha \boldsymbol{\Sigma}_\alpha \boldsymbol{D}_\alpha) - \mathrm{tr}(\boldsymbol{\Sigma}_\alpha \widehat{\boldsymbol{D}}_\alpha \boldsymbol{\Sigma}_\alpha \widehat{\boldsymbol{D}}_\alpha)| \\
& + n_\alpha^2 \|\boldsymbol{\alpha}\|^4 |\boldsymbol{\alpha}^T \boldsymbol{\Sigma}_\alpha \boldsymbol{D}_\alpha \boldsymbol{\Sigma}_\alpha \boldsymbol{D}_\alpha \boldsymbol{\Sigma}_\alpha \boldsymbol{\alpha} / \|\boldsymbol{\alpha}\|^2 - \boldsymbol{\alpha}^T \boldsymbol{\Sigma}_\alpha \widehat{\boldsymbol{D}}_\alpha \boldsymbol{\Sigma}_\alpha \widehat{\boldsymbol{D}}_\alpha \boldsymbol{\Sigma}_\alpha \boldsymbol{\alpha} / \|\boldsymbol{\alpha}\|^2| \\
& + n_\alpha^2 \|\boldsymbol{\alpha}\|^4 |(\boldsymbol{\alpha}^T \boldsymbol{\Sigma}_\alpha \boldsymbol{D}_\alpha \boldsymbol{\Sigma}_\alpha \boldsymbol{\alpha})^2 / \|\boldsymbol{\alpha}\|^4 - (\boldsymbol{\alpha}^T \boldsymbol{\Sigma}_\alpha \widehat{\boldsymbol{D}}_\alpha \boldsymbol{\Sigma}_\alpha \boldsymbol{\alpha})^2 / \|\boldsymbol{\alpha}\|^4|,
\end{aligned}$$

where $\widehat{\boldsymbol{D}}_\alpha = \mathrm{diag}([\boldsymbol{H}\widehat{\boldsymbol{\ell}}_a]_1, \ldots, [\boldsymbol{H}\widehat{\boldsymbol{\ell}}_a]_p)$.

By inequality (22), under Conditions **??** and **??**, we have

$$f(\boldsymbol{\ell}_a) \gtrsim \|\boldsymbol{\alpha}\|^4 \boldsymbol{\ell}_{a,\min}^2 (n_\alpha p + n_\alpha^2) \gtrsim \|\boldsymbol{\alpha}\|^4 (n_\alpha p + n_\alpha^2).$$

Note that

$$\begin{aligned}
&\frac{1}{p} |\mathrm{tr}(\boldsymbol{\Sigma}_\alpha \boldsymbol{D}_\alpha \boldsymbol{\Sigma}_\alpha \boldsymbol{D}_\alpha) - \mathrm{tr}(\boldsymbol{\Sigma}_\alpha \widehat{\boldsymbol{D}}_\alpha \boldsymbol{\Sigma}_\alpha \widehat{\boldsymbol{D}}_\alpha)| \\
\leq & \frac{1}{p} \Big[ |\mathrm{tr}\{\boldsymbol{\Sigma}_\alpha \boldsymbol{D}_\alpha \boldsymbol{\Sigma}_\alpha (\boldsymbol{D}_\alpha - \widehat{\boldsymbol{D}}_\alpha)\}| + |\mathrm{tr}\{\boldsymbol{\Sigma}_\alpha (\boldsymbol{D}_\alpha - \widehat{\boldsymbol{D}}_\alpha) \boldsymbol{\Sigma}_\alpha (\boldsymbol{D}_\alpha - \widehat{\boldsymbol{D}}_\alpha)\}| \\
& + \mathrm{tr}\{\boldsymbol{\Sigma}_\alpha (\boldsymbol{D}_\alpha - \widehat{\boldsymbol{D}}_\alpha) \boldsymbol{\Sigma}_\alpha \boldsymbol{D}_\alpha\} \Big]
\end{aligned}$$

and

$$\begin{aligned}
|\mathrm{tr}\{\boldsymbol{\Sigma}_\alpha \boldsymbol{D}_\alpha \boldsymbol{\Sigma}_\alpha (\boldsymbol{D}_\alpha - \widehat{\boldsymbol{D}}_\alpha)\}| &\leq p \|\boldsymbol{D}_\alpha - \widehat{\boldsymbol{D}}_\alpha\|_2 \|\boldsymbol{\Sigma}_\alpha \boldsymbol{D}_\alpha \boldsymbol{\Sigma}_\alpha\|_2 \\
&\leq p \|\boldsymbol{D}_\alpha - \widehat{\boldsymbol{D}}_\alpha\|_2 \|\boldsymbol{\Sigma}_\alpha\|_2^2 \|\boldsymbol{D}_\alpha\|_2.
\end{aligned}$$

By Condition **??**, (31), and (32), we have

$$\frac{1}{p} |\mathrm{tr}\{\boldsymbol{\Sigma}_\alpha \boldsymbol{D}_\alpha \boldsymbol{\Sigma}_\alpha (\boldsymbol{D}_\alpha - \widehat{\boldsymbol{D}}_\alpha)\}| \xrightarrow{p} 0,$$

Similarly, we have

$$\frac{1}{p} |\mathrm{tr}\{\boldsymbol{\Sigma}_\alpha (\boldsymbol{D}_\alpha - \widehat{\boldsymbol{D}}_\alpha) \boldsymbol{\Sigma}_\alpha (\boldsymbol{D}_\alpha - \widehat{\boldsymbol{D}}_\alpha)\}| \xrightarrow{p} 0$$

and

$$\frac{1}{p} \mathrm{tr}\{\boldsymbol{\Sigma}_\alpha (\boldsymbol{D}_\alpha - \widehat{\boldsymbol{D}}_\alpha) \boldsymbol{\Sigma}_\alpha \boldsymbol{D}_\alpha\} \xrightarrow{p} 0,$$

which implies

$$\frac{1}{p} |\mathrm{tr}(\boldsymbol{\Sigma}_\alpha \boldsymbol{D}_\alpha \boldsymbol{\Sigma}_\alpha \boldsymbol{D}_\alpha) - \mathrm{tr}(\boldsymbol{\Sigma}_\alpha \widehat{\boldsymbol{D}}_\alpha \boldsymbol{\Sigma}_\alpha \widehat{\boldsymbol{D}}_\alpha)| \xrightarrow{p} 0.$$

By (31) and (32), we have

$$\begin{aligned}
&\frac{1}{\|\boldsymbol{\alpha}\|^2} |\boldsymbol{\alpha}^T \boldsymbol{\Sigma}_\alpha \boldsymbol{D}_\alpha \boldsymbol{\Sigma}_\alpha \boldsymbol{D}_\alpha \boldsymbol{\Sigma}_\alpha \boldsymbol{\alpha} - \boldsymbol{\alpha}^T \boldsymbol{\Sigma}_\alpha \widehat{\boldsymbol{D}}_\alpha \boldsymbol{\Sigma}_\alpha \widehat{\boldsymbol{D}}_\alpha \boldsymbol{\Sigma}_\alpha \boldsymbol{\alpha}| \\
\leq & \frac{1}{\|\boldsymbol{\alpha}\|^2} \{ |\boldsymbol{\alpha}^T \boldsymbol{\Sigma}_\alpha (\boldsymbol{D}_\alpha - \widehat{\boldsymbol{D}}_\alpha) \boldsymbol{\Sigma}_\alpha \boldsymbol{D}_\alpha \boldsymbol{\Sigma}_\alpha \boldsymbol{\alpha}| + |\boldsymbol{\alpha}^T \boldsymbol{\Sigma}_\alpha \widehat{\boldsymbol{D}}_\alpha \boldsymbol{\Sigma}_\alpha (\boldsymbol{D}_\alpha - \widehat{\boldsymbol{D}}_\alpha) \boldsymbol{\Sigma}_\alpha \boldsymbol{\alpha}| \} \xrightarrow{p} 0.
\end{aligned}$$

Similarly, we have

$$\begin{aligned}&\frac{1}{\|\boldsymbol{\alpha}\|^4}|(\boldsymbol{\alpha}^T\boldsymbol{\Sigma}_\alpha\boldsymbol{D}_\alpha\boldsymbol{\Sigma}_\alpha\boldsymbol{\alpha})^2-(\boldsymbol{\alpha}^T\boldsymbol{\Sigma}_\alpha\widehat{\boldsymbol{D}}_\alpha\boldsymbol{\Sigma}_\alpha\boldsymbol{\alpha})^2|\\ \le&\frac{1}{\|\boldsymbol{\alpha}\|^4}|\boldsymbol{\alpha}^T\boldsymbol{\Sigma}_\alpha(\boldsymbol{D}_\alpha-\widehat{\boldsymbol{D}}_\alpha)\boldsymbol{\Sigma}_\alpha\boldsymbol{\alpha}|\left[|\boldsymbol{\alpha}^T\boldsymbol{\Sigma}_\alpha(\boldsymbol{D}_\alpha-\widehat{\boldsymbol{D}}_\alpha)\boldsymbol{\Sigma}_\alpha\boldsymbol{\alpha}|+2|\boldsymbol{\alpha}^T\boldsymbol{\Sigma}_\alpha\boldsymbol{D}_\alpha\boldsymbol{\Sigma}_\alpha\boldsymbol{\alpha}|\right]\xrightarrow{p}0.\end{aligned}$$

It follows that

$$\frac{f(\widehat{\boldsymbol{\ell}}_a)}{f(\boldsymbol{\ell}_a)}\xrightarrow{p}1$$

as $n_{r\alpha}$ and $p\to\infty$. Following (29), we have

$$\frac{\widehat{\boldsymbol{\ell}}_a^T\boldsymbol{H}\widehat{\boldsymbol{\ell}}_a}{\boldsymbol{\ell}_a^T\boldsymbol{H}\boldsymbol{\ell}_a}\xrightarrow{p}1.$$

Thus, by (35) and (36), we have

$$\frac{\zeta_\alpha(\widehat{\boldsymbol{\ell}}_a)}{\zeta_\alpha(\boldsymbol{\ell}_a)}\xrightarrow{p}1$$

and

$$\frac{(\widehat{\boldsymbol{\ell}}_a^T\boldsymbol{H}\widehat{\boldsymbol{\ell}}_a)^{-1}\widehat{\boldsymbol{\ell}}_a^T\boldsymbol{H}(\widehat{\boldsymbol{w}}_a-\boldsymbol{w}_a)}{\zeta_\alpha(\boldsymbol{\ell}_a)}\xrightarrow{d}N(0,1),\tag{38}$$

as $n_{r\alpha}$ and $p\to\infty$.

By (31) and Lemma S4, under Condition **??**, we have

$$\mathrm{tr}(\boldsymbol{\Sigma}_\alpha\boldsymbol{D}_\alpha\boldsymbol{\Sigma}_\alpha\boldsymbol{D}_\alpha)\lesssim p,$$

$$\boldsymbol{\alpha}^T\boldsymbol{\Sigma}_\alpha\boldsymbol{D}_\alpha\boldsymbol{\Sigma}_\alpha\boldsymbol{D}_\alpha\boldsymbol{\Sigma}_\alpha\boldsymbol{\alpha}\lesssim\|\boldsymbol{\alpha}\|_2^2,$$

and

$$|\boldsymbol{\alpha}^T\boldsymbol{\Sigma}_\alpha\boldsymbol{D}_\alpha\boldsymbol{\Sigma}_\alpha\boldsymbol{\alpha}|\le\|\boldsymbol{D}_\alpha\|_2\|\boldsymbol{\Sigma}\|_2^2\|\boldsymbol{\alpha}\|_2^2\lesssim\|\boldsymbol{\alpha}\|_2^2,$$

which implies

$$\zeta_\alpha^2(\boldsymbol{\ell}_a)\lesssim\frac{\|\boldsymbol{\alpha}\|^4}{(\boldsymbol{\ell}_a^T\boldsymbol{H}\boldsymbol{\ell}_a)\cdot n_\alpha^2}+\frac{\|\boldsymbol{\alpha}\|^4}{(\boldsymbol{\ell}_a^T\boldsymbol{H}\boldsymbol{\ell}_a)^2\cdot n_\alpha}.\tag{39}$$

By Condition **??**, we have $\|\boldsymbol{\alpha}\|^2=O(p)$, which implies

$$\frac{\|\boldsymbol{\alpha}\|^4}{p^2\cdot\min\{n_\alpha,n_{r\alpha}^2\}}\lesssim\frac{1}{\min\{n_\alpha,n_{r\alpha}^2\}}\to0,\tag{40}$$

as $p,n_\alpha\to\infty$.

By (26), (39), and (40), under Condition **??**, we have $\zeta_\alpha^2(\boldsymbol{\ell}_a)\to0$ as $p,n_\alpha\to\infty$. □

S6.4. *Proof of Theorem S1.*

PROOF. We have $\zeta_\alpha^2(\boldsymbol{\ell}_a)\to0$ as $p,n_\alpha\to\infty$ under Conditions **??**, **??**, and **??** by (26), (39), and (40). Moreover,

$$\begin{aligned}\widehat{\sigma}_\alpha^2-\sigma_\alpha^2=&(\widehat{\boldsymbol{\ell}}_a^T\boldsymbol{H}\widehat{\boldsymbol{\ell}}_a)^{-1}\widehat{\boldsymbol{\ell}}_a^T\boldsymbol{H}(\widehat{\boldsymbol{w}}_a-\boldsymbol{w}_a)+\{(\widehat{\boldsymbol{\ell}}_a^T\boldsymbol{H}\widehat{\boldsymbol{\ell}}_a)^{-1}\widehat{\boldsymbol{\ell}}_a^T-(\boldsymbol{\ell}_a^T\boldsymbol{H}\boldsymbol{\ell}_a)^{-1}\boldsymbol{\ell}_a^T\}\boldsymbol{H}\boldsymbol{w}_a\\&+(\boldsymbol{\ell}_a^T\boldsymbol{H}\boldsymbol{\ell}_a)^{-1}\boldsymbol{\ell}_a^T\boldsymbol{H}\boldsymbol{\varepsilon}_a.\end{aligned}$$

By (26) and Condition **??**, we have $(\boldsymbol{\ell}_a^T \boldsymbol{H} \boldsymbol{\ell}_a)^{-1} \boldsymbol{\ell}_a^T \boldsymbol{H} \boldsymbol{\varepsilon}_a \to 0$. Note that

$$
\begin{aligned}
&\{(\widehat{\boldsymbol{\ell}}_a^T \boldsymbol{H} \widehat{\boldsymbol{\ell}}_a)^{-1} \widehat{\boldsymbol{\ell}}_a^T - (\boldsymbol{\ell}_a^T \boldsymbol{H} \boldsymbol{\ell}_a)^{-1} \boldsymbol{\ell}_a^T\} \boldsymbol{H} \boldsymbol{w}_a \\
&= \left\{ (\widehat{\boldsymbol{\ell}}_a^T \boldsymbol{H} \widehat{\boldsymbol{\ell}}_a / \boldsymbol{\ell}_a^T \boldsymbol{H} \boldsymbol{\ell}_a)^{-1} - 1 \right\} \frac{(\widehat{\boldsymbol{\ell}}_a - \boldsymbol{\ell}_a)^T \boldsymbol{H} \boldsymbol{w}_a}{\boldsymbol{\ell}_a^T \boldsymbol{H} \boldsymbol{\ell}_a} + \left\{ (\widehat{\boldsymbol{\ell}}_a^T \boldsymbol{H} \widehat{\boldsymbol{\ell}}_a / \boldsymbol{\ell}_a^T \boldsymbol{H} \boldsymbol{\ell}_a)^{-1} - 1 \right\} \frac{\boldsymbol{\ell}_a^T \boldsymbol{H} \boldsymbol{w}_a}{\boldsymbol{\ell}_a^T \boldsymbol{H} \boldsymbol{\ell}_a} \\
&\quad + \frac{(\widehat{\boldsymbol{\ell}}_a - \boldsymbol{\ell}_a)^T \boldsymbol{H} \boldsymbol{w}_a}{\boldsymbol{\ell}_a^T \boldsymbol{H} \boldsymbol{\ell}_a}.
\end{aligned}
$$

By Condition **??**, (27), and (40), we have

$$
\frac{(\widehat{\boldsymbol{\ell}}_a - \boldsymbol{\ell}_a)^T \boldsymbol{H} \boldsymbol{w}_a}{\boldsymbol{\ell}_a^T \boldsymbol{H} \boldsymbol{\ell}_a} \xrightarrow{p} 0.
$$

Following (29), we have $(\widehat{\boldsymbol{\ell}}_a^T \boldsymbol{H} \widehat{\boldsymbol{\ell}}_a - \boldsymbol{\ell}_a^T \boldsymbol{H} \boldsymbol{\ell}_a) / \boldsymbol{\ell}_a^T \boldsymbol{H} \boldsymbol{\ell}_a \xrightarrow{p} 0$. It follows that $\{(\widehat{\boldsymbol{\ell}}_a^T \widehat{\boldsymbol{\ell}}_a)^{-1} \widehat{\boldsymbol{\ell}}_a^T - (\boldsymbol{\ell}_a^T \boldsymbol{\ell}_a)^{-1} \boldsymbol{\ell}_a^T\} \boldsymbol{w}_a \xrightarrow{p} 0$. Under Condition 18 (for Lemma S7), by the convergence in (38) and $\zeta_\alpha^2(\boldsymbol{\ell}_a) \to 0$, we have

$$
(\widehat{\boldsymbol{\ell}}_a^T \widehat{\boldsymbol{\ell}}_a)^{-1} \widehat{\boldsymbol{\ell}}_a^T (\widehat{\boldsymbol{w}}_a - \boldsymbol{w}_a) \xrightarrow{p} 0.
$$

□

**S7. Bivariate LDSC.** In this section, we present the proof of Theorems **??**-**??** and S2. We begin by providing derivations of the bivariate LDSC estimator. Recall that $\sigma_{\alpha\beta} = \sum_{i=1}^p \alpha_i \beta_i / p$. For $j = 1, \ldots, p$, we have

$$
\begin{aligned}
E(\widehat{a}_j \widehat{b}_j) =& a_j b_j = \boldsymbol{\alpha}^T \boldsymbol{\Sigma}_{\alpha_j}^T \boldsymbol{\Sigma}_{\beta_j} \boldsymbol{\beta} = \sum_{i=1}^p \alpha_i \beta_i (\boldsymbol{\Sigma}_\alpha)_{ji} (\boldsymbol{\Sigma}_\beta)_{ji} + \sum_{i \neq k} \alpha_i \beta_k (\boldsymbol{\Sigma}_\alpha)_{ji} (\boldsymbol{\Sigma}_\beta)_{jk} \\
=& \sigma_{\alpha\beta} \cdot \sum_{i=1}^p (\boldsymbol{\Sigma}_\alpha)_{ji} (\boldsymbol{\Sigma}_\beta)_{ji} + \left\{ \sum_{i=1}^p \alpha_i \beta_i (\boldsymbol{\Sigma}_\alpha)_{ji} (\boldsymbol{\Sigma}_\beta)_{ji} - \sigma_{\alpha\beta} \cdot \sum_{i=1}^p (\boldsymbol{\Sigma}_\alpha)_{ji} (\boldsymbol{\Sigma}_\beta)_{ji} \right\} \\
&+ \sum_{i \neq k} \alpha_i \beta_k (\boldsymbol{\Sigma}_\alpha)_{ji} (\boldsymbol{\Sigma}_\beta)_{jk} \\
=& \sigma_{\alpha\beta} \cdot \ell_{ab,j} + \varepsilon_{ab,j},
\end{aligned}
$$

where $\varepsilon_{ab,j} = \sum_{i=1}^p \alpha_i \beta_i \boldsymbol{\Sigma}_{\alpha,ij} \boldsymbol{\Sigma}_{\beta,ij} - \sigma_{\alpha\beta} \cdot \sum_{i=1}^p \boldsymbol{\Sigma}_{\alpha,ij} \boldsymbol{\Sigma}_{\beta,ij} + \sum_{i \neq k} \alpha_i \beta_k \boldsymbol{\Sigma}_{\alpha,ij} \boldsymbol{\Sigma}_{\beta,kj}$.

S7.1. *Proof of Theorem* **??**.

PROOF. Let

$$
S_{p_{ab}} = \frac{(\widehat{\boldsymbol{\ell}}_{ab} - E\widehat{\boldsymbol{\ell}}_{ab})^T \boldsymbol{w}_{ab}}{\rho_{ab}},
$$

then we have

$$
\mathrm{Var}(S_{p_{ab}}) = \boldsymbol{w}_{ab}^T \mathrm{Cov}(\widehat{\boldsymbol{\ell}}_{ab}) \boldsymbol{w}_{ab} / \rho_{ab}^2.
$$

Since the elements in $\widehat{\boldsymbol{\ell}}_{ab}$ corresponding to genetic variants in different $\mathcal{N}$'s are independent under Condition **??**, $\mathrm{Cov}(\widehat{\boldsymbol{\ell}}_{ab})$ is block-diagonal with the same structure as $\mathcal{A}$.

For $1 \le m \le p_b$, let $W_m = (\widehat{\boldsymbol{\ell}}_{ab,\mathcal{N}(m)} - E\widehat{\boldsymbol{\ell}}_{ab,\mathcal{N}(m)})^T \boldsymbol{w}_{ab,\mathcal{N}(m)}/\rho_{ab}$, where $\widehat{\boldsymbol{\ell}}_{ab,\mathcal{N}(m)}$ and $\boldsymbol{w}_{ab,\mathcal{N}(m)}$ are sub-vectors of $\widehat{\boldsymbol{\ell}}_{ab}$ and $\boldsymbol{w}_{ab}$, respectively, consisting of elements corresponding to $\mathcal{N}(m)$. Then, $W_1, \dots, W_{p_b}$ are independent, and $\sum_{m=1}^{p_b} W_m = S_{p_{ab}}$. For $j, k \in \mathcal{N}(m)$, we have

$$\text{Cov}(\widehat{\ell}_{ab,j}, \widehat{\ell}_{ab,k}) = \sum_{i \in \mathcal{N}(m)} \sum_{l \in \mathcal{N}(m)} \text{Cov}(\widehat{\boldsymbol{\Sigma}}_{\alpha,ji}\widehat{\boldsymbol{\Sigma}}_{\beta,ji}, \widehat{\boldsymbol{\Sigma}}_{\alpha,kl}\widehat{\boldsymbol{\Sigma}}_{\beta,kl}).$$

Since $\widehat{\boldsymbol{\Sigma}}_{\alpha,ji}$ and $\widehat{\boldsymbol{\Sigma}}_{\alpha,kl}$ are sample covariance estimators, $n_{r\alpha}\widehat{\boldsymbol{\Sigma}}_{\alpha,ji}$ and $n_{r\alpha}\widehat{\boldsymbol{\Sigma}}_{\alpha,kl}$ are two elements in a Wishart random matrix under Condition **??**. By [10], we have

$$\text{Cov}(n_{r\alpha}\widehat{\boldsymbol{\Sigma}}_{\alpha,ji}, n_{r\alpha}\widehat{\boldsymbol{\Sigma}}_{\alpha,kl}) = n_{r\alpha}(\boldsymbol{\Sigma}_{\alpha,ki}\boldsymbol{\Sigma}_{\alpha,lj} + \boldsymbol{\Sigma}_{\alpha,kj}\boldsymbol{\Sigma}_{\alpha,li}). \tag{41}$$

Similarly, we have

$$\text{Cov}(n_{r\beta}\widehat{\boldsymbol{\Sigma}}_{\beta,ji}, n_{r\beta}\widehat{\boldsymbol{\Sigma}}_{\alpha,kl}) = n_{r\beta}(\boldsymbol{\Sigma}_{\beta,ki}\boldsymbol{\Sigma}_{\beta,lj} + \boldsymbol{\Sigma}_{\beta,kj}\boldsymbol{\Sigma}_{\beta,li}). \tag{42}$$

Note that

$$\begin{aligned}
&\text{Cov}(\widehat{\boldsymbol{\Sigma}}_{\alpha,ji}\widehat{\boldsymbol{\Sigma}}_{\beta,ji}, \widehat{\boldsymbol{\Sigma}}_{\alpha,kl}\widehat{\boldsymbol{\Sigma}}_{\beta,kl})\\
=&E(\widehat{\boldsymbol{\Sigma}}_{\alpha,ji}\widehat{\boldsymbol{\Sigma}}_{\beta,ji}\widehat{\boldsymbol{\Sigma}}_{\alpha,kl}\widehat{\boldsymbol{\Sigma}}_{\beta,kl}) - E(\widehat{\boldsymbol{\Sigma}}_{\alpha,ji}\widehat{\boldsymbol{\Sigma}}_{\beta,ji})E(\widehat{\boldsymbol{\Sigma}}_{\alpha,kl}\widehat{\boldsymbol{\Sigma}}_{\beta,kl})\\
=&E(\widehat{\boldsymbol{\Sigma}}_{\alpha,ji}\widehat{\boldsymbol{\Sigma}}_{\alpha,kl})E(\widehat{\boldsymbol{\Sigma}}_{\beta,ji}\widehat{\boldsymbol{\Sigma}}_{\beta,kl}) - E(\widehat{\boldsymbol{\Sigma}}_{\alpha,ji})E(\widehat{\boldsymbol{\Sigma}}_{\beta,ji})E(\widehat{\boldsymbol{\Sigma}}_{\alpha,kl})E(\widehat{\boldsymbol{\Sigma}}_{\beta,kl})\\
=&\{\text{Cov}(\widehat{\boldsymbol{\Sigma}}_{\alpha,ji}, \widehat{\boldsymbol{\Sigma}}_{\alpha,kl}) + \boldsymbol{\Sigma}_{\alpha,ji}\boldsymbol{\Sigma}_{\alpha,kl}\}\{\text{Cov}(\widehat{\boldsymbol{\Sigma}}_{\beta,ji}, \widehat{\boldsymbol{\Sigma}}_{\beta,kl}) + \boldsymbol{\Sigma}_{\beta,ij}\boldsymbol{\Sigma}_{\beta,kl}\}\\
&- \boldsymbol{\Sigma}_{\alpha,ji}\boldsymbol{\Sigma}_{\beta,ji}\boldsymbol{\Sigma}_{\alpha,kl}\boldsymbol{\Sigma}_{\beta,kl}\\
=&\{n_{r\alpha}^{-1} \cdot (\boldsymbol{\Sigma}_{\alpha,ki}\boldsymbol{\Sigma}_{\alpha,lj} + \boldsymbol{\Sigma}_{\alpha,kj}\boldsymbol{\Sigma}_{\alpha,li}) + \boldsymbol{\Sigma}_{\alpha,ji}\boldsymbol{\Sigma}_{\alpha,kl}\}\\
&\cdot \{n_{r\beta}^{-1} \cdot (\boldsymbol{\Sigma}_{\beta,ki}\boldsymbol{\Sigma}_{\beta,lj} + \boldsymbol{\Sigma}_{\beta,kj}\boldsymbol{\Sigma}_{\beta,li}) + \boldsymbol{\Sigma}_{\beta,ij}\boldsymbol{\Sigma}_{\beta,kl}\}\\
&- \boldsymbol{\Sigma}_{\alpha,ji}\boldsymbol{\Sigma}_{\beta,ji}\boldsymbol{\Sigma}_{\alpha,kl}\boldsymbol{\Sigma}_{\beta,kl}\\
=&n_{r\alpha}^{-1}n_{r\beta}^{-1} \cdot (\boldsymbol{\Sigma}_{\alpha,ki}\boldsymbol{\Sigma}_{\alpha,lj} + \boldsymbol{\Sigma}_{\alpha,kj}\boldsymbol{\Sigma}_{\alpha,li})(\boldsymbol{\Sigma}_{\beta,ki}\boldsymbol{\Sigma}_{\beta,lj} + \boldsymbol{\Sigma}_{\beta,kj}\boldsymbol{\Sigma}_{\beta,li})\\
&+ n_{r\alpha}^{-1} \cdot (\boldsymbol{\Sigma}_{\alpha,ki}\boldsymbol{\Sigma}_{\alpha,lj} + \boldsymbol{\Sigma}_{\alpha,kj}\boldsymbol{\Sigma}_{\alpha,li})\boldsymbol{\Sigma}_{\beta,ij}\boldsymbol{\Sigma}_{\beta,kl}\\
&+ n_{r\beta}^{-1} \cdot \boldsymbol{\Sigma}_{\alpha,ji}\boldsymbol{\Sigma}_{\alpha,kl}(\boldsymbol{\Sigma}_{\beta,ki}\boldsymbol{\Sigma}_{\beta,lj} + \boldsymbol{\Sigma}_{\beta,kj}\boldsymbol{\Sigma}_{\beta,li}).
\end{aligned} \tag{43}$$

The second equation in (43) comes from the independence of the two reference panels, and the fourth equation in (43) follows from (41) and (42). Thus, we have

$$\begin{aligned}
&\text{Cov}(\widehat{\ell}_{ab,j}, \widehat{\ell}_{ab,k})\\
=&n_{r\alpha}^{-1}n_{r\beta}^{-1} \cdot \{(\boldsymbol{\Sigma}_\alpha\boldsymbol{\Sigma}_\beta)_{kk}(\boldsymbol{\Sigma}_\alpha\boldsymbol{\Sigma}_\beta)_{jj} + \boldsymbol{\Sigma}_{\beta,kj}(\boldsymbol{\Sigma}_\alpha\boldsymbol{\Sigma}_\beta\boldsymbol{\Sigma}_\alpha)_{kj} + \boldsymbol{\Sigma}_{\alpha,kj}(\boldsymbol{\Sigma}_\beta\boldsymbol{\Sigma}_\alpha\boldsymbol{\Sigma}_\beta)_{kj}\\
&+ \boldsymbol{\Sigma}_{\alpha,kj}\boldsymbol{\Sigma}_{\beta,kj}\text{tr}(\boldsymbol{\Sigma}_{\alpha,\mathcal{N}(m)\mathcal{N}(m)}\boldsymbol{\Sigma}_{\beta,\mathcal{N}(m)\mathcal{N}(m)})\}\\
&+ n_{r\alpha}^{-1} \cdot \{(\boldsymbol{\Sigma}_\alpha\boldsymbol{\Sigma}_\beta)_{kj}(\boldsymbol{\Sigma}_\beta\boldsymbol{\Sigma}_\alpha)_{kj} + \boldsymbol{\Sigma}_{\alpha,kj}(\boldsymbol{\Sigma}_\beta\boldsymbol{\Sigma}_\alpha\boldsymbol{\Sigma}_\beta)_{kj}\}\\
&+ n_{r\beta}^{-1} \cdot \{(\boldsymbol{\Sigma}_\alpha\boldsymbol{\Sigma}_\beta)_{kj}(\boldsymbol{\Sigma}_\beta\boldsymbol{\Sigma}_\alpha)_{kj} + \boldsymbol{\Sigma}_{\beta,kj}(\boldsymbol{\Sigma}_\alpha\boldsymbol{\Sigma}_\beta\boldsymbol{\Sigma}_\alpha)_{kj}\}\\
=&n_{r\alpha}^{-1}n_{r\beta}^{-1} \cdot \{(\boldsymbol{\Sigma}_\alpha\boldsymbol{\Sigma}_\beta)_{kk}(\boldsymbol{\Sigma}_\alpha\boldsymbol{\Sigma}_\beta)_{jj} + \boldsymbol{\Sigma}_{\alpha,kj}\boldsymbol{\Sigma}_{\beta,kj}\text{tr}(\boldsymbol{\Sigma}_{\alpha,\mathcal{N}(m)\mathcal{N}(m)}\boldsymbol{\Sigma}_{\beta,\mathcal{N}(m)\mathcal{N}(m)})\}\\
&+ \frac{1 + n_{r\beta}}{n_{r\alpha}n_{r\beta}} \cdot \boldsymbol{\Sigma}_{\alpha,kj}(\boldsymbol{\Sigma}_\beta\boldsymbol{\Sigma}_\alpha\boldsymbol{\Sigma}_\beta)_{kj} + \frac{1 + n_{r\alpha}}{n_{r\alpha}n_{r\beta}} \cdot \boldsymbol{\Sigma}_{\beta,kj}(\boldsymbol{\Sigma}_\alpha\boldsymbol{\Sigma}_\beta\boldsymbol{\Sigma}_\alpha)_{kj}\\
&+ \frac{n_{r\alpha} + n_{r\beta}}{n_{r\alpha}n_{r\beta}} \cdot (\boldsymbol{\Sigma}_\alpha\boldsymbol{\Sigma}_\beta)_{kj}(\boldsymbol{\Sigma}_\beta\boldsymbol{\Sigma}_\alpha)_{kj}
\end{aligned} \tag{44}$$

and

$$\begin{aligned}
\text{Var}(S_{p_{ab}}) =&\rho_{ab}^{-2} \cdot \sum_{m=1}^{p_b} \sum_{j,k\in\mathcal{N}(m)} \boldsymbol{w}_{ab,j}\boldsymbol{w}_{ab,k}\text{Cov}(\widehat{\ell}_{ab,j}, \widehat{\ell}_{ab,k})\\
=&\rho_{ab}^{-2} \cdot \sum_{m=1}^{p_b} \sum_{j,k\in\mathcal{N}(m)} \boldsymbol{w}_{ab,j}\boldsymbol{w}_{ab,k}\Big[n_{r\alpha}^{-1}n_{r\beta}^{-1} \cdot \{(\boldsymbol{\Sigma}_\alpha\boldsymbol{\Sigma}_\beta)_{kk}(\boldsymbol{\Sigma}_\alpha\boldsymbol{\Sigma}_\beta)_{jj}\\
&+ \boldsymbol{\Sigma}_{\alpha,kj}\boldsymbol{\Sigma}_{\beta,kj}\text{tr}(\boldsymbol{\Sigma}_{\alpha,\mathcal{N}(m)\mathcal{N}(m)}\boldsymbol{\Sigma}_{\beta,\mathcal{N}(m)\mathcal{N}(m)})\}\\
&+ \frac{1+n_{r\beta}}{n_{r\alpha}n_{r\beta}} \cdot \boldsymbol{\Sigma}_{\alpha,kj}(\boldsymbol{\Sigma}_\beta\boldsymbol{\Sigma}_\alpha\boldsymbol{\Sigma}_\beta)_{kj} + \frac{1+n_{r\alpha}}{n_{r\alpha}n_{r\beta}} \cdot \boldsymbol{\Sigma}_{\beta,kj}(\boldsymbol{\Sigma}_\alpha\boldsymbol{\Sigma}_\beta\boldsymbol{\Sigma}_\alpha)_{kj}\\
&+\frac{n_{r\alpha}+n_{r\beta}}{n_{r\alpha}n_{r\beta}} \cdot (\boldsymbol{\Sigma}_\alpha\boldsymbol{\Sigma}_\beta)_{kj}(\boldsymbol{\Sigma}_\beta\boldsymbol{\Sigma}_\alpha)_{kj}\Big]\\
=&1,
\end{aligned}$$

where $\boldsymbol{w}_{ab,j}$ is the $j$th element of $\boldsymbol{w}_{ab}$. Let

$$\gamma_{ab} = \sum_{m=1}^{p_b} E(|W_m|^3) = \rho_{ab}^{-3} \cdot \sum_{m=1}^{p_b} E(|(\widehat{\boldsymbol{\ell}}_{ab,\mathcal{N}(m)} - E\widehat{\boldsymbol{\ell}}_{ab,\mathcal{N}(m)})^T \boldsymbol{w}_{ab,\mathcal{N}(m)}|^3).$$

Then we have

$$\gamma_{ab} \lesssim \rho_{ab}^{-3} \cdot \sum_{j=1}^{p} |\boldsymbol{w}_{ab,j}|^3 E|\widehat{\ell}_{ab,j} - E\widehat{\ell}_{ab,j}|^3.$$

For $j \in \mathcal{N}(m)$, we have

$$\begin{aligned}
|\widehat{\ell}_{ab,j} - E\widehat{\ell}_{ab,j}|^3 =&|\sum_{i\in\mathcal{N}(m)} (\widehat{\boldsymbol{\Sigma}}_{\alpha,ji}\widehat{\boldsymbol{\Sigma}}_{\beta,ji} - \boldsymbol{\Sigma}_{\alpha,ji}\boldsymbol{\Sigma}_{\beta,ji})|^3\\
=&|\sum_{i\in\mathcal{N}(m)} (\widehat{\boldsymbol{\Sigma}}_{\alpha,ji}\widehat{\boldsymbol{\Sigma}}_{\beta,ji} - \widehat{\boldsymbol{\Sigma}}_{\alpha,ji}\boldsymbol{\Sigma}_{\beta,ji} + \widehat{\boldsymbol{\Sigma}}_{\alpha,ji}\boldsymbol{\Sigma}_{\beta,ji} - \boldsymbol{\Sigma}_{\alpha,ji}\boldsymbol{\Sigma}_{\beta,ji})|^3\\
\lesssim& \sum_{i\in\mathcal{N}(m)} |\widehat{\boldsymbol{\Sigma}}_{\alpha,ji}(\widehat{\boldsymbol{\Sigma}}_{\beta,ji} - \boldsymbol{\Sigma}_{\beta,ji})|^3 + \sum_{i\in\mathcal{N}(m)} |(\widehat{\boldsymbol{\Sigma}}_{\alpha,ji} - \boldsymbol{\Sigma}_{\alpha,ji})\boldsymbol{\Sigma}_{\beta,ji}|^3\\
\lesssim& \sum_{i\in\mathcal{N}(m)} |(\widehat{\boldsymbol{\Sigma}}_{\alpha,ji} - \boldsymbol{\Sigma}_{\alpha,ji})(\widehat{\boldsymbol{\Sigma}}_{\beta,ji} - \boldsymbol{\Sigma}_{\beta,ji})|^3 + \sum_{i\in\mathcal{N}(m)} |\boldsymbol{\Sigma}_{\alpha,ji}(\widehat{\boldsymbol{\Sigma}}_{\beta,ji} - \boldsymbol{\Sigma}_{\beta,ji})|^3\\
&+ \sum_{i\in\mathcal{N}(m)} |(\widehat{\boldsymbol{\Sigma}}_{\alpha,ji} - \boldsymbol{\Sigma}_{\alpha,ji})\boldsymbol{\Sigma}_{\beta,ji}|^3\\
\lesssim& \sum_{i\in\mathcal{N}(m)} |\widehat{\boldsymbol{\Sigma}}_{\beta,ji} - \boldsymbol{\Sigma}_{\beta,ji}|^3 + \sum_{i\in\mathcal{N}(m)} |\widehat{\boldsymbol{\Sigma}}_{\alpha,ji} - \boldsymbol{\Sigma}_{\alpha,ji}|^3. \qquad (45)
\end{aligned}$$

The last inequality in (45) follows from Condition **??**. By Lemma S2, we have

$$E|\widehat{\boldsymbol{\Sigma}}_{\beta,ji} - \boldsymbol{\Sigma}_{\beta,ji}|^3 \le \left[n_{r\beta}^{-3} \cdot E(\boldsymbol{X}_{\beta,1i}\boldsymbol{X}_{\beta,1j})^4 + \frac{6(n_{r\beta}-1)}{n_{r\beta}^3} \cdot \{E(\boldsymbol{X}_{\beta,1i}\boldsymbol{X}_{\beta,1j})^2\}^2\right]^{3/4}.$$

By Condition **??**, for $j = 1, \ldots, p$, $E\boldsymbol{X}_{\alpha,1j}^8$ and $E\boldsymbol{X}_{\beta,1j}^8$ are bounded by constants. Therefore, we have

$$E|\widehat{\boldsymbol{\Sigma}}_{\beta,ji} - \boldsymbol{\Sigma}_{\beta,ji}|^3 \lesssim n_{r\beta}^{-3/2}.$$

Similarly, we have

$$E|\widehat{\mathbf{\Sigma}}_{\alpha,ji} - \mathbf{\Sigma}_{\alpha,ji}|^3 \lesssim n_{r\alpha}^{-3/2}.$$

It follows that

$$E|\widehat{\ell}_{ab,j} - E\widehat{\ell}_{ab,j}|^3 \lesssim q_b(n_{r\alpha}^{-3/2} + n_{r\beta}^{-3/2})$$

and

$$\gamma_{ab} \lesssim \frac{q_b(n_{r\alpha}^{-3/2} + n_{r\beta}^{-3/2})}{\rho_{ab}^3} \|\boldsymbol{w}_{ab}\|_3^3.$$

Recall that

$$\begin{aligned}\rho_{ab}^2 = \sum_{m=1}^{p_b} \sum_{j,k\in\mathcal{N}(m)} \boldsymbol{w}_{ab,j}\boldsymbol{w}_{ab,k} \Big[ & n_{r\alpha}^{-1}n_{r\beta}^{-1} \cdot \{(\mathbf{\Sigma}_\alpha\mathbf{\Sigma}_\beta)_{kk}(\mathbf{\Sigma}_\alpha\mathbf{\Sigma}_\beta)_{jj} \\ & + \mathbf{\Sigma}_{\alpha,kj}\mathbf{\Sigma}_{\beta,kj}\mathrm{tr}(\mathbf{\Sigma}_{\alpha,\mathcal{N}(m)\mathcal{N}(m)}\mathbf{\Sigma}_{\beta,\mathcal{N}(m)\mathcal{N}(m)})\} \\ & + \frac{1+n_{r\beta}}{n_{r\alpha}n_{r\beta}} \cdot \mathbf{\Sigma}_{\alpha,kj}(\mathbf{\Sigma}_\beta\mathbf{\Sigma}_\alpha\mathbf{\Sigma}_\beta)_{kj} + \frac{1+n_{r\alpha}}{n_{r\alpha}n_{r\beta}} \cdot \mathbf{\Sigma}_{\beta,kj}(\mathbf{\Sigma}_\alpha\mathbf{\Sigma}_\beta\mathbf{\Sigma}_\alpha)_{kj} \\ & + \frac{n_{r\alpha}+n_{r\beta}}{n_{r\alpha}n_{r\beta}} \cdot (\mathbf{\Sigma}_\alpha\mathbf{\Sigma}_\beta)_{kj}(\mathbf{\Sigma}_\beta\mathbf{\Sigma}_\alpha)_{kj} \Big].\end{aligned}$$

Note that the matrix with $(\mathbf{\Sigma}_\alpha\mathbf{\Sigma}_\beta)_{kk}(\mathbf{\Sigma}_\alpha\mathbf{\Sigma}_\beta)_{jj}$ as the $(k,j)$ element for $j,k\in\mathcal{N}(m)$ is positive semi-definite. The matrix with $\mathbf{\Sigma}_{\alpha,kj}\mathbf{\Sigma}_{\beta,kj}$ as the $(k,j)$ element is the Hadamard product of $\mathbf{\Sigma}_\alpha$ and $\mathbf{\Sigma}_\beta$, which is also a principal sub-matrix of the Kronecker product of $\mathbf{\Sigma}_\alpha$ and $\mathbf{\Sigma}_\beta$. Since $\mathbf{\Sigma}_\alpha$ and $\mathbf{\Sigma}_\beta$ are positive definite, the matrix with $\mathbf{\Sigma}_{\alpha,kj}\mathbf{\Sigma}_{\beta,kj}$ as the $(k,j)$ element is positive definite. Similarly, the eigenvalues of matrices with $\mathbf{\Sigma}_{\alpha,kj}(\mathbf{\Sigma}_\beta\mathbf{\Sigma}_\alpha\mathbf{\Sigma}_\beta)_{kj}$, $\mathbf{\Sigma}_{\beta,kj}(\mathbf{\Sigma}_\alpha\mathbf{\Sigma}_\beta\mathbf{\Sigma}_\alpha)_{kj}$, $(\mathbf{\Sigma}_\alpha\mathbf{\Sigma}_\beta)_{kj}(\mathbf{\Sigma}_\beta\mathbf{\Sigma}_\alpha)_{kj}$ as the $(k,j)$ element are bounded below by $\lambda_{\min}(\mathbf{\Sigma}_\alpha)\lambda_{\min}(\mathbf{\Sigma}_\beta\mathbf{\Sigma}_\alpha\mathbf{\Sigma}_\beta)$, $\lambda_{\min}(\mathbf{\Sigma}_\beta)\lambda_{\min}(\mathbf{\Sigma}_\alpha\mathbf{\Sigma}_\beta\mathbf{\Sigma}_\alpha)$, $\lambda_{\min}(\mathbf{\Sigma}_\beta\mathbf{\Sigma}_\alpha)\lambda_{\min}(\mathbf{\Sigma}_\alpha\mathbf{\Sigma}_\beta)$, respectively. Since eigenvalues $\lambda(\mathbf{\Sigma}_\alpha\mathbf{\Sigma}_\beta) = \lambda(\mathbf{\Sigma}_\alpha^{1/2}\mathbf{\Sigma}_\beta\mathbf{\Sigma}_\alpha^{1/2})$, we have

$$\lambda_{\min}(\mathbf{\Sigma}_\alpha\mathbf{\Sigma}_\beta\mathbf{\Sigma}_\alpha) \geq \lambda_{\min}^2(\mathbf{\Sigma}_\alpha)\lambda_{\min}(\mathbf{\Sigma}_\beta)$$

and $\lambda_{\min}(\mathbf{\Sigma}_\alpha\mathbf{\Sigma}_\beta) \geq \lambda_{\min}(\mathbf{\Sigma}_\alpha)\lambda_{\min}(\mathbf{\Sigma}_\beta)$. Then, by Condition **??** and Lemma S4, we have

$$\rho_{ab}^2 \gtrsim \frac{n_{r\alpha}+n_{r\beta}}{n_{r\alpha}n_{r\beta}} \cdot \sum_{m=1}^{p_b} \|\boldsymbol{w}_{ab,\mathcal{N}(m)}\|_2^2 = \frac{n_{r\alpha}+n_{r\beta}}{n_{r\alpha}n_{r\beta}} \cdot \|\boldsymbol{w}_{ab}\|_2^2.$$

Similarly, we have

$$\rho_{ab}^2 \lesssim \frac{n_{r\alpha}+n_{r\beta}}{n_{r\alpha}n_{r\beta}} \cdot \|\boldsymbol{w}_{ab}\|_2^2.$$

It follows that

$$\rho_{ab}^2 \asymp \frac{n_{r\alpha}+n_{r\beta}}{n_{r\alpha}n_{r\beta}} \cdot \|\boldsymbol{w}_{ab}\|_2^2,$$

$$\rho_{ab}^{-3} \lesssim \frac{n_{r\alpha}^{3/2}n_{r\beta}^{3/2}}{(n_{r\alpha}+n_{r\beta})^{3/2}} \cdot \|\boldsymbol{w}_{ab}\|_2^{-3},$$

and

$$\gamma_{ab} \lesssim \frac{q_b(n_{r\alpha}^{-3/2}+n_{r\beta}^{-3/2})n_{r\alpha}^{3/2}n_{r\beta}^{3/2}}{(n_{r\alpha}+n_{r\beta})^{3/2}} \cdot \left(\frac{\|\boldsymbol{w}_{ab}\|_3}{\|\boldsymbol{w}_{ab}\|_2}\right)^3 \lesssim \left(\frac{\|\boldsymbol{w}_{ab}\|_3}{\|\boldsymbol{w}_{ab}\|_2}\right)^3.$$

By Condition **??**, we have $\gamma_{ab} = o(1)$, which implies the convergence in distribution to a normal distribution. □

S7.2. *Proof of Theorem* **??**.

PROOF. Recall that $\widehat{\boldsymbol{w}}_{ab} = (\widehat{a}_1\widehat{b}_1, \ldots, \widehat{a}_j\widehat{b}_j, \ldots, \widehat{a}_p\widehat{b}_p)^T$. Since $\widehat{a}_j$ and $\widehat{b}_j$ are independent for $j = 1, \ldots, p$, $E\widetilde{\sigma}^2_{\alpha\beta} = (\boldsymbol{\ell}^T_{ab}\boldsymbol{\ell}_{ab})^{-1}\boldsymbol{\ell}^T_{ab}E\widehat{\boldsymbol{w}}_{ab} = (\boldsymbol{\ell}^T_{ab}\boldsymbol{\ell}_{ab})^{-1}\boldsymbol{\ell}^T_{ab}\boldsymbol{w}_{ab}$. Let $\overline{\sigma}_{\alpha\beta} = (\boldsymbol{\ell}^T_{ab}\boldsymbol{\ell}_{ab})^{-1}\boldsymbol{\ell}^T_{ab}\boldsymbol{w}_{ab}$. We also recall that

$$\zeta^2_{\alpha\beta}(\boldsymbol{\ell}_{ab}) = \text{Var}(\widetilde{\sigma}^2_{\alpha\beta}) = (\boldsymbol{\ell}^T_{ab}\boldsymbol{\ell}_{ab})^{-2}\text{Var}(\boldsymbol{\ell}^T_{ab}\widehat{\boldsymbol{w}}_{ab}).$$

**Step 1** (Calculation of the variance $\zeta^2_{\alpha\beta}$):
Since

$$\boldsymbol{\ell}^T_{ab}\widehat{\boldsymbol{w}}_{ab} = \sum_{j=1}^{p} \ell_{ab,j}\widehat{a}_j\widehat{b}_j = n_\alpha^{-1}n_\beta^{-1} \cdot \left\langle \boldsymbol{D}_{\alpha\beta}\boldsymbol{X}^T_\alpha\boldsymbol{y}_\alpha, \boldsymbol{X}^T_\beta\boldsymbol{y}_\beta \right\rangle,$$

we have

$$\text{Var}(\boldsymbol{\ell}^T_a\widehat{\boldsymbol{w}}_a) = n_\alpha^{-2}n_\beta^{-2} \cdot \text{Var}\left(\left\langle \boldsymbol{D}_{\alpha\beta}\boldsymbol{X}^T_\alpha\boldsymbol{y}_\alpha, \boldsymbol{X}^T_\beta\boldsymbol{y}_\beta \right\rangle\right).$$

Note that

$$\begin{aligned}\text{Var}\left(\left\langle \boldsymbol{D}_{\alpha\beta}\boldsymbol{X}^T_\alpha\boldsymbol{y}_\alpha, \boldsymbol{X}^T_\beta\boldsymbol{y}_\beta \right\rangle\right) =& E\left\{\text{Var}\left(\left\langle \boldsymbol{D}_{\alpha\beta}\boldsymbol{X}^T_\alpha\boldsymbol{y}_\alpha, \boldsymbol{X}^T_\beta\boldsymbol{y}_\beta \right\rangle \mid \boldsymbol{X}_\alpha, \boldsymbol{X}_\beta\right)\right\} \\ &+ \text{Var}\left\{E\left(\left\langle \boldsymbol{D}_{\alpha\beta}\boldsymbol{X}^T_\alpha\boldsymbol{y}_\alpha, \boldsymbol{X}^T_\beta\boldsymbol{y}_\beta \right\rangle \mid \boldsymbol{X}_\alpha, \boldsymbol{X}_\beta\right)\right\}.\end{aligned}$$

Since

$$\boldsymbol{D}_{\alpha\beta}\boldsymbol{X}^T_\alpha\boldsymbol{y}_\alpha = \boldsymbol{D}_{\alpha\beta}\boldsymbol{X}^T_\alpha(\boldsymbol{X}_\alpha\boldsymbol{\alpha} + \boldsymbol{\epsilon}_\alpha) = \boldsymbol{D}_{\alpha\beta}\boldsymbol{X}^T_\alpha\boldsymbol{X}_\alpha\boldsymbol{\alpha} + \boldsymbol{D}_{\alpha\beta}\boldsymbol{X}^T_\alpha\boldsymbol{\epsilon}_\alpha$$

and

$$\boldsymbol{X}^T_\beta\boldsymbol{y}_\beta = \boldsymbol{X}^T_\beta(\boldsymbol{X}_\beta\boldsymbol{\alpha} + \boldsymbol{\epsilon}_\beta) = \boldsymbol{X}^T_\beta\boldsymbol{X}_\beta\boldsymbol{\beta} + \boldsymbol{X}^T_\beta\boldsymbol{\epsilon}_\beta,$$

we have

$$\begin{aligned}&\text{Var}\left(\left\langle \boldsymbol{D}_{\alpha\beta}\boldsymbol{X}^T_\alpha\boldsymbol{y}_\alpha, \boldsymbol{X}^T_\beta\boldsymbol{y}_\beta \right\rangle \mid \boldsymbol{X}_\alpha, \boldsymbol{X}_\beta\right) \\ =&\text{Var}\left\{(\boldsymbol{D}_{\alpha\beta}\boldsymbol{X}^T_\alpha\boldsymbol{X}_\alpha\boldsymbol{\alpha})^T\boldsymbol{X}^T_\beta\boldsymbol{\epsilon}_\beta \mid \boldsymbol{X}_\alpha, \boldsymbol{X}_\beta\right\} + \text{Var}\left\{(\boldsymbol{D}_{\alpha\beta}\boldsymbol{X}^T_\alpha\boldsymbol{\epsilon}_\alpha)^T\boldsymbol{X}^T_\beta\boldsymbol{X}_\beta\boldsymbol{\beta} \mid \boldsymbol{X}_\alpha, \boldsymbol{X}_\beta\right\} \\ &+ \text{Var}\left\{(\boldsymbol{D}_{\alpha\beta}\boldsymbol{X}^T_\alpha\boldsymbol{\epsilon}_\alpha)^T\boldsymbol{X}^T_\beta\boldsymbol{\epsilon}_\beta \mid \boldsymbol{X}_\alpha, \boldsymbol{X}_\beta\right\} \\ &+ \text{Cov}\left\{(\boldsymbol{D}_{\alpha\beta}\boldsymbol{X}^T_\alpha\boldsymbol{X}_\alpha\boldsymbol{\alpha})^T\boldsymbol{X}^T_\beta\boldsymbol{\epsilon}_\beta, (\boldsymbol{D}_{\alpha\beta}\boldsymbol{X}^T_\alpha\boldsymbol{\epsilon}_\alpha)^T\boldsymbol{X}^T_\beta\boldsymbol{\epsilon}_\beta \mid \boldsymbol{X}_\alpha, \boldsymbol{X}_\beta\right\} \\ &+ \text{Cov}\left\{(\boldsymbol{D}_{\alpha\beta}\boldsymbol{X}^T_\alpha\boldsymbol{\epsilon}_\alpha)^T\boldsymbol{X}^T_\beta\boldsymbol{X}_\beta\boldsymbol{\beta}, (\boldsymbol{D}_{\alpha\beta}\boldsymbol{X}^T_\alpha\boldsymbol{\epsilon}_\alpha)^T\boldsymbol{X}^T_\beta\boldsymbol{\epsilon}_\beta \mid \boldsymbol{X}_\alpha, \boldsymbol{X}_\beta\right\} \\ =&\sigma^2_{\epsilon_\beta} \cdot \boldsymbol{\alpha}^T\boldsymbol{X}^T_\alpha\boldsymbol{X}_\alpha\boldsymbol{D}_{\alpha\beta}\boldsymbol{X}^T_\beta\boldsymbol{X}_\beta\boldsymbol{D}_{\alpha\beta}\boldsymbol{X}^T_\alpha\boldsymbol{X}_\alpha\boldsymbol{\alpha} + \sigma^2_{\epsilon_\alpha} \cdot \boldsymbol{\beta}^T\boldsymbol{X}^T_\beta\boldsymbol{X}_\beta\boldsymbol{D}_{\alpha\beta}\boldsymbol{X}^T_\alpha\boldsymbol{X}_\alpha\boldsymbol{D}_{\alpha\beta}\boldsymbol{X}^T_\beta\boldsymbol{X}_\beta\boldsymbol{\beta} \\ &+ \sigma^2_{\epsilon_\beta}\sigma^2_{\epsilon_\alpha} \cdot \text{tr}(\boldsymbol{X}_\alpha\boldsymbol{D}_{\alpha\beta}\boldsymbol{X}^T_\beta\boldsymbol{X}_\beta\boldsymbol{D}_{\alpha\beta}\boldsymbol{X}^T_\alpha).\end{aligned}$$

The last equality follows from $\boldsymbol{\epsilon}_\alpha \sim N(\boldsymbol{0}, \sigma^2_{\epsilon_\alpha}\boldsymbol{I})$, $\boldsymbol{\epsilon}_\beta \sim N(\boldsymbol{0}, \sigma^2_{\epsilon_\beta}\boldsymbol{I})$, and Lemma S13. In addition, we have

$$\begin{aligned}&E\left(\left\langle \boldsymbol{D}_{\alpha\beta}\boldsymbol{X}^T_\alpha\boldsymbol{y}_\alpha, \boldsymbol{X}^T_\beta\boldsymbol{y}_\beta \right\rangle \mid \boldsymbol{X}_\alpha, \boldsymbol{X}_\beta\right) \\ =&(\boldsymbol{D}_{\alpha\beta}\boldsymbol{X}^T_\alpha\boldsymbol{X}_\alpha\boldsymbol{\alpha})^T\boldsymbol{X}^T_\beta\boldsymbol{X}_\beta\boldsymbol{\beta} + E\left\{(\boldsymbol{D}_{\alpha\beta}\boldsymbol{X}^T_\alpha\boldsymbol{\epsilon}_\alpha)^T\boldsymbol{X}^T_\beta\boldsymbol{\epsilon}_\beta \mid \boldsymbol{X}_\alpha, \boldsymbol{X}_\beta\right\} \\ =&\boldsymbol{\alpha}^T\boldsymbol{X}^T_\alpha\boldsymbol{X}_\alpha\boldsymbol{D}_{\alpha\beta}\boldsymbol{X}^T_\beta\boldsymbol{X}_\beta\boldsymbol{\beta} + E\left(\boldsymbol{\epsilon}^T_\alpha\boldsymbol{X}_\alpha\boldsymbol{D}_{\alpha\beta}\boldsymbol{X}^T_\beta\boldsymbol{\epsilon}_\beta \mid \boldsymbol{X}_\alpha, \boldsymbol{X}_\beta\right) \\ =&\boldsymbol{\alpha}^T\boldsymbol{X}^T_\alpha\boldsymbol{X}_\alpha\boldsymbol{D}_{\alpha\beta}\boldsymbol{X}^T_\beta\boldsymbol{X}_\beta\boldsymbol{\beta}.\end{aligned}$$

The last equality above also follows from Lemma S13.

Note that, for any $p \times p$ matrix $\boldsymbol{A}$, $\boldsymbol{X}_\alpha \boldsymbol{A}$ and $\boldsymbol{X}_\beta \boldsymbol{A}$ are $n_\alpha \times p$ and $n_\beta \times p$ matrices with independent and identically distributed rows, respectively. By Condition **??**, we have that $\boldsymbol{X}_\alpha$ and $\boldsymbol{X}_\beta$ are normally distributed. Then each row in $\boldsymbol{X}_\alpha \boldsymbol{A}$ and $\boldsymbol{X}_\beta \boldsymbol{A}$ follows a multivariate normal distribution with mean $\mathbf{0}$ and covariance matrix $\boldsymbol{A}^T \boldsymbol{\Sigma}_\alpha \boldsymbol{A}$ and $\boldsymbol{A}^T \boldsymbol{\Sigma}_\beta \boldsymbol{A}$, which implies that $\boldsymbol{A}^T \boldsymbol{X}_\alpha^T \boldsymbol{X}_\alpha \boldsymbol{A}$ and $\boldsymbol{A}^T \boldsymbol{X}_\beta^T \boldsymbol{X}_\beta \boldsymbol{A}$ are Wishart$(n_\alpha, \boldsymbol{A}^T \boldsymbol{\Sigma}_\alpha \boldsymbol{A})$ and Wishart$(n_\beta, \boldsymbol{A}^T \boldsymbol{\Sigma}_\beta \boldsymbol{A})$, respectively. Then, by [11, Proposition S1], we have

$$
\begin{aligned}
& E\left(\boldsymbol{\alpha}^T \boldsymbol{X}_\alpha^T \boldsymbol{X}_\alpha \boldsymbol{D}_{\alpha\beta} \boldsymbol{X}_\beta^T \boldsymbol{X}_\beta \boldsymbol{D}_{\alpha\beta} \boldsymbol{X}_\alpha^T \boldsymbol{X}_\alpha \boldsymbol{\alpha}\right) \\
=& E\left\{E\left(\boldsymbol{\alpha}^T \boldsymbol{X}_\alpha^T \boldsymbol{X}_\alpha \boldsymbol{D}_{\alpha\beta} \boldsymbol{X}_\beta^T \boldsymbol{X}_\beta \boldsymbol{D}_{\alpha\beta} \boldsymbol{X}_\alpha^T \boldsymbol{X}_\alpha \boldsymbol{\alpha} \mid \boldsymbol{X}_\alpha\right)\right\} \\
=& n_\beta \cdot E\left(\boldsymbol{\alpha}^T \boldsymbol{X}_\alpha^T \boldsymbol{X}_\alpha \boldsymbol{D}_{\alpha\beta} \boldsymbol{\Sigma}_\beta \boldsymbol{D}_{\alpha\beta} \boldsymbol{X}_\alpha^T \boldsymbol{X}_\alpha \boldsymbol{\alpha}\right) \\
=& n_\beta \cdot E\left\{\boldsymbol{\alpha}^T \boldsymbol{D}_{\alpha\beta}^{-1} \boldsymbol{\Sigma}_\beta^{-1/2} \left(\boldsymbol{\Sigma}_\beta^{1/2} \boldsymbol{D}_{\alpha\beta} \boldsymbol{X}_\alpha^T \boldsymbol{X}_\alpha \boldsymbol{D}_{\alpha\beta} \boldsymbol{\Sigma}_\beta^{1/2}\right) \left(\boldsymbol{\Sigma}_\beta^{1/2} \boldsymbol{D}_{\alpha\beta} \boldsymbol{X}_\alpha^T \boldsymbol{X}_\alpha \boldsymbol{D}_{\alpha\beta} \boldsymbol{\Sigma}_\beta^{1/2}\right)\right. \\
& \left. \cdot \boldsymbol{\Sigma}_\beta^{-1/2} \boldsymbol{D}_{\alpha\beta}^{-1} \boldsymbol{\alpha}\right\} \\
=& n_\beta n_\alpha \cdot \operatorname{tr}(\boldsymbol{\Sigma}_\beta^{1/2} \boldsymbol{D}_{\alpha\beta} \boldsymbol{\Sigma}_\alpha \boldsymbol{D}_{\alpha\beta} \boldsymbol{\Sigma}_\beta^{1/2}) \cdot \boldsymbol{\alpha}^T \boldsymbol{\Sigma}_\alpha \boldsymbol{\alpha} + n_\beta n_\alpha (n_\alpha + 1) \cdot \boldsymbol{\alpha}^T \boldsymbol{\Sigma}_\alpha \boldsymbol{D}_{\alpha\beta} \boldsymbol{\Sigma}_\beta \boldsymbol{D}_{\alpha\beta} \boldsymbol{\Sigma}_\alpha \boldsymbol{\alpha} \\
=& n_\beta n_\alpha \cdot \operatorname{tr}(\boldsymbol{D}_{\alpha\beta} \boldsymbol{\Sigma}_\alpha \boldsymbol{D}_{\alpha\beta} \boldsymbol{\Sigma}_\beta) \cdot \boldsymbol{\alpha}^T \boldsymbol{\Sigma}_\alpha \boldsymbol{\alpha} + n_\beta n_\alpha (n_\alpha + 1) \cdot \boldsymbol{\alpha}^T \boldsymbol{\Sigma}_\alpha \boldsymbol{D}_{\alpha\beta} \boldsymbol{\Sigma}_\beta \boldsymbol{D}_{\alpha\beta} \boldsymbol{\Sigma}_\alpha \boldsymbol{\alpha}.
\end{aligned}
$$

Similarly, we have

$$
\begin{aligned}
& E\left(\boldsymbol{\beta}^T \boldsymbol{X}_\beta^T \boldsymbol{X}_\beta \boldsymbol{D}_{\alpha\beta} \boldsymbol{X}_\alpha^T \boldsymbol{X}_\alpha \boldsymbol{D}_{\alpha\beta} \boldsymbol{X}_\beta^T \boldsymbol{X}_\beta \boldsymbol{\beta}\right) \\
=& n_\beta n_\alpha \cdot \operatorname{tr}(\boldsymbol{D}_{\alpha\beta} \boldsymbol{\Sigma}_\alpha \boldsymbol{D}_{\alpha\beta} \boldsymbol{\Sigma}_\beta) \cdot \boldsymbol{\beta}^T \boldsymbol{\Sigma}_\beta \boldsymbol{\beta} + n_\beta n_\alpha (n_\beta + 1) \cdot \boldsymbol{\beta}^T \boldsymbol{\Sigma}_\beta \boldsymbol{D}_{\alpha\beta} \boldsymbol{\Sigma}_\alpha \boldsymbol{D}_{\alpha\beta} \boldsymbol{\Sigma}_\beta \boldsymbol{\beta}.
\end{aligned}
$$

Note that

$$
\begin{aligned}
& E\left\{\operatorname{tr}\left(\boldsymbol{D}_{\alpha\beta} \boldsymbol{X}_\beta^T \boldsymbol{X}_\beta \boldsymbol{D}_{\alpha\beta} \boldsymbol{X}_\alpha^T \boldsymbol{X}_\alpha\right)\right\} \\
=& \operatorname{tr}\left\{\boldsymbol{D}_{\alpha\beta} E\left(\boldsymbol{X}_\beta^T \boldsymbol{X}_\beta\right) \boldsymbol{D}_{\alpha\beta} E\left(\boldsymbol{X}_\alpha^T \boldsymbol{X}_\alpha\right)\right\} \\
=& n_\beta n_\alpha \cdot \operatorname{tr}\left(\boldsymbol{D}_{\alpha\beta} \boldsymbol{\Sigma}_\beta \boldsymbol{D}_{\alpha\beta} \boldsymbol{\Sigma}_\alpha\right).
\end{aligned}
$$

By Lemma S14 and [11, Proposition S1], we have

$$
\begin{aligned}
& \operatorname{Var}\left(\boldsymbol{\alpha}^T \boldsymbol{X}_\alpha^T \boldsymbol{X}_\alpha \boldsymbol{D}_{\alpha\beta} \boldsymbol{X}_\beta^T \boldsymbol{X}_\beta \boldsymbol{\beta}\right) \\
=& E\left[E\left\{\left(\boldsymbol{\alpha}^T \boldsymbol{X}_\alpha^T \boldsymbol{X}_\alpha \boldsymbol{D}_{\alpha\beta} \boldsymbol{X}_\beta^T \boldsymbol{X}_\beta \boldsymbol{\beta}\right)^2 \mid \boldsymbol{X}_\beta\right\}\right] - \left[E\left\{\boldsymbol{\alpha}^T \boldsymbol{X}_\alpha^T \boldsymbol{X}_\alpha \boldsymbol{D}_{\alpha\beta} \boldsymbol{X}_\beta^T \boldsymbol{X}_\beta \boldsymbol{\beta}\right\}\right]^2 \\
=& n_\alpha \cdot \boldsymbol{\alpha}^T \boldsymbol{\Sigma}_\alpha \boldsymbol{\alpha} E\left\{(\boldsymbol{D}_{\alpha\beta} \boldsymbol{X}_\beta^T \boldsymbol{X}_\beta \boldsymbol{\beta})^T \boldsymbol{\Sigma}_\alpha \boldsymbol{D}_{\alpha\beta} \boldsymbol{X}_\beta^T \boldsymbol{X}_\beta \boldsymbol{\beta}\right\} \\
& + n_\alpha (n_\alpha + 1) \cdot E\left(\boldsymbol{\alpha}^T \boldsymbol{\Sigma}_\alpha \boldsymbol{D}_{\alpha\beta} \boldsymbol{X}_\beta^T \boldsymbol{X}_\beta \boldsymbol{\beta}\right)^2 - n_\alpha^2 n_\beta^2 \cdot (\boldsymbol{\alpha}^T \boldsymbol{\Sigma}_\alpha \boldsymbol{D}_{\alpha\beta} \boldsymbol{\Sigma}_\beta \boldsymbol{\beta})^2 \\
=& n_\alpha \cdot \boldsymbol{\alpha}^T \boldsymbol{\Sigma}_\alpha \boldsymbol{\alpha} E\left\{\boldsymbol{\beta}^T \boldsymbol{D}_{\alpha\beta}^{-1} \boldsymbol{\Sigma}_\alpha^{-1/2} (\boldsymbol{\Sigma}_\alpha^{1/2} \boldsymbol{D}_{\alpha\beta} \boldsymbol{X}_\beta^T \boldsymbol{X}_\beta \boldsymbol{D}_{\alpha\beta} \boldsymbol{\Sigma}_\alpha^{1/2}) (\boldsymbol{\Sigma}_\alpha^{1/2} \boldsymbol{D}_{\alpha\beta} \boldsymbol{X}_\beta^T \boldsymbol{X}_\beta \boldsymbol{D}_{\alpha\beta} \boldsymbol{\Sigma}_\alpha^{1/2})\right. \\
& \left. \cdot \boldsymbol{\Sigma}_\alpha^{-1/2} \boldsymbol{D}_{\alpha\beta}^{-1} \boldsymbol{\beta}\right\} + n_\alpha (n_\alpha + 1) n_\beta \cdot \left(\boldsymbol{\alpha}^T \boldsymbol{\Sigma}_\alpha \boldsymbol{D}_{\alpha\beta} \boldsymbol{\Sigma}_\beta \boldsymbol{D}_{\alpha\beta} \boldsymbol{\Sigma}_\alpha \boldsymbol{\alpha} \cdot \boldsymbol{\beta}^T \boldsymbol{\Sigma}_\beta \boldsymbol{\beta}\right) \\
& + n_\alpha (n_\alpha + 1) n_\beta (n_\beta + 1) \cdot \left(\boldsymbol{\alpha}^T \boldsymbol{\Sigma}_\alpha \boldsymbol{D}_{\alpha\beta} \boldsymbol{\Sigma}_\beta \boldsymbol{\beta}\right)^2 - n_\alpha^2 n_\beta^2 \cdot (\boldsymbol{\alpha}^T \boldsymbol{\Sigma}_\alpha \boldsymbol{D}_{\alpha\beta} \boldsymbol{\Sigma}_\beta \boldsymbol{\beta})^2 \\
=& n_\alpha n_\beta \cdot \boldsymbol{\alpha}^T \boldsymbol{\Sigma}_\alpha \boldsymbol{\alpha} \cdot \operatorname{tr}(\boldsymbol{\Sigma}_\alpha^{1/2} \boldsymbol{D}_{\alpha\beta} \boldsymbol{\Sigma}_\beta \boldsymbol{D}_{\alpha\beta} \boldsymbol{\Sigma}_\alpha^{1/2}) \cdot \boldsymbol{\beta}^T \boldsymbol{\Sigma}_\beta \boldsymbol{\beta} + n_\alpha n_\beta (n_\beta + 1) \cdot \boldsymbol{\alpha}^T \boldsymbol{\Sigma}_\alpha \boldsymbol{\alpha} \\
& \cdot \boldsymbol{\beta}^T \boldsymbol{\Sigma}_\beta \boldsymbol{D}_{\alpha\beta} \boldsymbol{\Sigma}_\alpha \boldsymbol{D}_{\alpha\beta} \boldsymbol{\Sigma}_\beta \boldsymbol{\beta} + n_\alpha (n_\alpha + 1) n_\beta \cdot \left(\boldsymbol{\alpha}^T \boldsymbol{\Sigma}_\alpha \boldsymbol{D}_{\alpha\beta} \boldsymbol{\Sigma}_\beta \boldsymbol{D}_{\alpha\beta} \boldsymbol{\Sigma}_\alpha \boldsymbol{\alpha} \cdot \boldsymbol{\beta}^T \boldsymbol{\Sigma}_\beta \boldsymbol{\beta}\right) \\
& + n_\alpha (n_\alpha + 1) n_\beta (n_\beta + 1) \cdot \left(\boldsymbol{\alpha}^T \boldsymbol{\Sigma}_\alpha \boldsymbol{D}_{\alpha\beta} \boldsymbol{\Sigma}_\beta \boldsymbol{\beta}\right)^2 - n_\alpha^2 n_\beta^2 \cdot (\boldsymbol{\alpha}^T \boldsymbol{\Sigma}_\alpha \boldsymbol{D}_{\alpha\beta} \boldsymbol{\Sigma}_\beta \boldsymbol{\beta})^2 \\
=& n_\alpha n_\beta \cdot \boldsymbol{\alpha}^T \boldsymbol{\Sigma}_\alpha \boldsymbol{\alpha} \cdot \boldsymbol{\beta}^T \boldsymbol{\Sigma}_\beta \boldsymbol{\beta} \cdot \operatorname{tr}(\boldsymbol{\Sigma}_\alpha^{1/2} \boldsymbol{D}_{\alpha\beta} \boldsymbol{\Sigma}_\beta \boldsymbol{D}_{\alpha\beta} \boldsymbol{\Sigma}_\alpha^{1/2})
\end{aligned}
$$

$$
\begin{aligned}
&+ n_\alpha n_\beta (n_\beta + 1) \cdot \boldsymbol{\alpha}^T \boldsymbol{\Sigma}_\alpha \boldsymbol{\alpha} \cdot \boldsymbol{\beta}^T \boldsymbol{\Sigma}_\beta \boldsymbol{D}_{\alpha\beta} \boldsymbol{\Sigma}_\alpha \boldsymbol{D}_{\alpha\beta} \boldsymbol{\Sigma}_\beta \boldsymbol{\beta} \\
&+ n_\alpha n_\beta (n_\alpha + 1) \cdot \boldsymbol{\beta}^T \boldsymbol{\Sigma}_\beta \boldsymbol{\beta} \cdot \boldsymbol{\alpha}^T \boldsymbol{\Sigma}_\alpha \boldsymbol{D}_{\alpha\beta} \boldsymbol{\Sigma}_\beta \boldsymbol{D}_{\alpha\beta} \boldsymbol{\Sigma}_\alpha \boldsymbol{\alpha} \\
&+ n_\alpha n_\beta (n_\alpha + n_\beta + 1) \cdot \left( \boldsymbol{\alpha}^T \boldsymbol{\Sigma}_\alpha \boldsymbol{D}_{\alpha\beta} \boldsymbol{\Sigma}_\beta \boldsymbol{\beta} \right)^2 .
\end{aligned}
$$

Therefore, we have

$$
\begin{aligned}
\zeta^2_{\alpha\beta}(\boldsymbol{\ell}_{ab}) = & \frac{1}{(\boldsymbol{\ell}_{ab}^T \boldsymbol{\ell}_{ab})^2 n_\alpha n_\beta} \cdot \Big[ \sigma^2_{\epsilon_\beta} \cdot \big\{ \mathrm{tr}(\boldsymbol{D}_{\alpha\beta} \boldsymbol{\Sigma}_\alpha \boldsymbol{D}_{\alpha\beta} \boldsymbol{\Sigma}_\beta) \cdot \boldsymbol{\alpha}^T \boldsymbol{\Sigma}_\alpha \boldsymbol{\alpha} \\
& + (n_\alpha + 1) \cdot \boldsymbol{\alpha}^T \boldsymbol{\Sigma}_\alpha \boldsymbol{D}_{\alpha\beta} \boldsymbol{\Sigma}_\beta \boldsymbol{D}_{\alpha\beta} \boldsymbol{\Sigma}_\alpha \boldsymbol{\alpha} \big\} \\
& + \sigma^2_{\epsilon_\alpha} \cdot \big\{ \mathrm{tr}(\boldsymbol{D}_{\alpha\beta} \boldsymbol{\Sigma}_\alpha \boldsymbol{D}_{\alpha\beta} \boldsymbol{\Sigma}_\beta) \cdot \boldsymbol{\beta}^T \boldsymbol{\Sigma}_\beta \boldsymbol{\beta} + (n_\beta + 1) \cdot \boldsymbol{\beta}^T \boldsymbol{\Sigma}_\beta \boldsymbol{D}_{\alpha\beta} \boldsymbol{\Sigma}_\alpha \boldsymbol{D}_{\alpha\beta} \boldsymbol{\Sigma}_\beta \boldsymbol{\beta} \big\} \\
& + \sigma^2_{\epsilon_\beta} \sigma^2_{\epsilon_\alpha} \cdot \mathrm{tr} \left\{ \boldsymbol{D}_{\alpha\beta} \boldsymbol{\Sigma}_\beta \boldsymbol{D}_{\alpha\beta} \boldsymbol{\Sigma}_\alpha \right\} \\
& + \boldsymbol{\alpha}^T \boldsymbol{\Sigma}_\alpha \boldsymbol{\alpha} \cdot \boldsymbol{\beta}^T \boldsymbol{\Sigma}_\beta \boldsymbol{\beta} \cdot \mathrm{tr}(\boldsymbol{\Sigma}_\alpha^{1/2} \boldsymbol{D}_{\alpha\beta} \boldsymbol{\Sigma}_\beta \boldsymbol{D}_{\alpha\beta} \boldsymbol{\Sigma}_\alpha^{1/2}) \\
& + (n_\beta + 1) \cdot \boldsymbol{\alpha}^T \boldsymbol{\Sigma}_\alpha \boldsymbol{\alpha} \cdot \boldsymbol{\beta}^T \boldsymbol{\Sigma}_\beta \boldsymbol{D}_{\alpha\beta} \boldsymbol{\Sigma}_\alpha \boldsymbol{D}_{\alpha\beta} \boldsymbol{\Sigma}_\beta \boldsymbol{\beta} \\
& + (n_\alpha + 1) \cdot \boldsymbol{\beta}^T \boldsymbol{\Sigma}_\beta \boldsymbol{\beta} \cdot \boldsymbol{\alpha}^T \boldsymbol{\Sigma}_\alpha \boldsymbol{D}_{\alpha\beta} \boldsymbol{\Sigma}_\beta \boldsymbol{D}_{\alpha\beta} \boldsymbol{\Sigma}_\alpha \boldsymbol{\alpha} \\
& + (n_\alpha + n_\beta + 1) \cdot \left( \boldsymbol{\alpha}^T \boldsymbol{\Sigma}_\alpha \boldsymbol{D}_{\alpha\beta} \boldsymbol{\Sigma}_\beta \boldsymbol{\beta} \right)^2 \Big] .
\end{aligned}
$$

By Lemma S4, we have

$$
\begin{aligned}
\mathrm{tr}(\boldsymbol{\Sigma}_\alpha^{1/2} \boldsymbol{D}_{\alpha\beta} \boldsymbol{\Sigma}_\beta \boldsymbol{D}_{\alpha\beta} \boldsymbol{\Sigma}_\alpha^{1/2}) \geq & \lambda_{\min}(\boldsymbol{\Sigma}_\alpha) \mathrm{tr}(\boldsymbol{D}_{\alpha\beta} \boldsymbol{\Sigma}_\beta \boldsymbol{D}_{\alpha\beta}) \\
= & \lambda_{\min}(\boldsymbol{\Sigma}_\alpha) \mathrm{tr}(\boldsymbol{\Sigma}_\beta^{1/2} \boldsymbol{D}^2_{\alpha\beta} \boldsymbol{\Sigma}_\beta^{1/2}) \\
\geq & \lambda_{\min}(\boldsymbol{\Sigma}_\alpha) \lambda_{\min}(\boldsymbol{\Sigma}_\beta) \cdot \boldsymbol{\ell}_{ab}^T \boldsymbol{\ell}_{ab} \\
\geq & p \cdot \lambda_{\min}(\boldsymbol{\Sigma}_\alpha) \lambda_{\min}(\boldsymbol{\Sigma}_\beta) \boldsymbol{\ell}^2_{ab,\min} \qquad (46)
\end{aligned}
$$

and

$$
\mathrm{tr}(\boldsymbol{\Sigma}_\alpha^{1/2} \boldsymbol{D}_{\alpha\beta} \boldsymbol{\Sigma}_\beta \boldsymbol{D}_{\alpha\beta} \boldsymbol{\Sigma}_\alpha^{1/2}) \leq \lambda_{\max}(\boldsymbol{\Sigma}_\alpha) \lambda_{\max}(\boldsymbol{\Sigma}_\beta) \cdot \boldsymbol{\ell}_{ab}^T \boldsymbol{\ell}_{ab}.
$$

By Condition **??**, there exists constants $c_1$ and $c_2$ such that $\lambda_{\min}(\boldsymbol{\Sigma}_\alpha) \geq c_1$ and $\lambda_{\min}(\boldsymbol{\Sigma}_\beta) \geq c_2$. We also have $\sigma^2_{\epsilon_\alpha} \asymp \|\boldsymbol{\alpha}\|^2$ and $\sigma^2_{\epsilon_\beta} \asymp \|\boldsymbol{\beta}\|^2$. Therefore, we have

$$
\zeta^2_{\alpha\beta} \gtrsim \frac{(p + n_\beta + n_\alpha) \|\boldsymbol{\alpha}\|_2^2 \|\boldsymbol{\beta}\|_2^2}{(\boldsymbol{\ell}_{ab}^T \boldsymbol{\ell}_{ab})^2 n_\alpha n_\beta} \cdot \boldsymbol{\ell}^2_{ab,\min}. \qquad (47)
$$

Similarly, by Condition **??**, we have

$$
\zeta^2_{\alpha\beta}(\boldsymbol{\ell}_{ab}) \lesssim \frac{\|\boldsymbol{\alpha}\|^2 \|\boldsymbol{\beta}\|^2}{\boldsymbol{\ell}_{ab}^T \boldsymbol{\ell}_{ab} n_\alpha n_\beta} + \frac{\boldsymbol{\ell}^2_{ab,\max} \|\boldsymbol{\alpha}\|^2 \|\boldsymbol{\beta}\|^2}{(\boldsymbol{\ell}_{ab}^T \boldsymbol{\ell}_{ab})^2 n_\beta} + \frac{\boldsymbol{\ell}^2_{ab,\max} \|\boldsymbol{\alpha}\|^2 \|\boldsymbol{\beta}\|^2}{(\boldsymbol{\ell}_{ab}^T \boldsymbol{\ell}_{ab})^2 n_\alpha}. \qquad (48)
$$

**Step 2** (Asymptotic normality):
Note that

$$
\begin{aligned}
\widehat{a}_j &= n_\alpha^{-1} \cdot \sum_{i=1}^{n_\alpha} \boldsymbol{X}_{\alpha,ij} \boldsymbol{y}_{\alpha,i} \\
&= n_\alpha^{-1} \cdot \boldsymbol{X}_{\alpha,\cdot j}^T \boldsymbol{y}_\alpha \\
&= n_\alpha^{-1} \cdot \boldsymbol{X}_{\alpha,\cdot j}^T (\boldsymbol{X}_\alpha \boldsymbol{\alpha} + \boldsymbol{\epsilon}_\alpha) \\
&= n_\alpha^{-1} \cdot \boldsymbol{X}_{\alpha,\cdot j}^T \boldsymbol{X}_\alpha \boldsymbol{\alpha} + n_\alpha^{-1} \cdot \boldsymbol{X}_{\alpha,\cdot j}^T \boldsymbol{\epsilon}_\alpha,
\end{aligned}
$$

where $\boldsymbol{X}_{\alpha,ij}$ denotes the $(i,j)$th element in $\boldsymbol{X}_\alpha$, $\boldsymbol{y}_{\alpha,i}$ denotes the $i$th element in $\boldsymbol{y}_\alpha$, and $\boldsymbol{X}_{\alpha,\cdot j}$ denotes the $j$th column in $\boldsymbol{X}_\alpha$. Thus, $\widetilde{\sigma}^2_{\alpha\beta}$ is a continuous function of $\boldsymbol{X}_\alpha$, $\boldsymbol{X}_\beta$, $\boldsymbol{\epsilon}_\alpha$, and $\boldsymbol{\epsilon}_\beta$. We use $g(\boldsymbol{X}_\alpha, \boldsymbol{X}_\beta, \boldsymbol{\epsilon}_\alpha, \boldsymbol{\epsilon}_\beta)$ to denote this function. Let

$$\begin{aligned}\mathcal{U} = \Big[&\widetilde{\boldsymbol{U}} = \{(\boldsymbol{u}_\alpha^T\ \boldsymbol{u}_\beta^T)^T\ (\boldsymbol{U}_\alpha^T\ \boldsymbol{U}_\beta^T)^T\} : \boldsymbol{u}_\alpha = (u_{\alpha,1}, \ldots, u_{\alpha,n_\alpha})^T \in \mathbb{R}^{n_\alpha},\\ &\boldsymbol{u}_\beta = (u_{\alpha,1}, \ldots, u_{\beta,n_\beta})^T \in \mathbb{R}^{n_\beta}, \boldsymbol{U}_\alpha = (u_{\alpha,ij})_{1\le i\le n_\alpha, 1\le j\le p}, \boldsymbol{U}_\beta = (u_{\beta,ij})_{1\le i\le n_\beta, 1\le j\le p},\\ &\sum_{k=1}^{n_\alpha} u_{\alpha,k}^2 + \sum_{k=1}^{n_\beta} u_{\beta,k}^2 + \sum_{i=1}^{n_\alpha}\sum_{j=1}^{p} u_{\alpha,ij}^2 + \sum_{i=1}^{n_\beta}\sum_{j=1}^{p} u_{\beta,ij}^2 = 1\Big]\end{aligned}$$

be the collection of partitioned $(n_\alpha + n_\beta) \times (p+1)$ matrices with Frobenius norm equal to 1. For $\widetilde{\boldsymbol{U}} \in \mathcal{U}$, we define the differential operator

$$D_{\widetilde{\boldsymbol{U}}} = \sum_{i=1}^{n_\alpha}\sum_{j=1}^{p} u_{\alpha,ij}\frac{\partial}{\partial \boldsymbol{X}_{\alpha,ij}} + \sum_{i=1}^{n_\beta}\sum_{j=1}^{p} u_{\beta,ij}\frac{\partial}{\partial \boldsymbol{X}_{\beta,ij}} + \sum_{k=1}^{n_\alpha} u_{\alpha,k}\frac{\partial}{\partial \boldsymbol{\epsilon}_{\alpha,k}} + \sum_{k=1}^{n_\beta} u_{\beta,k}\frac{\partial}{\partial \boldsymbol{\epsilon}_{\beta,k}}.$$

Note that

$$\begin{aligned}&D_{\widetilde{\boldsymbol{U}}} g(\boldsymbol{X}_\alpha, \boldsymbol{X}_\beta, \boldsymbol{\epsilon}_\alpha, \boldsymbol{\epsilon}_\beta)\\ &= (\boldsymbol{\ell}_{ab}^T\boldsymbol{\ell}_{ab})^{-1}\sum_{k=1}^{p}\boldsymbol{\ell}_{ab,k}\Big\{\widehat{a}_k \cdot n_\beta^{-1}\cdot\big(\boldsymbol{X}_{\beta,\cdot k}^T\boldsymbol{U}_\beta\boldsymbol{\beta} + \boldsymbol{U}_{\beta,\cdot k}^T\boldsymbol{X}_\beta\boldsymbol{\beta} + \boldsymbol{U}_{\beta,\cdot k}^T\boldsymbol{\epsilon}_\beta + \boldsymbol{X}_{\beta,\cdot k}^T\boldsymbol{u}_\beta\big)\\ &\quad + \widehat{b}_k \cdot n_\alpha^{-1}\cdot\big(\boldsymbol{X}_{\alpha,\cdot k}^T\boldsymbol{U}_\alpha\boldsymbol{\alpha} + \boldsymbol{U}_{\alpha,\cdot k}^T\boldsymbol{X}_\alpha\boldsymbol{\alpha} + \boldsymbol{U}_{\alpha,\cdot k}^T\boldsymbol{\epsilon}_\alpha + \boldsymbol{X}_{\alpha,\cdot k}^T\boldsymbol{u}_\alpha\big)\Big\},\end{aligned}$$

where $\boldsymbol{U}_{\beta,\cdot k}$ denotes the $k$-th column in $\boldsymbol{U}_\beta$. Let $\eta_{x\alpha} = \left\|\boldsymbol{X}_\alpha/\sqrt{n_\alpha}\right\|, \eta_{\epsilon\alpha} = \left\|\epsilon_\alpha/\sqrt{n_\alpha}\right\|, \eta_\alpha = \|\boldsymbol{\alpha}\|, \eta_{v\alpha} = \|\boldsymbol{\Sigma}_\alpha^{1/2}\|$, $\eta_{x\epsilon\alpha} = \left\|\boldsymbol{X}_\alpha^T\boldsymbol{\epsilon}_\alpha/n_\alpha\right\|$, $\eta_{x\beta} = \left\|\boldsymbol{X}_\beta/\sqrt{n_\beta}\right\|, \eta_{\epsilon\beta} = \left\|\epsilon_\beta/\sqrt{n_\beta}\right\|, \eta_\beta = \|\boldsymbol{\beta}\|, \eta_{v\beta} = \|\boldsymbol{\Sigma}_\beta^{1/2}\|$, and $\eta_{x\epsilon\beta} = \left\|\boldsymbol{X}_\beta^T\boldsymbol{\epsilon}_\beta/n_\beta\right\|$. Then we have

$$\|\widehat{\boldsymbol{a}}\| = n_\alpha^{-1}\cdot\|\boldsymbol{X}_\alpha^T\boldsymbol{X}_\alpha\boldsymbol{\alpha} + \boldsymbol{X}_\alpha^T\boldsymbol{\epsilon}_\alpha\| \le \|\boldsymbol{\alpha}\|\|\boldsymbol{X}_\alpha^T\boldsymbol{X}_\alpha/n_\alpha\| + \|\boldsymbol{X}_\alpha^T\boldsymbol{\epsilon}_\alpha/n_\alpha\| = \eta_\alpha\eta_{x\alpha}^2 + \eta_{x\epsilon\alpha},$$

$$\|\widehat{\boldsymbol{b}}\| \le \eta_\beta\eta_{x\beta}^2 + \eta_{x\epsilon\beta},$$

and

$$\begin{aligned}&\big|D_{\widetilde{\boldsymbol{U}}} g(\boldsymbol{X}_\alpha, \boldsymbol{X}_\beta, \boldsymbol{\epsilon}_\alpha, \boldsymbol{\epsilon}_\beta)\big|\\ \le&(\boldsymbol{\ell}_{ab}^T\boldsymbol{\ell}_{ab})^{-1}\boldsymbol{\ell}_{ab,\max}\Big\{n_\beta^{-1}\cdot\widehat{\boldsymbol{a}}^T\big(\boldsymbol{X}_\beta^T\boldsymbol{U}_\beta\boldsymbol{\beta} + \boldsymbol{U}_\beta^T\boldsymbol{X}_\beta\boldsymbol{\beta} + \boldsymbol{U}_\beta^T\boldsymbol{\epsilon}_\beta + \boldsymbol{X}_\beta^T\boldsymbol{u}_\beta\big)\\ &+ n_\alpha^{-1}\cdot\widehat{\boldsymbol{b}}^T\big(\boldsymbol{X}_\alpha^T\boldsymbol{U}_\alpha\boldsymbol{\alpha} + \boldsymbol{U}_\alpha^T\boldsymbol{X}_\alpha\boldsymbol{\alpha} + \boldsymbol{U}_\alpha^T\boldsymbol{\epsilon}_\alpha + \boldsymbol{X}_\alpha^T\boldsymbol{u}_\alpha\big)\Big\},\\ \le&(\boldsymbol{\ell}_{ab}^T\boldsymbol{\ell}_{ab})^{-1}\boldsymbol{\ell}_{ab,\max}\Big\{n_\beta^{-1}\cdot\|\widehat{\boldsymbol{a}}\|\big(\|\boldsymbol{X}_\beta^T\boldsymbol{U}_\beta\boldsymbol{\beta}\| + \|\boldsymbol{U}_\beta^T\boldsymbol{X}_\beta\boldsymbol{\beta}\| + \|\boldsymbol{U}_\beta^T\boldsymbol{\epsilon}_\beta\| + \|\boldsymbol{X}_\beta^T\boldsymbol{u}_\beta\|\big)\\ &+ n_\alpha^{-1}\cdot\|\widehat{\boldsymbol{b}}\|\big(\|\boldsymbol{X}_\alpha^T\boldsymbol{U}_\alpha\boldsymbol{\alpha}\| + \|\boldsymbol{U}_\alpha^T\boldsymbol{X}_\alpha\boldsymbol{\alpha}\| + \|\boldsymbol{U}_\alpha^T\boldsymbol{\epsilon}_\alpha\| + \|\boldsymbol{X}_\alpha^T\boldsymbol{u}_\alpha\|\big)\Big\},\\ \le&(\boldsymbol{\ell}_{ab}^T\boldsymbol{\ell}_{ab})^{-1}\boldsymbol{\ell}_{ab,\max}\Big\{n_\beta^{-1/2}\cdot(\eta_\alpha\eta_{x\alpha}^2 + \eta_{x\epsilon\alpha})(2\eta_\beta\eta_{x\beta} + \eta_{\epsilon\beta} + \eta_{x\beta})\\ &+ n_\alpha^{-1/2}\cdot(\eta_\beta\eta_{x\beta}^2 + \eta_{x\epsilon\beta})(2\eta_\alpha\eta_{x\alpha} + \eta_{\epsilon\alpha} + \eta_{x\alpha})\Big\}.\end{aligned}$$

It follows that

$$
\begin{aligned}
&\left(E\|\nabla g(\boldsymbol{X}_\alpha, \boldsymbol{X}_\beta, \boldsymbol{\epsilon}_\alpha, \boldsymbol{\epsilon}_\beta)\|^4\right)^{1/4} \\
\lesssim&(\boldsymbol{\ell}_{ab}^T\boldsymbol{\ell}_{ab})^{-1}\boldsymbol{\ell}_{ab,\max}\Big\{n_\beta^{-2}\cdot E(\eta_\alpha\eta_{x\alpha}^2+\eta_{x\epsilon\alpha})^4 E(2\eta_\beta\eta_{x\beta}+\eta_{\epsilon\beta}+\eta_{x\beta})^4 \\
&+n_\alpha^{-2}\cdot E(\eta_\beta\eta_{x\beta}^2+\eta_{x\epsilon\beta})^4 E(2\eta_\alpha\eta_{x\alpha}+\eta_{\epsilon\alpha}+\eta_{x\alpha})^4\Big\}^{1/4}.
\end{aligned}
$$

By $\eta_{x\epsilon\alpha}\le\eta_{x\alpha}\eta_{\epsilon\alpha}$ and independence between $\boldsymbol{X}_\alpha$ and $\boldsymbol{\epsilon}_\alpha$, we have

$$
E(\eta_\alpha\eta_{x\alpha}^2+\eta_{x\epsilon\alpha})^4\lesssim E(\eta_\alpha\eta_{x\alpha}^2+\eta_{x\alpha}\eta_{\epsilon\alpha})^4\lesssim\eta_\alpha^4E\eta_{x\alpha}^8+E\eta_{x\alpha}^4E\eta_{\epsilon\alpha}^4,
$$

and

$$
E(2\eta_\alpha\eta_{x\alpha}+\eta_{\epsilon\alpha}+\eta_{x\alpha})^4\lesssim E\{(2\eta_\alpha+1)\eta_{x\alpha}+\eta_{\epsilon\alpha}\}^4\lesssim(2\eta_\alpha+1)^4E\eta_{x\alpha}^4+E\eta_{\epsilon\alpha}^4.
$$

For $k=1,\dots,8$, by Hölder's inequality, we have

$$
E\eta_{\epsilon\alpha}^k=E\left(\frac{\sum_{i=1}^{n_\alpha}\epsilon_{\alpha,i}^2}{n_\alpha}\right)^{k/2}\le\left\{E\left(\frac{\sum_{i=1}^{n_\alpha}\epsilon_{\alpha,i}^2}{n_\alpha}\right)^k\right\}^{1/2}.
$$

Since $\sum_{i=1}^{n_\alpha}\epsilon_{\alpha,i}^2/\sigma_{\epsilon_\alpha}^2\sim\chi^2(n_\alpha)$ and $E(\sum_{i=1}^{n_\alpha}\epsilon_{\alpha,i}^2/\sigma_{\epsilon_\alpha}^2)^k=O(n_\alpha^k)$, we have $E\eta_{\epsilon\alpha}^k=O(\|\boldsymbol{\alpha}\|^k)$. These results also hold if we replace $\boldsymbol{\alpha}$ with $\boldsymbol{\beta}$. Similarly, we have $E\eta_{\epsilon\beta}^k=O(\|\boldsymbol{\beta}\|^k)$.

By Condition **??** and Lemma S5, we have

$$
E\eta_{x\alpha}^8=E\left[\{\lambda_{\max}(\boldsymbol{X}_\alpha^T\boldsymbol{X}_\alpha/n_\alpha)\}^4\right]=O(1)\ \text{ and }\ E\eta_{x\beta}^8=E\left[\{\lambda_{\max}(\boldsymbol{X}_\beta^T\boldsymbol{X}_\beta/n_\beta)\}^4\right]=O(1).
$$

It follows that

$$
\begin{aligned}
\left(E\|\nabla g(\boldsymbol{X}_\alpha, \boldsymbol{X}_\beta, \boldsymbol{\epsilon}_\alpha, \boldsymbol{\epsilon}_\beta)\|^4\right)^{1/4}\lesssim&(\boldsymbol{\ell}_{ab}^T\boldsymbol{\ell}_{ab})^{-1}\boldsymbol{\ell}_{ab,\max}\Big\{(n_\alpha^{-2}+n_\beta^{-2})\|\boldsymbol{\alpha}\|^4\|\boldsymbol{\beta}\|^4\Big\}^{1/4} \\
\lesssim&(\boldsymbol{\ell}_{ab}^T\boldsymbol{\ell}_{ab})^{-1}\boldsymbol{\ell}_{ab,\max}(n_\alpha^{-1/2}+n_\beta^{-1/2})\|\boldsymbol{\alpha}\|\|\boldsymbol{\beta}\|.
\end{aligned}
$$

Let $\kappa_1=\left(E\|\nabla g(\boldsymbol{X}_\alpha, \boldsymbol{X}_\beta, \boldsymbol{\epsilon}_\alpha, \boldsymbol{\epsilon}_\beta)\|^4\right)^{1/4}$, then we have

$$
\kappa_1\lesssim(\boldsymbol{\ell}_{ab}^T\boldsymbol{\ell}_{ab})^{-1}\boldsymbol{\ell}_{ab,\max}(n_\alpha^{-1/2}+n_\beta^{-1/2})\|\boldsymbol{\alpha}\|\|\boldsymbol{\beta}\|. \tag{49}
$$

Note that

$$
\begin{aligned}
D_{\widetilde{\boldsymbol{U}}}^2g(\boldsymbol{X}_\alpha, \boldsymbol{X}_\beta, \boldsymbol{\epsilon}_\alpha, \boldsymbol{\epsilon}_\beta)=&2(\boldsymbol{\ell}_{ab}^T\boldsymbol{\ell}_{ab})^{-1}\sum_{k=1}^p\boldsymbol{\ell}_{ab,k}\cdot n_\alpha^{-1}n_\beta^{-1} \\
&\cdot\left(\boldsymbol{X}_{\beta,\cdot k}^T\boldsymbol{U}_\beta\boldsymbol{\beta}+\boldsymbol{U}_{\beta,\cdot k}^T\boldsymbol{X}_\beta\boldsymbol{\beta}+\boldsymbol{U}_{\beta,\cdot k}^T\boldsymbol{\epsilon}_\beta+\boldsymbol{X}_{\beta,\cdot k}^T\boldsymbol{u}_\beta\right) \\
&\cdot\left(\boldsymbol{X}_{\alpha,\cdot k}^T\boldsymbol{U}_\alpha\boldsymbol{\alpha}+\boldsymbol{U}_{\alpha,\cdot k}^T\boldsymbol{X}_\alpha\boldsymbol{\alpha}+\boldsymbol{U}_{\alpha,\cdot k}^T\boldsymbol{\epsilon}_\alpha+\boldsymbol{X}_{\alpha,\cdot k}^T\boldsymbol{u}_\alpha\right) \\
&+(\boldsymbol{\ell}_{ab}^T\boldsymbol{\ell}_{ab})^{-1}\sum_{k=1}^p\boldsymbol{\ell}_{ab,k}\widehat{b}_k\cdot2n_\alpha^{-1}\cdot\left(\boldsymbol{U}_{\alpha,\cdot k}^T\boldsymbol{U}_\alpha\boldsymbol{\alpha}+\boldsymbol{U}_{\alpha,\cdot k}^T\boldsymbol{u}_\alpha\right) \\
&+(\boldsymbol{\ell}_{ab}^T\boldsymbol{\ell}_{ab})^{-1}\sum_{k=1}^p\boldsymbol{\ell}_{ab,k}\widehat{a}_k\cdot2n_\beta^{-1}\cdot\left(\boldsymbol{U}_{\beta,\cdot k}^T\boldsymbol{U}_\beta\boldsymbol{\beta}+\boldsymbol{U}_{\beta,\cdot k}^T\boldsymbol{u}_\beta\right).
\end{aligned}
$$

Then we have

$$
|D_{\widetilde{\boldsymbol{U}}}^2g(\boldsymbol{X}_\alpha, \boldsymbol{X}_\beta, \boldsymbol{\epsilon}_\alpha, \boldsymbol{\epsilon}_\beta)|
$$

$$\begin{aligned}
&\lesssim \frac{1}{\sqrt{n_\alpha n_\beta}} (\boldsymbol{\ell}_{ab}^T \boldsymbol{\ell}_{ab})^{-1} \boldsymbol{\ell}_{ab,\max} \left( \frac{\boldsymbol{\alpha}^T \boldsymbol{U}_\alpha^T \boldsymbol{X}_\alpha \boldsymbol{X}_\beta^T \boldsymbol{U}_\beta \boldsymbol{\beta}}{\sqrt{n_\alpha n_\beta}} + \frac{\boldsymbol{\alpha}^T \boldsymbol{X}_\alpha^T \boldsymbol{U}_\alpha \boldsymbol{U}_\beta^T \boldsymbol{X}_\beta \boldsymbol{\beta}}{\sqrt{n_\alpha n_\beta}} \right. \\
&\quad \left. + \frac{\boldsymbol{\epsilon}_\alpha^T \boldsymbol{U}_\alpha \boldsymbol{U}_\beta^T \boldsymbol{\epsilon}_\beta}{\sqrt{n_\alpha n_\beta}} + \frac{\boldsymbol{u}_\alpha^T \boldsymbol{X}_\alpha \boldsymbol{X}_\alpha^T \boldsymbol{u}_\beta}{\sqrt{n_\alpha n_\beta}} \right) \\
&\quad + n_\alpha^{-1} \cdot (\boldsymbol{\ell}_{ab}^T \boldsymbol{\ell}_{ab})^{-1} \boldsymbol{\ell}_{ab,\max} |\widehat{\boldsymbol{b}}^T (\boldsymbol{U}_\alpha^T \boldsymbol{U}_\alpha \boldsymbol{\alpha} + \boldsymbol{U}_\alpha^T \boldsymbol{u}_\alpha)| \\
&\quad + n_\beta^{-1} \cdot (\boldsymbol{\ell}_{ab}^T \boldsymbol{\ell}_{ab})^{-1} \boldsymbol{\ell}_{ab,\max} |\widehat{\boldsymbol{a}}^T (\boldsymbol{U}_\beta^T \boldsymbol{U}_\beta \boldsymbol{\beta} + \boldsymbol{U}_\beta^T \boldsymbol{u}_\beta)| \\
&\le (\boldsymbol{\ell}_{ab}^T \boldsymbol{\ell}_{ab})^{-1} \boldsymbol{\ell}_{ab,\max} \left\{ \frac{2\eta_\alpha \eta_\beta \eta_{x\alpha} \eta_{x\beta} + \eta_{\epsilon\alpha}\eta_{\epsilon\beta} + \eta_{x\alpha}\eta_{x\beta}}{\sqrt{n_\alpha n_\beta}} \right. \\
&\quad \left. + \frac{(\eta_\beta \eta_{x\beta}^2 + \eta_{x\epsilon\beta})(\eta_\alpha + 1)}{n_\alpha} + \frac{(\eta_\alpha \eta_{x\alpha}^2 + \eta_{x\epsilon\alpha})(\eta_\beta + 1)}{n_\beta} \right\}
\end{aligned}$$

and

$$\begin{aligned}
&\left(E\|\nabla^2 g(\boldsymbol{X}_\alpha, \boldsymbol{X}_\beta, \boldsymbol{\epsilon}_\alpha, \boldsymbol{\epsilon}_\beta)\|^4\right)^{1/4} \\
&\lesssim (\boldsymbol{\ell}_{ab}^T \boldsymbol{\ell}_{ab})^{-1} \boldsymbol{\ell}_{ab,\max} \left\{ \frac{(2\eta_\alpha\eta_\beta + 1)^4 E\eta_{x\alpha}^4 E\eta_{x\beta}^4 + E\eta_{\epsilon\alpha}^4 E\eta_{\epsilon\beta}^4}{n_\alpha^2 n_\beta^2} \right. \\
&\quad \left. + \frac{(\eta_\alpha + 1)^4 E(\eta_\beta \eta_{x\beta}^2 + \eta_{x\epsilon\beta})^4}{n_\alpha^4} + \frac{(\eta_\beta + 1)^4 E(\eta_\alpha \eta_{x\alpha}^2 + \eta_{x\epsilon\alpha})^4}{n_\beta^4} \right\}^{1/4}.
\end{aligned}$$

Recall that $\eta_\alpha = \|\boldsymbol{\alpha}\|$, $\eta_\beta = \|\boldsymbol{\beta}\|$, $E\eta_{\epsilon\alpha}^k = O(\|\boldsymbol{\alpha}\|^k)$, $E\eta_{x\alpha}^8 = O(1)$, $E\eta_{\epsilon\beta}^k = O(\|\boldsymbol{\beta}\|^k)$, and $E\eta_{x\beta}^8 = O(1)$. Thus, we have

$$\begin{aligned}
&\left\{E\|\nabla^2 g(\boldsymbol{X}_\alpha, \boldsymbol{X}_\beta, \boldsymbol{\epsilon}_\alpha, \boldsymbol{\epsilon}_\beta)\|^4\right\}^{1/4} \\
\lesssim& (\boldsymbol{\ell}_{ab}^T \boldsymbol{\ell}_{ab})^{-1} \boldsymbol{\ell}_{ab,\max} \left( \frac{\|\boldsymbol{\alpha}\|^4 \|\boldsymbol{\beta}\|^4 + 1}{n_\alpha^2 n_\beta^2} + \frac{\|\boldsymbol{\alpha}\|^4 \|\boldsymbol{\beta}\|^4 + \|\boldsymbol{\beta}\|^4}{n_\alpha^4} + \frac{\|\boldsymbol{\alpha}\|^4 \|\boldsymbol{\beta}\|^4 + \|\boldsymbol{\alpha}\|^4}{n_\beta^4} \right)^{1/4} \\
\lesssim& (\boldsymbol{\ell}_{ab}^T \boldsymbol{\ell}_{ab})^{-1} \boldsymbol{\ell}_{ab,\max} \left( \frac{\|\boldsymbol{\alpha}\| \|\boldsymbol{\beta}\| + 1}{\sqrt{n_\alpha n_\beta}} + \frac{\|\boldsymbol{\alpha}\| \|\boldsymbol{\beta}\| + \|\boldsymbol{\beta}\|}{n_\alpha} + \frac{\|\boldsymbol{\alpha}\| \|\boldsymbol{\beta}\| + \|\boldsymbol{\alpha}\|}{n_\beta} \right).
\end{aligned}$$

Let $\kappa_2 = \left(E\|\nabla^2 g(\boldsymbol{X}_\alpha, \boldsymbol{X}_\beta, \boldsymbol{\epsilon}_\alpha, \boldsymbol{\epsilon}_\beta)\|^4\right)^{1/4}$, then we have

$$\kappa_2 \lesssim (\boldsymbol{\ell}_{ab}^T \boldsymbol{\ell}_{ab})^{-1} \boldsymbol{\ell}_{ab,\max} \left( n_\alpha^{-1/2} n_\beta^{-1/2} + n_\alpha^{-1} + n_\beta^{-1} \right) (\|\boldsymbol{\alpha}\| + 1)(\|\boldsymbol{\beta}\| + 1). \tag{50}$$

Let $Z$ be a random variable from $N(\overline{\sigma}_{\alpha\beta}^2, \zeta_{\alpha\beta}^2)$ and $d_{TV}(\widetilde{\sigma}_{\alpha\beta}^2, Z)$ be the total variation distance between the laws of $\widetilde{\sigma}_{\alpha\beta}^2$ and $Z$. If $\|\cdot\|$ of a matrix represents the spectral norm $\|\cdot\|_2$, by [9, Theorem 2.2], we have

$$d_{TV}(\widetilde{\sigma}_{\alpha\beta}^2, Z) \lesssim \frac{\max(\|\boldsymbol{\Sigma}_\alpha\|, \|\boldsymbol{\Sigma}_\beta\|)^{3/2} \kappa_1 \kappa_2}{\zeta_{\alpha\beta}^2(\boldsymbol{\ell}_{ab})}.$$

By Condition **??**, we have $\lambda_{\max}(\boldsymbol{\Sigma}_\alpha) = O(1)$ and $\lambda_{\max}(\boldsymbol{\Sigma}_\beta) = O(1)$. By inequalities in (47), (49), and (50), we have

$$\frac{\kappa_1 \kappa_2}{\zeta_{\alpha\beta}^2(\boldsymbol{\ell}_{ab})} \lesssim (\boldsymbol{\ell}_{ab}^T \boldsymbol{\ell}_{ab})^{-2} \boldsymbol{\ell}_{ab,\max}^2 \left( n_\alpha^{-1/2} + n_\beta^{-1/2} \right) \|\boldsymbol{\alpha}\| \|\boldsymbol{\beta}\| \left( \frac{\|\boldsymbol{\alpha}\| \|\boldsymbol{\beta}\| + 1}{\sqrt{n_\alpha n_\beta}} + \frac{\|\boldsymbol{\alpha}\| \|\boldsymbol{\beta}\| + \|\boldsymbol{\beta}\|}{n_\alpha} \right.$$

$$+\frac{\|\boldsymbol{\alpha}\|\|\boldsymbol{\beta}\|+\|\boldsymbol{\alpha}\|}{n_\beta}\Big)\frac{(\boldsymbol{\ell}_{ab}^T\boldsymbol{\ell}_{ab})^2 n_\alpha n_\beta\cdot\boldsymbol{\ell}_{ab,\min}^{-2}}{(p+n_\beta+n_\alpha)\|\boldsymbol{\alpha}\|_2^2\|\boldsymbol{\beta}\|_2^2}$$

$$=\left(n_\alpha^{-1/2}+n_\beta^{-1/2}\right)\left(1+\frac{1}{\|\boldsymbol{\alpha}\|\|\boldsymbol{\beta}\|}+\sqrt{\frac{n_\beta}{n_\alpha}}+\sqrt{\frac{n_\beta}{n_\alpha}}\frac{1}{\|\boldsymbol{\alpha}\|}+\sqrt{\frac{n_\alpha}{n_\beta}}+\sqrt{\frac{n_\alpha}{n_\beta}}\frac{1}{\|\boldsymbol{\beta}\|}\right)$$

$$\cdot\frac{1}{(p+n_\beta+n_\alpha)}\cdot\frac{\ell_{ab,\max}^2}{\boldsymbol{\ell}_{ab,\min}^2}.$$

By Conditions **??** and **??**, we have $\boldsymbol{\ell}_{ab,\min}$ bounded from below and $\boldsymbol{\ell}_{ab,\max}=O(1)$. By Condition **??**, we have $\kappa_1\kappa_2/\zeta_{\alpha\beta}^2(\boldsymbol{\ell}_{ab})=o(1)$, which implies that

$$\frac{\widetilde{\sigma}_{\alpha\beta}^2-\overline{\sigma}_{\alpha\beta}}{\zeta_{\alpha\beta}(\boldsymbol{\ell}_{ab})}\xrightarrow{d}N(0,1)$$

as $p\to\infty$. □

S7.3. *Proof of Theorem* **??**.

PROOF. Since elements in $\boldsymbol{\ell}_{ab}$ are diagonals of $\boldsymbol{\Sigma}_\alpha\boldsymbol{\Sigma}_\beta$, by Lemma S4, we have

$$\boldsymbol{\ell}_{ab}^T\boldsymbol{\ell}_{ab}\gtrsim\{\mathrm{tr}(\boldsymbol{\Sigma}_\alpha\boldsymbol{\Sigma}_\beta)\}^2/p\ge\{\lambda_{\min}(\boldsymbol{\Sigma}_\alpha)\lambda_{\min}(\boldsymbol{\Sigma}_\beta)\}^2p.$$

Under Condition **??**, we have

$$\boldsymbol{\ell}_{ab}^T\boldsymbol{\ell}_{ab}\gtrsim p. \tag{51}$$

**Step 1: To obtain (??)**
By (48) and Condition **??**, we have

$$\zeta_{\alpha\beta}^2(\boldsymbol{\ell}_{ab})\gtrsim\frac{(p+n_\beta+n_\alpha)\|\boldsymbol{\alpha}\|_2^2\|\boldsymbol{\beta}\|_2^2}{(\boldsymbol{\ell}_{ab}^T\boldsymbol{\ell}_{ab})^2n_\alpha n_\beta}\cdot\boldsymbol{\ell}_{ab,\min}^2\gtrsim\frac{(p+n_\beta+n_\alpha)\|\boldsymbol{\alpha}\|_2^2\|\boldsymbol{\beta}\|_2^2}{(\boldsymbol{\ell}_{ab}^T\boldsymbol{\ell}_{ab})^2n_\alpha n_\beta}. \tag{52}$$

It follows that

$$\frac{\boldsymbol{\ell}_{ab}^T\boldsymbol{\varepsilon}_{ab}}{\boldsymbol{\ell}_{ab}^T\boldsymbol{\ell}_{ab}\cdot\zeta_{\alpha\beta}(\boldsymbol{\ell}_{ab})}\lesssim\frac{n_\alpha^{1/2}n_\beta^{1/2}\boldsymbol{\ell}_{ab}^T\boldsymbol{\varepsilon}_{ab}}{(p+n_\alpha+n_\beta)^{1/2}\|\boldsymbol{\alpha}\|\|\boldsymbol{\beta}\|}.$$

By Conditions **??** and **??**, we have

$$\frac{\boldsymbol{\ell}_{ab}^T\boldsymbol{\varepsilon}_{ab}}{\boldsymbol{\ell}_{ab}^T\boldsymbol{\ell}_{ab}\cdot\zeta_{\alpha\beta}(\boldsymbol{\ell}_{ab})}=o(1),$$

which implies (**??**).

**Step 2: To obtain (??)**
Note that

$$\frac{\{(\widehat{\boldsymbol{\ell}}_{ab}^T\widehat{\boldsymbol{\ell}}_{ab})^{-1}\widehat{\boldsymbol{\ell}}_{ab}^T-(\boldsymbol{\ell}_{ab}^T\boldsymbol{\ell}_{ab})^{-1}\boldsymbol{\ell}_{ab}^T\}\boldsymbol{w}_{ab}}{\zeta_{\alpha\beta}(\boldsymbol{\ell}_{ab})}$$

$$=\frac{[\{(\widehat{\boldsymbol{\ell}}_{ab}^T\widehat{\boldsymbol{\ell}}_{ab})^{-1}-(\boldsymbol{\ell}_{ab}^T\boldsymbol{\ell}_{ab})^{-1}\}\widehat{\boldsymbol{\ell}}_{ab}^T}{\zeta_{\alpha\beta}(\boldsymbol{\ell}_{ab})}+\frac{(\boldsymbol{\ell}_{ab}^T\boldsymbol{\ell}_{ab})^{-1}(\widehat{\boldsymbol{\ell}}_{ab}^T-\boldsymbol{\ell}_{ab}^T)]\boldsymbol{w}_{ab}}{\zeta_{\alpha\beta}(\boldsymbol{\ell}_{ab})}$$

$$=\frac{\{(\widehat{\boldsymbol{\ell}}_{ab}^T\widehat{\boldsymbol{\ell}}_{ab})^{-1}-(\boldsymbol{\ell}_{ab}^T\boldsymbol{\ell}_{ab})^{-1}\}(\widehat{\boldsymbol{\ell}}_{ab}-\boldsymbol{\ell}_{ab})^T\boldsymbol{w}_{ab}}{\zeta_{\alpha\beta}(\boldsymbol{\ell}_{ab})}+\frac{\{(\widehat{\boldsymbol{\ell}}_{ab}^T\widehat{\boldsymbol{\ell}}_{ab})^{-1}-(\boldsymbol{\ell}_{ab}^T\boldsymbol{\ell}_{ab})^{-1}\}\boldsymbol{\ell}_{ab}^T\boldsymbol{w}_{ab}}{\zeta_{\alpha\beta}(\boldsymbol{\ell}_{ab})}$$

$$+ \frac{(\boldsymbol{\ell}_{ab}^T\boldsymbol{\ell}_{ab})^{-1}(\widehat{\boldsymbol{\ell}}_{ab} - \boldsymbol{\ell}_{ab})^T\boldsymbol{w}_{ab}}{\zeta_{\alpha\beta}(\boldsymbol{\ell}_{ab})}$$

$$= \left\{(\widehat{\boldsymbol{\ell}}_{ab}^T\widehat{\boldsymbol{\ell}}_{ab}/\boldsymbol{\ell}_{ab}^T\boldsymbol{\ell}_{ab})^{-1} - 1\right\} \frac{(\widehat{\boldsymbol{\ell}}_{ab} - \boldsymbol{\ell}_{ab})^T\boldsymbol{w}_{ab}}{\boldsymbol{\ell}_{ab}^T\boldsymbol{\ell}_{ab} \cdot \zeta_{\alpha\beta}(\boldsymbol{\ell}_{ab})} + \frac{(\widehat{\boldsymbol{\ell}}_{ab}^T\widehat{\boldsymbol{\ell}}_{ab}/\boldsymbol{\ell}_{ab}^T\boldsymbol{\ell}_{ab})^{-1} - 1}{\zeta_{\alpha\beta}(\boldsymbol{\ell}_{ab})} \frac{\boldsymbol{\ell}_{ab}^T\boldsymbol{w}_{ab}}{\boldsymbol{\ell}_{ab}^T\boldsymbol{\ell}_{ab}}$$

$$+ \frac{(\widehat{\boldsymbol{\ell}}_{ab} - \boldsymbol{\ell}_{ab})^T\boldsymbol{w}_{ab}}{\boldsymbol{\ell}_{ab}^T\boldsymbol{\ell}_{ab} \cdot \zeta_{\alpha\beta}(\boldsymbol{\ell}_{ab})}.$$

**Step 2.1:**
By (**??**), we have

$$\frac{\boldsymbol{\ell}_{ab}^T\boldsymbol{w}_{ab}}{\boldsymbol{\ell}_{ab}^T\boldsymbol{\ell}_{ab}} = \sigma_{\alpha\beta} + \frac{\boldsymbol{\ell}_{ab}^T\boldsymbol{\varepsilon}_{ab}}{\boldsymbol{\ell}_{ab}^T\boldsymbol{\ell}_{ab}}.$$

Note that $\sigma_{\alpha\beta} = \sum_{i=1}^p \alpha_i\beta_i/p$. By Condition **??** and (51), we have $\sum_{i=1}^p \alpha_i\beta_i/p = O(1)$ and

$$\frac{\boldsymbol{\ell}_{ab}^T\boldsymbol{\varepsilon}_{ab}}{\boldsymbol{\ell}_{ab}^T\boldsymbol{\ell}_{ab}} = o(1),$$

which implies

$$\frac{\boldsymbol{\ell}_{ab}^T\boldsymbol{w}_{ab}}{\boldsymbol{\ell}_{ab}^T\boldsymbol{\ell}_{ab}} = O(1).$$

**Step 2.2:**
If $\boldsymbol{w}_{ab} = \mathbf{0}$, then we have

$$\frac{(\widehat{\boldsymbol{\ell}}_{ab} - \boldsymbol{\ell}_{ab})^T\boldsymbol{w}_{ab}}{\boldsymbol{\ell}_{ab}^T\boldsymbol{\ell}_{ab} \cdot \zeta_{\alpha\beta}(\boldsymbol{\ell}_{ab})} = 0.$$

If $\boldsymbol{w}_{ab} \neq \mathbf{0}$, then we have

$$\frac{(\widehat{\boldsymbol{\ell}}_{ab} - \boldsymbol{\ell}_{ab})^T\boldsymbol{w}_{ab}}{\boldsymbol{\ell}_{ab}^T\boldsymbol{\ell}_{ab} \cdot \zeta_{\alpha\beta}(\boldsymbol{\ell}_{ab})} = \frac{(n_{r\alpha} + n_{r\beta})^{1/2}\|\boldsymbol{w}_{ab}\|_2}{(n_{r\alpha}n_{r\beta})^{1/2}\boldsymbol{\ell}_{ab}^T\boldsymbol{\ell}_{ab} \cdot \zeta_{\alpha\beta}(\boldsymbol{\ell}_{ab})} \cdot \frac{(n_{r\alpha}n_{r\beta})^{1/2}(\widehat{\boldsymbol{\ell}}_{ab} - \boldsymbol{\ell}_{ab})^T\boldsymbol{w}_{ab}}{(n_{r\alpha} + n_{r\beta})^{1/2}\|\boldsymbol{w}_{ab}\|_2}. \tag{53}$$

By Theorem **??**,

$$\frac{(n_{r\alpha}n_{r\beta})^{1/2}(\widehat{\boldsymbol{\ell}}_{ab} - \boldsymbol{\ell}_{ab})^T\boldsymbol{w}_{ab}}{(n_{r\alpha} + n_{r\beta})^{1/2}\|\boldsymbol{w}_{ab}\|_2}$$

converges in distribution to a normal distribution as $p \to \infty$. By (52), we have

$$\frac{(n_{r\alpha} + n_{r\beta})^{1/2}\|\boldsymbol{w}_{ab}\|_2}{(n_{r\alpha}n_{r\beta})^{1/2}\boldsymbol{\ell}_{ab}^T\boldsymbol{\ell}_{ab} \cdot \zeta_{\alpha\beta}(\boldsymbol{\ell}_{ab})} \lesssim \left\{\frac{n_\alpha n_\beta(n_{r\alpha} + n_{r\beta})\|\boldsymbol{w}_{ab}\|_2^2}{n_{r\alpha}n_{r\beta}(p + n_\alpha + n_\beta)\|\boldsymbol{\alpha}\|^2\|\boldsymbol{\beta}\|^2}\right\}^{1/2}$$

$$= \left\{\frac{n_\alpha n_\beta}{p + n_\alpha + n_\beta}\left(\frac{1}{n_{r\alpha}} + \frac{1}{n_{r\beta}}\right)\frac{\|\boldsymbol{w}_{ab}\|_2^2}{\|\boldsymbol{\alpha}\|^2\|\boldsymbol{\beta}\|^2}\right\}^{1/2}.$$

By Conditions **??** and **??**, we have

$$\frac{(n_{r\alpha} + n_{r\beta})^{1/2}\|\boldsymbol{w}_{ab}\|_2}{(n_{r\alpha}n_{r\beta})^{1/2}\boldsymbol{\ell}_{ab}^T\boldsymbol{\ell}_{ab} \cdot \zeta_{\alpha\beta}(\boldsymbol{\ell}_{ab})} \to 0$$

and

$$\frac{(\widehat{\boldsymbol{\ell}}_{ab} - \boldsymbol{\ell}_{ab})^T\boldsymbol{w}_{ab}}{\boldsymbol{\ell}_{ab}^T\boldsymbol{\ell}_{ab} \cdot \zeta_{\alpha\beta}(\boldsymbol{\ell}_{ab})} \xrightarrow{p} 0,$$

as $p \to \infty$.

**Step 2.3:**
Note that

$$\frac{(\widehat{\boldsymbol{\ell}}_{ab}^T\widehat{\boldsymbol{\ell}}_{ab}/\boldsymbol{\ell}_{ab}^T\boldsymbol{\ell}_{ab})^{-1}-1}{\zeta_{\alpha\beta}(\boldsymbol{\ell}_{ab})} = \frac{(p/n_{r\alpha}+p/n_{r\beta})^{1/2}}{\boldsymbol{\ell}_{ab}^T\boldsymbol{\ell}_{ab}\cdot\zeta_{\alpha\beta}(\boldsymbol{\ell}_{ab})}\cdot\frac{\{E(\widehat{\boldsymbol{\ell}}_{ab}^T\widehat{\boldsymbol{\ell}}_{ab})-\widehat{\boldsymbol{\ell}}_{ab}^T\widehat{\boldsymbol{\ell}}_{ab}\}/(p/n_{r\alpha}+p/n_{r\beta})^{1/2}}{(\widehat{\boldsymbol{\ell}}_{ab}^T\widehat{\boldsymbol{\ell}}_{ab}-\boldsymbol{\ell}_{ab}^T\boldsymbol{\ell}_{ab})/\boldsymbol{\ell}_{ab}^T\boldsymbol{\ell}_{ab}+1} + \frac{1}{\boldsymbol{\ell}_{ab}^T\boldsymbol{\ell}_{ab}\cdot\zeta_{\alpha\beta}(\boldsymbol{\ell}_{ab})}\cdot\frac{\boldsymbol{\ell}_{ab}^T\boldsymbol{\ell}_{ab}-E(\widehat{\boldsymbol{\ell}}_{ab}^T\widehat{\boldsymbol{\ell}}_{ab})}{(\widehat{\boldsymbol{\ell}}_{ab}^T\widehat{\boldsymbol{\ell}}_{ab}-\boldsymbol{\ell}_{ab}^T\boldsymbol{\ell}_{ab})/\boldsymbol{\ell}_{ab}^T\boldsymbol{\ell}_{ab}+1}.$$

By Lemma **??** and (51), we have

$$(\widehat{\boldsymbol{\ell}}_{ab}^T\widehat{\boldsymbol{\ell}}_{ab}-\boldsymbol{\ell}_{ab}^T\boldsymbol{\ell}_{ab})/\boldsymbol{\ell}_{ab}^T\boldsymbol{\ell}_{ab}\xrightarrow{p}0,$$

and $\{E(\boldsymbol{\ell}_{ab}^T\boldsymbol{\ell}_{ab})-\widehat{\boldsymbol{\ell}}_{ab}^T\widehat{\boldsymbol{\ell}}_{ab}\}/(p/n_{r\alpha}+p/n_{r\beta})^{1/2}$ converges in distribution to a normal distribution, as $p\to\infty$. Note that

$$\frac{(p/n_{r\alpha}+p/n_{r\beta})^{1/2}}{\boldsymbol{\ell}_{ab}^T\boldsymbol{\ell}_{ab}\cdot\zeta_{\alpha\beta}(\boldsymbol{\ell}_{ab})}\lesssim\left\{\frac{n_\alpha n_\beta(p/n_{r\alpha}+p/n_{r\beta})}{(p+n_\alpha+n_\beta)\|\boldsymbol{\alpha}\|^2\|\boldsymbol{\beta}\|^2}\right\}^{1/2} \lesssim\left(\frac{n_\alpha n_\beta/n_{r\alpha}+n_\alpha n_\beta/n_{r\beta}}{\|\boldsymbol{\alpha}\|^2\|\boldsymbol{\beta}\|^2}\right)^{1/2}$$

and

$$\left|\frac{1}{\boldsymbol{\ell}_{ab}^T\boldsymbol{\ell}_{ab}\cdot\zeta_{\alpha\beta}(\boldsymbol{\ell}_{ab})}\cdot\frac{\boldsymbol{\ell}_{ab}^T\boldsymbol{\ell}_{ab}-E(\widehat{\boldsymbol{\ell}}_{ab}^T\widehat{\boldsymbol{\ell}}_{ab})}{(\widehat{\boldsymbol{\ell}}_{ab}^T\widehat{\boldsymbol{\ell}}_{ab}-\boldsymbol{\ell}_{ab}^T\boldsymbol{\ell}_{ab})/\boldsymbol{\ell}_{ab}^T\boldsymbol{\ell}_{ab}+1}\right| \lesssim\frac{E(\widehat{\boldsymbol{\ell}}_{ab}^T\widehat{\boldsymbol{\ell}}_{ab})-\boldsymbol{\ell}_{ab}^T\boldsymbol{\ell}_{ab}}{\boldsymbol{\ell}_{ab}^T\boldsymbol{\ell}_{ab}\cdot\zeta_{\alpha\beta}(\boldsymbol{\ell}_{ab})} \lesssim(\frac{p}{n_{r\alpha}}+\frac{p}{n_{r\beta}})\left\{\frac{n_\alpha n_\beta}{(p+n_\alpha+n_\beta)\|\boldsymbol{\alpha}\|^2\|\boldsymbol{\beta}\|^2}\right\}^{1/2} \lesssim\sqrt{p}(\frac{1}{n_{r\alpha}}+\frac{1}{n_{r\beta}})\left(\frac{n_\alpha n_\beta}{\|\boldsymbol{\alpha}\|^2\|\boldsymbol{\beta}\|^2}\right)^{1/2}.$$

By Condition **??**, we have $\|\boldsymbol{\alpha}\|^2\|\boldsymbol{\beta}\|^2/(n_\alpha n_\beta/n_{r\alpha}+n_\alpha n_\beta/n_{r\beta})\to\infty$. It follows that

$$\frac{(p/n_{r\alpha}+p/n_{r\beta})^{1/2}}{\boldsymbol{\ell}_{ab}^T\boldsymbol{\ell}_{ab}\cdot\zeta_{\alpha\beta}(\boldsymbol{\ell}_{ab})}\xrightarrow{p}0$$

as $p\to\infty$. By Conditions **??** and **??**, we have

$$\left|\frac{1}{\boldsymbol{\ell}_{ab}^T\boldsymbol{\ell}_{ab}\cdot\zeta_{\alpha\beta}(\boldsymbol{\ell}_{ab})}\cdot\frac{\boldsymbol{\ell}_{ab}^T\boldsymbol{\ell}_{ab}-E(\widehat{\boldsymbol{\ell}}_{ab}^T\widehat{\boldsymbol{\ell}}_{ab})}{(\widehat{\boldsymbol{\ell}}_{ab}^T\widehat{\boldsymbol{\ell}}_{ab}-\boldsymbol{\ell}_{ab}^T\boldsymbol{\ell}_{ab})/\boldsymbol{\ell}_{ab}^T\boldsymbol{\ell}_{ab}+1}\right|\xrightarrow{p}0$$

and

$$\frac{(\widehat{\boldsymbol{\ell}}_{ab}^T\widehat{\boldsymbol{\ell}}_{ab}/\boldsymbol{\ell}_{ab}^T\boldsymbol{\ell}_{ab})^{-1}-1}{\zeta_{\alpha\beta}(\boldsymbol{\ell}_{ab})}\xrightarrow{p}0.$$

Similarly,

$$(\widehat{\boldsymbol{\ell}}_{ab}^T\widehat{\boldsymbol{\ell}}_{ab}/\boldsymbol{\ell}_{ab}^T\boldsymbol{\ell}_{ab})^{-1}-1=\frac{(p/n_{r\alpha}+p/n_{r\beta})^{1/2}}{\boldsymbol{\ell}_{ab}^T\boldsymbol{\ell}_{ab}}\cdot\frac{\{E(\boldsymbol{\ell}_{ab}^T\boldsymbol{\ell}_{ab})-\widehat{\boldsymbol{\ell}}_{ab}^T\widehat{\boldsymbol{\ell}}_{ab}\}/(p/n_{r\alpha}+p/n_{r\beta})^{1/2}}{(\widehat{\boldsymbol{\ell}}_{ab}^T\widehat{\boldsymbol{\ell}}_{ab}-\boldsymbol{\ell}_{ab}^T\boldsymbol{\ell}_{ab})/\boldsymbol{\ell}_{ab}^T\boldsymbol{\ell}_{ab}+1}$$
$$+\frac{\boldsymbol{\ell}_{ab}^T\boldsymbol{\ell}_{ab}-E(\boldsymbol{\ell}_{ab}^T\boldsymbol{\ell}_{ab})}{\boldsymbol{\ell}_{ab}^T\boldsymbol{\ell}_{ab}}\cdot\frac{1}{(\widehat{\boldsymbol{\ell}}_{ab}^T\widehat{\boldsymbol{\ell}}_{ab}-\boldsymbol{\ell}_{ab}^T\boldsymbol{\ell}_{ab})/\boldsymbol{\ell}_{ab}^T\boldsymbol{\ell}_{ab}+1}.$$

converges in probability to zero.

**Step 3: To obtain (??)**
**Step 3.1:** Let

$$V(\widehat{\boldsymbol{\ell}}_{ab})=\frac{(\widehat{\boldsymbol{\ell}}_{ab}^T\widehat{\boldsymbol{\ell}}_{ab})^{-1}\widehat{\boldsymbol{\ell}}_{ab}^T(\widehat{\boldsymbol{w}}_{ab}-\boldsymbol{w}_{ab})}{\zeta_{\alpha\beta}(\widehat{\boldsymbol{\ell}}_{ab})}.$$

Since

$$|\ell_{ab,j}|=\left|\sum_{i\in\mathcal{N}(k)}\boldsymbol{\Sigma}_{\alpha,ji}\boldsymbol{\Sigma}_{\beta,ji}\right|\le\sum_{i\in\mathcal{N}(k)}|\boldsymbol{\Sigma}_{\alpha,ji}||\boldsymbol{\Sigma}_{\beta,ji}|\le\sqrt{\sum_{i\in\mathcal{N}(k)}\boldsymbol{\Sigma}_{\alpha,ji}^2\sum_{i\in\mathcal{N}(k)}\boldsymbol{\Sigma}_{\beta,ji}^2},$$

by Condition **??**, we have

$$\boldsymbol{\ell}_{ab,\max}=O(1). \tag{54}$$

Under Condition **??**, there exists a positive constant $c$ such that $\boldsymbol{\ell}_{ab,\min}>c$. Note that

$$\widehat{\boldsymbol{\ell}}_{ab,\max}(n_{r\alpha},n_{r\beta})\le\boldsymbol{\ell}_{ab,\max}+\max_{1\le i\le p}|\widehat{\ell}_{ab,i}(n_{r\alpha},n_{r\beta})-\ell_{ab,i}|$$

and

$$\widehat{\boldsymbol{\ell}}_{ab,\min}(n_{r\alpha},n_{r\beta})\ge\boldsymbol{\ell}_{ab,\min}-\max_{1\le i\le p}|\widehat{\ell}_{ab,i}(n_{r\alpha},n_{r\beta})-\ell_{ab,i}|.$$

By Lemma S7, the second terms on the right-hand side in the above two inequalities converge in probability to zero, which implies that there exists positive constants $c_2$ and $c_3$ such that

$$\lim_{n_{r\alpha},n_{r\beta}\to\infty}P(\widehat{\boldsymbol{\ell}}_{ab,\max}(n_{r\alpha},n_{r\beta})<c_2)=1 \tag{55}$$

and

$$\lim_{n_{r\alpha},n_{r\beta}\to\infty}P(\widehat{\boldsymbol{\ell}}_{ab,\min}(n_{r\alpha},n_{r\beta})>c_3)=1. \tag{56}$$

Let $\mathcal{C}(c_2,c_3)=\{\widehat{\boldsymbol{\ell}}_{ab}(n_{r\alpha},n_{r\beta}):\widehat{\boldsymbol{\ell}}_{ab,\max}(n_{r\alpha},n_{r\beta})<c_2,\widehat{\boldsymbol{\ell}}_{ab,\min}(n_{r\alpha},n_{r\beta})>c_3\}$. For each $\widehat{\boldsymbol{\ell}}_{ab}(n_{r\alpha},n_{r\beta})\in\mathcal{C}(c_2,c_3)$, $V(\widehat{\boldsymbol{\ell}}_{ab})\mid\widehat{\boldsymbol{\ell}}_{ab}\xrightarrow{d}N(0,1)$ by Theorem **??** and Remark **??**. Let $Z$ be a normally distributed random variable. Note that

$$\begin{aligned}&\left|E_{\widehat{\boldsymbol{\ell}}_{ab}}[P(V(\widehat{\boldsymbol{\ell}}_{ab})\le t\mid\widehat{\boldsymbol{\ell}}_{ab})]-P(Z\le t)\right|\\ =&\left|\int_{\widehat{\boldsymbol{\ell}}_{ab}\in\mathcal{C}(c)}P(V(\widehat{\boldsymbol{\ell}}_{ab})\le t\mid\widehat{\boldsymbol{\ell}}_{ab})p(\widehat{\boldsymbol{\ell}}_{ab})d\widehat{\boldsymbol{\ell}}_{ab}-P(Z\le t)\right.\\ &\left.+\int_{\widehat{\boldsymbol{\ell}}_{ab}\in\mathcal{C}(c)^c}P(V(\widehat{\boldsymbol{\ell}}_{ab})\le t\mid\widehat{\boldsymbol{\ell}}_{ab})p(\widehat{\boldsymbol{\ell}}_{ab})d\widehat{\boldsymbol{\ell}}_{ab}\right|\end{aligned}$$

$$
\begin{aligned}
&= \left| \int_{\widehat{\boldsymbol{\ell}}_{ab} \in \mathcal{C}(c)} [P(Z \le t) + o(1)] p(\widehat{\boldsymbol{\ell}}_{ab}) d\widehat{\boldsymbol{\ell}}_{ab} - P(Z \le t) \right. \\
&\quad \left. + \int_{\widehat{\boldsymbol{\ell}}_{ab} \in \mathcal{C}(c)^c} P(V(\widehat{\boldsymbol{\ell}}_{ab}) \le t \mid \widehat{\boldsymbol{\ell}}_{ab}) p(\widehat{\boldsymbol{\ell}}_{ab}) d\widehat{\boldsymbol{\ell}}_{ab} \right| \\
&\le o(1) + P(\mathcal{C}(c_2, c_3)^c),
\end{aligned}
$$

where $p(\widehat{\boldsymbol{\ell}}_{ab})$ represents the density function of $\widehat{\boldsymbol{\ell}}_{ab}$. By (55) and (56), we have $P(\mathcal{C}(c_2, c_3)^c) \to 0$. Thus, we have

$$
P(V(\widehat{\boldsymbol{\ell}}_{ab}) \le t) - P(Z \le t) = E_{\widehat{\boldsymbol{\ell}}_{ab}}[P(V(\widehat{\boldsymbol{\ell}}_{ab}) \le t \mid \widehat{\boldsymbol{\ell}}_{ab})] - P(Z \le t) \to 0.
$$

This implies that $V(\widehat{\boldsymbol{\ell}}_{ab}) \xrightarrow{d} N(0,1)$ as $n_{r\alpha}, n_{r\beta}$, and $p \to \infty$.

**Step 3.2:**
Note that

$$
\frac{(\widehat{\boldsymbol{\ell}}_{ab}^T \widehat{\boldsymbol{\ell}}_{ab})^{-1} \widehat{\boldsymbol{\ell}}_{ab}^T (\widehat{\boldsymbol{w}}_{ab} - \boldsymbol{w}_{ab})}{\zeta_{\alpha\beta}(\boldsymbol{\ell}_{ab})} = V(\widehat{\boldsymbol{\ell}}_{ab}) \cdot \frac{\zeta_{\alpha\beta}(\widehat{\boldsymbol{\ell}}_{ab})}{\zeta_{\alpha\beta}(\boldsymbol{\ell}_{ab})} \tag{57}
$$

and

$$
\frac{\zeta_{\alpha\beta}(\widehat{\boldsymbol{\ell}}_{ab})}{\zeta_{\alpha\beta}(\boldsymbol{\ell}_{ab})} = \left\{ \frac{f(\widehat{\boldsymbol{\ell}}_{ab})}{f(\boldsymbol{\ell}_{ab})} \right\}^{1/2} \cdot \frac{\boldsymbol{\ell}_{ab}^T \boldsymbol{\ell}_{ab}}{\widehat{\boldsymbol{\ell}}_{ab}^T \widehat{\boldsymbol{\ell}}_{ab}}, \tag{58}
$$

where

$$
\begin{aligned}
f(\boldsymbol{\ell}_{ab}) =& \sigma_{\epsilon_\beta}^2 \cdot \left\{ \mathrm{tr}(\boldsymbol{D}_{\alpha\beta} \boldsymbol{\Sigma}_\alpha \boldsymbol{D}_{\alpha\beta} \boldsymbol{\Sigma}_\beta) \cdot \boldsymbol{\alpha}^T \boldsymbol{\Sigma}_\alpha \boldsymbol{\alpha} + (n_\alpha + 1) \cdot \boldsymbol{\alpha}^T \boldsymbol{\Sigma}_\alpha \boldsymbol{D}_{\alpha\beta} \boldsymbol{\Sigma}_\beta \boldsymbol{D}_{\alpha\beta} \boldsymbol{\Sigma}_\alpha \boldsymbol{\alpha} \right\} \\
&+ \sigma_{\epsilon_\alpha}^2 \cdot \left\{ \mathrm{tr}(\boldsymbol{D}_{\alpha\beta} \boldsymbol{\Sigma}_\alpha \boldsymbol{D}_{\alpha\beta} \boldsymbol{\Sigma}_\beta) \cdot \boldsymbol{\beta}^T \boldsymbol{\Sigma}_\beta \boldsymbol{\beta} + (n_\beta + 1) \cdot \boldsymbol{\beta}^T \boldsymbol{\Sigma}_\beta \boldsymbol{D}_{\alpha\beta} \boldsymbol{\Sigma}_\alpha \boldsymbol{D}_{\alpha\beta} \boldsymbol{\Sigma}_\beta \boldsymbol{\beta} \right\} \\
&+ \sigma_{\epsilon_\beta}^2 \sigma_{\epsilon_\alpha}^2 \cdot \mathrm{tr}\left( \boldsymbol{D}_{\alpha\beta} \boldsymbol{\Sigma}_\beta \boldsymbol{D}_{\alpha\beta} \boldsymbol{\Sigma}_\alpha \right) \\
&+ \boldsymbol{\alpha}^T \boldsymbol{\Sigma}_\alpha \boldsymbol{\alpha} \cdot \boldsymbol{\beta}^T \boldsymbol{\Sigma}_\beta \boldsymbol{\beta} \cdot \mathrm{tr}(\boldsymbol{\Sigma}_\alpha^{1/2} \boldsymbol{D}_{\alpha\beta} \boldsymbol{\Sigma}_\beta \boldsymbol{D}_{\alpha\beta} \boldsymbol{\Sigma}_\alpha^{1/2}) \\
&+ (n_\beta + 1) \cdot \boldsymbol{\alpha}^T \boldsymbol{\Sigma}_\alpha \boldsymbol{\alpha} \cdot \boldsymbol{\beta}^T \boldsymbol{\Sigma}_\beta \boldsymbol{D}_{\alpha\beta} \boldsymbol{\Sigma}_\alpha \boldsymbol{D}_{\alpha\beta} \boldsymbol{\Sigma}_\beta \boldsymbol{\beta} \\
&+ (n_\alpha + 1) \cdot \boldsymbol{\beta}^T \boldsymbol{\Sigma}_\beta \boldsymbol{\beta} \cdot \boldsymbol{\alpha}^T \boldsymbol{\Sigma}_\alpha \boldsymbol{D}_{\alpha\beta} \boldsymbol{\Sigma}_\beta \boldsymbol{D}_{\alpha\beta} \boldsymbol{\Sigma}_\alpha \boldsymbol{\alpha} \\
&+ (n_\alpha + n_\beta + 1) \cdot \left( \boldsymbol{\alpha}^T \boldsymbol{\Sigma}_\alpha \boldsymbol{D}_{\alpha\beta} \boldsymbol{\Sigma}_\beta \boldsymbol{\beta} \right)^2
\end{aligned}
$$

and

$$
\frac{f(\widehat{\boldsymbol{\ell}}_{ab})}{f(\boldsymbol{\ell}_{ab})} - 1 = \frac{f(\widehat{\boldsymbol{\ell}}_{ab}) - f(\boldsymbol{\ell}_{ab})}{f(\boldsymbol{\ell}_{ab})}. \tag{59}
$$

By Condition **??**, we have

$$
\begin{aligned}
&|f(\widehat{\boldsymbol{\ell}}_{ab}) - f(\boldsymbol{\ell}_{ab})| \\
\lesssim& \|\boldsymbol{\alpha}\|^2 \|\boldsymbol{\beta}\|^2 |\mathrm{tr}(\boldsymbol{D}_{\alpha\beta} \boldsymbol{\Sigma}_\alpha \boldsymbol{D}_{\alpha\beta} \boldsymbol{\Sigma}_\beta) - \mathrm{tr}(\widehat{\boldsymbol{D}}_{\alpha\beta} \boldsymbol{\Sigma}_\alpha \widehat{\boldsymbol{D}}_{\alpha\beta} \boldsymbol{\Sigma}_\beta)| \\
&+ n_\alpha \cdot \|\boldsymbol{\alpha}\|^2 \|\boldsymbol{\beta}\|^2 |\boldsymbol{\alpha}^T \boldsymbol{\Sigma}_\alpha \boldsymbol{D}_{\alpha\beta} \boldsymbol{\Sigma}_\beta \boldsymbol{D}_{\alpha\beta} \boldsymbol{\Sigma}_\alpha \boldsymbol{\alpha} / \|\boldsymbol{\alpha}\|^2 - \boldsymbol{\alpha}^T \boldsymbol{\Sigma}_\alpha \widehat{\boldsymbol{D}}_{\alpha\beta} \boldsymbol{\Sigma}_\beta \widehat{\boldsymbol{D}}_{\alpha\beta} \boldsymbol{\Sigma}_\alpha \boldsymbol{\alpha} / \|\boldsymbol{\alpha}\|^2| \\
&+ n_\beta \cdot \|\boldsymbol{\alpha}\|^2 \|\boldsymbol{\beta}\|^2 |\boldsymbol{\beta}^T \boldsymbol{\Sigma}_\beta \boldsymbol{D}_{\alpha\beta} \boldsymbol{\Sigma}_\alpha \boldsymbol{D}_{\alpha\beta} \boldsymbol{\Sigma}_\beta \boldsymbol{\beta} / \|\boldsymbol{\beta}\|^2 - \boldsymbol{\beta}^T \boldsymbol{\Sigma}_\beta \widehat{\boldsymbol{D}}_{\alpha\beta} \boldsymbol{\Sigma}_\alpha \widehat{\boldsymbol{D}}_{\alpha\beta} \boldsymbol{\Sigma}_\beta \boldsymbol{\beta} / \|\boldsymbol{\beta}\|^2| \\
&+ (n_\alpha + n_\beta) \cdot \|\boldsymbol{\alpha}\|^2 \|\boldsymbol{\beta}\|^2 |(\boldsymbol{\alpha}^T \boldsymbol{\Sigma}_\alpha \boldsymbol{D}_{\alpha\beta} \boldsymbol{\Sigma}_\beta \boldsymbol{\beta})^2 / \|\boldsymbol{\alpha}\|^2 \|\boldsymbol{\beta}\|^2 \\
&- (\boldsymbol{\alpha}^T \boldsymbol{\Sigma}_\alpha \widehat{\boldsymbol{D}}_{\alpha\beta} \boldsymbol{\Sigma}_\beta \boldsymbol{\beta})^2 / \|\boldsymbol{\alpha}\|^2 \|\boldsymbol{\beta}\|^2|.
\end{aligned}
$$

By inequality (46), under Conditions **??** and **??**, we have

$$f(\boldsymbol{\ell}_{ab}) \gtrsim \|\boldsymbol{\alpha}\|^2\|\boldsymbol{\beta}\|^2 \cdot \boldsymbol{\ell}_{ab}^T\boldsymbol{\ell}_{ab} + (n_\alpha + n_\beta)\|\boldsymbol{\alpha}\|^2\|\boldsymbol{\beta}\|^2\boldsymbol{\ell}_{ab,\min}^2$$
$$\gtrsim (p + n_\alpha + n_\beta)\|\boldsymbol{\alpha}\|^2\|\boldsymbol{\beta}\|^2.$$

The last inequality above follows from (51). Under Condition **??**, by Lemma S9, we have

$$p^{-1} \cdot |\mathrm{tr}(\boldsymbol{D}_{\alpha\beta}\boldsymbol{\Sigma}_\alpha\boldsymbol{D}_{\alpha\beta}\boldsymbol{\Sigma}_\beta) - \mathrm{tr}(\widehat{\boldsymbol{D}}_{\alpha\beta}\boldsymbol{\Sigma}_\alpha\widehat{\boldsymbol{D}}_{\alpha\beta}\boldsymbol{\Sigma}_\beta)| \xrightarrow{p} 0$$

as $n_{r\alpha}, n_{r\beta}$, and $p \to \infty$. Note that

$$\begin{aligned}
&|\boldsymbol{\alpha}^T\boldsymbol{\Sigma}_\alpha\boldsymbol{D}_{\alpha\beta}\boldsymbol{\Sigma}_\beta\boldsymbol{D}_{\alpha\beta}\boldsymbol{\Sigma}_\alpha\boldsymbol{\alpha} - \boldsymbol{\alpha}^T\boldsymbol{\Sigma}_\alpha\widehat{\boldsymbol{D}}_{\alpha\beta}\boldsymbol{\Sigma}_\beta\widehat{\boldsymbol{D}}_{\alpha\beta}\boldsymbol{\Sigma}_\alpha\boldsymbol{\alpha}|\\
=&|\boldsymbol{\alpha}^T(\boldsymbol{\Sigma}_\alpha(\boldsymbol{D}_{\alpha\beta} - \widehat{\boldsymbol{D}}_{\alpha\beta})\boldsymbol{\Sigma}_\beta\boldsymbol{D}_{\alpha\beta}\boldsymbol{\Sigma}_\alpha - \boldsymbol{\Sigma}_\alpha\widehat{\boldsymbol{D}}_{\alpha\beta}\boldsymbol{\Sigma}_\beta(\boldsymbol{D}_{\alpha\beta} - \widehat{\boldsymbol{D}}_{\alpha\beta})\boldsymbol{\Sigma}_\alpha)\boldsymbol{\alpha}|\\
\le&\|\boldsymbol{\alpha}\|_2^2(\|\boldsymbol{\Sigma}_\alpha(\boldsymbol{D}_{\alpha\beta} - \widehat{\boldsymbol{D}}_{\alpha\beta})\boldsymbol{\Sigma}_\beta\boldsymbol{D}_{\alpha\beta}\boldsymbol{\Sigma}_\alpha\|_2 + \|\boldsymbol{\Sigma}_\alpha\widehat{\boldsymbol{D}}_{\alpha\beta}\boldsymbol{\Sigma}_\beta(\boldsymbol{D}_{\alpha\beta} - \widehat{\boldsymbol{D}}_{\alpha\beta})\boldsymbol{\Sigma}_\alpha\|_2)\\
\lesssim&\|\boldsymbol{\alpha}\|_2^2(\max_{1\le i\le p}|\widehat{\ell}_{ab,i}(n_{r\alpha}, n_{r\beta}) - \ell_{ab,i}| + \|\widehat{\boldsymbol{D}}_{\alpha\beta}\boldsymbol{\Sigma}_\beta(\boldsymbol{D}_{\alpha\beta} - \widehat{\boldsymbol{D}}_{\alpha\beta})\|_2).
\end{aligned}$$

The last inequality above follows from Condition **??** and (54). By Lemma S7, we have

$$\max_{1\le i\le p}|\widehat{\ell}_{ab,i}(n_{r\alpha}, n_{r\beta}) - \ell_{ab,i}| \xrightarrow{p} 0$$

as $n_{r\alpha}$ and $n_{r\beta} \to \infty$. Since

$$\max_{1\le i\le p}|\widehat{\ell}_{ab,i}| \le \max_{1\le i\le p}|\widehat{\ell}_{ab,i}(n_{r\alpha}, n_{r\beta}) - \ell_{ab,i}| + \max_{1\le i\le p}|\ell_{ab,i}|,$$

we have $\max_{1\le i\le p}|\widehat{\ell}_{ab,i}| = O(1)$ by (54). It follows that

$$|\boldsymbol{\alpha}^T\boldsymbol{\Sigma}_\alpha\boldsymbol{D}_{\alpha\beta}\boldsymbol{\Sigma}_\beta\boldsymbol{D}_{\alpha\beta}\boldsymbol{\Sigma}_\alpha\boldsymbol{\alpha} - \boldsymbol{\alpha}^T\boldsymbol{\Sigma}_\alpha\widehat{\boldsymbol{D}}_{\alpha\beta}\boldsymbol{\Sigma}_\beta\widehat{\boldsymbol{D}}_{\alpha\beta}\boldsymbol{\Sigma}_\alpha\boldsymbol{\alpha}|/\|\boldsymbol{\alpha}\|_2^2 \xrightarrow{p} 0.$$

Similarly, we have

$$|\boldsymbol{\beta}^T\boldsymbol{\Sigma}_\beta\boldsymbol{D}_{\alpha\beta}\boldsymbol{\Sigma}_\alpha\boldsymbol{D}_{\alpha\beta}\boldsymbol{\Sigma}_\beta\boldsymbol{\beta} - \boldsymbol{\beta}^T\boldsymbol{\Sigma}_\beta\widehat{\boldsymbol{D}}_{\alpha\beta}\boldsymbol{\Sigma}_\alpha\widehat{\boldsymbol{D}}_{\alpha\beta}\boldsymbol{\Sigma}_\beta\boldsymbol{\beta}|/\|\boldsymbol{\beta}\|^2 \xrightarrow{p} 0.$$

Since

$$\begin{aligned}
&|(\boldsymbol{\alpha}^T\boldsymbol{\Sigma}_\alpha\boldsymbol{D}_{\alpha\beta}\boldsymbol{\Sigma}_\beta\boldsymbol{\beta})^2 - (\boldsymbol{\alpha}^T\boldsymbol{\Sigma}_\alpha\widehat{\boldsymbol{D}}_{\alpha\beta}\boldsymbol{\Sigma}_\beta\boldsymbol{\beta})^2|\\
=&|(\boldsymbol{\alpha}^T\boldsymbol{\Sigma}_\alpha(\boldsymbol{D}_{\alpha\beta} - \widehat{\boldsymbol{D}}_{\alpha\beta} + \widehat{\boldsymbol{D}}_{\alpha\beta})\boldsymbol{\Sigma}_\beta\boldsymbol{\beta})^2 - (\boldsymbol{\alpha}^T\boldsymbol{\Sigma}_\alpha\widehat{\boldsymbol{D}}_{\alpha\beta}\boldsymbol{\Sigma}_\beta\boldsymbol{\beta})^2|\\
\lesssim&|(\boldsymbol{\alpha}^T\boldsymbol{\Sigma}_\alpha(\boldsymbol{D}_{\alpha\beta} - \widehat{\boldsymbol{D}}_{\alpha\beta})\boldsymbol{\Sigma}_\beta\boldsymbol{\beta})^2| + |\boldsymbol{\alpha}^T\boldsymbol{\Sigma}_\alpha(\boldsymbol{D}_{\alpha\beta} - \widehat{\boldsymbol{D}}_{\alpha\beta})\boldsymbol{\Sigma}_\beta\boldsymbol{\beta}||\boldsymbol{\alpha}^T\boldsymbol{\Sigma}_\alpha\widehat{\boldsymbol{D}}_{\alpha\beta}\boldsymbol{\Sigma}_\beta\boldsymbol{\beta}|,
\end{aligned}$$

we have

$$|(\boldsymbol{\alpha}^T\boldsymbol{\Sigma}_\alpha\boldsymbol{D}_{\alpha\beta}\boldsymbol{\Sigma}_\beta\boldsymbol{\beta})^2 - (\boldsymbol{\alpha}^T\boldsymbol{\Sigma}_\alpha\widehat{\boldsymbol{D}}_{\alpha\beta}\boldsymbol{\Sigma}_\beta\boldsymbol{\beta})^2|/(\|\boldsymbol{\alpha}\|^2\|\boldsymbol{\beta}\|^2) \xrightarrow{p} 0.$$

Thus, we have

$$\frac{f(\widehat{\boldsymbol{\ell}}_{ab})}{f(\boldsymbol{\ell}_{ab})} \xrightarrow{p} 1$$

as $n_{r\alpha}, n_{r\beta}$, and $p \to \infty$. Since

$$\frac{\widehat{\boldsymbol{\ell}}_{ab}^T\widehat{\boldsymbol{\ell}}_{ab}}{\boldsymbol{\ell}_{ab}^T\boldsymbol{\ell}_{ab}} - 1 = \frac{\widehat{\boldsymbol{\ell}}_{ab}^T\widehat{\boldsymbol{\ell}}_{ab}/p - \boldsymbol{\ell}_{ab}^T\boldsymbol{\ell}_{ab}/p}{\boldsymbol{\ell}_{ab}^T\boldsymbol{\ell}_{ab}/p},$$

by Lemma S9 and (51), we have

$$\frac{\widehat{\boldsymbol{\ell}}_{ab}^T \widehat{\boldsymbol{\ell}}_{ab}}{\boldsymbol{\ell}_{ab}^T \boldsymbol{\ell}_{ab}} \xrightarrow{p} 1.$$

Thus, by (57) and (58), we have

$$\frac{\zeta_{\alpha\beta}(\widehat{\boldsymbol{\ell}}_{ab})}{\zeta_{\alpha\beta}(\boldsymbol{\ell}_{ab})} \xrightarrow{p} 1$$

and

$$\frac{(\widehat{\boldsymbol{\ell}}_{ab}^T \widehat{\boldsymbol{\ell}}_{ab})^{-1} \widehat{\boldsymbol{\ell}}_{ab}^T (\widehat{\boldsymbol{w}}_{ab} - \boldsymbol{w}_{ab})}{\zeta_{\alpha\beta}(\boldsymbol{\ell}_{ab})} \xrightarrow{d} N(0,1) \tag{60}$$

as $n_{r\alpha}, n_{r\beta}$, and $p \to \infty$. □

S7.4. *Proof of Theorem S2.*

PROOF. By (48), (51), and (54), we have

$$\zeta_{\alpha\beta}^2(\boldsymbol{\ell}_{ab}) \lesssim \frac{\|\boldsymbol{\alpha}\|^2\|\boldsymbol{\beta}\|^2}{pn_\alpha n_\beta} + \frac{\|\boldsymbol{\alpha}\|^2\|\boldsymbol{\beta}\|^2}{p^2 n_\beta} + \frac{\|\boldsymbol{\alpha}\|^2\|\boldsymbol{\beta}\|^2}{p^2 n_\alpha}.$$

By Conditions **??** and **??**, $\zeta_{\alpha\beta}^2(\boldsymbol{\ell}_{ab}) \to 0$ as $p \to \infty$. Note that

$$\begin{aligned}\widehat{\sigma}_{\alpha\beta} - \sigma_{\alpha\beta} =& (\widehat{\boldsymbol{\ell}}_{ab}^T \widehat{\boldsymbol{\ell}}_{ab})^{-1} \widehat{\boldsymbol{\ell}}_{ab}^T (\widehat{\boldsymbol{w}}_{ab} - \boldsymbol{w}_{ab}) + \{(\widehat{\boldsymbol{\ell}}_{ab}^T \widehat{\boldsymbol{\ell}}_{ab})^{-1} \widehat{\boldsymbol{\ell}}_{ab}^T - (\boldsymbol{\ell}_{ab}^T \boldsymbol{\ell}_{ab})^{-1} \boldsymbol{\ell}_{ab}^T\} \boldsymbol{w}_{ab} \\ &+ (\boldsymbol{\ell}_{ab}^T \boldsymbol{\ell}_{ab})^{-1} \boldsymbol{\ell}_{ab}^T \boldsymbol{\varepsilon}_{ab}.\end{aligned}$$

By Condition **??** and (51), we have $(\boldsymbol{\ell}_{ab}^T \boldsymbol{\ell}_{ab})^{-1} \boldsymbol{\ell}_{ab}^T \boldsymbol{\varepsilon}_{ab} \to 0$. Note that

$$\begin{aligned}&\{(\widehat{\boldsymbol{\ell}}_{ab}^T \widehat{\boldsymbol{\ell}}_{ab})^{-1} \widehat{\boldsymbol{\ell}}_{ab}^T - (\boldsymbol{\ell}_{ab}^T \boldsymbol{\ell}_{ab})^{-1} \boldsymbol{\ell}_{ab}^T\} \boldsymbol{w}_{ab} \\ =& \left\{(\widehat{\boldsymbol{\ell}}_{ab}^T \widehat{\boldsymbol{\ell}}_{ab} / \boldsymbol{\ell}_{ab}^T \boldsymbol{\ell}_{ab})^{-1} - 1\right\} \frac{(\widehat{\boldsymbol{\ell}}_{ab} - \boldsymbol{\ell}_{ab})^T \boldsymbol{w}_{ab}}{\boldsymbol{\ell}_{ab}^T \boldsymbol{\ell}_{ab}} + \left\{(\widehat{\boldsymbol{\ell}}_{ab}^T \widehat{\boldsymbol{\ell}}_{ab} / \boldsymbol{\ell}_{ab}^T \boldsymbol{\ell}_{ab})^{-1} - 1\right\} \frac{\boldsymbol{\ell}_{ab}^T \boldsymbol{w}_{ab}}{\boldsymbol{\ell}_{ab}^T \boldsymbol{\ell}_{ab}} \\ &+ \frac{(\widehat{\boldsymbol{\ell}}_{ab} - \boldsymbol{\ell}_{ab})^T \boldsymbol{w}_{ab}}{\boldsymbol{\ell}_{ab}^T \boldsymbol{\ell}_{ab}}.\end{aligned}$$

By Condition 19 and (53), we have

$$\frac{(\widehat{\boldsymbol{\ell}}_{ab} - \boldsymbol{\ell}_{ab})^T \boldsymbol{w}_{ab}}{\boldsymbol{\ell}_{ab}^T \boldsymbol{\ell}_{ab}} \xrightarrow{p} 0.$$

By Lemma **??** and (51), we have

$$(\widehat{\boldsymbol{\ell}}_{ab}^T \widehat{\boldsymbol{\ell}}_{ab} - \boldsymbol{\ell}_{ab}^T \boldsymbol{\ell}_{ab}) / \boldsymbol{\ell}_{ab}^T \boldsymbol{\ell}_{ab} \xrightarrow{p} 0.$$

It follows that

$$\{(\widehat{\boldsymbol{\ell}}_{ab}^T \widehat{\boldsymbol{\ell}}_{ab})^{-1} \widehat{\boldsymbol{\ell}}_{ab}^T - (\boldsymbol{\ell}_{ab}^T \boldsymbol{\ell}_{ab})^{-1} \boldsymbol{\ell}_{ab}^T\} \boldsymbol{w}_{ab} \xrightarrow{p} 0.$$

Under Condition 20 (for Lemma S7), by the convergence in (60) and $\zeta_{\alpha\beta}^2(\boldsymbol{\ell}_{ab}) \to 0$, we have

$$(\widehat{\boldsymbol{\ell}}_{ab}^T \widehat{\boldsymbol{\ell}}_{ab})^{-1} \widehat{\boldsymbol{\ell}}_{ab}^T (\widehat{\boldsymbol{w}}_{ab} - \boldsymbol{w}_{ab}) \xrightarrow{p} 0.$$

□

## S8. Supplementary figures and tables.

| Method | Proposed (LDSC) | [11] $\hat{\tau}^2(\widetilde{\Sigma})$ | [11] $\tilde{\tau}^2$ | [45] |
|---|---|---|---|---|
| Allow genetic covariance estimation | Yes | No | No | Yes |
| Require covariance matrix estimator | No | Yes | No | Yes |
| Require precision matrix estimator | No | No | No | Yes |
| Require large reference panel | No | — | — | Yes |
| Allow cross-ancestry estimation | Yes | No | No | No |

SUPPLEMENTARY TABLE 1. *Overview of method comparison. We compare the LDSC estimators (and their cross-ancestry extension) analyzed in our paper with the estimators proposed in [11] and [45].*

| | Phenotye_ID | 1MB-Window | 2MB-Window | Independent | Pooled subjects |
|---|---|---|---|---|---|
| 1 | BMI | 1.04 (0.04) | 1.04 (0.04) | 1.06 (0.04) | 0.91 (0.04) |
| 2 | BW | 1.07 (0.03) | 1.07 (0.03) | 1.09 (0.04) | 0.93 (0.03) |
| 3 | DBP | 1.00 (0.08) | 1.00 (0.08) | 1.02 (0.09) | 0.80 (0.07) |
| 4 | Eosino | 1.40 (0.22) | 1.39 (0.22) | 1.39 (0.22) | 1.20 (0.15) |
| 5 | Hb | 1.00 (0.15) | 1.00 (0.15) | 1.03 (0.17) | 0.89 (0.14) |
| 6 | Height | 1.10 (0.04) | 1.10 (0.04) | 1.10 (0.04) | 0.93 (0.03) |
| 7 | Ht | 0.99 (0.11) | 0.99 (0.11) | 1.01 (0.12) | 0.92 (0.11) |
| 8 | Lym | 1.30 (0.18) | 1.30 (0.19) | 1.26 (0.19) | 1.14 (0.14) |
| 9 | MCHC | 1.10 (0.18) | 1.12 (0.18) | 1.08 (0.19) | 0.87 (0.16) |
| 10 | MCH | 1.13 (0.15) | 1.13 (0.15) | 1.15 (0.17) | 1.04 (0.15) |
| 11 | MCV | 1.15 (0.14) | 1.14 (0.14) | 1.17 (0.16) | 1.06 (0.18) |
| 12 | Mono | 1.32 (0.19) | 1.30 (0.19) | 1.40 (0.22) | 1.18 (0.18) |
| 13 | Neutro | 1.31 (0.13) | 1.32 (0.13) | 1.34 (0.17) | 1.11 (0.10) |
| 14 | Plt | 1.14 (0.10) | 1.14 (0.10) | 1.12 (0.11) | 0.99 (0.08) |
| 15 | RBC | 1.13 (0.07) | 1.12 (0.07) | 1.20 (0.09) | 1.04 (0.06) |
| 16 | WBC | 0.96 (0.11) | 0.97 (0.11) | 0.97 (0.13) | 0.86 (0.10) |
| 17 | Allergic_Rhinitis | 0.44 (0.12) | 0.45 (0.12) | 0.44 (0.12) | 0.43 (0.11) |
| 18 | Angina | 0.91 (0.14) | 0.92 (0.14) | 0.86 (0.17) | 0.69 (0.14) |
| 19 | Asthma | 0.52 (0.07) | 0.51 (0.07) | 0.52 (0.07) | 0.40 (0.07) |
| 20 | BrC | 1.79 (0.32) | 1.78 (0.32) | 1.73 (0.34) | 1.65 (0.32) |
| 21 | Cataract | 0.77 (0.25) | 0.78 (0.25) | 0.77 (0.27) | 0.73 (0.34) |
| 22 | CHF | 0.56 (0.37) | 0.58 (0.37) | 0.48 (0.52) | 0.17 (0.37) |
| 23 | Cholelithiasis | 0.97 (0.17) | 0.98 (0.17) | 1.06 (0.23) | 0.92 (0.17) |
| 24 | Gastric_Ulcer | 0.42 (0.70) | 0.42 (0.69) | 1.31 (1.57) | 0.79 (0.98) |
| 25 | Glaucoma | 0.51 (0.12) | 0.53 (0.12) | 0.52 (0.13) | 0.43 (0.14) |
| 26 | IS | 1.13 (0.34) | 1.15 (0.34) | 1.09 (0.34) | 0.89 (0.24) |
| 27 | MI | 1.02 (0.14) | 1.02 (0.14) | 1.08 (0.15) | 0.91 (0.13) |
| 28 | Pneumonia | 0.76 (0.92) | 0.68 (0.89) | 0.38 (0.68) | 0.26 (0.77) |
| 29 | PrC | 1.37 (0.31) | 1.35 (0.31) | 1.48 (0.42) | 1.07 (0.35) |
| 30 | RA | 0.85 (0.45) | 0.85 (0.44) | 0.85 (0.53) | 0.88 (0.36) |
| 31 | SAP | 1.10 (0.19) | 1.11 (0.19) | 1.20 (0.23) | 0.88 (0.18) |
| 32 | T2D | 0.77 (0.17) | 0.76 (0.17) | 0.69 (0.15) | 0.65 (0.16) |
| 33 | UAP | 0.88 (0.28) | 0.89 (0.28) | 0.85 (0.28) | 0.95 (0.29) |
| 34 | Urticaria | 1.11 (1.21) | 1.07 (1.18) | 1.50 (2.53) | 1.27 (1.24) |

SUPPLEMENTARY TABLE 2. *Cross-ancestry genetic correlation between 34 pairs of matched phenotypes in Biobank Japan and UK Biobank. The descriptions of the phenotype IDs can be found at https://pheweb.jp/downloads. We show the estimates and associated standard errors from four methods used in our simulation analysis: "1MB-Window", "2MB-Window", "Independent", and "Pooled subjects". An visualization of the estimates can be found in Supplementary Figure 15.*

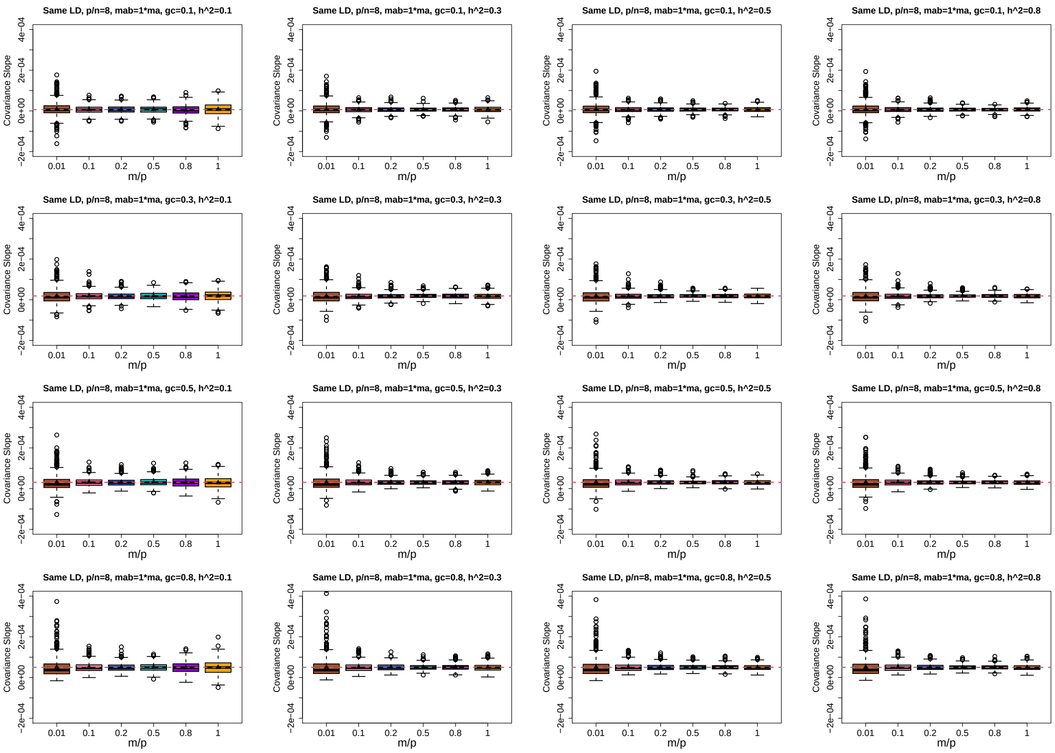


SUPPLEMENTARY FIG. 1. *Bivariate LDSC estimator $\widehat{\sigma}_{\alpha\beta}$ across different genetic correlation (gc), signal sparsity ($m/p$), and heritability ($h^2$) settings. We simulate the data with $n_\alpha = n_\beta = 2{,}000$, $p = 16{,}000$, and $m_\alpha = m_\beta = m_{\alpha\beta}$. The $\mathbf{\Sigma}_\alpha = \mathbf{\Sigma}_\beta$ is estimated from 1KG-EUR subjects. The horizontal line represents the true value $\sigma_{\alpha\beta}$.*

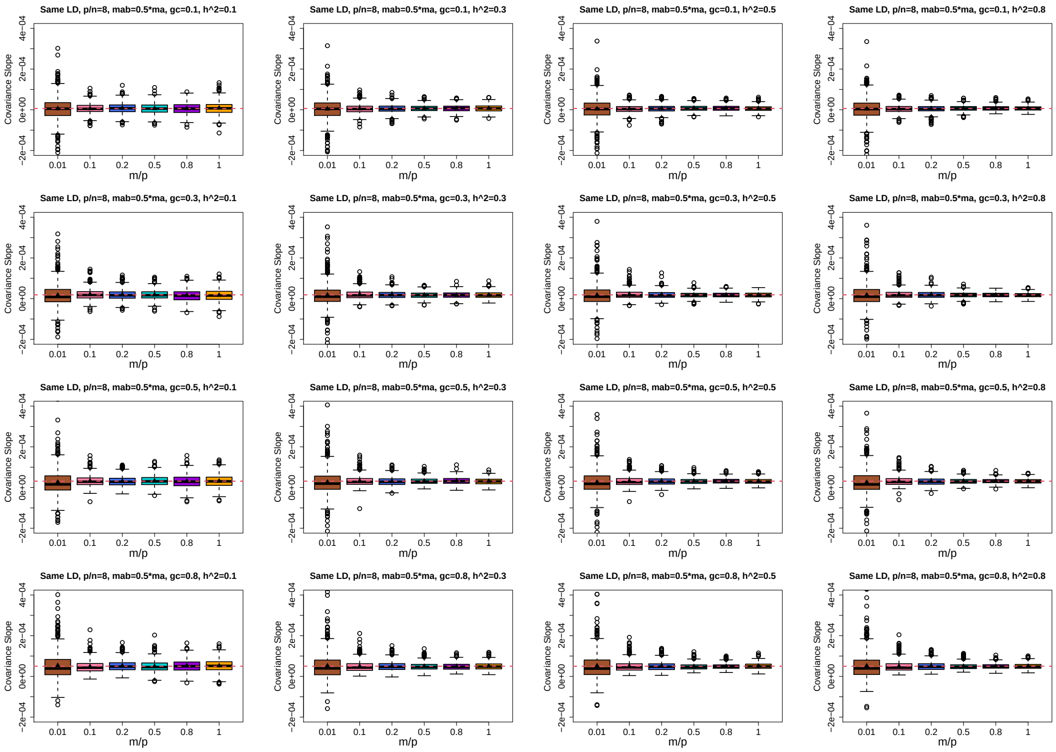


SUPPLEMENTARY FIG. 2. *Bivariate LDSC estimator $\widehat{\sigma}_{\alpha\beta}$ across different genetic correlation (gc), signal sparsity ($m/p$), and heritability settings ($h^2$). We simulate the data with $n_\alpha = n_\beta = 2{,}000$, $p = 16{,}000$, and $m_{\alpha\beta}/m_\alpha = m_{\alpha\beta}/m_\beta = 0.5$. The $\mathbf{\Sigma}_\alpha = \mathbf{\Sigma}_\beta$ is estimated from 1KG-EUR subjects. The horizontal line represents the true value $\sigma_{\alpha\beta}$.*

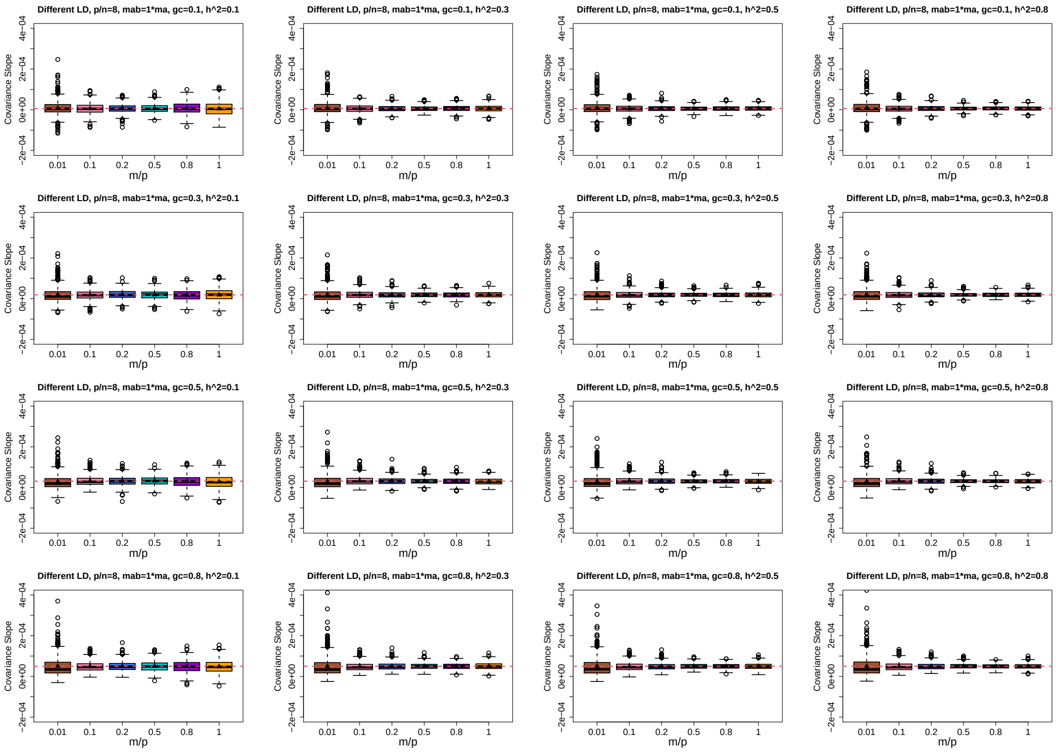


SUPPLEMENTARY FIG. 3. *Bivariate LDSC estimator $\widehat{\sigma}_{\alpha\beta}$ across different genetic correlation (gc), signal sparsity ($m/p$), and heritability ($h^2$) settings. We simulate the data with $n_\alpha = n_\beta = 2{,}000$, $p = 16{,}000$, and $m_\alpha = m_\beta = m_{\alpha\beta}$. The $\mathbf{\Sigma}_\alpha$ and $\mathbf{\Sigma}_\beta$ are estimated from 1KG-EUR and 1KG-EAS subjects, respectively. The horizontal line represents the true value $\sigma_{\alpha\beta}$.*

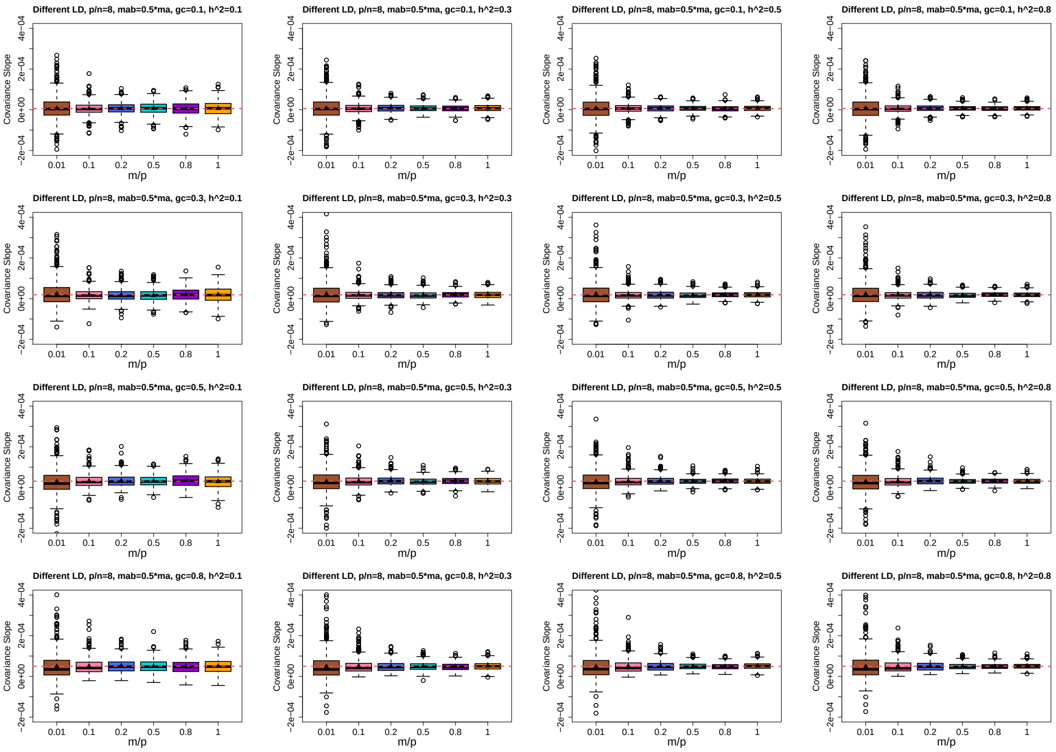


SUPPLEMENTARY FIG. 4. *Bivariate LDSC estimator $\widehat{\sigma}_{\alpha\beta}$ across different genetic correlation (gc), signal sparsity ($m/p$), and heritability settings ($h^2$). We simulate the data with $n_\alpha = n_\beta = 2{,}000$, $p = 16{,}000$, and $m_{\alpha\beta}/m_\alpha = m_{\alpha\beta}/m_\beta = 0.5$. The $\mathbf{\Sigma}_\alpha$ and $\mathbf{\Sigma}_\beta$ are estimated from 1KG-EUR and 1KG-EAS subjects, respectively. The horizontal line represents the true value $\sigma_{\alpha\beta}$.*

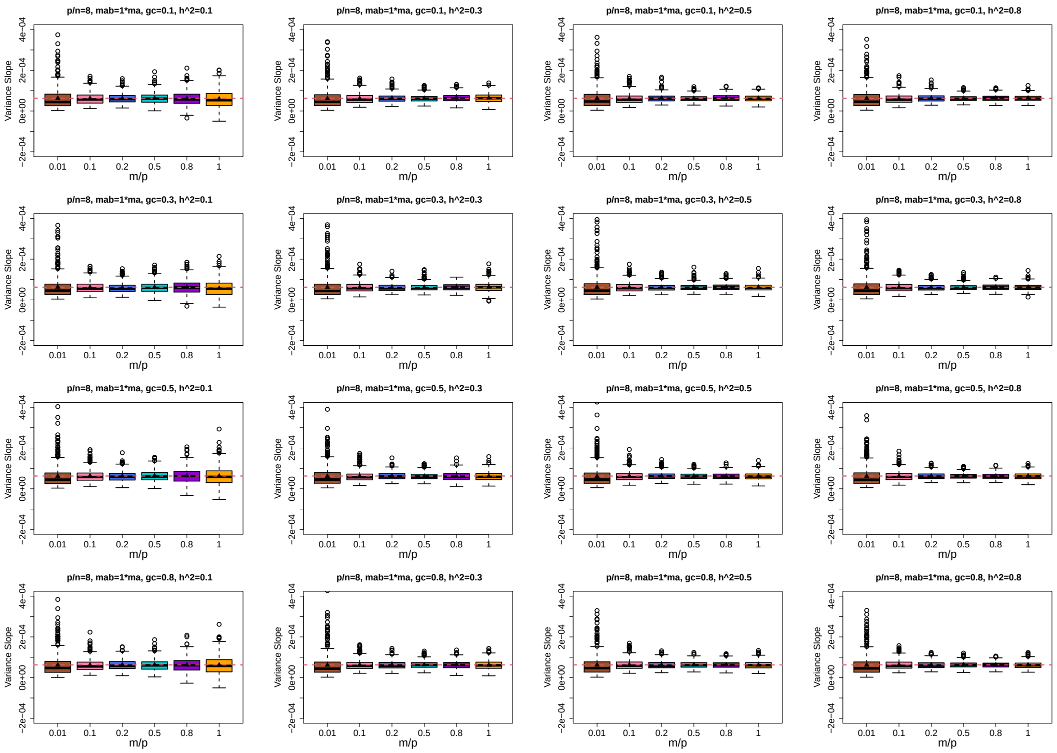


SUPPLEMENTARY FIG. 5. *Univariate LDSC estimator $\widehat{\sigma}^2_\alpha$ across different genetic correlation (gc), signal sparsity ($m/p$), and heritability ($h^2$) settings. We simulate the data with $n_\alpha = n_\beta = 2{,}000$, $p = 16{,}000$, and $m_\alpha = m_\beta = m_{\alpha\beta}$. The $\mathbf{\Sigma}_\alpha$ is estimated from 1KG-EUR subjects. The horizontal line represents the true value $\sigma^2_\alpha$.*

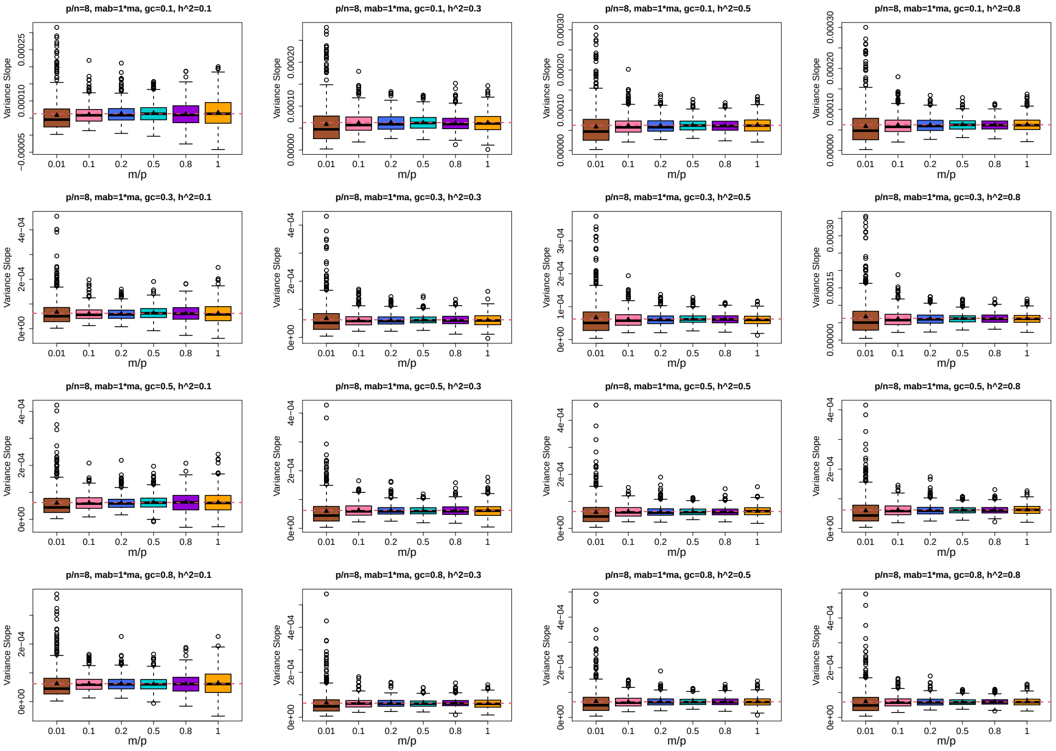


SUPPLEMENTARY FIG. 6. *Univariate LDSC estimator* $\widehat{\sigma}^2_{\beta}$ *across different genetic correlation (gc), signal sparsity (m/p), and heritability settings (*$h^2$*). We simulate the data with* $n_{\alpha} = n_{\beta} = 2{,}000$*,* $p = 16{,}000$*, and* $m_{\alpha\beta}/m_{\alpha} = m_{\alpha\beta}/m_{\beta} = 0.5$*. The* $\mathbf{\Sigma}_{\beta}$ *is estimated from 1KG-EUR subjects. The horizontal line represents the true value* $\sigma^2_{\beta}$*.*

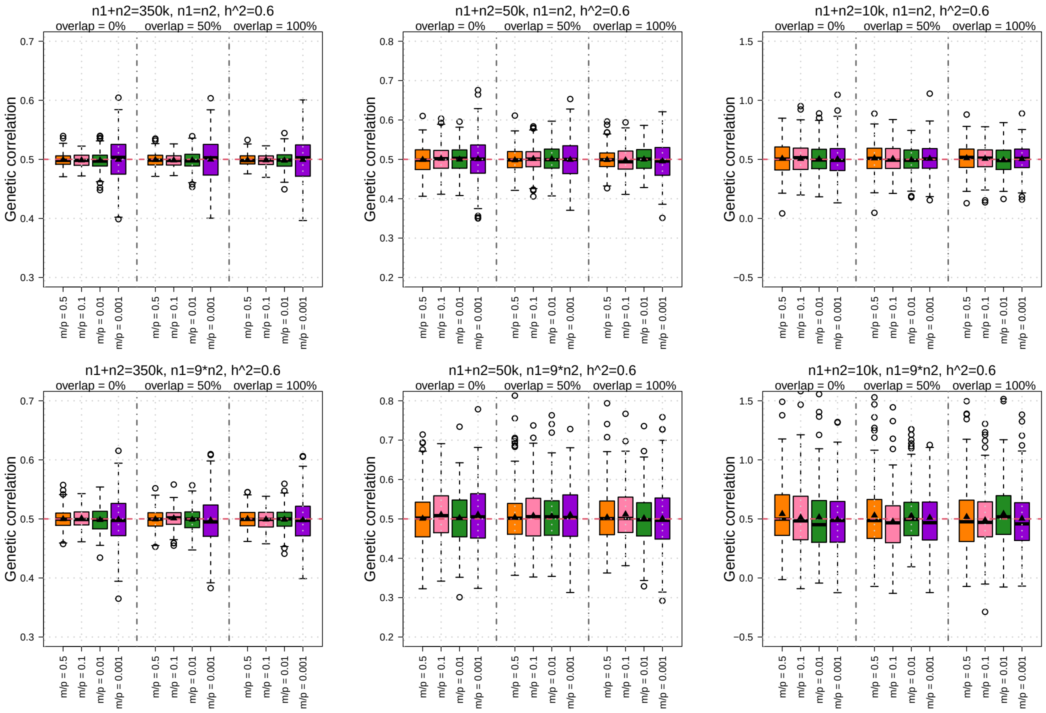


SUPPLEMENTARY FIG. 7. *Bivariate LDSC estimator across different sample sizes ($n_\alpha$ and $n_\beta$), signal sparsity ($m/p$), and sample overlaps in the UK Biobank data simulation. We report the genetic correlation, which is closely related to both genetic covariance and variance. We set the heritability $h^2_\alpha = h^2_\beta = 0.6$. We simulate the data with $n_\alpha + n_\beta = 350{,}000$, $50{,}000$, or $10{,}000$. We have $n_\alpha = n_\beta$ in the top panels and $n_\alpha = 9 \times n_\beta$ in the bottom panels. In each panel, we consider three cases of sample overlaps: 1) no sample overlap ($0\%$), 2) half of the $n_\beta$ samples overlap with the $n_\alpha$ samples ($50\%$), and 3) all the $n_\beta$ samples overlap with the $n_\alpha$ samples ($100\%$). The horizontal line represents the true genetic correlation $0.5$.*

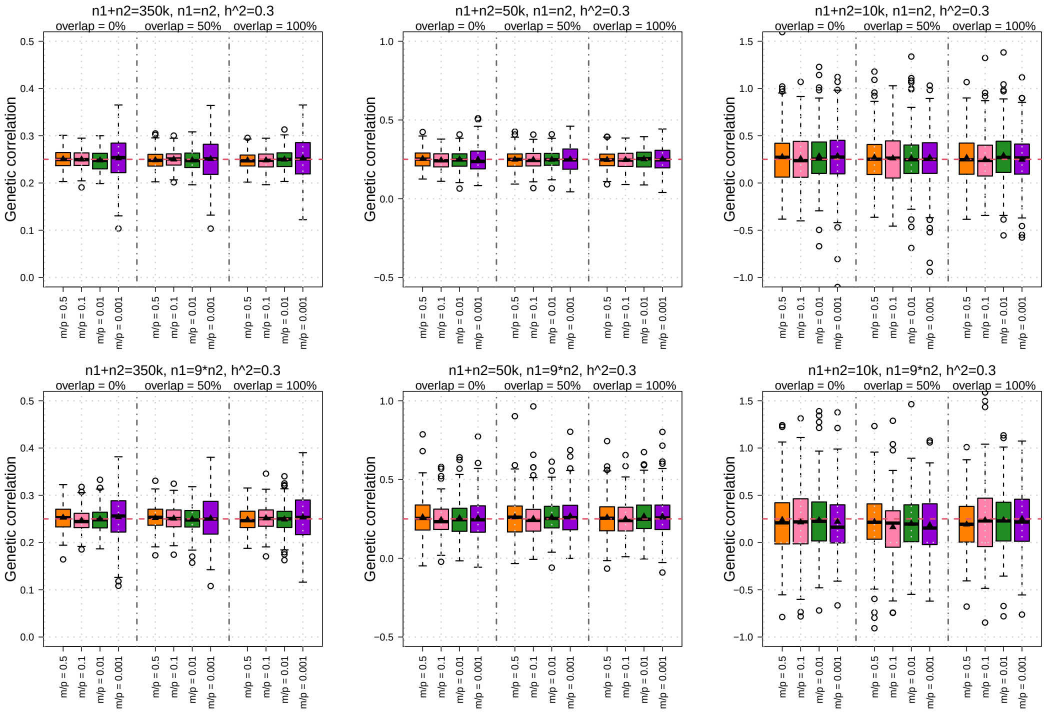


SUPPLEMENTARY FIG. 8. *Bivariate LDSC estimator across different sample sizes ($n_\alpha$ and $n_\beta$), signal sparsity ($m/p$), and sample overlaps in the UK Biobank data simulation. We report the genetic correlation, which is closely related to both genetic covariance and variance. We set the heritability $h^2_\alpha = h^2_\beta = 0.3$. We simulate the data with $n_\alpha + n_\beta = 350{,}000$, $50{,}000$, or $10{,}000$. We have $n_\alpha = n_\beta$ in the top panels and $n_\alpha = 9 \times n_\beta$ in the bottom panels. In each panel, we consider three cases of sample overlaps: 1) no sample overlap ($0\%$), 2) half of the $n_\beta$ samples overlap with the $n_\alpha$ samples ($50\%$), and 3) all the $n_\beta$ samples overlap with the $n_\alpha$ samples ($100\%$). The horizontal line represents the true genetic correlation $0.25$.*

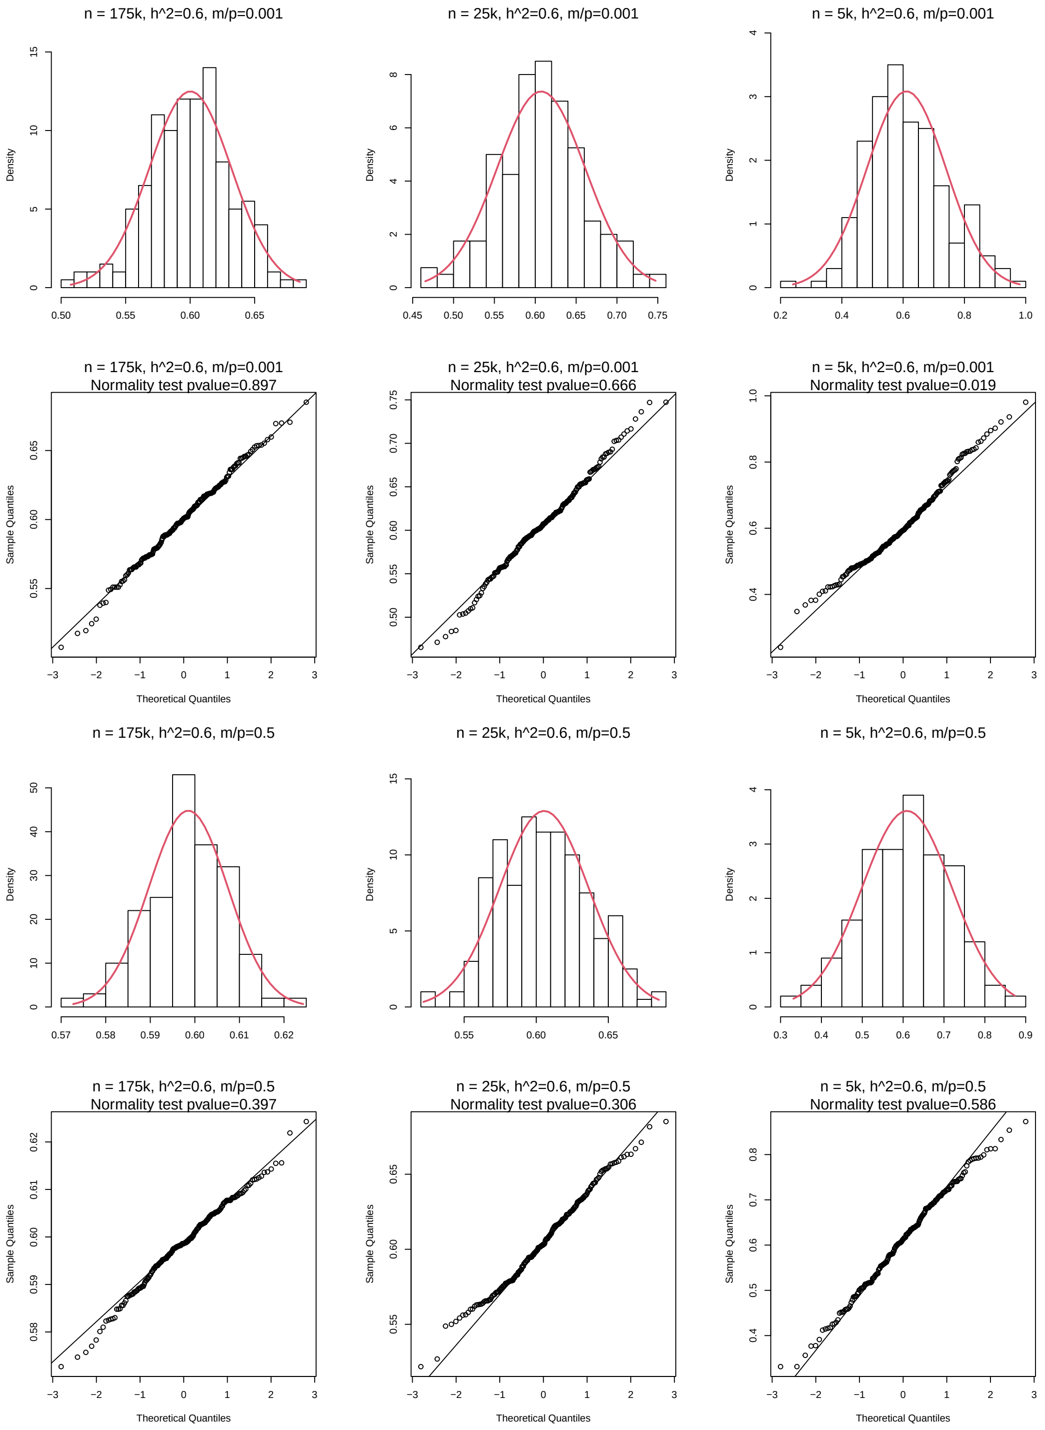


SUPPLEMENTARY FIG. 9. *Histogram and quantile-quantile plot of univariate LDSC estimator across different sample sizes ($n_\alpha$) in the UK Biobank data simulation. We set the heritability $h_\alpha^2 = 0.6$ and sparsity $m/p = 0.001$ or $0.5$. We simulate the data with $n_\alpha = 175{,}000$, $25{,}000$, or $5{,}000$. The Shapiro-Wilk method is used to test whether the distribution of the estimates is significantly different from the normal distribution.*

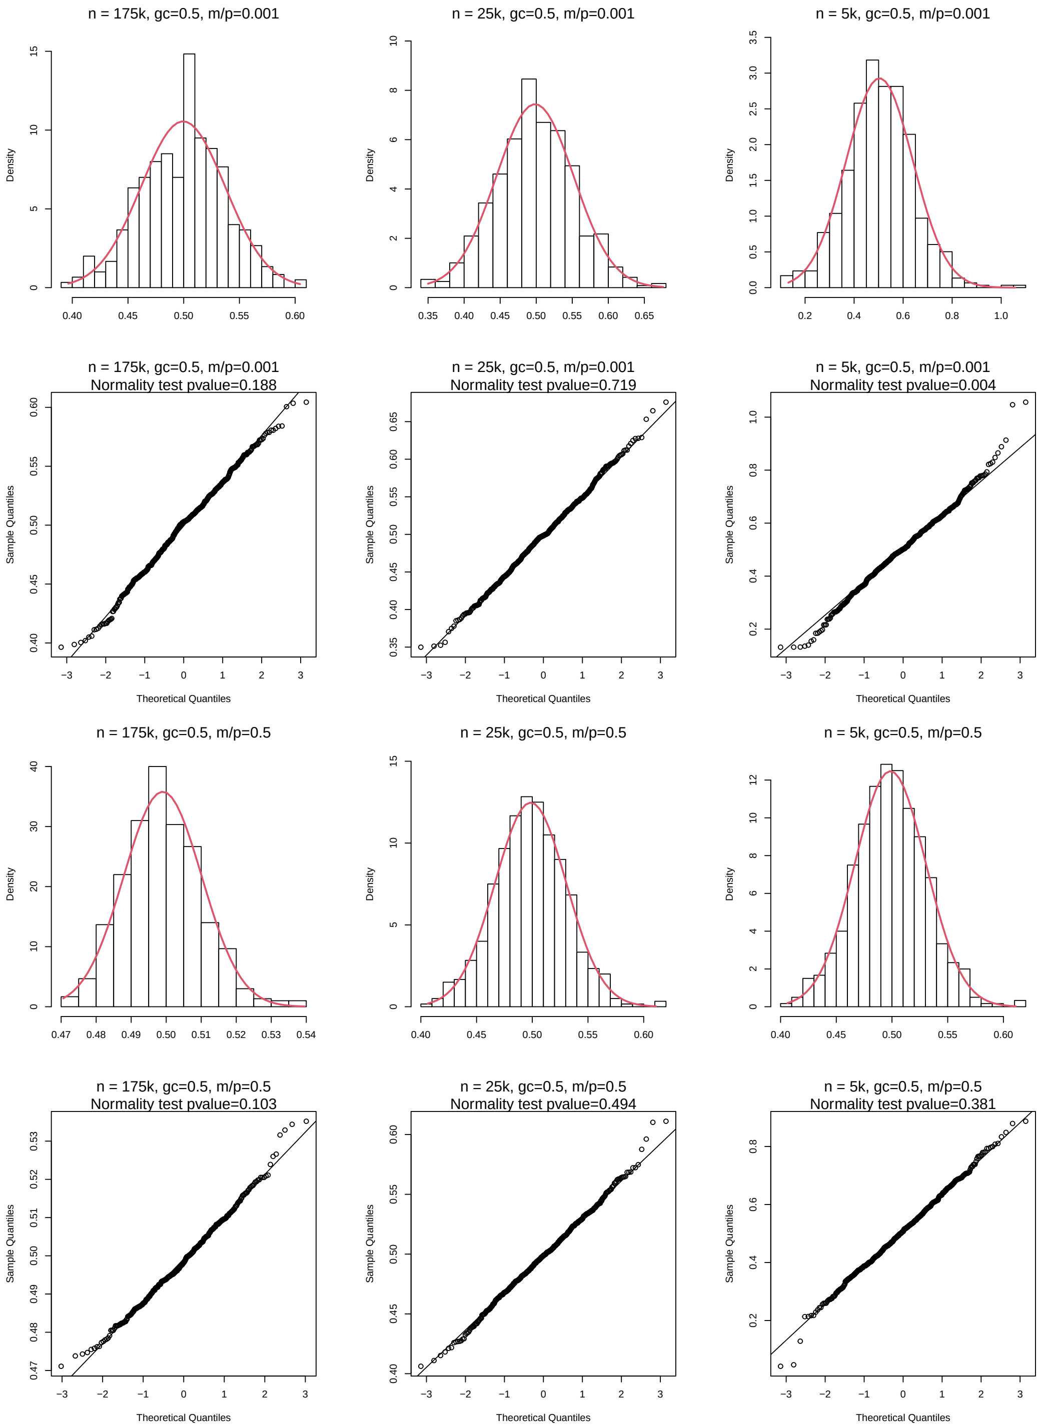


SUPPLEMENTARY FIG. 10. *Histogram and quantile-quantile plot of bivariate LDSC estimator across different sample sizes ($n_\alpha$ and $n_\beta$) in the UK Biobank data simulation. We report the genetic correlation, which is closely related to both genetic covariance and variance. We set the heritability $h^2_\alpha = 0.6$ and sparsity $m/p = 0.001$ or* $0.5$. *We simulate the data with $n_\alpha + n_\beta = 350{,}000$, $50{,}000$, or $10{,}000$ and we have $n_\alpha = n_\beta$. The Shapiro-Wilk method is used to test whether the distribution of the estimates is significantly different from the normal distribution.*

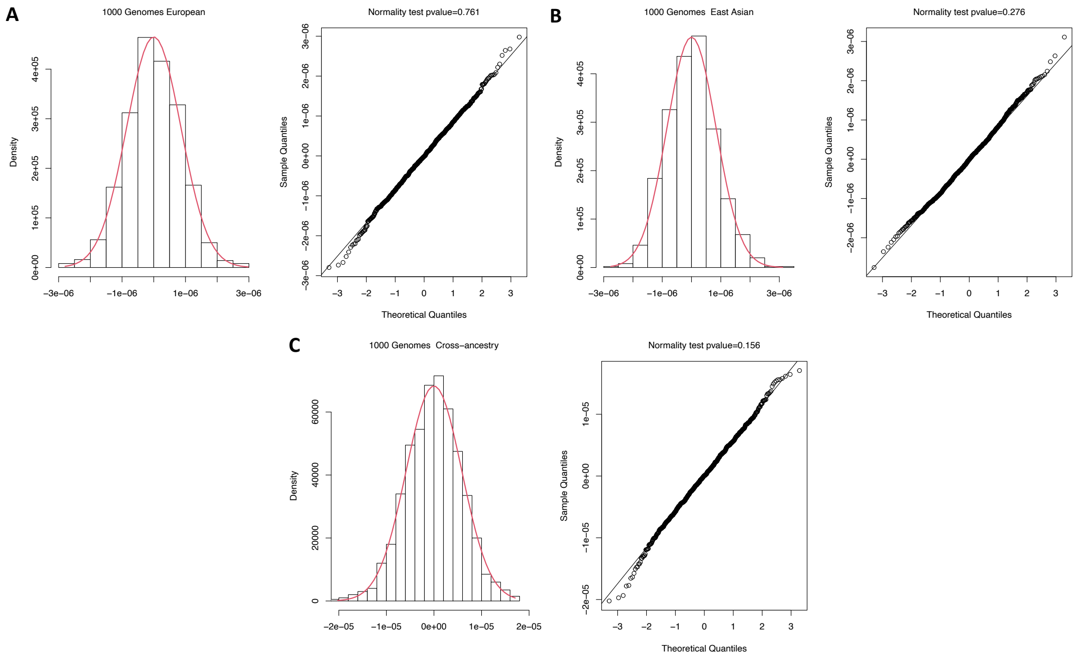


SUPPLEMENTARY FIG. 11. *Histogram and quantile-quantile plot of inner products of estimated LD scores in the 1KG project. Panel A:* $\widehat{\boldsymbol{\ell}}_a^T\widehat{\boldsymbol{\ell}}_a$ *using 1KG-EUR. Panel B:* $\widehat{\boldsymbol{\ell}}_b^T\widehat{\boldsymbol{\ell}}_b$ *using 1KG-EAS. Panel C:* $\widehat{\boldsymbol{\ell}}_{ab}^T\widehat{\boldsymbol{\ell}}_{ab}$ *using 1KG-EUR and 1KG-EUR. We obtain the empirical distribution using* $1{,}000$ *bootstrap samples. The Shapiro-Wilk method is used to test whether the distribution of the estimates is significantly different from the normal distribution.*

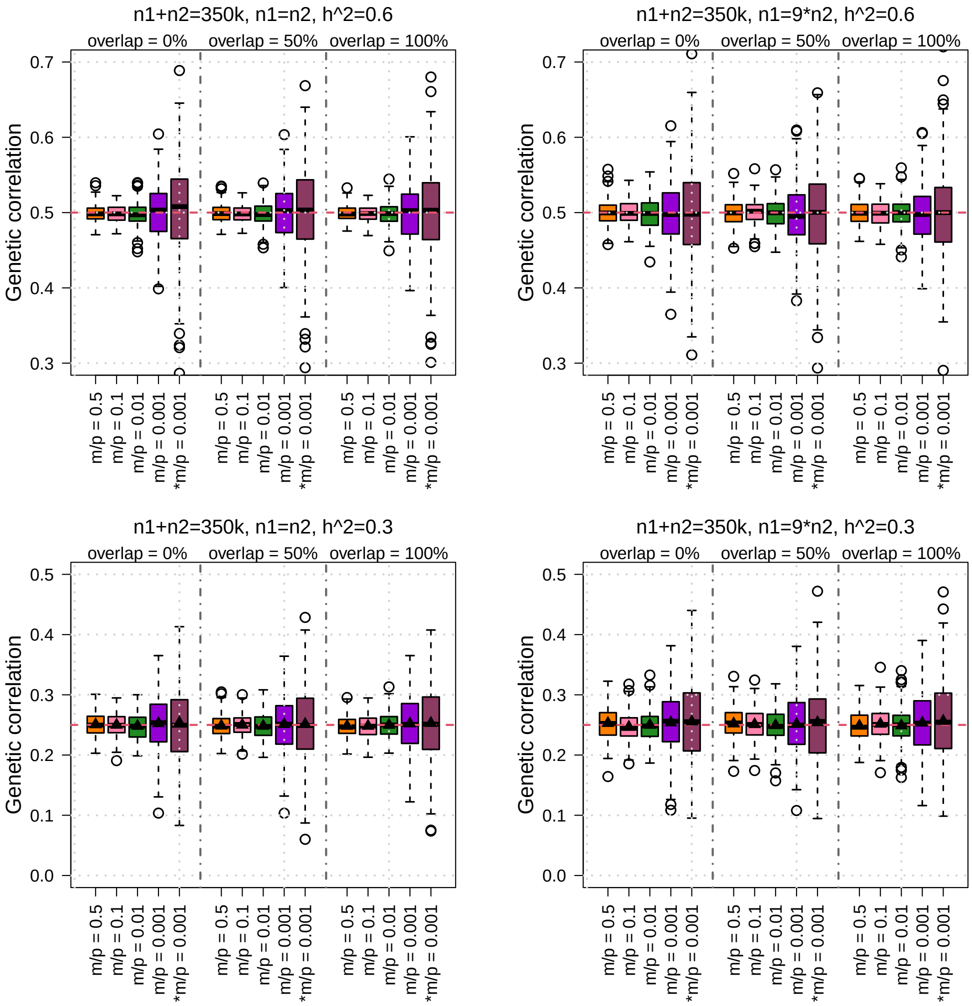


SUPPLEMENTARY FIG. 12. *Bivariate LDSC estimator across different signal sparsity* $(m/p)$ *and sample overlaps. We set the heritability* $h_\alpha^2 = h_\beta^2 = 0.6$ *and genetic correlation* $\varphi_{\alpha\beta} = 0.5$ *in the top panels and* $h_\alpha^2 = h_\beta^2 = 0.3$ *and* $\varphi_{\alpha\beta} = 0.25$ *in the bottom panels. We simulate the data with* $n_\alpha = n_\beta = 175{,}000$. *In each panel, we consider three cases of sample overlaps: 1) no sample overlap* $(0\%)$, *2) half sample overlap* $(50\%)$, *and 3) all samples overlap* $(100\%)$. *In each panel, the last column with an asterisk label indicates the version of LDSC estimates obtained using only the genetic variants known to have a nonzero genetic effect. The horizontal line represents the true genetic correlations.*

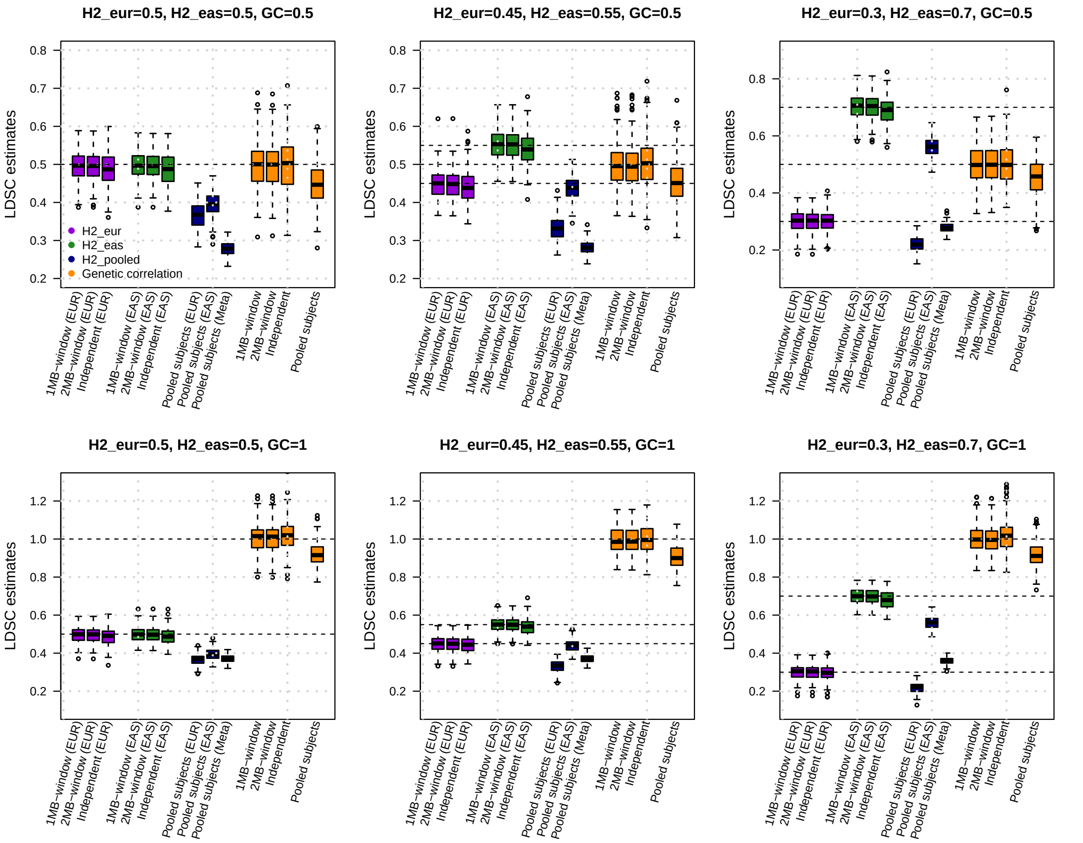


SUPPLEMENTARY FIG. 13. *LDSC estimators across different heritability and genetic correlation levels in HAPNEST simulation analysis. We set the heritability* $h^2_{eur} = h^2_{eas} = 0.5$ *in the left panels, and make them different in the middle* ($h^2_{eur} = 0.45$, $h^2_{eas} = 0.55$) *and right panels* ($h^2_{eur} = 0.3$, $h^2_{eas} = 0.7$)*. We simulate the data with* $n_\alpha = n_\beta = 16{,}800$ *and the proportion of causal variants being* $3\%$*. The genetic correlation (GC) is* $0.5$ *and* $1$ *in the upper and bottom panels, respectively. In each panel, we show the estimates of heritability and genetic correlation in different colors. The horizontal line represents the true heritability and genetic correlation values.*

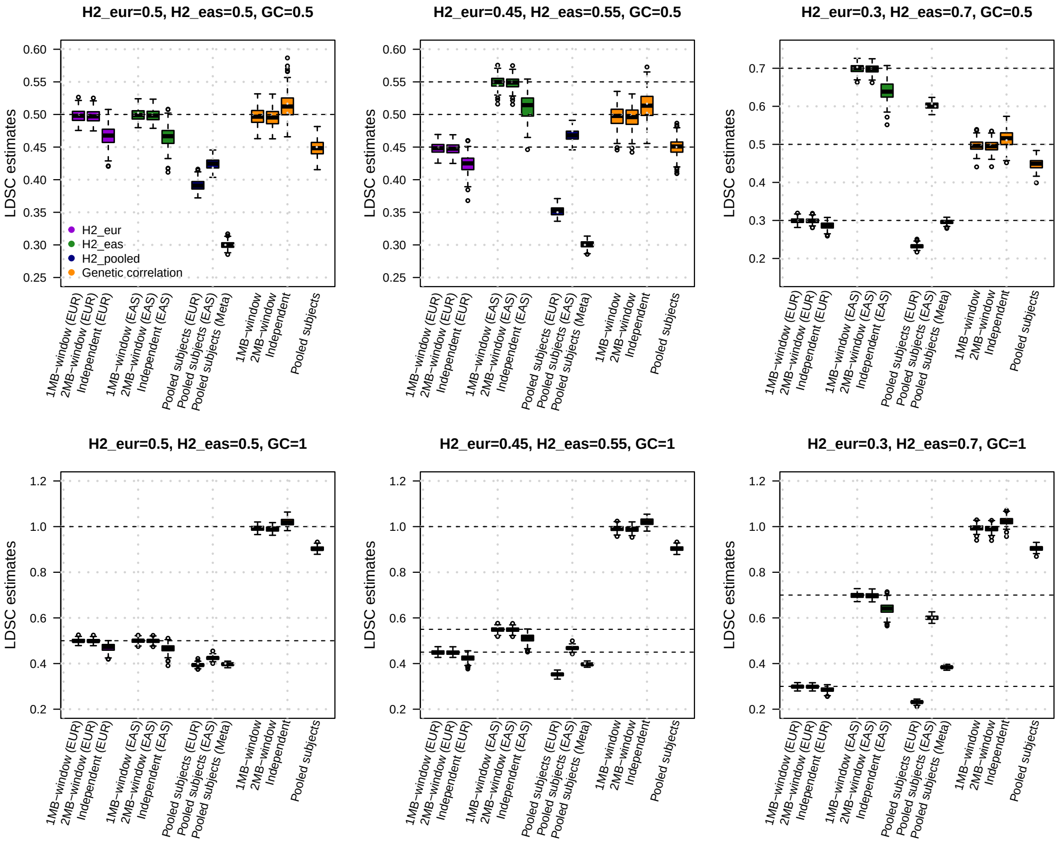


SUPPLEMENTARY FIG. 14. *LDSC estimators across different heritability and genetic correlation levels in HAPNEST simulation analysis. We set the heritability* $h^2_{eur} = h^2_{eas} = 0.5$ *in the left panels, and make them different in the middle* ($h^2_{eur} = 0.45$, $h^2_{eas} = 0.55$) *and right panels* ($h^2_{eur} = 0.3$, $h^2_{eas} = 0.7$)*. We simulate the data with* $n_\alpha = n_\beta = 168{,}000$ *and the proportion of causal variants being* $3\%$*. The genetic correlation (GC) is* $0.5$ *and* $1$ *in the upper and bottom panels, respectively. In each panel, we show the estimates of heritability and genetic correlation in different colors. The horizontal line represents the true heritability and genetic correlation values.*

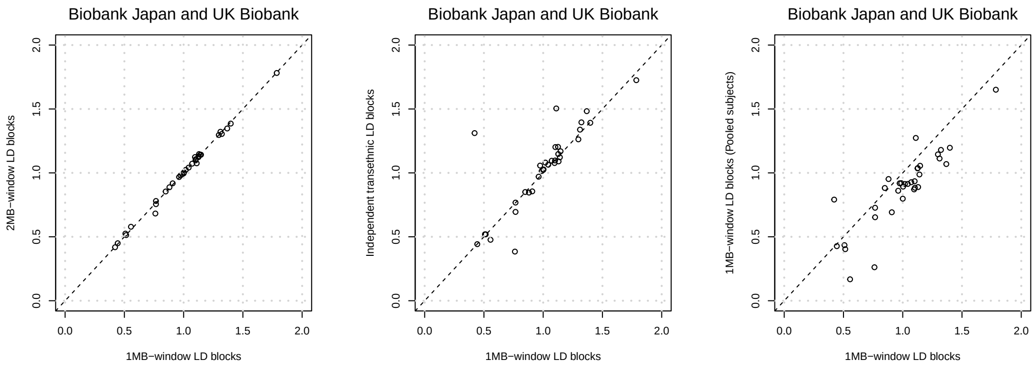


SUPPLEMENTARY FIG. 15. *Cross-ancestry genetic correlation between 34 pairs of matched phenotypes in Biobank Japan and UK Biobank. We compare the estimates from four methods used in the simulation analysis: "1MB-Window", "2MB-Window", "Independent", and "Pooled subjects".*

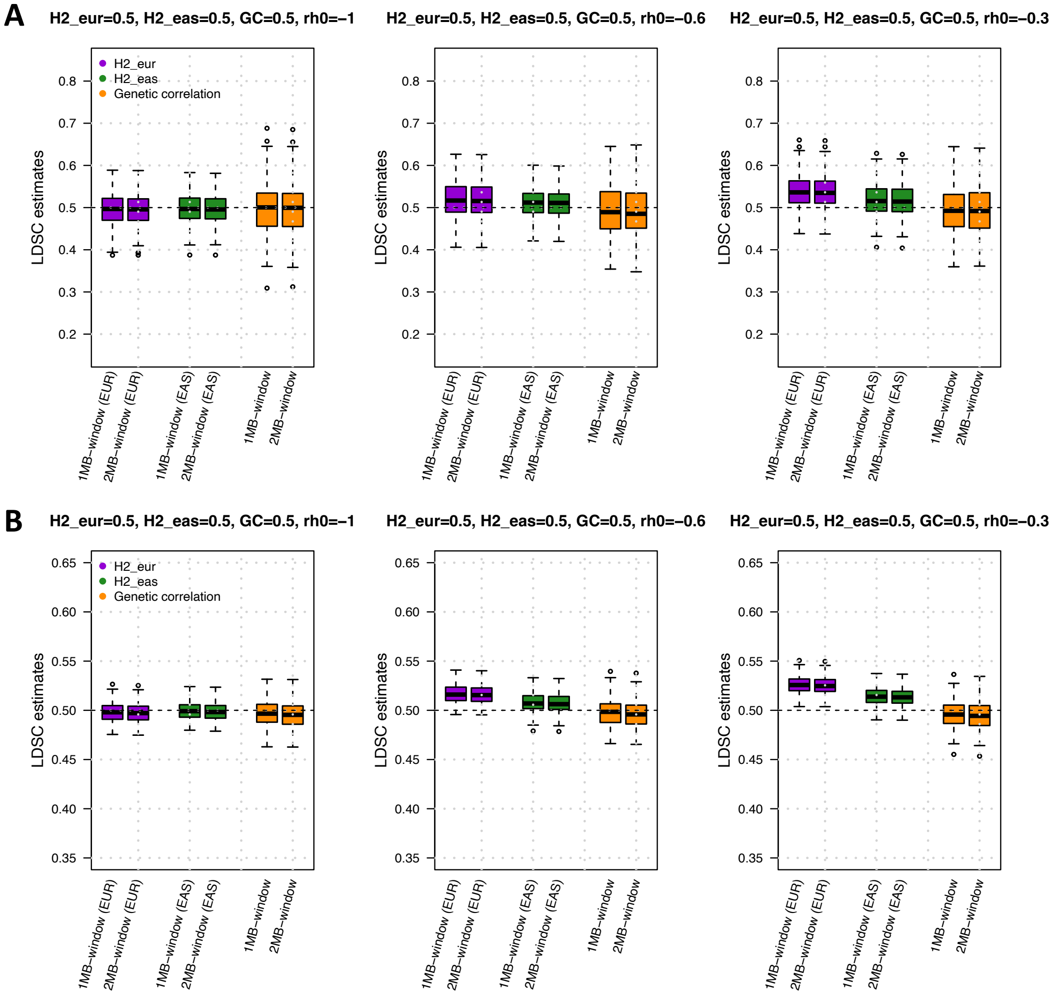


SUPPLEMENTARY FIG. 16. *LDSC estimators across different negative selection levels with MAF-dependence genetic architecture. We set the heritability* $h^2_{eur} = h^2_{eas} = 0.5$ *and genetic correlation (GC) is* $0.5$*. From left to right, we set* $\rho = -1, -0.6,$ *and* $-0.3$*. The sample size is* $n_\alpha = n_\beta = 16{,}800$ *in upper panels (A) and* $n_\alpha = n_\beta = 168{,}000$ *in bottom panels (B). Other settings remain the same as the HAPNEST simulation analysis. In each panel, we show the estimates of heritability and genetic correlation in different colors. The horizontal line represents the true heritability and genetic correlation values.*

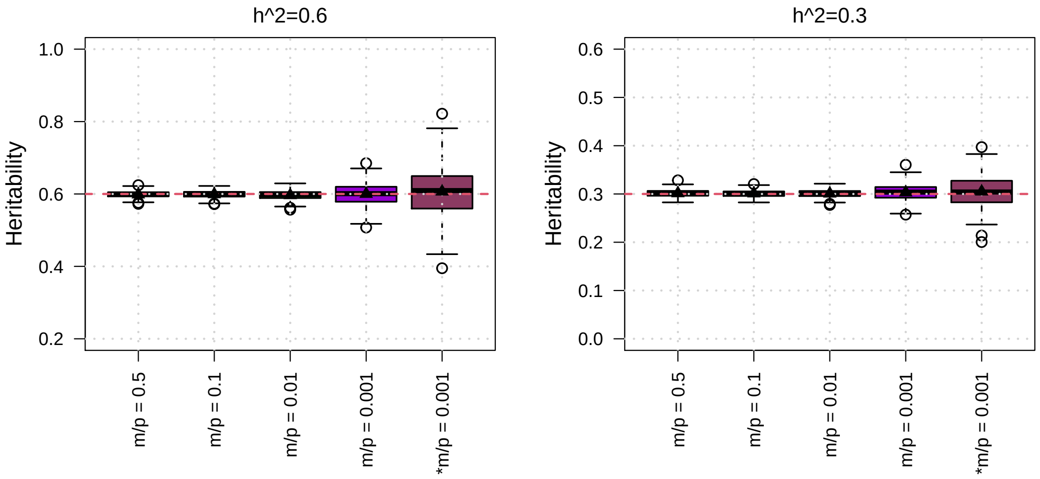


SUPPLEMENTARY FIG. 17. *Univariate LDSC estimator across different signal sparsity ($m/p$) and heritability level in the UK Biobank data simulation. We report the results of heritability, which is closely related to genetic variance. We set the heritability $h_\alpha^2 = 0.6$ and $0.3$ in the left and right panels, respectively. We simulate the data with $n_\alpha = 175{,}000$. In each panel, the last column with an asterisk label indicates the version of LDSC estimates obtained using only the genetic variants known to have a nonzero genetic effect. The horizontal line represents the true heritability.*

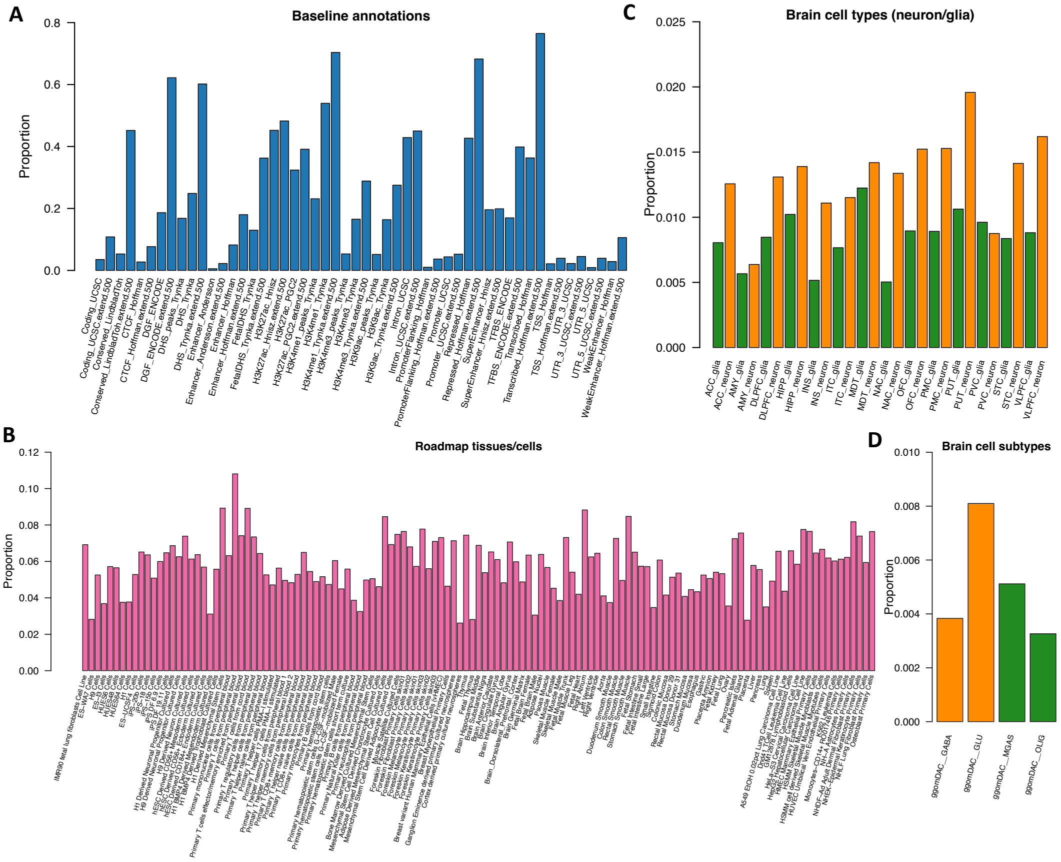


SUPPLEMENTARY FIG. 18. *Illustration of the sizes of functional annotations. We show the proportion of genetic variants covered by each annotation. It is recommended that stratified LDSC analyses are generally suitable for large annotations encompassing over* 0.5% *of genetic variants [41]. (A): baseline functional annotations provided by [14]; (B): tissue and cell type-specific regulatory elements from the Roadmap Epigenomics Consortium [24]; (C): chromatin accessibility data from neurons and glia sampled from 14 cortical and subcortical brain regions [15]; and (D): chromatin accessibility of two neuron subtypes (GABAergic and glutamatergic neurons) and two glial subtypes (oligodendrocyte and microglia) [20].*

# REFERENCES


[1] 1000-GENOMES-CONSORTIUM (2015). A global reference for human genetic variation. *Nature* **526** 68–74.

[2] BONNET, A., LÉVY-LEDUC, C., GASSIAT, E., TORO, R. and BOURGERON, T. (2018). Improving heritability estimation by a variable selection approach in sparse high dimensional linear mixed models. *Journal of the Royal Statistical Society Series C: Applied Statistics* **67** 813–839.

[3] BOYLE, A. P., HONG, E. L., HARIHARAN, M., CHENG, Y., SCHAUB, M. A., KASOWSKI, M., KARCZEWSKI, K. J., PARK, J., HITZ, B. C., WENG, S. et al. (2012). Annotation of functional variation in personal genomes using RegulomeDB. *Genome Research* **22** 1790–1797.

[4] BROWN, B. C., ASIAN GENETIC EPIDEMIOLOGY NETWORK TYPE 2 DIABETES CONSORTIUM, YE, C. J., PRICE, A. L. and ZAITLEN, N. (2016). Transethnic genetic-correlation estimates from summary statistics. *The American Journal of Human Genetics* **99** 76–88.

[5] BULIK-SULLIVAN, B., FINUCANE, H. K., ANTTILA, V., GUSEV, A., DAY, F. R., LOH, P.-R., DUNCAN, L., PERRY, J. R., PATTERSON, N., ROBINSON, E. B. et al. (2015). An atlas of genetic correlations across human diseases and traits. *Nature Genetics* **47** 1236-1241.

[6] BULIK-SULLIVAN, B. K., LOH, P.-R., FINUCANE, H. K., RIPKE, S., YANG, J., PATTERSON, N., DALY, M. J., PRICE, A. L., NEALE, B. M., OF THE PSYCHIATRIC GENOMICS CONSORTIUM, S. W. G. et al. (2015). LD Score regression distinguishes confounding from polygenicity in genome-wide association studies. *Nature Genetics* **47** 291-295.

[7] BYCROFT, C., FREEMAN, C., PETKOVA, D., BAND, G., ELLIOTT, L., SHARP, K., MOTYER, A., VUKCEVIC, D., DELANEAU, O., O'CONNELL, J. et al. (2018). The UK Biobank resource with deep phenotyping and genomic data. *Nature* **562** 203–209.

[8] CALDERON, D., BHASKAR, A., KNOWLES, D. A., GOLAN, D., RAJ, T., FU, A. Q. and PRITCHARD, J. K. (2017). Inferring relevant cell types for complex traits by using single-cell gene expression. *The American Journal of Human Genetics* **101** 686–699.

[9] CHATTERJEE, S. (2009). Fluctuations of eigenvalues and second order Poincaré inequalities. *Probability Theory and Related Fields* **143** 1–40.

[10] CHRISTENSEN, R. (2015). Covariance of the Wishart distribution with applications to regression. *Department of Mathematics and of Statistics, University of New Mexico*.

[11] DICKER, L. H. (2014). Variance estimation in high-dimensional linear models. *Biometrika* **101** 269–284.

[12] EMANI, P. S., LIU, J. J., CLARKE, D., JENSEN, M., WARRELL, J., GUPTA, C., MENG, R., LEE, C. Y., XU, S., DURSUN, C. et al. (2024). Single-cell genomics and regulatory networks for 388 human brains. *Science* **384** eadi5199.

[13] FINUCANE, H. K., BULIK-SULLIVAN, B., GUSEV, A., TRYNKA, G., RESHEF, Y., LOH, P.-R., ANTTILA, V., XU, H., ZANG, C., FARH, K. et al. (2015). Partitioning heritability by functional annotation using genome-wide association summary statistics. *Nature Genetics* **47** 1228–1235.

[14] FINUCANE, H. K., RESHEF, Y. A., ANTTILA, V., SLOWIKOWSKI, K., GUSEV, A., BYRNES, A., GAZAL, S., LOH, P.-R., LAREAU, C., SHORESH, N. et al. (2018). Heritability enrichment of specifically expressed genes identifies disease-relevant tissues and cell types. *Nature Genetics* **50** 621–629.

[15] FULLARD, J. F., HAUBERG, M. E., BENDL, J., EGERVARI, G., CIRNARU, M.-D., REACH, S. M., MOTL, J., EHRLICH, M. E., HURD, Y. L. and ROUSSOS, P. (2018). An atlas of chromatin accessibility in the adult human brain. *Genome Research* **28** 1243–1252.

[16] GOLAN, D., LANDER, E. S. and ROSSET, S. (2014). Measuring missing heritability: Inferring the contribution of common variants. *Proceedings of the National Academy of Sciences* **111** E5272–E5281.

[17] GUO, H., LI, J. J., LU, Q. and HOU, L. (2021). Detecting local genetic correlations with scan statistics. *Nature Communications* **12** 2033.

[18] GUO, Z., WANG, W., CAI, T. T. and LI, H. (2019). Optimal estimation of genetic relatedness in high-dimensional linear models. *Journal of the American Statistical Association* **114** 358–369.

[19] HASEMAN, J. K. and ELSTON, R. C. (1972). The investigation of linkage between a quantitative trait and a marker locus. *Behavior Genetics* **2** 3–19.

[20] HAUBERG, M. E., CREUS-MUNCUNILL, J., BENDL, J., KOZLENKOV, A., ZENG, B., CORWIN, C., CHOWDHURY, S., KRANZ, H., HURD, Y. L., WEGNER, M. et al. (2020). Common schizophrenia risk variants are enriched in open chromatin regions of human glutamatergic neurons. *Nature Communications* **11** 5581.

[21] HOU, K., BURCH, K. S., MAJUMDAR, A., SHI, H., MANCUSO, N., WU, Y., SANKARARAMAN, S. and PASANIUC, B. (2019). Accurate estimation of SNP-heritability from biobank-scale data irrespective of genetic architecture. *Nature Genetics* **51** 1244–1251.

[22] JAGADEESH, K. A., DEY, K. K., MONTORO, D. T., MOHAN, R., GAZAL, S., ENGREITZ, J. M., XAVIER, R. J., PRICE, A. L. and REGEV, A. (2022). Identifying disease-critical cell types and cellular processes by integrating single-cell RNA-sequencing and human genetics. *Nature Genetics* **54** 1479–1492.

[23] JERBY-ARNON, L. and REGEV, A. (2022). DIALOGUE maps multicellular programs in tissue from single-cell or spatial transcriptomics data. *Nature Biotechnology* **40** 1467–1477.

[24] KUNDAJE, A., MEULEMAN, W., ERNST, J., BILENKY, M., YEN, A., HERAVI-MOUSSAVI, A., KHERADPOUR, P., ZHANG, Z., WANG, J., ZILLER, M. J. et al. (2015). Integrative analysis of 111 reference human epigenomes. *Nature* **518** 317–330.

[25] LI, H., MAZUMDER, R. and LIN, X. (2023). Accurate and efficient estimation of local heritability using summary statistics and the linkage disequilibrium matrix. *Nature Communications* **14** 7954.

[26] LU, Q., LI, B., OU, D., ERLENDSDOTTIR, M., POWLES, R. L., JIANG, T., HU, Y., CHANG, D., JIN, C., DAI, W. et al. (2017). A powerful approach to estimating annotation-stratified genetic covariance via GWAS summary statistics. *The American Journal of Human Genetics* **101** 939–964.

[27] MA, R. and DICKER, L. H. (2019). The Mahalanobis kernel for heritability estimation in genome-wide association studies: fixed-effects and random-effects methods. *arXiv preprint arXiv:1901.02936*.

[28] MOMIN, M. M., SHIN, J., LEE, S., TRUONG, B., BENYAMIN, B. and LEE, S. H. (2023). A method for an unbiased estimate of cross-ancestry genetic correlation using individual-level data. *Nature Communications* **14** 722.

[29] NING, Z., PAWITAN, Y. and SHEN, X. (2020). High-definition likelihood inference of genetic correlations across human complex traits. *Nature Genetics* **52** 859–864.

[30] O'DONNELL, R. (2014). *Analysis of boolean functions*. Cambridge University Press.

[31] PALMER, D. S., ZHOU, W., ABBOTT, L., WIGDOR, E. M., BAYA, N., CHURCHHOUSE, C., SEED, C., POTERBA, T., KING, D., KANAI, M. et al. (2023). Analysis of genetic dominance in the UK Biobank. *Science* **379** 1341–1348.

[32] SAKAUE, S., KANAI, M., TANIGAWA, Y., KARJALAINEN, J., KURKI, M., KOSHIBA, S., NARITA, A., KONUMA, T., YAMAMOTO, K., AKIYAMA, M. et al. (2021). A cross-population atlas of genetic associations for 220 human phenotypes. *Nature Genetics* **53** 1415–1424.

[33] SCHOECH, A. P., JORDAN, D. M., LOH, P.-R., GAZAL, S., O'CONNOR, L. J., BALICK, D. J., PALAMARA, P. F., FINUCANE, H. K., SUNYAEV, S. R. and PRICE, A. L. (2019). Quantification of frequency-dependent genetic architectures in 25 UK Biobank traits reveals action of negative selection. *Nature Communications* **10** 790.

[34] SCHWARTZMAN, A., SCHORK, A. J., ZABLOCKI, R. and THOMPSON, W. K. (2019). A simple, consistent estimator of SNP heritability from genome-wide association studies. *The Annals of Applied Statistics* **13** 2509.

[35] SHI, H., KICHAEV, G. and PASANIUC, B. (2016). Contrasting the genetic architecture of 30 complex traits from summary association data. *The American Journal of Human Genetics* **99** 139–153.

[36] SHI, H., MANCUSO, N., SPENDLOVE, S. and PASANIUC, B. (2017). Local genetic correlation gives insights into the shared genetic architecture of complex traits. *The American Journal of Human Genetics* **101** 737–751.

[37] SKENE, N. G. and GRANT, S. G. (2016). Identification of vulnerable cell types in major brain disorders using single cell transcriptomes and expression weighted cell type enrichment. *Frontiers in Neuroscience* **10** 16.

[38] SMITH, S. P., DARNELL, G., UDWIN, D., HARPAK, A., RAMACHANDRAN, S. and CRAWFORD, L. (2023). Accounting for statistical non-additive interactions enables the recovery of missing heritability from GWAS summary statistics. *bioRxiv*. https://doi.org/10.1101/2022.07.21.501001

[39] SONG, S., JIANG, W., ZHANG, Y., HOU, L. and ZHAO, H. (2022). Leveraging LD eigenvalue regression to improve the estimation of SNP heritability and confounding inflation. *The American Journal of Human Genetics* **109** 802–811.

[40] SPEED, D. and BALDING, D. (2019). SumHer better estimates the SNP heritability of complex traits from summary statistics. *Nature Genetics* **51** 277–284.

[41] TASHMAN, K. C., CUI, R., O'CONNOR, L. J., NEALE, B. M. and FINUCANE, H. K. (2021). Significance testing for small annotations in stratified LD-Score regression. *medRxiv*. https://doi.org/10.1101/2021.03.13.21249938

[42] TIMSHEL, P. N., THOMPSON, J. J. and PERS, T. H. (2020). Genetic mapping of etiologic brain cell types for obesity. *Elife* **9** e55851.

[43] TONY CAI, T. and GUO, Z. (2020). Semisupervised inference for explained variance in high dimensional linear regression and its applications. *Journal of the Royal Statistical Society Series B: Statistical Methodology* **82** 391–419.

[44] VERSHYNIN, R. (2012). *Introduction to the non-asymptotic analysis of random matrices* In *Compressed Sensing: Theory and Applications* 210–268. Cambridge University Press. https://doi.org/10.1017/CBO9780511794308.006

[45] WANG, J. and LI, H. (2022). Estimation of genetic correlation with summary association statistics. *Biometrika* **109** 421–438.

[46] WANG, R., LIN, D.-Y. and JIANG, Y. (2022). EPIC: Inferring relevant cell types for complex traits by integrating genome-wide association studies and single-cell RNA sequencing. *PLoS Genetics* **18** e1010251.

[47] WATANABE, K., UMIĆEVIĆ MIRKOV, M., DE LEEUW, C. A., VAN DEN HEUVEL, M. P. and POSTHUMA, D. (2019). Genetic mapping of cell type specificity for complex traits. *Nature Communications* **10** 3222.

[48] WERME, J., VAN DER SLUIS, S., POSTHUMA, D. and DE LEEUW, C. A. (2022). An integrated framework for local genetic correlation analysis. *Nature Genetics* **54** 274–282.

[49] YANG, J., LEE, S. H., GODDARD, M. E. and VISSCHER, P. M. (2011). GCTA: a tool for genome-wide complex trait analysis. *The American Journal of Human Genetics* **88** 76–82.

[50] ZHANG, C., ZHANG, Y., ZHANG, Y. and ZHAO, H. (2023). Benchmarking of local genetic correlation estimation methods using summary statistics from genome-wide association studies. *Briefings in Bioinformatics* **24** bbad407.

[51] ZHANG, M. J., HOU, K., DEY, K. K., SAKAUE, S., JAGADEESH, K. A., WEINAND, K., TAYCHAMEEKIATCHAI, A., RAO, P., PISCO, A. O., ZOU, J. et al. (2022). Polygenic enrichment distinguishes disease associations of individual cells in single-cell RNA-seq data. *Nature Genetics* **54** 1572–1580.

[52] ZHANG, Y., LU, Q., YE, Y., HUANG, K., LIU, W., WU, Y., ZHONG, X., LI, B., YU, Z., TRAVERS, B. G. et al. (2021). SUPERGNOVA: local genetic correlation analysis reveals heterogeneous etiologic sharing of complex traits. *Genome Biology* **22** 1–30.

[53] ZHAO, B., YANG, X. and ZHU, H. (2022). Estimating trans-ancestry genetic correlation with unbalanced data resources. *arXiv preprint arXiv:2203.12154*.

[54] ZHAO, B. and ZHU, H. (2019). Cross-trait prediction accuracy of high-dimensional ridge-type estimators in genome-wide association studies. *arXiv preprint arXiv:1911.10142*.

[55] ZHAO, B. and ZHU, H. (2022). On genetic correlation estimation with summary statistics from genome-wide association studies. *Journal of the American Statistical Association* **117** 1–11.

[56] ZHOU, X. (2017). A unified framework for variance component estimation with summary statistics in genome-wide association studies. *The Annals of Applied Statistics* **11** 2027-2051.
